# Supplementary material for: Decays of an exotic $1^{-+}$ hybrid meson resonance in QCD
Source: arXiv:2009.10034 ancillary file (2021-03-22)
Supplement: Supplementary file 1 [file supplemental.pdf]

**Supplemental Material**  
 **$J^{P(C)} = 1^{-(+)}$  Amplitudes**

In this supplemental material, for each parameterisation of the eight  $J^{P(C)} = 1^{-(+)}$  coupled channels that gave a reasonable description of the computed finite-volume energy levels, we present the scattering parameters along with the statistical uncertainties and correlations. We also give the location of pole singularities found on the proximal sheet and the corresponding pole couplings, and additional figures showing the finite-volume spectrum, magnitude-squared amplitudes, and poles and couplings for each parameterisation.

All amplitudes are of the form,

$$K_{\ell S J a, \ell' S' J b} = \frac{(g_{\ell S J a}^{(0)} + g_{\ell S J a}^{(1)} s)(g_{\ell' S' J b}^{(0)} + g_{\ell' S' J b}^{(1)} s)}{m^2 - s} + \gamma_{\ell S J a, \ell' S' J b}^{(0)} + \gamma_{\ell S J a, \ell' S' J b}^{(1)} s, \quad (0.1)$$

and parameterisations differ by the restrictions we apply to  $g^{(0)}, g^{(1)}, \gamma^{(0)}$  and  $\gamma^{(1)}$ , and differences in the phase-space prescription. For brevity, we label the different parameterisation by a shorthand that represents the parameters not fixed to be zero in Eq. 0.1 and hence are allowed to freely vary under the minimisation routine described in the manuscript. We also include a label to identify the phase-space prescription. The shorthand we will use for identifying the channels is given by the following map:

$$\begin{aligned} \eta^1 \eta^8 \{^1 P_1\} &\longrightarrow \mathbf{a} \\ \omega^8 \eta^8 \{^3 P_1\} &\longrightarrow \mathbf{b} \\ \omega^8 \omega^8 \{^3 P_1\} &\longrightarrow \mathbf{c} \\ \omega^1 \omega^8 \{^1 P_1\} &\longrightarrow \mathbf{d}_1 \\ \omega^1 \omega^8 \{^3 P_1\} &\longrightarrow \mathbf{d}_2 \\ \omega^1 \omega^8 \{^5 P_1\} &\longrightarrow \mathbf{d}_3 \\ f_1^8 \eta^8 \{^3 S_1\} &\longrightarrow \mathbf{e} \\ h_1^8 \eta^8 \{^3 S_1\} &\longrightarrow \mathbf{f}. \end{aligned}$$

Therefore, if our amplitude has freedom in the parameter  $g_{\eta^1 \eta^8 \{^1 P_1\}}^{(0)}$ , the label for that amplitude will contain the reference  $g_{\mathbf{a}}^{(0)}$ . We shall indicate multiple non-zero parameters by a comma separated list on the subscript, e.g.  $g_{\mathbf{a}, \mathbf{b}, \mathbf{d}_1}^{(0)}$ . The  $\gamma$  matrix components are similarly represented, for example  $\gamma_{\eta^1 \eta^8 \{^1 P_1\}, \omega^8 \eta^8 \{^3 P_1\}}^{(0)}$  would be denoted by  $\gamma_{(\mathbf{a}, \mathbf{b})}^{(0)}$ . Again, we augment the subscript to include additional non-zero parameters by introducing a comma separated list, e.g.  $\gamma_{(\mathbf{a}, \mathbf{a}), (\mathbf{a}, \mathbf{b})}^{(0)}$ . All parameterisation have a freely varying mass parameter  $m$  that we will include in the label to make clear the total number of degrees of freedom. The notation for the three phase-space prescriptions is

$$\begin{aligned} \text{Chew-Mandelstam phase space with } \text{Re}\{I_a(s = m^2) = 0\} &\longrightarrow \text{CM}_m \\ \text{Chew-Mandelstam phase space with } \text{Re}\{I_a(s = s_a^{\text{thr}}) = 0\} &\longrightarrow \text{CM}_{\text{thr}} \\ I_a(s) = -i\rho_a(s) &\longrightarrow -i\rho. \end{aligned}$$

As a concrete example, the reference  $J^{P(C)} = 1^{-(+)}$  amplitude used in Section V.A is labelled:

$$\{m, g_{\mathbf{a}, \mathbf{b}, \mathbf{e}, \mathbf{f}}^{(0)}, \gamma_{(\mathbf{a}, \mathbf{a}), (\mathbf{b}, \mathbf{b}), (\mathbf{c}, \mathbf{c}), (\mathbf{d}_1, \mathbf{d}_1), (\mathbf{d}_2, \mathbf{d}_2), (\mathbf{d}_3, \mathbf{d}_3)}^{(0)}\}(\text{CM}_m),$$

and we clearly see that there are 11 free parameters.

The scattering parameter names that are displayed in the fit output for each amplitude also have labels that reflect the corresponding element of the  $K$ -matrix. These are self explanatory, but to be explicit we present some illustrative examples:

- `g_eta8:eta1/1^P_1_pole0` or `g_eta8:eta1/1^P_1_pole0_order0`  
corresponds to  $g_{\eta^1\eta^s\{^1P_1\}}^{(0)} = g_a^{(0)}$
- `g_eta8:eta1/1^P_1_pole0_order1`  
corresponds to  $g_{\eta^1\eta^s\{^1P_1\}}^{(1)} = g_a^{(1)}$
- `gamma_eta8:eta1/1^P_1|omega8:eta8/3^P_1_order0`  
corresponds to  $\gamma_{\eta^1\eta^s\{^1P_1\},\omega^s\eta^s\{^3P_1\}}^{(0)} = \gamma_{(a,b)}^{(0)}$
- `gamma_eta8:eta1/1^P_1|omega8:eta8/3^P_1_order1`  
corresponds to  $\gamma_{\eta^1\eta^s\{^1P_1\},\omega^s\eta^s\{^3P_1\}}^{(1)} = \gamma_{(a,b)}^{(1)}$
- `m_pole0`  
corresponds to  $m$ .

The different phase-space prescriptions are denoted

- `pole0_sub`  
 $\longrightarrow$  Chew-Mandelstam phase space with  $\text{Re}\{I_a(s = m^2) = 0\}$
- `threshold_sub`  
 $\longrightarrow$  Chew-Mandelstam phase space with  $\text{Re}\{I_a(s = s_a^{\text{thr}}) = 0\}$
- `irho_sub`  
 $\longrightarrow I_a(s) = -i\rho_a(s)$ .

# Contents

|          |                                                                                                                                    |          |
|----------|------------------------------------------------------------------------------------------------------------------------------------|----------|
| <b>1</b> | <b>Successful Parameterizations</b>                                                                                                | <b>6</b> |
| 1.1      | $\{m, g_{a,b,e,f}^{(0)}, \gamma_{(a,a),(b,b),(c,c),(d_1,d_1),(d_2,d_2),(d_3,d_3),(e,e)}^{(0)}\}(\text{CM}_m)$                      | 6        |
| 1.2      | $\{m, g_{b,f}^{(0)}, \gamma_{(a,a),(b,b),(c,c),(d_1,d_1),(d_2,d_2),(d_3,d_3),(e,e)}^{(0)}\}(\text{CM}_m)$                          | 11       |
| 1.3      | $\{m, g_{a,e,f}^{(0)}, \gamma_{(a,a),(b,b),(c,c),(d_1,d_1),(d_2,d_2),(d_3,d_3),(e,e)}^{(0)}\}(\text{CM}_m)$                        | 16       |
| 1.4      | $\{m, g_{a,b,c,f}^{(0)}, \gamma_{(a,a),(b,b),(c,c),(d_1,d_1),(d_2,d_2),(d_3,d_3),(e,e)}^{(0)}\}(\text{CM}_m)$                      | 21       |
| 1.5      | $\{m, g_{a,b,d_2,f}^{(0)}, \gamma_{(a,a),(b,b),(c,c),(d_1,d_1),(d_2,d_2),(d_3,d_3),(e,e)}^{(0)}\}(\text{CM}_m)$                    | 26       |
| 1.6      | $\{m, g_{a,b,d_1,d_2,d_3,f}^{(0)}, \gamma_{(a,a),(b,b),(c,c),(d_1,d_1),(d_2,d_2),(d_3,d_3),(e,e)}^{(0)}\}(\text{CM}_m)$            | 31       |
| 1.7      | $\{m, g_{a,b,c,d_1,d_2,d_3,f}^{(0)}, \gamma_{(a,a),(b,b),(c,c),(d_1,d_1),(d_2,d_2),(d_3,d_3),(e,e)}^{(0)}\}(\text{CM}_m)$          | 36       |
| 1.8      | $\{m, g_f^{(0)}, \gamma_{(a,a),(b,b),(c,c),(d_1,d_1),(d_2,d_2),(d_3,d_3),(e,e)}^{(0)}\}(\text{CM}_m)$                              | 41       |
| 1.9      | $\{m, g_{a,b,f}^{(0)}, \gamma_{(a,a),(b,b),(c,c),(d_1,d_1),(d_2,d_2),(d_3,d_3),(e,e)}^{(0)}\}(\text{CM}_m)$                        | 46       |
| 1.10     | $\{m, g_{a,b,f}^{(0)}, \gamma_{(a,a),(b,b),(c,c),(d_1,d_1),(d_2,d_2),(d_3,d_3),(e,e),(f,f)}^{(0)}\}(\text{CM}_m)$                  | 51       |
| 1.11     | $\{m, g_{a,b,f}^{(0)}, \gamma_{(b,b),(c,c),(d_1,d_1),(d_2,d_2),(d_3,d_3),(e,e),(f,f)}^{(0)}\}(\text{CM}_m)$                        | 56       |
| 1.12     | $\{m, g_{a,b,f}^{(0)}, \gamma_{(b,b),(c,c),(d_1,d_1),(d_2,d_2),(d_3,d_3),(e,e)}^{(0)}\}(\text{CM}_m)$                              | 61       |
| 1.13     | $\{m, g_{a,b,e,f}^{(0)}, \gamma_{(a,a),(b,b),(c,c),(d_1,d_1),(d_2,d_2),(d_3,d_3)}^{(0)}\}(\text{CM}_m)$                            | 66       |
| 1.14     | $\{m, g_{a,b,c,f}^{(0)}, \gamma_{(a,a),(b,b),(c,c),(d_1,d_1),(d_2,d_2),(d_3,d_3),(e,e)}^{(0)}\}(\text{CM}_{\text{thr}})$           | 71       |
| 1.15     | $\{m, g_f^{(0)}, \gamma_{(a,a),(b,b),(c,c),(d_1,d_1),(d_2,d_2),(d_3,d_3),(e,e)}^{(0)}\}(\text{CM}_{\text{thr}})$                   | 76       |
| 1.16     | $\{m, g_{a,b,f}^{(0)}, \gamma_{(a,a),(b,b),(c,c),(d_1,d_1),(d_2,d_2),(d_3,d_3),(e,e),(f,f)}^{(0)}\}(\text{CM}_{\text{thr}})$       | 81       |
| 1.17     | $\{m, g_{a,b,e,f}^{(0)}, \gamma_{(a,a),(b,b),(c,c),(d_1,d_1),(d_2,d_2),(d_3,d_3)}^{(0)}\}(\text{CM}_{\text{thr}})$                 | 86       |
| 1.18     | $\{m, g_{a,b,e,f}^{(0)}, \gamma_{(a,a),(b,b),(c,c),(d_1,d_1),(d_2,d_2),(d_3,d_3)}^{(0)}\}(-i\rho)$                                 | 91       |
| 1.19     | $\{m, g_{a,b,f}^{(0)}, \gamma_{(a,a),(b,b),(b,f),(c,c),(d_1,d_1),(d_2,d_2),(d_3,d_3),(e,e),(f,f)}^{(0)}\}(\text{CM}_m)$            | 96       |
| 1.20     | $\{m, g_{a,b,e,f}^{(0)}, \gamma_{(a,a),(b,b),(c,c),(d_1,d_1),(d_2,d_2),(d_3,d_3),(e,f)}^{(0)}\}(\text{CM}_m)$                      | 101      |
| 1.21     | $\{m, g_{a,b,f}^{(0)}, \gamma_{(a,a),(b,b),(b,f),(c,c),(d_1,d_1),(d_2,d_2),(d_3,d_3),(e,e),(f,f)}^{(0)}\}(\text{CM}_{\text{thr}})$ | 106      |
| 1.22     | $\{m, g_{a,b,f}^{(0)}, \gamma_{(a,a),(b,b),(c,c),(d_1,d_1),(d_2,d_2),(d_3,d_3),(e,e)}, \gamma_{(a,a)}^{(1)}\}(\text{CM}_m)$        | 111      |
| 1.23     | $\{m, g_{a,b,f}^{(0)}, \gamma_{(a,a),(b,b),(c,c),(d_1,d_1),(d_2,d_2),(d_3,d_3),(e,e)}, \gamma_{(a,b)}^{(1)}\}(\text{CM}_m)$        | 116      |
| 1.24     | $\{m, g_{a,b,f}^{(0)}, g_f^{(1)}, \gamma_{(a,a),(b,b),(c,c),(d_1,d_1),(d_2,d_2),(d_3,d_3),(e,e)}^{(0)}\}(\text{CM}_m)$             | 121      |
| 1.25     | $\{m, g_{a,b,f}^{(0)}, g_a^{(1)}, \gamma_{(a,a),(b,b),(c,c),(d_1,d_1),(d_2,d_2),(d_3,d_3),(e,e)}^{(0)}\}(\text{CM}_m)$             | 126      |

|      |                                                                                                                                                                                    |     |
|------|------------------------------------------------------------------------------------------------------------------------------------------------------------------------------------|-----|
| 1.26 | $\{m, g_{a,b,f}^{(0)}, g_b^{(1)}, \gamma_{(a,a),(b,b),(c,c),(\mathfrak{d}_1,\mathfrak{d}_1),(\mathfrak{d}_2,\mathfrak{d}_2),(\mathfrak{d}_3,\mathfrak{d}_3),(c,c)}\}(\text{CM}_m)$ | 131 |
| 1.27 | $\{m, g_{a,b}^{(0)}, g_f^{(1)}, \gamma_{(a,a),(b,b),(c,c),(\mathfrak{d}_1,\mathfrak{d}_1),(\mathfrak{d}_2,\mathfrak{d}_2),(\mathfrak{d}_3,\mathfrak{d}_3),(c,c)}\}(\text{CM}_m)$   | 136 |

# 1 Successful Parameterizations

## 1.1 $\{m, g_{a,b,c,f}^{(0)}, \gamma_{(a,a),(b,b),(c,c),(\partial_1,\partial_1),(\partial_2,\partial_2),(\partial_3,\partial_3),(\epsilon,\epsilon)}\}(\mathbf{CM}_m)$

minimised with  $\text{chisq}/\text{nDoF} = 45.49 / (53 - 12) = 1.11$

|                                                           |  |                        |  |      |      |      |      |      |      |       |       |       |       |       |       |
|-----------------------------------------------------------|--|------------------------|--|------|------|------|------|------|------|-------|-------|-------|-------|-------|-------|
| =====                                                     |  |                        |  |      |      |      |      |      |      |       |       |       |       |       |       |
| JP1-_g_eta8:eta1/1^P_1_pole0                              |  | 0.20814 +/- 0.16033    |  | 1.00 | 0.00 | 0.78 | 0.70 | 0.13 | 0.29 | -0.02 | -0.03 | 0.02  | -0.06 | -0.06 | 0.64  |
| JP1-_g_f8:eta8/3^S_1_pole0                                |  | 9.5963e-05 +/- 0.58084 |  |      | 1.00 | 0.00 | 0.00 | 0.00 | 0.00 | -0.00 | -0.00 | -0.00 | -0.00 | -0.00 | 0.00  |
| JP1-_g_h8:eta8/3^S_1_pole0                                |  | 0.85358 +/- 0.66629    |  |      |      | 1.00 | 0.90 | 0.31 | 0.43 | -0.08 | -0.00 | 0.06  | -0.00 | -0.01 | 0.51  |
| JP1-_g_omega8:eta8/3^P_1_pole0                            |  | 0.27398 +/- 0.19978    |  |      |      |      | 1.00 | 0.30 | 0.39 | -0.30 | 0.02  | 0.05  | 0.01  | 0.01  | 0.39  |
| JP1-_gamma_eta8:eta1/1^P_1 eta8:eta1/1^P_1_order0         |  | 1.4402 +/- 0.57091     |  |      |      |      |      | 1.00 | 0.55 | -0.02 | 0.02  | 0.06  | 0.03  | 0.02  | -0.02 |
| JP1-_gamma_f8:eta8/3^S_1 f8:eta8/3^S_1_order0             |  | -2.1029 +/- 0.30783    |  |      |      |      |      |      | 1.00 | 0.00  | 0.03  | 0.08  | 0.03  | 0.04  | 0.14  |
| JP1-_gamma_omega8:eta8/3^P_1 omega8:eta8/3^P_1_order0     |  | -3.5752 +/- 0.62221    |  |      |      |      |      |      |      | 1.00  | 0.05  | 0.08  | 0.06  | 0.13  | 0.11  |
| JP1-_gamma_omega8:omega1/1^P_1 omega8:omega1/1^P_1_order0 |  | 9.5770 +/- 2.3634      |  |      |      |      |      |      |      |       | 1.00  | 0.06  | 0.39  | 0.43  | -0.06 |
| JP1-_gamma_omega8:omega1/3^P_1 omega8:omega1/3^P_1_order0 |  | 12.067 +/- 4.9321      |  |      |      |      |      |      |      |       |       | 1.00  | 0.13  | 0.10  | 0.05  |
| JP1-_gamma_omega8:omega1/5^P_1 omega8:omega1/5^P_1_order0 |  | 19.265 +/- 3.7383      |  |      |      |      |      |      |      |       |       |       | 1.00  | 0.46  | -0.09 |
| JP1-_gamma_omega8:omega8/3^P_1 omega8:omega8/3^P_1_order0 |  | 10.555 +/- 2.8996      |  |      |      |      |      |      |      |       |       |       |       | 1.00  | -0.11 |
| JP1-_m_pole0                                              |  | 0.46076 +/- 0.0010264  |  |      |      |      |      |      |      |       |       |       |       |       | 1.00  |
| =====                                                     |  |                        |  |      |      |      |      |      |      |       |       |       |       |       |       |

Phase space prescription ::

pole0\_sub

eta8:eta1[-] f8:eta8[+] h8:eta8[+] omega8:eta8[-] omega8:omega1[-] omega8:omega8[-] lower half-plane

sqrt(s)\_pole = (0.46069 +/- 0.0010211)  
+ (i/2)\*(-0.0022529 +/- 0.0012423) [-0.01]

s\_pole = (0.21223 +/- 0.00094082)  
+ i\*(-0.0010379 +/- 0.00057232) [-0.01]

| eta8:eta1                | f8:eta8                  | h8:eta8                  | omega8:eta8              | omega8:omega1            | omega8:omega8            |
|--------------------------|--------------------------|--------------------------|--------------------------|--------------------------|--------------------------|
| k_re= 0.1491 +/- 0.0008  | k_re= -0.0029 +/- 0.0016 | k_re= -0.0020 +/- 0.0011 | k_re= 0.1402 +/- 0.0008  | k_re= 0.0789 +/- 0.0015  | k_re= 0.0816 +/- 0.0014  |
| k_im= -0.0009 +/- 0.0005 | k_im= 0.0386 +/- 0.0026  | k_im= 0.0533 +/- 0.0018  | k_im= -0.0009 +/- 0.0005 | k_im= -0.0016 +/- 0.0009 | k_im= -0.0016 +/- 0.0009 |
| corr= [-0.00]            | corr= [ 0.09]            | corr= [ 0.05]            | corr= [-0.00]            | corr= [ 0.01]            | corr= [ 0.01]            |

  

| eta8:eta1/1^P_1              | f8:eta8/3^S_1                  | h8:eta8/3^S_1(*)             | omega8:eta8/3^P_1             | omega8:omega1/1^P_1          | omega8:omega1/3^P_1          | omega8:omega1/5^P_1          | omega8:omega8/3^P_1          |
|------------------------------|--------------------------------|------------------------------|-------------------------------|------------------------------|------------------------------|------------------------------|------------------------------|
| g = 0.0258 +/- 0.0122        | g = 0.0082 +/- 0.1485          | g = 0.3562 +/- 0.0457        | g = 0.0315 +/- 0.0106         | g = 0.0000 +/- 0.0000        | g = 0.0000 +/- 0.0000        | g = 0.0000 +/- 0.0000        | g = 0.0000 +/- 0.0000        |
| arg(g)/pi= 0.0283 +/- 0.0105 | arg(g)/pi= -0.4915 +/- 11.1697 | arg(g)/pi= 0.0037 +/- 0.0028 | arg(g)/pi= -0.0524 +/- 0.0096 | arg(g)/pi= 0.4963 +/- 0.0028 | arg(g)/pi= 0.4963 +/- 0.0028 | arg(g)/pi= 0.4963 +/- 0.0028 | arg(g)/pi= 0.4963 +/- 0.0028 |
| g_re= 0.0257 +/- 0.0122      | g_re= 0.0000 +/- 0.2352        | g_re= 0.3562 +/- 0.0456      | g_re= 0.0311 +/- 0.0104       | g_re= 0.0000 +/- 0.0000      | g_re= 0.0000 +/- 0.0000      | g_re= 0.0000 +/- 0.0000      | g_re= 0.0000 +/- 0.0000      |
| g_im= 0.0023 +/- 0.0013      | g_im= 0.0000 +/- 0.0078        | g_im= 0.0041 +/- 0.0035      | g_im= -0.0052 +/- 0.0024      | g_im= 0.0000 +/- 0.0000      | g_im= 0.0000 +/- 0.0000      | g_im= 0.0000 +/- 0.0000      | g_im= 0.0000 +/- 0.0000      |
| corr= [ 0.75]                | corr= [ 1.00]                  | corr= [ 0.71]                | corr= [-0.94]                 | corr= [-0.50]                | corr= [-0.50]                | corr= [-0.50]                | corr= [-0.50]                |

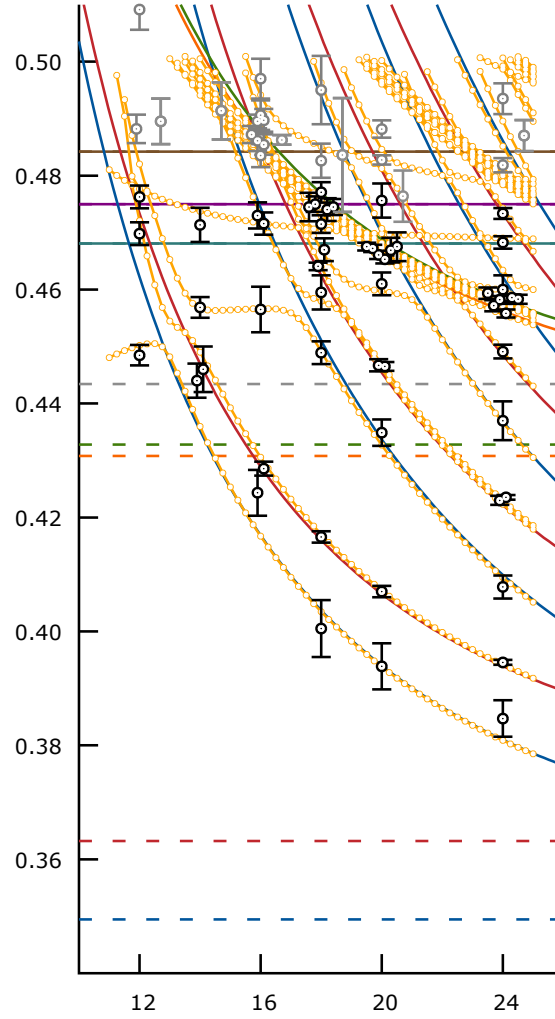

Figure 1.1: Similar to Figure 6 in the manuscript, the finite-volume spectrum, plotted as  $a_t E_{\text{cm}}$ , as a function of spatial extent  $L/a_s$ . Orange points/curves show the spectrum calculated from the amplitude given above (no uncertainties are shown). Black and grey points are the computed lattice energies on each volume, slightly displaced horizontally for clarity (black points correspond to energies used in the fit whereas grey points were not used). Two-meson non-interacting energies are shown as solid coloured curves/lines, two-meson thresholds are shown as dashed/solid horizontal lines, and the  $\eta^s \eta^s \eta^s$  threshold is shown as a dashed grey horizontal line.

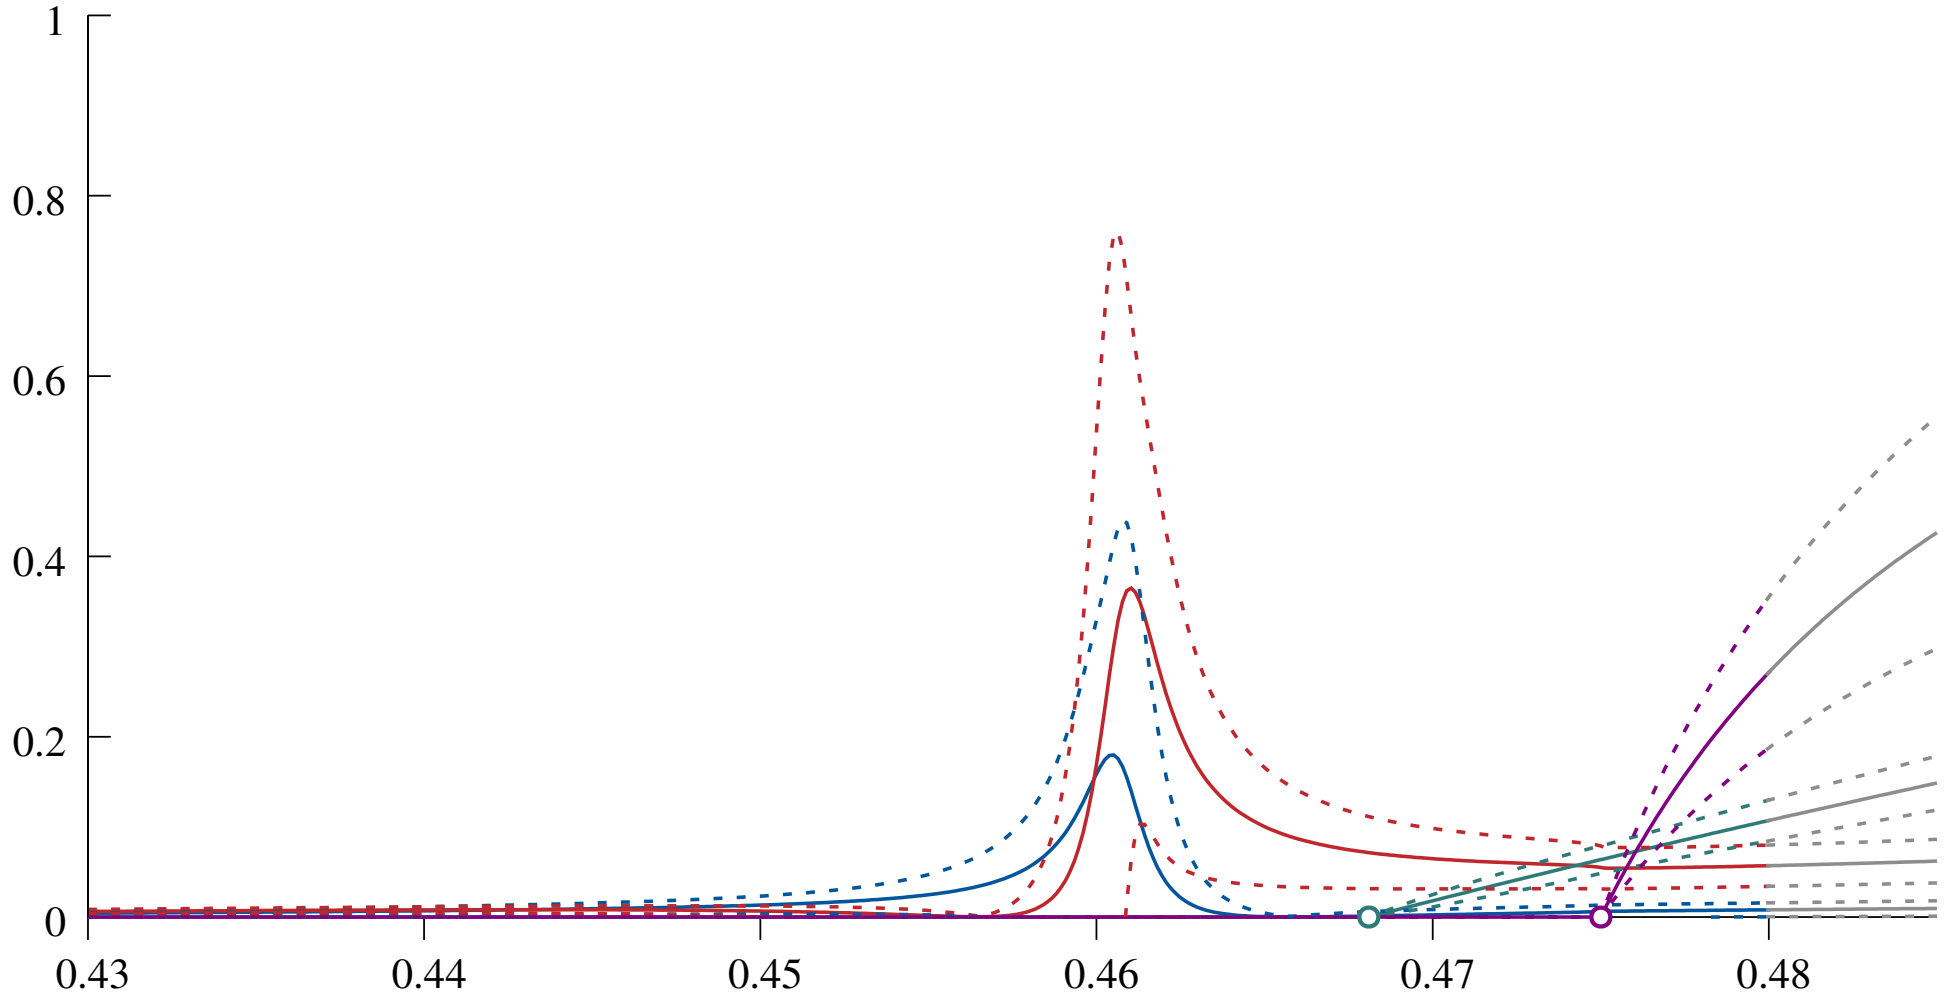

Figure 1.2: Similar to part (a) of Figure 7 in the manuscript,  $\rho_a \rho_b |t_{ab}|^2$  as a function of  $a_t E_{\text{cm}}$  for  $\eta^1 \eta^s \{^1P_1\} \rightarrow \eta^1 \eta^s \{^1P_1\}$  (blue),  $\omega^s \eta^s \{^3P_1\} \rightarrow \omega^s \eta^s \{^3P_1\}$  (red),  $f_1^s \eta^s \{^3S_1\} \rightarrow f_1^s \eta^s \{^3S_1\}$  (cyan), and  $h_1^s \eta^s \{^3S_1\} \rightarrow h_1^s \eta^s \{^3S_1\}$  (purple). Dashed lines indicate one standard deviation statistical uncertainties.

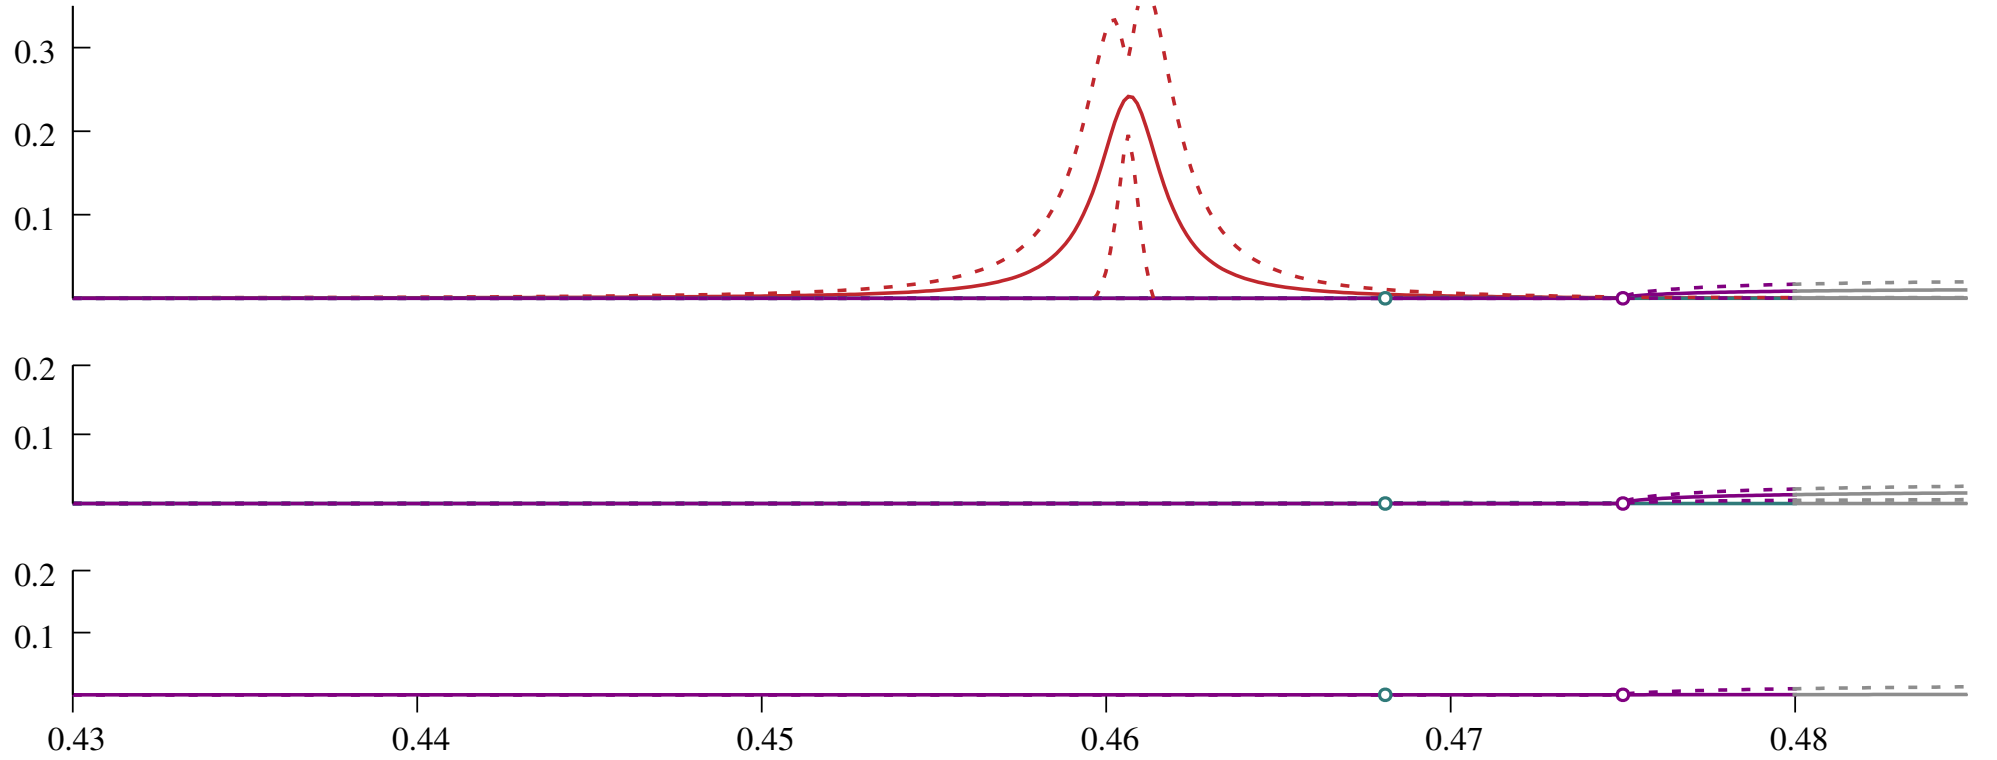

Figure 1.3: Similar to parts (b), (c) and (d) of Figure 7 in the manuscript,  $\rho_a \rho_b |t_{ab}|^2$  as a function of  $a_t E_{\text{cm}}$ . Top:  $\eta^1 \eta^s \{^1P_1\} \rightarrow \omega^s \eta^s \{^3P_1\}$  (red),  $\eta^1 \eta^s \{^1P_1\} \rightarrow f_1^s \eta^s \{^3S_1\}$  (cyan), and  $\eta^1 \eta^s \{^1P_1\} \rightarrow h_1^s \eta^s \{^3S_1\}$  (purple). Middle:  $\omega^s \eta^s \{^3P_1\} \rightarrow f_1^s \eta^s \{^3S_1\}$  (cyan), and  $\omega^s \eta^s \{^3P_1\} \rightarrow h_1^s \eta^s \{^3S_1\}$  (purple). Bottom:  $f_1^s \eta^s \{^3S_1\} \rightarrow h_1^s \eta^s \{^3S_1\}$  (purple). Dashed lines indicate one standard deviation statistical uncertainties.

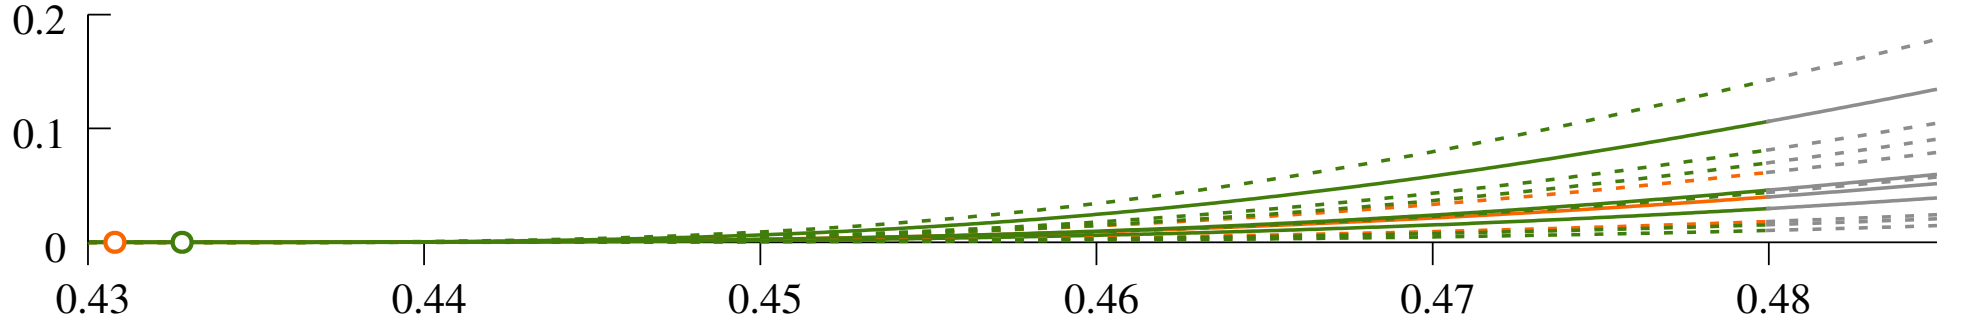

Figure 1.4: Similar to parts (e) and (f) of Figure 7 in the manuscript,  $\rho_a \rho_b |t_{ab}|^2$  as a function of  $a_t E_{cm}$  for  $\omega^s \omega^s \{^3P_1\} \rightarrow \omega^s \omega^s \{^3P_1\}$  (orange),  $\omega^1 \omega^s \{^1P_1, ^3P_1, ^5P_1\} \rightarrow \omega^s \omega^1 \{^1P_1, ^3P_1, ^5P_1\}$  (green). Dashed lines indicate one standard deviation statistical uncertainties.

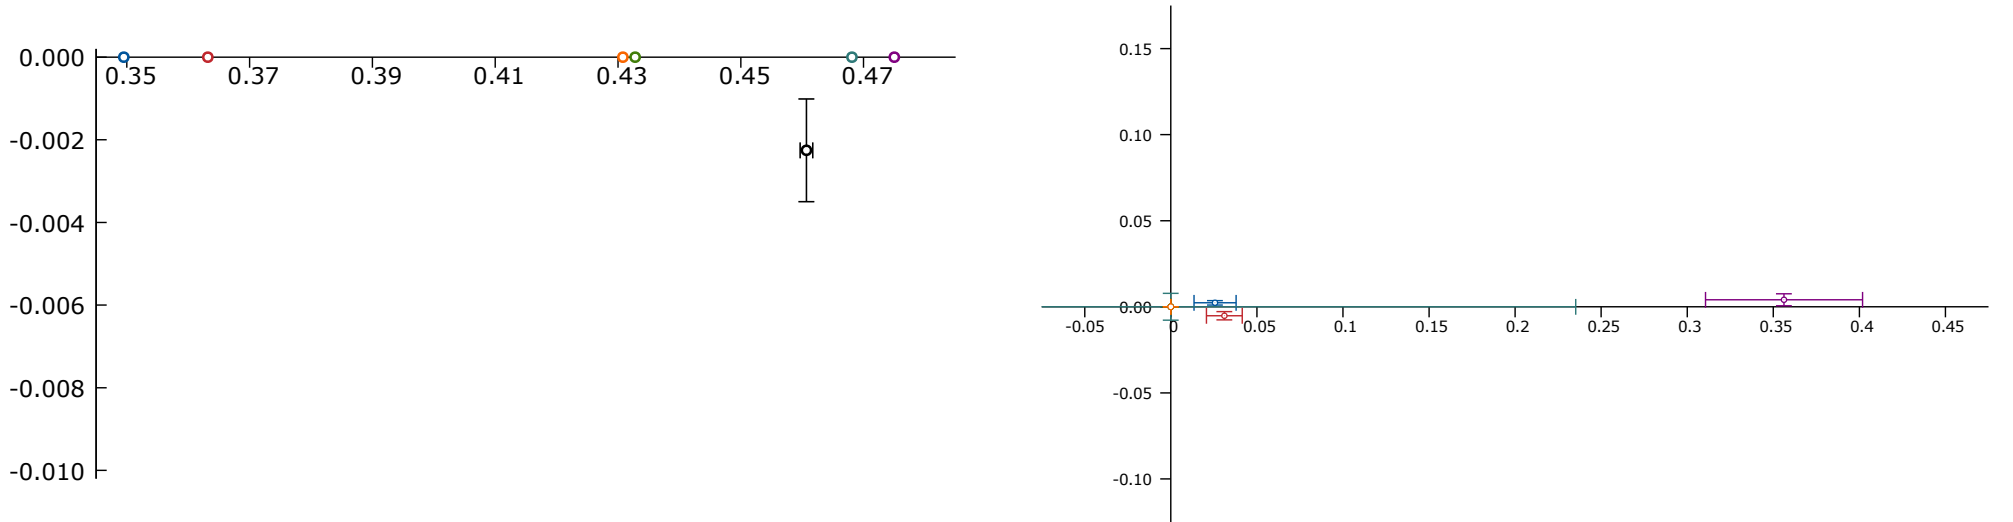

Figure 1.5: Left: Similar to Figure 13 in the manuscript, pole position on the proximal sheet (closest to physical scattering) with  $\text{Re}(a_t \sqrt{s})$  on the horizontal axis and  $2 \text{Im}(a_t \sqrt{s})$  on the vertical axis. Right: Similar to Figure 14 in the manuscript, the corresponding couplings with  $\text{Re}(a_t c)$  on the horizontal axis and  $\text{Im}(a_t c)$  on the vertical axis.

## 1.2 $\{m, g_{b,f}^{(0)}, \gamma_{(a,a),(b,b),(c,c),(\partial_1,\partial_1),(\partial_2,\partial_2),(\partial_3,\partial_3),(e,e)}^{(0)}\}(\text{CM}_m)$

minimised with  $\text{chisq}/\text{nDoF} = 46.85 / (53 - 10) = 1.09$

|                                                           |  |                        |  |      |      |      |      |       |       |      |       |       |       |
|-----------------------------------------------------------|--|------------------------|--|------|------|------|------|-------|-------|------|-------|-------|-------|
| =====                                                     |  |                        |  |      |      |      |      |       |       |      |       |       |       |
| JP1-_g_h8:eta8/3`S_1_pole0                                |  | 0.92831 +/- 0.78192    |  | 1.00 | 0.92 | 0.33 | 0.42 | -0.10 | -0.00 | 0.05 | -0.00 | -0.01 | 0.54  |
| JP1-_g_omega8:eta8/3`P_1_pole0                            |  | 0.29086 +/- 0.23094    |  |      | 1.00 | 0.33 | 0.39 | -0.29 | 0.02  | 0.04 | 0.01  | 0.00  | 0.43  |
| JP1-_gamma_eta8:eta1/1`P_1 eta8:eta1/1`P_1_order0         |  | 1.5929 +/- 0.5444      |  |      |      | 1.00 | 0.55 | -0.02 | 0.01  | 0.05 | 0.01  | 0.00  | 0.02  |
| JP1-_gamma_f8:eta8/3`S_1 f8:eta8/3`S_1_order0             |  | -2.0567 +/- 0.30927    |  |      |      |      | 1.00 | -0.00 | 0.03  | 0.07 | 0.03  | 0.03  | 0.14  |
| JP1-_gamma_omega8:eta8/3`P_1 omega8:eta8/3`P_1_order0     |  | -3.6136 +/- 0.61734    |  |      |      |      |      | 1.00  | 0.06  | 0.08 | 0.07  | 0.13  | 0.08  |
| JP1-_gamma_omega8:omega1/1`P_1 omega8:omega1/1`P_1_order0 |  | 9.7096 +/- 2.3644      |  |      |      |      |      |       | 1.00  | 0.05 | 0.39  | 0.43  | -0.04 |
| JP1-_gamma_omega8:omega1/3`P_1 omega8:omega1/3`P_1_order0 |  | 12.324 +/- 4.9414      |  |      |      |      |      |       |       | 1.00 | 0.13  | 0.10  | 0.07  |
| JP1-_gamma_omega8:omega1/5`P_1 omega8:omega1/5`P_1_order0 |  | 19.682 +/- 3.7412      |  |      |      |      |      |       |       |      | 1.00  | 0.45  | -0.06 |
| JP1-_gamma_omega8:omega8/3`P_1 omega8:omega8/3`P_1_order0 |  | 10.798 +/- 2.8983      |  |      |      |      |      |       |       |      |       | 1.00  | -0.08 |
| JP1-_m_pole0                                              |  | 0.46042 +/- 0.00083988 |  |      |      |      |      |       |       |      |       |       | 1.00  |
| =====                                                     |  |                        |  |      |      |      |      |       |       |      |       |       |       |

Phase space prescription ::

pole0\_sub

eta8:eta1[-] f8:eta8[+] h8:eta8[+] omega8:eta8[-] omega8:omega1[-] omega8:omega8[-] lower half-plane

sqrt(s)\_pole = (0.46031 +/- 0.00086008)  
+ (1/2)\*(-0.0012978 +/- 0.00077233) [ 0.25]

s\_pole = (0.21188 +/- 0.00079193)  
+ i\*(-0.00059737 +/- 0.00035524) [ 0.25]

| eta8:eta1                                                            | f8:eta8                                                              | h8:eta8                                                              | omega8:eta8                                                          | omega8:omega1                                                        | omega8:omega8                                                        |
|----------------------------------------------------------------------|----------------------------------------------------------------------|----------------------------------------------------------------------|----------------------------------------------------------------------|----------------------------------------------------------------------|----------------------------------------------------------------------|
| k_re= 0.1488 +/- 0.0007<br>k_im= -0.0005 +/- 0.0003<br>corr= [ 0.25] | k_re= -0.0016 +/- 0.0009<br>k_im= 0.0395 +/- 0.0022<br>corr= [-0.17] | k_re= -0.0012 +/- 0.0007<br>k_im= 0.0540 +/- 0.0015<br>corr= [-0.21] | k_re= 0.1399 +/- 0.0007<br>k_im= -0.0005 +/- 0.0003<br>corr= [ 0.25] | k_re= 0.0784 +/- 0.0013<br>k_im= -0.0010 +/- 0.0006<br>corr= [ 0.27] | k_re= 0.0811 +/- 0.0012<br>k_im= -0.0009 +/- 0.0006<br>corr= [ 0.26] |

  

| eta8:eta1/1^P_1                                                     | f8:eta8/3^S_1                                                       | h8:eta8/3^S_1(*)                                                    | omega8:eta8/3^P_1                                                    | omega8:omega1/1^P_1                                                 | omega8:omega1/3^P_1                                                 | omega8:omega1/5^P_1                                                 | omega8:omega8/3^P_1                                                 |
|---------------------------------------------------------------------|---------------------------------------------------------------------|---------------------------------------------------------------------|----------------------------------------------------------------------|---------------------------------------------------------------------|---------------------------------------------------------------------|---------------------------------------------------------------------|---------------------------------------------------------------------|
| g = 0.0000 +/- 0.0000<br>arg(g)/pi= 0.4980 +/- 0.0017               | g = 0.0000 +/- 0.0000<br>arg(g)/pi= 0.4980 +/- 0.0017               | g = 0.3630 +/- 0.0477<br>arg(g)/pi= 0.0020 +/- 0.0017               | g = 0.0313 +/- 0.0093<br>arg(g)/pi= -0.0534 +/- 0.0083               | g = 0.0000 +/- 0.0000<br>arg(g)/pi= 0.4980 +/- 0.0017               | g = 0.0000 +/- 0.0000<br>arg(g)/pi= 0.4980 +/- 0.0017               | g = 0.0000 +/- 0.0000<br>arg(g)/pi= 0.4980 +/- 0.0017               | g = 0.0000 +/- 0.0000<br>arg(g)/pi= 0.4980 +/- 0.0017               |
| g_re= 0.0000 +/- 0.0000<br>g_im= 0.0000 +/- 0.0000<br>corr= [-0.67] | g_re= 0.0000 +/- 0.0000<br>g_im= 0.0000 +/- 0.0000<br>corr= [-0.67] | g_re= 0.3630 +/- 0.0477<br>g_im= 0.0023 +/- 0.0021<br>corr= [ 0.81] | g_re= 0.0309 +/- 0.0091<br>g_im= -0.0052 +/- 0.0020<br>corr= [-0.93] | g_re= 0.0000 +/- 0.0000<br>g_im= 0.0000 +/- 0.0000<br>corr= [-0.67] | g_re= 0.0000 +/- 0.0000<br>g_im= 0.0000 +/- 0.0000<br>corr= [-0.67] | g_re= 0.0000 +/- 0.0000<br>g_im= 0.0000 +/- 0.0000<br>corr= [-0.67] | g_re= 0.0000 +/- 0.0000<br>g_im= 0.0000 +/- 0.0000<br>corr= [-0.67] |

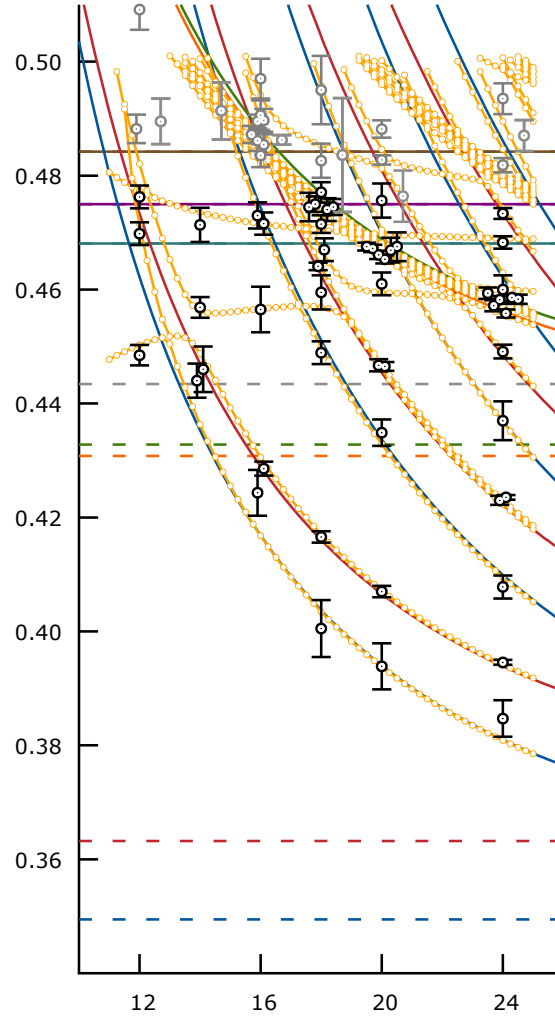

Figure 1.6: Similar to Figure 6 in the manuscript, the finite-volume spectrum, plotted as  $a_t E_{\text{cm}}$ , as a function of spatial extent  $L/a_s$ . Orange points/curves show the spectrum calculated from the amplitude given above (no uncertainties are shown). Black and grey points are the computed lattice energies on each volume, slightly displaced horizontally for clarity (black points correspond to energies used in the fit whereas grey points were not used). Two-meson non-interacting energies are shown as solid coloured curves/lines, two-meson thresholds are shown as dashed/solid horizontal lines, and the  $\eta^s \eta^s \eta^s$  threshold is shown as a dashed grey horizontal line.

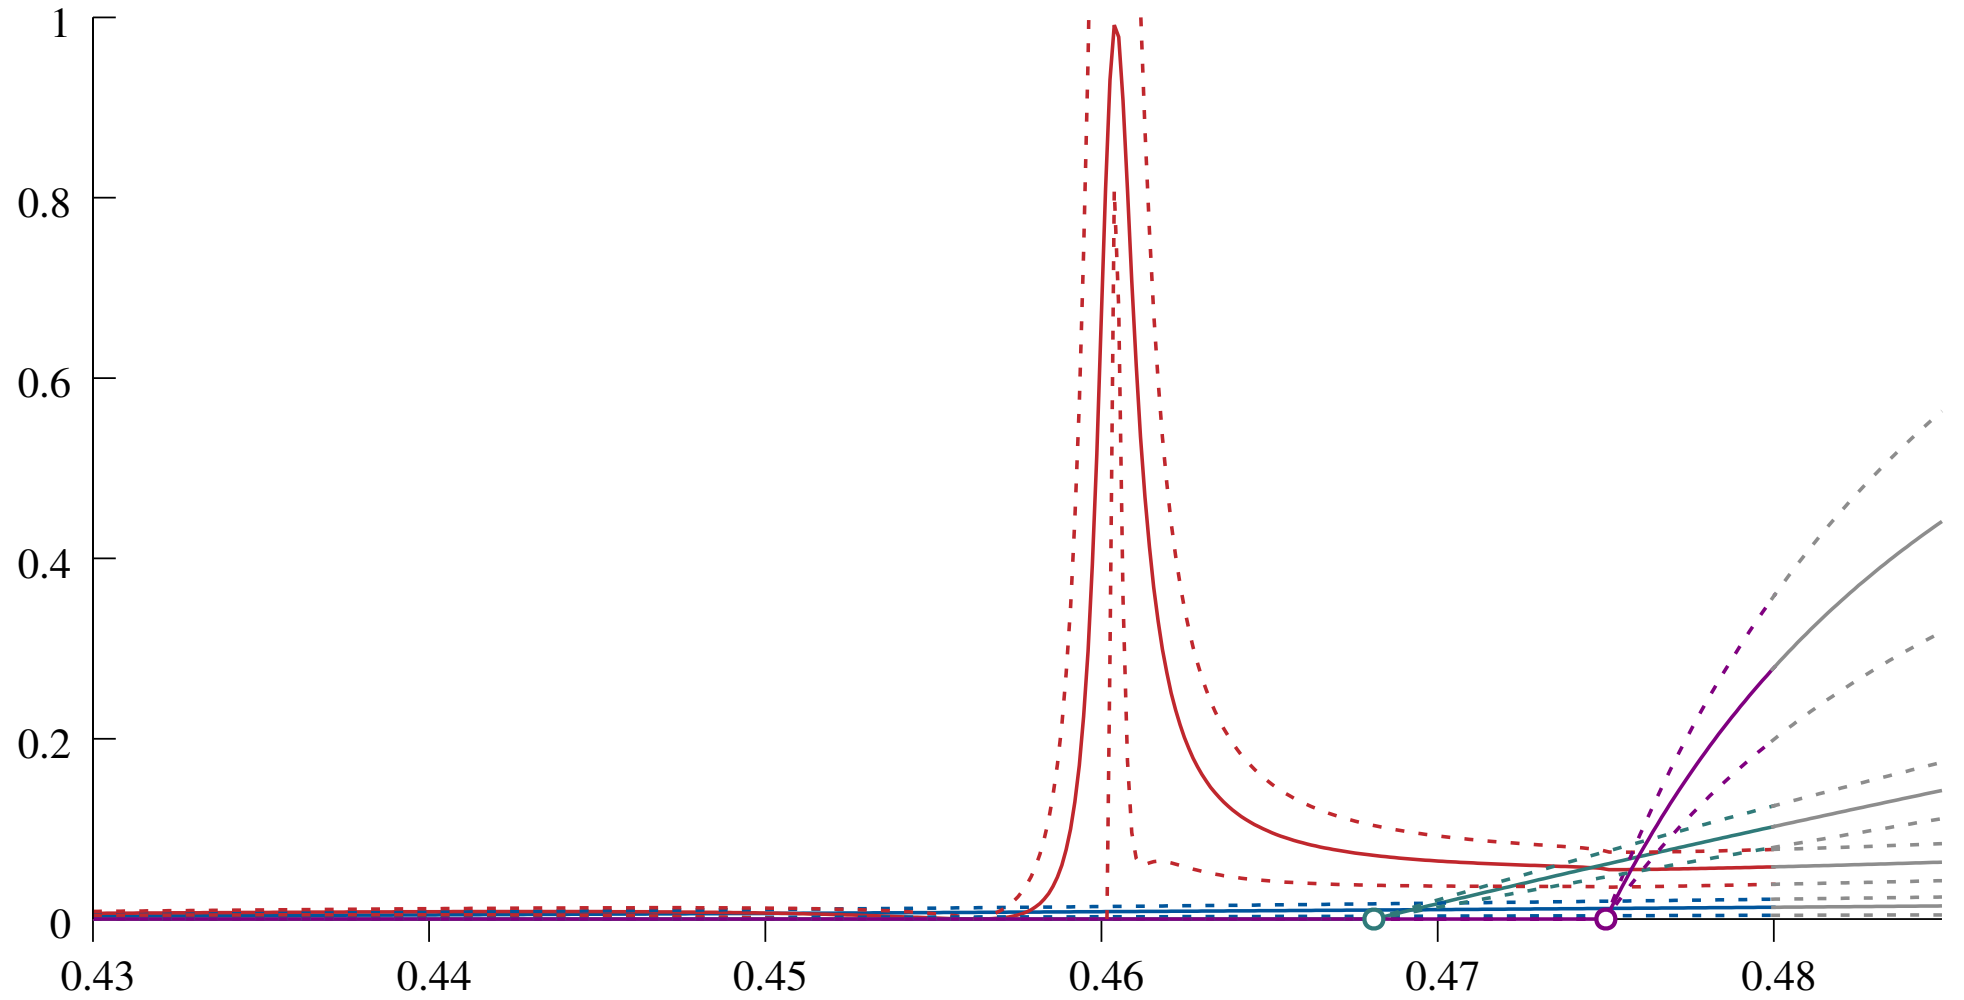

Figure 1.7: Similar to part (a) of Figure 7 in the manuscript,  $\rho_a \rho_b |t_{ab}|^2$  as a function of  $a_t E_{\text{cm}}$  for  $\eta^1 \eta^s \{^1P_1\} \rightarrow \eta^1 \eta^s \{^1P_1\}$  (blue),  $\omega^s \eta^s \{^3P_1\} \rightarrow \omega^s \eta^s \{^3P_1\}$  (red),  $f_1^s \eta^s \{^3S_1\} \rightarrow f_1^s \eta^s \{^3S_1\}$  (cyan), and  $h_1^s \eta^s \{^3S_1\} \rightarrow h_1^s \eta^s \{^3S_1\}$  (purple). Dashed lines indicate one standard deviation statistical uncertainties.

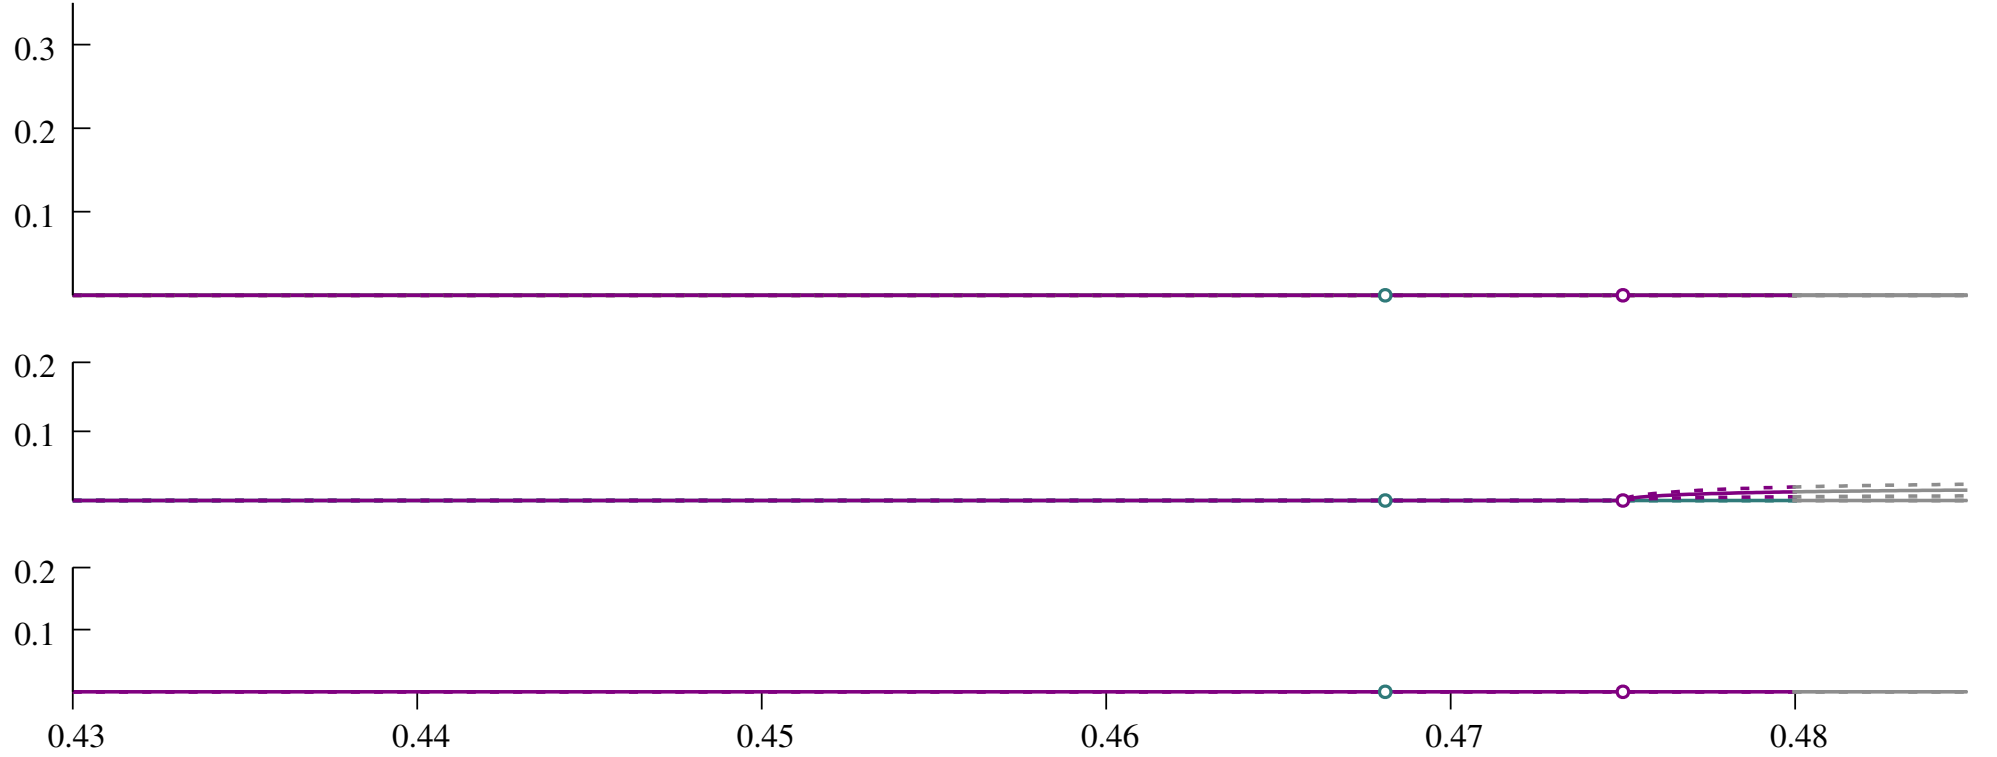

Figure 1.8: Similar to parts (b), (c) and (d) of Figure 7 in the manuscript,  $\rho_a \rho_b |t_{ab}|^2$  as a function of  $a_t E_{\text{cm}}$ . Top:  $\eta^1 \eta^s \{^1P_1\} \rightarrow \omega^s \eta^s \{^3P_1\}$  (red),  $\eta^1 \eta^s \{^1P_1\} \rightarrow f_1^s \eta^s \{^3S_1\}$  (cyan), and  $\eta^1 \eta^s \{^1P_1\} \rightarrow h_1^s \eta^s \{^3S_1\}$  (purple). Middle:  $\omega^s \eta^s \{^3P_1\} \rightarrow f_1^s \eta^s \{^3S_1\}$  (cyan), and  $\omega^s \eta^s \{^3P_1\} \rightarrow h_1^s \eta^s \{^3S_1\}$  (purple). Bottom:  $f_1^s \eta^s \{^3S_1\} \rightarrow h_1^s \eta^s \{^3S_1\}$  (purple). Dashed lines indicate one standard deviation statistical uncertainties.

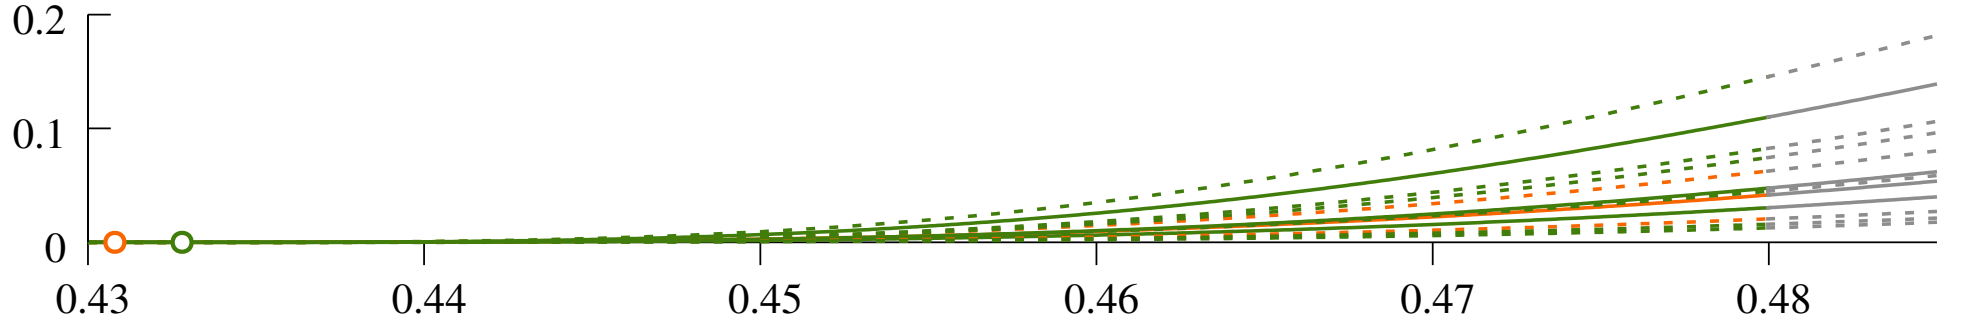

Figure 1.9: Similar to parts (e) and (f) of Figure 7 in the manuscript,  $\rho_a \rho_b |t_{ab}|^2$  as a function of  $a_t E_{\text{cm}}$  for  $\omega^s \omega^s \{^3P_1\} \rightarrow \omega^s \omega^s \{^3P_1\}$  (orange),  $\omega^1 \omega^s \{^1P_1, ^3P_1, ^5P_1\} \rightarrow \omega^s \omega^1 \{^1P_1, ^3P_1, ^5P_1\}$  (green). Dashed lines indicate one standard deviation statistical uncertainties.

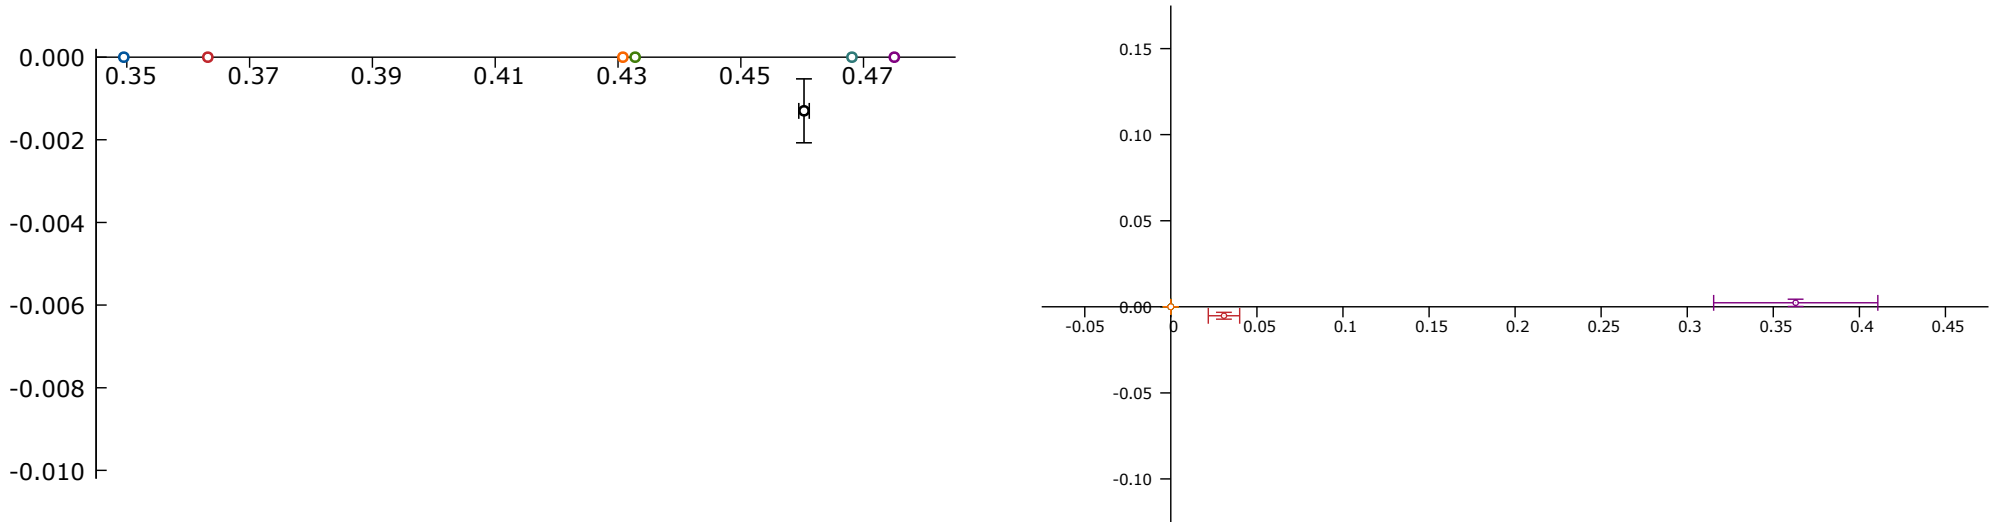

Figure 1.10: Left: Similar to Figure 13 in the manuscript, pole position on the proximal sheet (closest to physical scattering) with  $\text{Re}(a_t \sqrt{s})$  on the horizontal axis and  $2 \text{Im}(a_t \sqrt{s})$  on the vertical axis. Right: Similar to Figure 14 in the manuscript, the corresponding couplings with  $\text{Re}(a_t c)$  on the horizontal axis and  $\text{Im}(a_t c)$  on the vertical axis.

### 1.3 $\{m, g_{a,e,f}^{(0)}, \gamma_{(a,a),(b,b),(c,c),(\partial_1,\partial_1),(\partial_2,\partial_2),(\partial_3,\partial_3),(e,e)}^{(0)}\}(\mathbf{CM}_m)$

minimised with  $\text{chisq}/\text{nDoF} = 48.82 / (53 - 11) = 1.16$

|                                                          |  |                        |  |      |      |      |      |      |       |       |       |       |       |       |
|----------------------------------------------------------|--|------------------------|--|------|------|------|------|------|-------|-------|-------|-------|-------|-------|
| JP1-g_eta8:eta1/1^P_1_pole0                              |  | 0.20647 +/- 0.14179    |  | 1.00 | 0.00 | 0.78 | 0.12 | 0.29 | 0.06  | -0.04 | 0.01  | -0.07 | -0.06 | 0.68  |
| JP1-g_f8:eta8/3^S_1_pole0                                |  | 0.00042914 +/- 0.35056 |  |      | 1.00 | 0.00 | 0.00 | 0.00 | -0.00 | -0.00 | -0.00 | -0.00 | -0.00 | 0.00  |
| JP1-g_h8:eta8/3^S_1_pole0                                |  | 0.77746 +/- 0.51235    |  |      |      | 1.00 | 0.28 | 0.42 | 0.07  | -0.00 | 0.06  | -0.01 | -0.01 | 0.58  |
| JP1-gamma_eta8:eta1/1^P_1 eta8:eta1/1^P_1_order0         |  | 1.3357 +/- 0.56104     |  |      |      |      | 1.00 | 0.54 | 0.09  | 0.01  | 0.06  | 0.02  | 0.01  | 0.01  |
| JP1-gamma_f8:eta8/3^S_1 f8:eta8/3^S_1_order0             |  | -2.1310 +/- 0.30158    |  |      |      |      |      | 1.00 | 0.09  | 0.03  | 0.08  | 0.03  | 0.03  | 0.17  |
| JP1-gamma_omega8:eta8/3^P_1 omega8:eta8/3^P_1_order0     |  | -3.0671 +/- 0.51282    |  |      |      |      |      |      | 1.00  | 0.10  | 0.10  | 0.10  | 0.18  | 0.02  |
| JP1-gamma_omega8:omega1/1^P_1 omega8:omega1/1^P_1_order0 |  | 9.3550 +/- 2.3541      |  |      |      |      |      |      |       | 1.00  | 0.06  | 0.39  | 0.43  | -0.06 |
| JP1-gamma_omega8:omega1/3^P_1 omega8:omega1/3^P_1_order0 |  | 12.102 +/- 4.9342      |  |      |      |      |      |      |       |       | 1.00  | 0.14  | 0.10  | 0.04  |
| JP1-gamma_omega8:omega1/5^P_1 omega8:omega1/5^P_1_order0 |  | 18.987 +/- 3.7214      |  |      |      |      |      |      |       |       |       | 1.00  | 0.46  | -0.09 |
| JP1-gamma_omega8:omega8/3^P_1 omega8:omega8/3^P_1_order0 |  | 10.320 +/- 2.8877      |  |      |      |      |      |      |       |       |       |       | 1.00  | -0.10 |
| JP1-m_pole0                                              |  | 0.46110 +/- 0.00097779 |  |      |      |      |      |      |       |       |       |       |       | 1.00  |

Phase space prescription ::

pole0\_sub

eta8:eta1[-] f8:eta8[+] h8:eta8[+] omega8:eta8[-] omega8:omega1[-] omega8:omega8[-] lower half-plane

$\text{sqrt}(s)_{\text{pole}} = (0.46114 \pm 0.0009311)$   
 $+ (i/2) * (-0.0010622 \pm 0.00094036) [-0.38]$

$s_{\text{pole}} = (0.21265 \pm 0.00085855)$   
 $+ i * (-0.00048981 \pm 0.00043402) [-0.38]$

| eta8:eta1                | f8:eta8                  | h8:eta8                  | omega8:eta8              | omega8:omega1            | omega8:omega8            |
|--------------------------|--------------------------|--------------------------|--------------------------|--------------------------|--------------------------|
| k_re= 0.1494 +/- 0.0007  | k_re= -0.0014 +/- 0.0013 | k_re= -0.0010 +/- 0.0009 | k_re= 0.1405 +/- 0.0008  | k_re= 0.0796 +/- 0.0014  | k_re= 0.0823 +/- 0.0013  |
| k_im= -0.0004 +/- 0.0004 | k_im= 0.0373 +/- 0.0024  | k_im= 0.0525 +/- 0.0017  | k_im= -0.0004 +/- 0.0004 | k_im= -0.0008 +/- 0.0007 | k_im= -0.0007 +/- 0.0007 |
| corr= [-0.38]            | corr= [ 0.43]            | corr= [ 0.41]            | corr= [-0.38]            | corr= [-0.37]            | corr= [-0.37]            |

  

| eta8:eta1/1^P_1              | f8:eta8/3^S_1                  | h8:eta8/3^S_1(*)             | omega8:eta8/3^P_1            | omega8:omega1/1^P_1          | omega8:omega1/3^P_1          | omega8:omega1/5^P_1          | omega8:omega8/3^P_1          |
|------------------------------|--------------------------------|------------------------------|------------------------------|------------------------------|------------------------------|------------------------------|------------------------------|
| g = 0.0275 +/- 0.0122        | g = 0.0057 +/- 0.0962          | g = 0.3474 +/- 0.0427        | g = 0.0000 +/- 0.0000        | g = 0.0000 +/- 0.0000        | g = 0.0000 +/- 0.0000        | g = 0.0000 +/- 0.0000        | g = 0.0000 +/- 0.0000        |
| arg(g)/pi= 0.0256 +/- 0.0105 | arg(g)/pi= -0.4627 +/- 11.1463 | arg(g)/pi= 0.0019 +/- 0.0019 | arg(g)/pi= 0.4981 +/- 0.0019 | arg(g)/pi= 0.4981 +/- 0.0019 | arg(g)/pi= 0.4981 +/- 0.0019 | arg(g)/pi= 0.4981 +/- 0.0019 | arg(g)/pi= 0.4981 +/- 0.0019 |
| g_re= 0.0274 +/- 0.0122      | g_re= 0.0002 +/- 0.1592        | g_re= 0.3474 +/- 0.0427      | g_re= 0.0000 +/- 0.0000      | g_re= 0.0000 +/- 0.0000      | g_re= 0.0000 +/- 0.0000      | g_re= 0.0000 +/- 0.0000      | g_re= 0.0000 +/- 0.0000      |
| g_im= 0.0022 +/- 0.0013      | g_im= 0.0000 +/- 0.0026        | g_im= 0.0021 +/- 0.0022      | g_im= 0.0000 +/- 0.0000      | g_im= 0.0000 +/- 0.0000      | g_im= 0.0000 +/- 0.0000      | g_im= 0.0000 +/- 0.0000      | g_im= 0.0000 +/- 0.0000      |
| corr= [ 0.71]                | corr= [ 1.00]                  | corr= [ 0.45]                | corr= [-0.25]                | corr= [-0.25]                | corr= [-0.25]                | corr= [-0.25]                | corr= [-0.25]                |

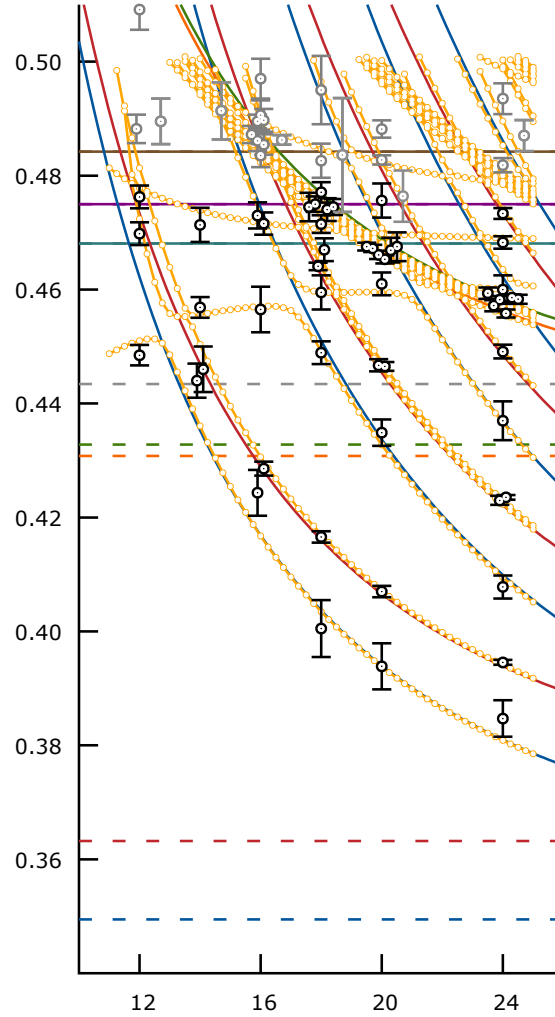

Figure 1.11: Similar to Figure 6 in the manuscript, the finite-volume spectrum, plotted as  $a_t E_{\text{cm}}$ , as a function of spatial extent  $L/a_s$ . Orange points/curves show the spectrum calculated from the amplitude given above (no uncertainties are shown). Black and grey points are the computed lattice energies on each volume, slightly displaced horizontally for clarity (black points correspond to energies used in the fit whereas grey points were not used). Two-meson non-interacting energies are shown as solid coloured curves/lines, two-meson thresholds are shown as dashed/solid horizontal lines, and the  $\eta^s \eta^s \eta^s$  threshold is shown as a dashed grey horizontal line.

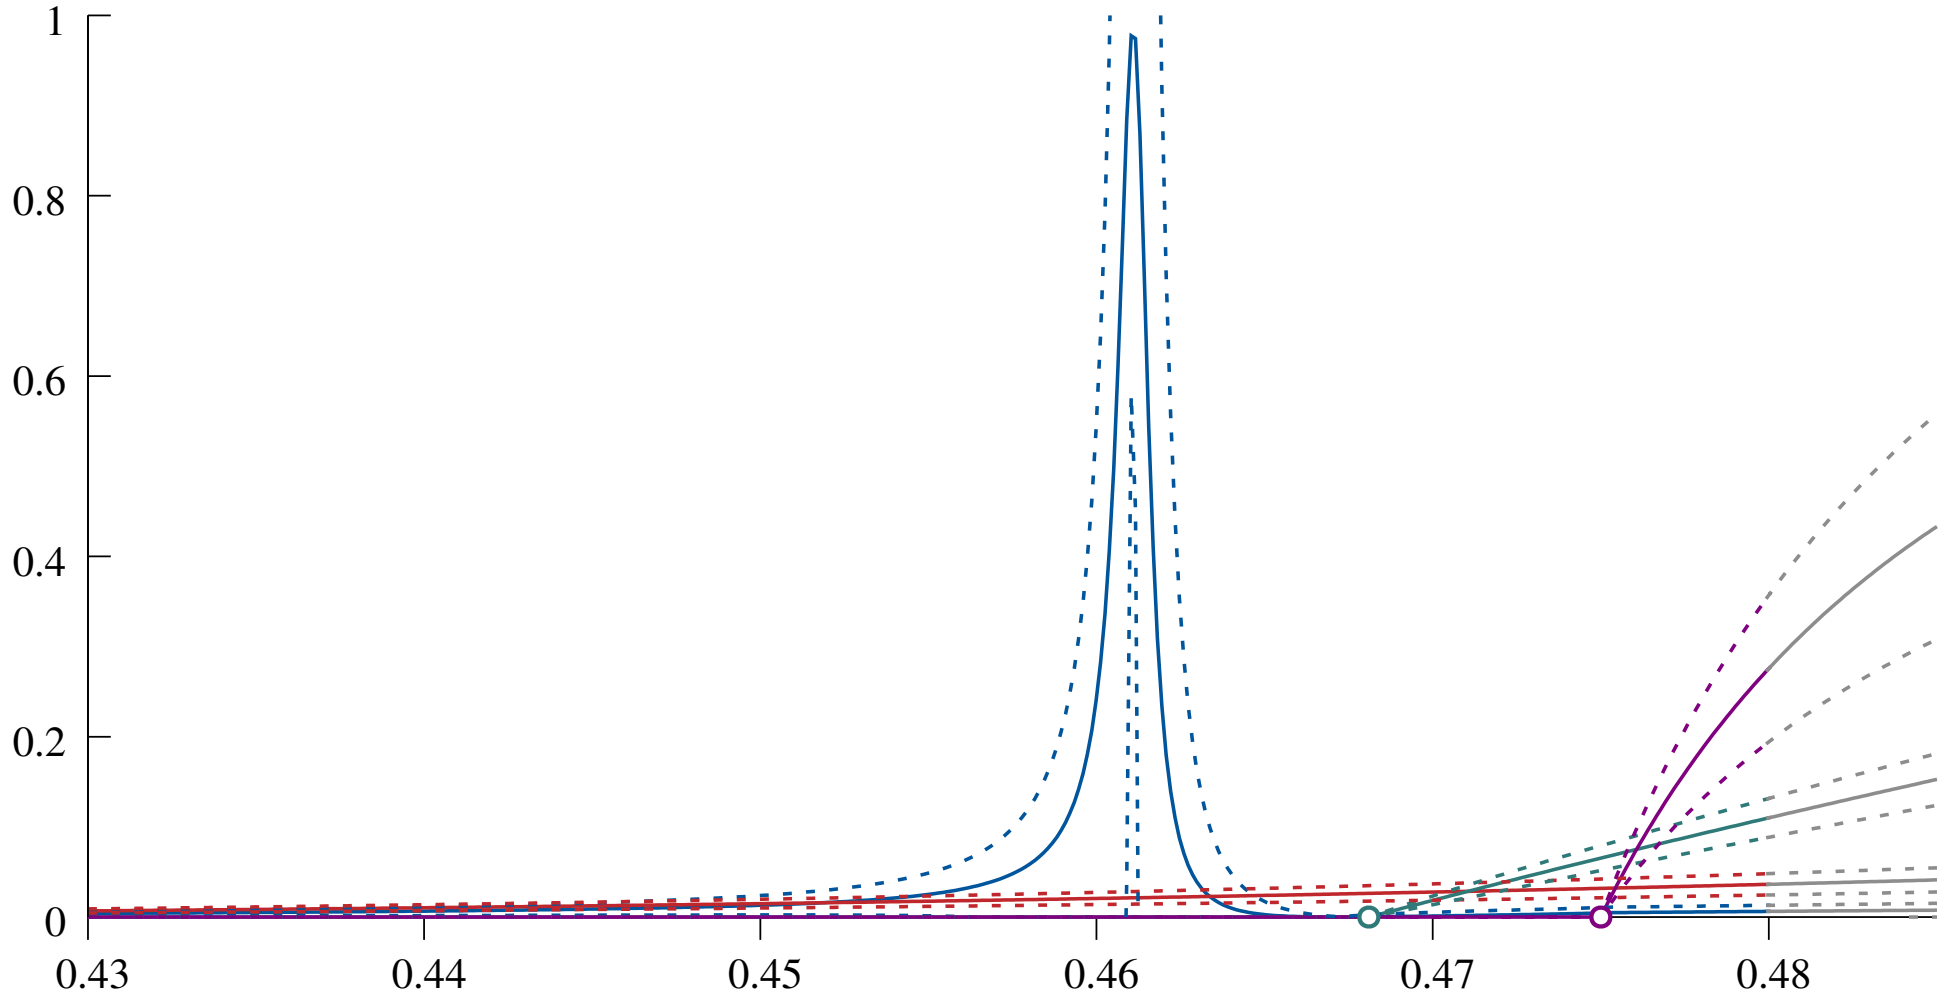

Figure 1.12: Similar to part (a) of Figure 7 in the manuscript,  $\rho_a \rho_b |t_{ab}|^2$  as a function of  $a_t E_{\text{cm}}$  for  $\eta^1 \eta^s \{^1P_1\} \rightarrow \eta^1 \eta^s \{^1P_1\}$  (blue),  $\omega^s \eta^s \{^3P_1\} \rightarrow \omega^s \eta^s \{^3P_1\}$  (red),  $f_1^s \eta^s \{^3S_1\} \rightarrow f_1^s \eta^s \{^3S_1\}$  (cyan), and  $h_1^s \eta^s \{^3S_1\} \rightarrow h_1^s \eta^s \{^3S_1\}$  (purple). Dashed lines indicate one standard deviation statistical uncertainties.

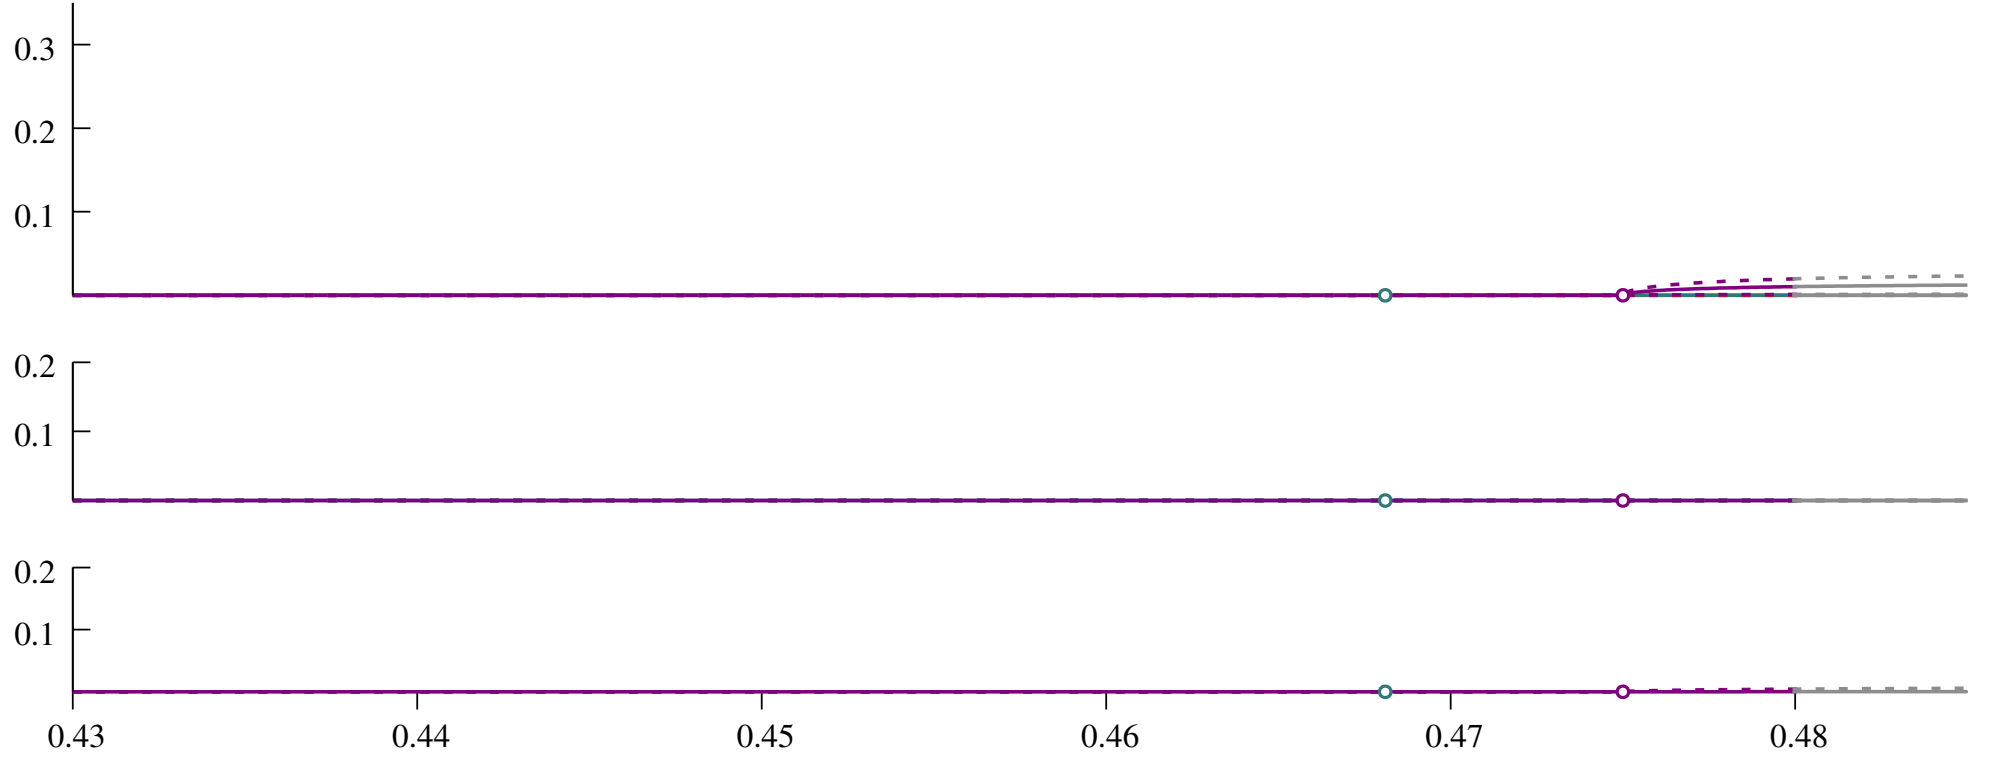

Figure 1.13: Similar to parts (b), (c) and (d) of Figure 7 in the manuscript,  $\rho_a \rho_b |t_{ab}|^2$  as a function of  $a_t E_{\text{cm}}$ . Top:  $\eta^1 \eta^s \{^1P_1\} \rightarrow \omega^s \eta^s \{^3P_1\}$  (red),  $\eta^1 \eta^s \{^1P_1\} \rightarrow f_1^s \eta^s \{^3S_1\}$  (cyan), and  $\eta^1 \eta^s \{^1P_1\} \rightarrow h_1^s \eta^s \{^3S_1\}$  (purple). Middle:  $\omega^s \eta^s \{^3P_1\} \rightarrow f_1^s \eta^s \{^3S_1\}$  (cyan), and  $\omega^s \eta^s \{^3P_1\} \rightarrow h_1^s \eta^s \{^3S_1\}$  (purple). Bottom:  $f_1^s \eta^s \{^3S_1\} \rightarrow h_1^s \eta^s \{^3S_1\}$  (purple). Dashed lines indicate one standard deviation statistical uncertainties.

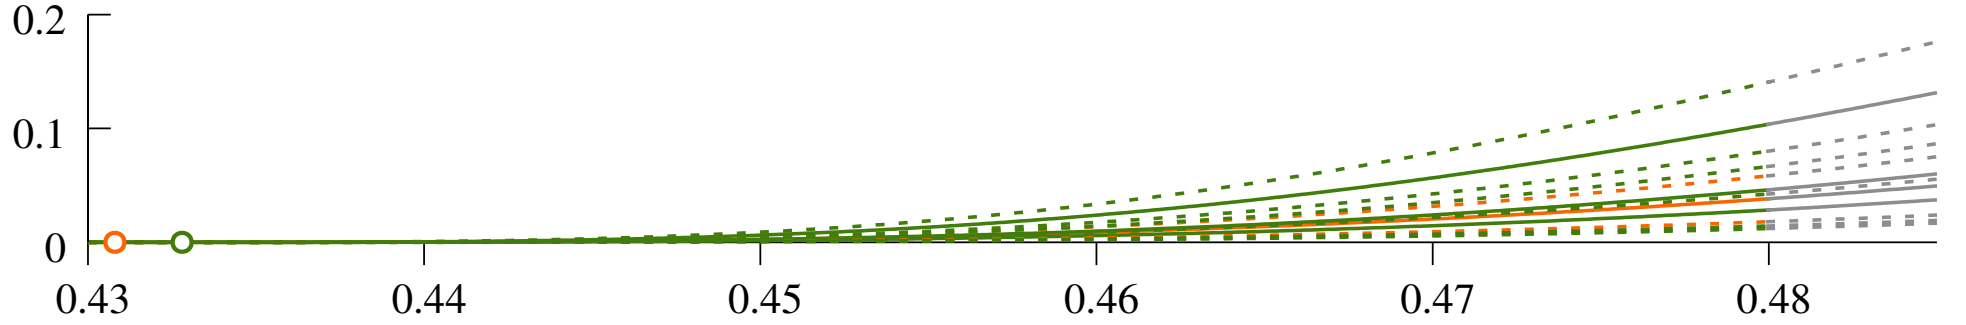

Figure 1.14: Similar to parts (e) and (f) of Figure 7 in the manuscript,  $\rho_a \rho_b |t_{ab}|^2$  as a function of  $a_t E_{cm}$  for  $\omega^s \omega^s \{^3P_1\} \rightarrow \omega^s \omega^s \{^3P_1\}$  (orange),  $\omega^1 \omega^s \{^1P_1, ^3P_1, ^5P_1\} \rightarrow \omega^s \omega^1 \{^1P_1, ^3P_1, ^5P_1\}$  (green). Dashed lines indicate one standard deviation statistical uncertainties.

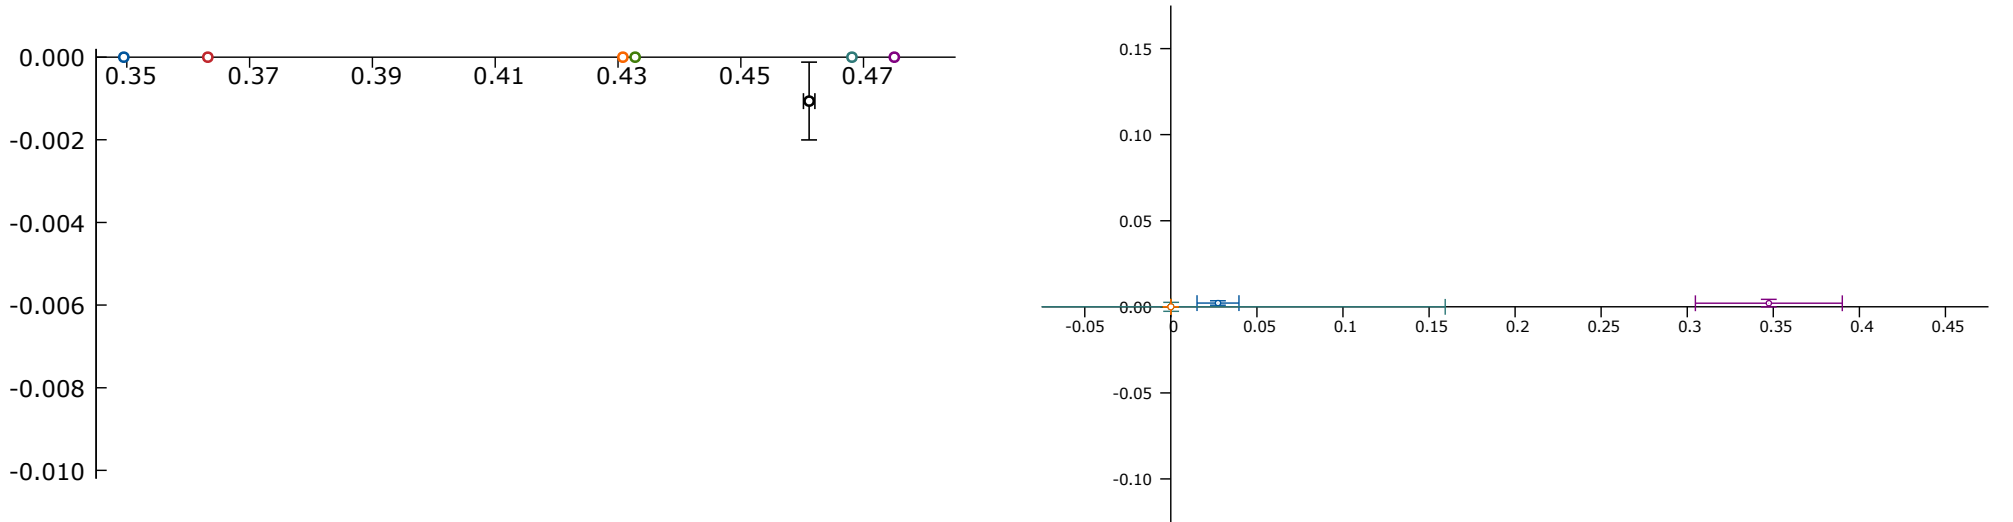

Figure 1.15: Left: Similar to Figure 13 in the manuscript, pole position on the proximal sheet (closest to physical scattering) with  $\text{Re}(a_t \sqrt{s})$  on the horizontal axis and  $2 \text{Im}(a_t \sqrt{s})$  on the vertical axis. Right: Similar to Figure 14 in the manuscript, the corresponding couplings with  $\text{Re}(a_t c)$  on the horizontal axis and  $\text{Im}(a_t c)$  on the vertical axis.

# 1.4 $\{m, g_{a,b,c,f}^{(0)}, \gamma_{(a,a),(b,b),(c,c),(\mathfrak{d}_1,\mathfrak{d}_1),(\mathfrak{d}_2,\mathfrak{d}_2),(\mathfrak{d}_3,\mathfrak{d}_3),(\mathfrak{e},\mathfrak{e})}^{(0)}\}(\mathbf{CM}_m)$

minimised with chisq/nDoF = 45.15 / (53 - 12) = 1.10

|                                                           |  |                       |  |      |      |      |      |      |      |       |       |      |       |       |       |
|-----------------------------------------------------------|--|-----------------------|--|------|------|------|------|------|------|-------|-------|------|-------|-------|-------|
| =====                                                     |  |                       |  |      |      |      |      |      |      |       |       |      |       |       |       |
| JP1-_g_eta8:eta1/1^P_1_pole0                              |  | 0.21010 +/- 0.15216   |  | 1.00 | 0.78 | 0.70 | 0.51 | 0.13 | 0.29 | -0.01 | -0.04 | 0.02 | -0.07 | -0.05 | 0.63  |
| JP1-_g_h8:eta8/3^S_1_pole0                                |  | 0.82078 +/- 0.61632   |  |      | 1.00 | 0.89 | 0.54 | 0.30 | 0.43 | -0.08 | 0.02  | 0.06 | 0.01  | -0.02 | 0.52  |
| JP1-_g_omega8:eta8/3^P_1_pole0                            |  | 0.26840 +/- 0.18634   |  |      |      | 1.00 | 0.52 | 0.30 | 0.39 | -0.31 | 0.03  | 0.05 | 0.02  | 0.01  | 0.38  |
| JP1-_g_omega8:omega8/3^P_1_pole0                          |  | 0.24546 +/- 0.25871   |  |      |      |      | 1.00 | 0.18 | 0.25 | 0.02  | -0.19 | 0.03 | -0.16 | 0.09  | 0.21  |
| JP1-_gamma_eta8:eta1/1^P_1 eta8:eta1/1^P_1_order0         |  | 1.4398 +/- 0.57293    |  |      |      |      |      | 1.00 | 0.55 | -0.02 | 0.02  | 0.06 | 0.03  | 0.01  | -0.02 |
| JP1-_gamma_f8:eta8/3^S_1 f8:eta8/3^S_1_order0             |  | -2.1047 +/- 0.30944   |  |      |      |      |      |      | 1.00 | 0.00  | 0.03  | 0.08 | 0.03  | 0.03  | 0.14  |
| JP1-_gamma_omega8:eta8/3^P_1 omega8:eta8/3^P_1_order0     |  | -3.5446 +/- 0.62675   |  |      |      |      |      |      |      | 1.00  | 0.03  | 0.08 | 0.04  | 0.13  | 0.10  |
| JP1-_gamma_omega8:omega1/1^P_1 omega8:omega1/1^P_1_order0 |  | 9.2396 +/- 2.4264     |  |      |      |      |      |      |      |       | 1.00  | 0.06 | 0.42  | 0.39  | -0.02 |
| JP1-_gamma_omega8:omega1/3^P_1 omega8:omega1/3^P_1_order0 |  | 12.020 +/- 4.9329     |  |      |      |      |      |      |      |       |       | 1.00 | 0.13  | 0.10  | 0.05  |
| JP1-_gamma_omega8:omega1/5^P_1 omega8:omega1/5^P_1_order0 |  | 18.831 +/- 3.7943     |  |      |      |      |      |      |      |       |       |      | 1.00  | 0.42  | -0.05 |
| JP1-_gamma_omega8:omega8/3^P_1 omega8:omega8/3^P_1_order0 |  | 10.751 +/- 2.981      |  |      |      |      |      |      |      |       |       |      |       | 1.00  | -0.07 |
| JP1-_m_pole0                                              |  | 0.46065 +/- 0.0010777 |  |      |      |      |      |      |      |       |       |      |       |       | 1.00  |
| =====                                                     |  |                       |  |      |      |      |      |      |      |       |       |      |       |       |       |

Phase space prescription ::

pole0\_sub

eta8:eta1[-] f8:eta8[+] h8:eta8[+] omega8:eta8[-] omega8:omega1[-] omega8:omega8[-] lower half-plane

sqrt(s)\_pole = (0.46059 +/- 0.0010589)  
+ (i/2)\*(-0.0026067 +/- 0.0013372) [ 0.02]

s\_pole = (0.21214 +/- 0.00097545)  
+ i\*(-0.0012006 +/- 0.00061586) [ 0.02]

| eta8:eta1                | f8:eta8                  | h8:eta8                  | omega8:eta8              | omega8:omega1            | omega8:omega8            |
|--------------------------|--------------------------|--------------------------|--------------------------|--------------------------|--------------------------|
| k_re= 0.1490 +/- 0.0008  | k_re= -0.0033 +/- 0.0017 | k_re= -0.0024 +/- 0.0012 | k_re= 0.1401 +/- 0.0009  | k_re= 0.0788 +/- 0.0015  | k_re= 0.0815 +/- 0.0015  |
| k_im= -0.0010 +/- 0.0005 | k_im= 0.0389 +/- 0.0027  | k_im= 0.0535 +/- 0.0019  | k_im= -0.0011 +/- 0.0005 | k_im= -0.0019 +/- 0.0010 | k_im= -0.0018 +/- 0.0009 |
| corr= [ 0.03]            | corr= [ 0.06]            | corr= [ 0.03]            | corr= [ 0.03]            | corr= [ 0.04]            | corr= [ 0.04]            |

  

| eta8:eta1/1^P_1              | f8:eta8/3^S_1                | h8:eta8/3^S_1(*)             | omega8:eta8/3^P_1             | omega8:omega1/1^P_1          | omega8:omega1/3^P_1          | omega8:omega1/5^P_1          | omega8:omega8/3^P_1          |
|------------------------------|------------------------------|------------------------------|-------------------------------|------------------------------|------------------------------|------------------------------|------------------------------|
| g = 0.0270 +/- 0.0120        | g = 0.0000 +/- 0.0000        | g = 0.3550 +/- 0.0459        | g = 0.0320 +/- 0.0097         | g = 0.0000 +/- 0.0000        | g = 0.0000 +/- 0.0000        | g = 0.0000 +/- 0.0000        | g = 0.0173 +/- 0.0161        |
| arg(g)/pi= 0.0278 +/- 0.0106 | arg(g)/pi= 0.4965 +/- 0.0030 | arg(g)/pi= 0.0035 +/- 0.0030 | arg(g)/pi= -0.0523 +/- 0.0095 | arg(g)/pi= 0.4965 +/- 0.0030 | arg(g)/pi= 0.4965 +/- 0.0030 | arg(g)/pi= 0.4965 +/- 0.0030 | arg(g)/pi= 0.0289 +/- 0.0099 |
| g_re= 0.0269 +/- 0.0119      | g_re= 0.0000 +/- 0.0000      | g_re= 0.3550 +/- 0.0459      | g_re= 0.0315 +/- 0.0095       | g_re= 0.0000 +/- 0.0000      | g_re= 0.0000 +/- 0.0000      | g_re= 0.0000 +/- 0.0000      | g_re= 0.0173 +/- 0.0160      |
| g_im= 0.0024 +/- 0.0013      | g_im= 0.0000 +/- 0.0000      | g_im= 0.0039 +/- 0.0037      | g_im= -0.0052 +/- 0.0022      | g_im= 0.0000 +/- 0.0000      | g_im= 0.0000 +/- 0.0000      | g_im= 0.0000 +/- 0.0000      | g_im= 0.0016 +/- 0.0015      |
| corr= [ 0.72]                | corr= [-0.58]                | corr= [ 0.75]                | corr= [-0.93]                 | corr= [-0.58]                | corr= [-0.58]                | corr= [-0.58]                | corr= [ 0.93]                |

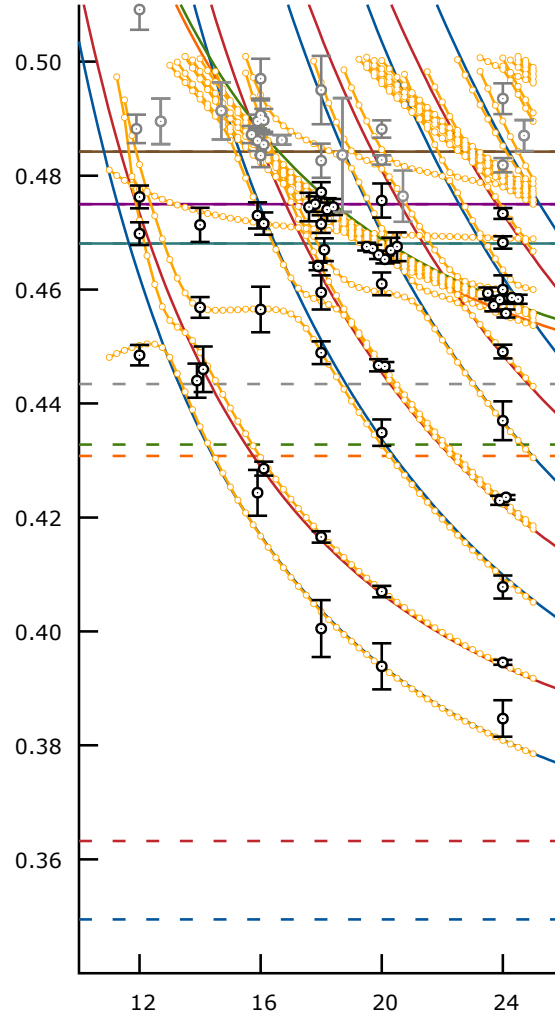

Figure 1.16: Similar to Figure 6 in the manuscript, the finite-volume spectrum, plotted as  $a_t E_{\text{cm}}$ , as a function of spatial extent  $L/a_s$ . Orange points/curves show the spectrum calculated from the amplitude given above (no uncertainties are shown). Black and grey points are the computed lattice energies on each volume, slightly displaced horizontally for clarity (black points correspond to energies used in the fit whereas grey points were not used). Two-meson non-interacting energies are shown as solid coloured curves/lines, two-meson thresholds are shown as dashed/solid horizontal lines, and the  $\eta^s \eta^s \eta^s$  threshold is shown as a dashed grey horizontal line.

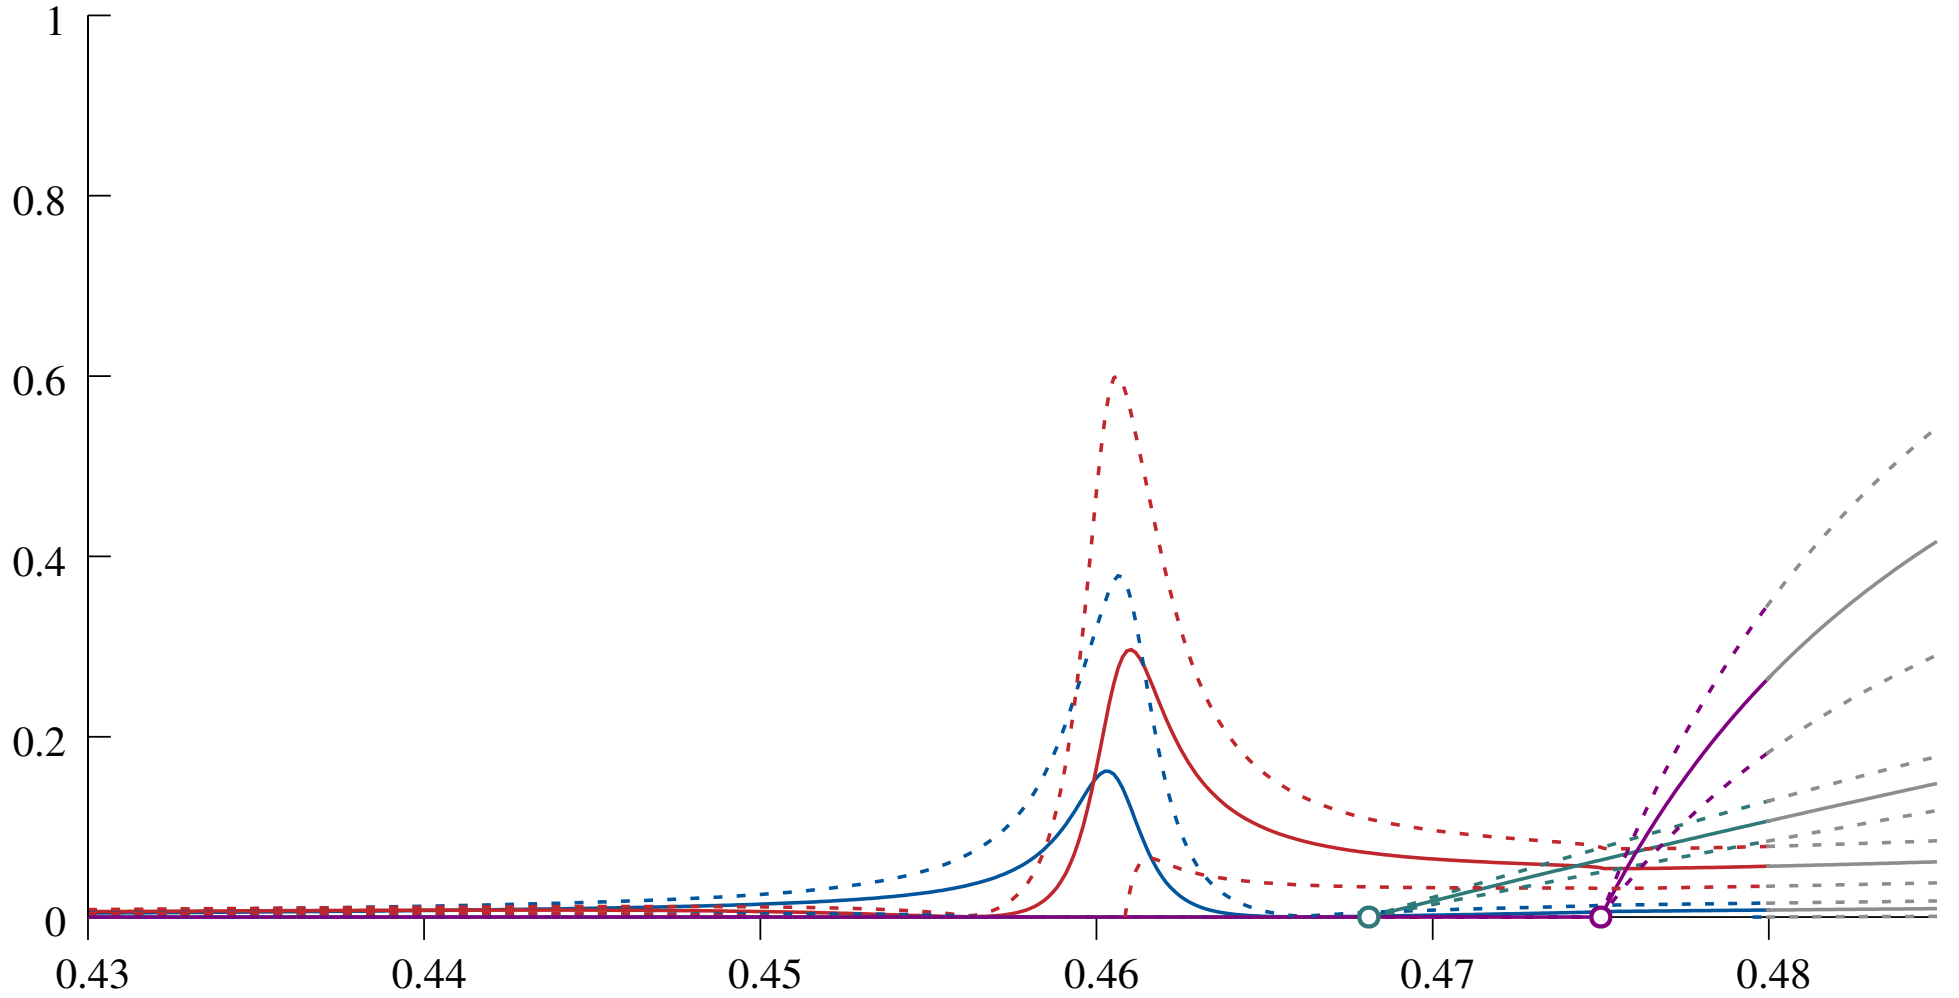

Figure 1.17: Similar to part (a) of Figure 7 in the manuscript,  $\rho_a \rho_b |t_{ab}|^2$  as a function of  $a_t E_{cm}$  for  $\eta^1 \eta^s \{^1P_1\} \rightarrow \eta^1 \eta^s \{^1P_1\}$  (blue),  $\omega^s \eta^s \{^3P_1\} \rightarrow \omega^s \eta^s \{^3P_1\}$  (red),  $f_1^s \eta^s \{^3S_1\} \rightarrow f_1^s \eta^s \{^3S_1\}$  (cyan), and  $h_1^s \eta^s \{^3S_1\} \rightarrow h_1^s \eta^s \{^3S_1\}$  (purple). Dashed lines indicate one standard deviation statistical uncertainties.

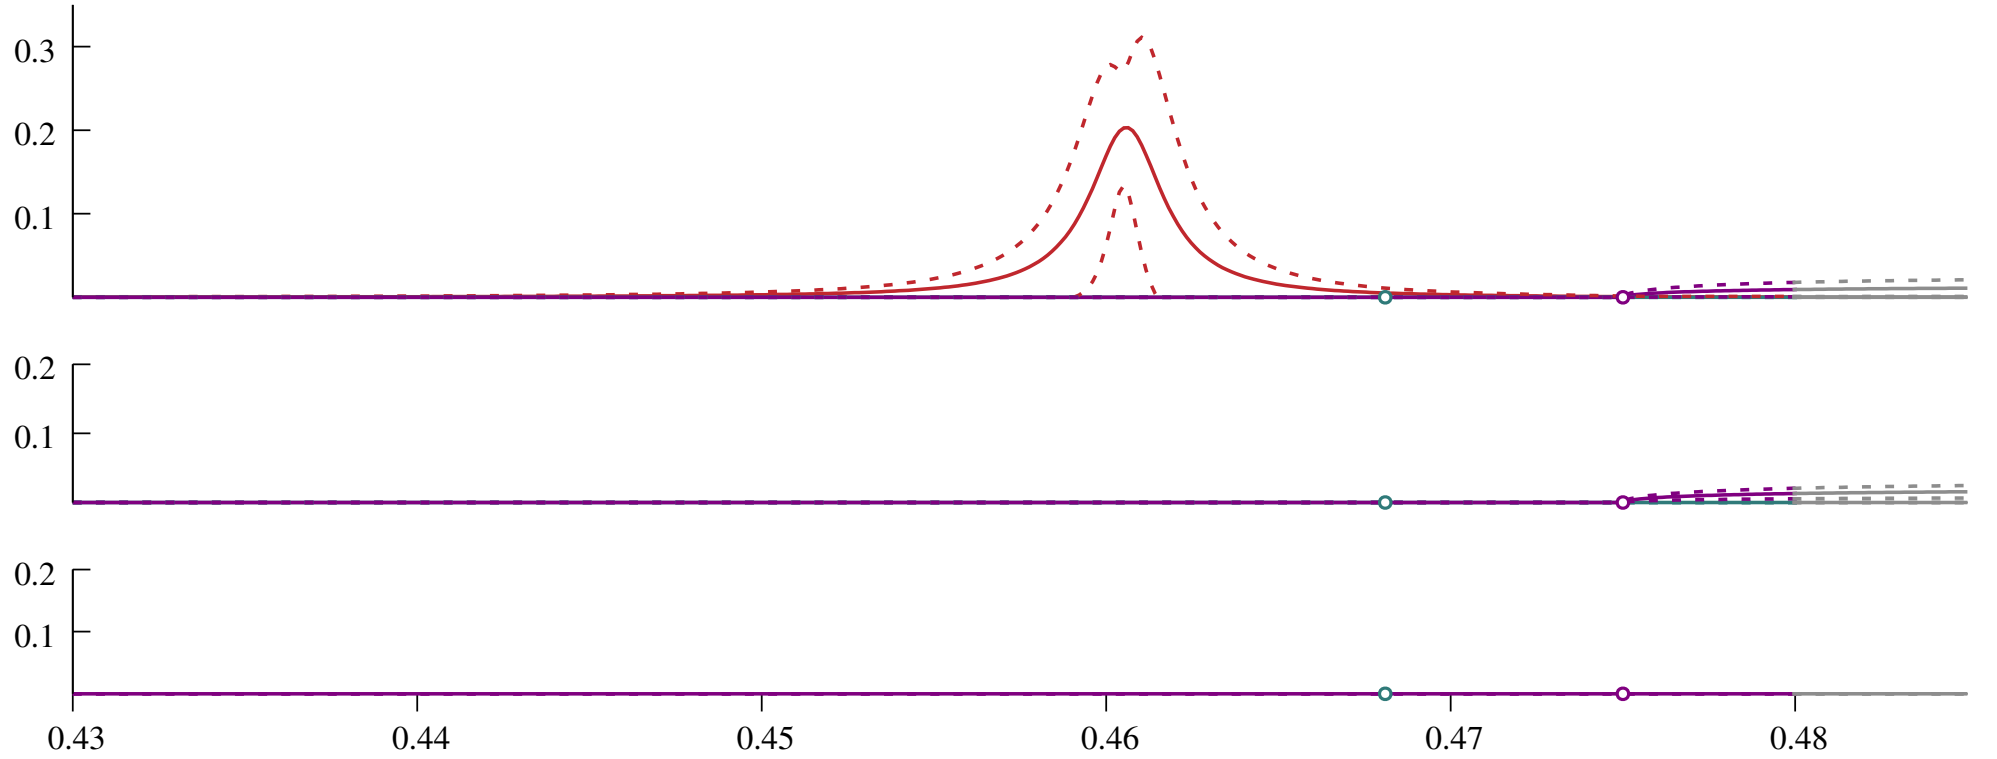

Figure 1.18: Similar to parts (b), (c) and (d) of Figure 7 in the manuscript,  $\rho_a \rho_b |t_{ab}|^2$  as a function of  $a_t E_{\text{cm}}$ . Top:  $\eta^1 \eta^s \{^1P_1\} \rightarrow \omega^s \eta^s \{^3P_1\}$  (red),  $\eta^1 \eta^s \{^1P_1\} \rightarrow f_1^s \eta^s \{^3S_1\}$  (cyan), and  $\eta^1 \eta^s \{^1P_1\} \rightarrow h_1^s \eta^s \{^3S_1\}$  (purple). Middle:  $\omega^s \eta^s \{^3P_1\} \rightarrow f_1^s \eta^s \{^3S_1\}$  (cyan), and  $\omega^s \eta^s \{^3P_1\} \rightarrow h_1^s \eta^s \{^3S_1\}$  (purple). Bottom:  $f_1^s \eta^s \{^3S_1\} \rightarrow h_1^s \eta^s \{^3S_1\}$  (purple). Dashed lines indicate one standard deviation statistical uncertainties.

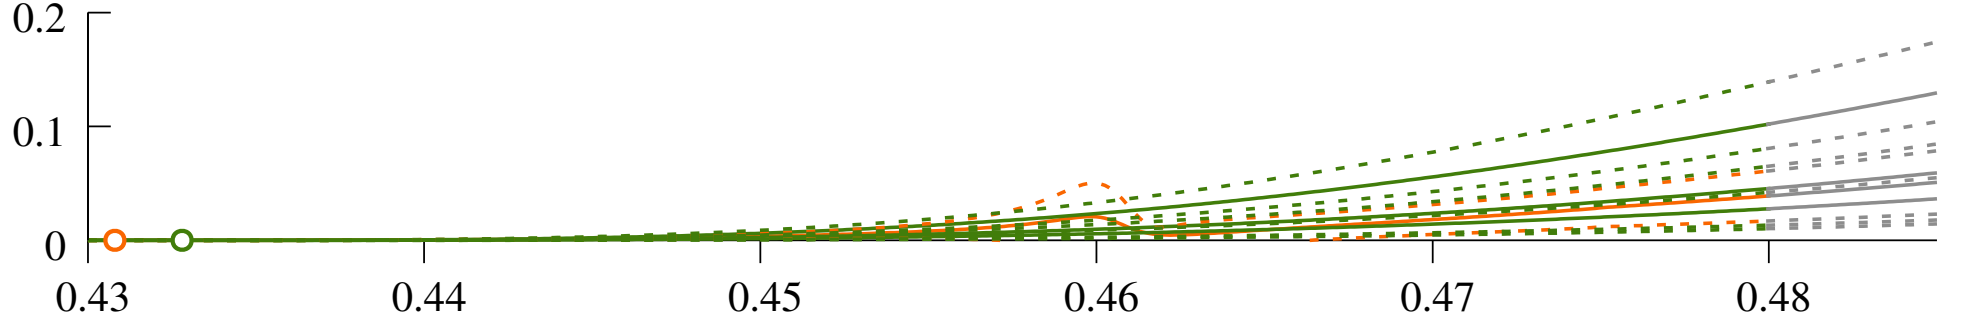

Figure 1.19: Similar to parts (e) and (f) of Figure 7 in the manuscript,  $\rho_a \rho_b |t_{ab}|^2$  as a function of  $a_t E_{cm}$  for  $\omega^s \omega^s \{^3P_1\} \rightarrow \omega^s \omega^s \{^3P_1\}$  (orange),  $\omega^1 \omega^s \{^1P_1, ^3P_1, ^5P_1\} \rightarrow \omega^s \omega^1 \{^1P_1, ^3P_1, ^5P_1\}$  (green). Dashed lines indicate one standard deviation statistical uncertainties.

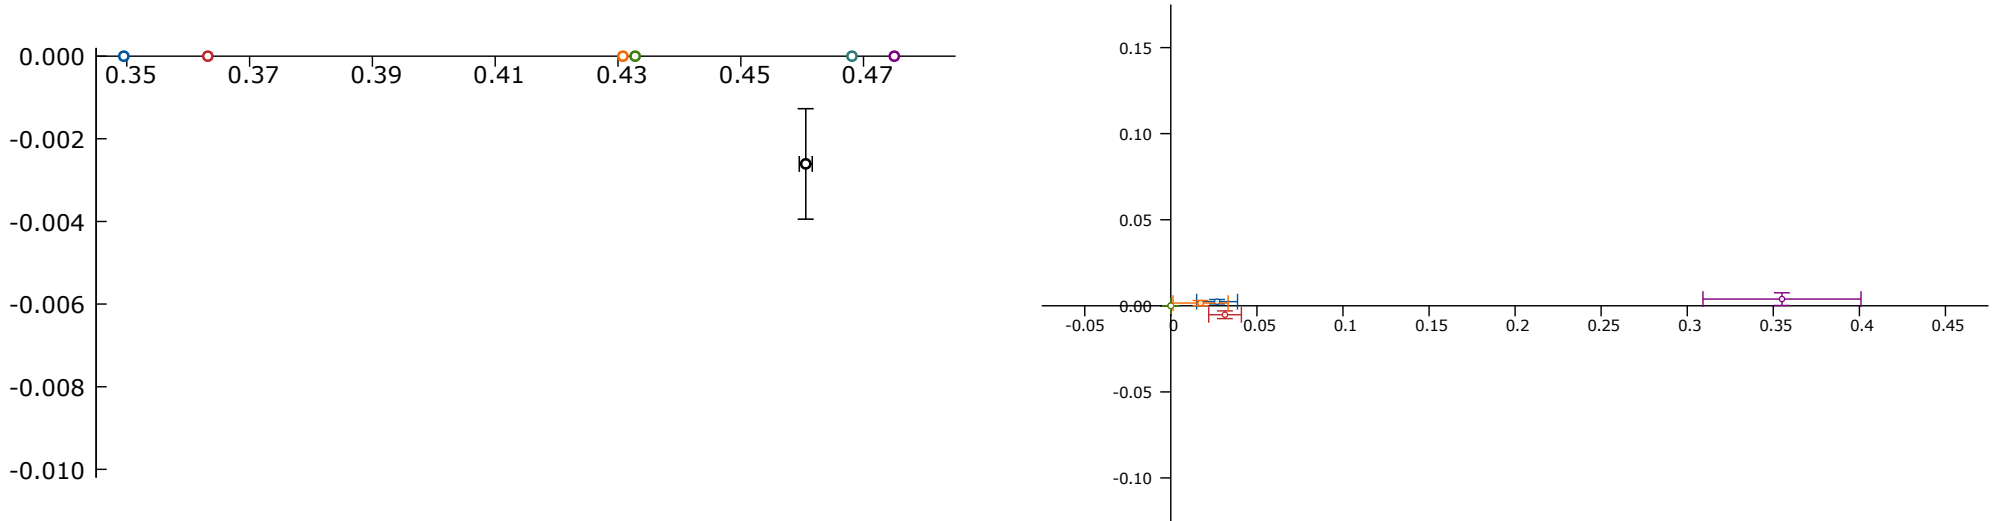

Figure 1.20: Left: Similar to Figure 13 in the manuscript, pole position on the proximal sheet (closest to physical scattering) with  $\text{Re}(a_t \sqrt{s})$  on the horizontal axis and  $2 \text{Im}(a_t \sqrt{s})$  on the vertical axis. Right: Similar to Figure 14 in the manuscript, the corresponding couplings with  $\text{Re}(a_t c)$  on the horizontal axis and  $\text{Im}(a_t c)$  on the vertical axis.

$$1.5 \quad \{m, g_{a,b,d_2,f}^{(0)}, \gamma_{(a,a),(b,b),(c,c),(d_1,d_1),(d_2,d_2),(d_3,d_3),(e,e)}^{(0)}\}(\mathbf{CM}_m)$$

minimised with chisq/nDoF = 45.49 / (53 - 12) = 1.11

|                                                           |  |                        |  |      |      |      |      |      |      |       |       |       |       |       |       |
|-----------------------------------------------------------|--|------------------------|--|------|------|------|------|------|------|-------|-------|-------|-------|-------|-------|
| =====                                                     |  |                        |  |      |      |      |      |      |      |       |       |       |       |       |       |
| JP1-_g_eta8:eta1/1^P_1_pole0                              |  | 0.20804 +/- 0.16031    |  | 1.00 | 0.78 | 0.70 | 0.00 | 0.13 | 0.29 | -0.02 | -0.03 | 0.02  | -0.06 | -0.06 | 0.64  |
| JP1-_g_h8:eta8/3^S_1_pole0                                |  | 0.85396 +/- 0.66681    |  |      | 1.00 | 0.90 | 0.00 | 0.31 | 0.43 | -0.08 | -0.00 | 0.06  | -0.00 | -0.01 | 0.51  |
| JP1-_g_omega8:eta8/3^P_1_pole0                            |  | 0.27413 +/- 0.19996    |  |      |      | 1.00 | 0.00 | 0.31 | 0.39 | -0.30 | 0.02  | 0.05  | 0.01  | 0.01  | 0.39  |
| JP1-_g_omega8:omega1/3^P_1_pole0                          |  | 1.1862e-05 +/- 0.22387 |  |      |      |      | 1.00 | 0.00 | 0.00 | -0.00 | -0.00 | -0.00 | -0.00 | -0.00 | 0.00  |
| JP1-_gamma_eta8:eta1/1^P_1 eta8:eta1/1^P_1_order0         |  | 1.4411 +/- 0.57094     |  |      |      |      |      | 1.00 | 0.55 | -0.02 | 0.02  | 0.06  | 0.03  | 0.02  | -0.02 |
| JP1-_gamma_f8:eta8/3^S_1 f8:eta8/3^S_1_order0             |  | -2.1023 +/- 0.30785    |  |      |      |      |      |      | 1.00 | 0.00  | 0.03  | 0.08  | 0.03  | 0.04  | 0.14  |
| JP1-_gamma_omega8:eta8/3^P_1 omega8:eta8/3^P_1_order0     |  | -3.5756 +/- 0.62224    |  |      |      |      |      |      |      | 1.00  | 0.05  | 0.08  | 0.06  | 0.13  | 0.11  |
| JP1-_gamma_omega8:omega1/1^P_1 omega8:omega1/1^P_1_order0 |  | 9.5810 +/- 2.3636      |  |      |      |      |      |      |      |       | 1.00  | 0.06  | 0.39  | 0.43  | -0.06 |
| JP1-_gamma_omega8:omega1/3^P_1 omega8:omega1/3^P_1_order0 |  | 12.062 +/- 4.9318      |  |      |      |      |      |      |      |       |       | 1.00  | 0.13  | 0.10  | 0.05  |
| JP1-_gamma_omega8:omega1/5^P_1 omega8:omega1/5^P_1_order0 |  | 19.269 +/- 3.7386      |  |      |      |      |      |      |      |       |       |       | 1.00  | 0.46  | -0.09 |
| JP1-_gamma_omega8:omega8/3^P_1 omega8:omega8/3^P_1_order0 |  | 10.560 +/- 2.8998      |  |      |      |      |      |      |      |       |       |       |       | 1.00  | -0.11 |
| JP1-_m_pole0                                              |  | 0.46076 +/- 0.0010259  |  |      |      |      |      |      |      |       |       |       |       |       | 1.00  |
| =====                                                     |  |                        |  |      |      |      |      |      |      |       |       |       |       |       |       |

Phase space prescription ::

pole0\_sub

eta8:eta1[-] f8:eta8[+] h8:eta8[-] omega8:eta8[-] omega8:omega1[-] omega8:omega8[-] lower half-plane

sqrt(s)\_pole = (0.46069 +/- 0.001003)  
+ (i/2)\*(-0.0022546 +/- 0.0011865) [-0.06]

s\_pole = (0.21223 +/- 0.00092402)  
+ i\*(-0.0010387 +/- 0.00054674) [-0.06]

| eta8:eta1                | f8:eta8                  | h8:eta8                  | omega8:eta8              | omega8:omega1            | omega8:omega8            |
|--------------------------|--------------------------|--------------------------|--------------------------|--------------------------|--------------------------|
| k_re= 0.1491 +/- 0.0008  | k_re= -0.0029 +/- 0.0015 | k_re= -0.0020 +/- 0.0011 | k_re= 0.1402 +/- 0.0008  | k_re= 0.0789 +/- 0.0015  | k_re= 0.0816 +/- 0.0014  |
| k_im= -0.0009 +/- 0.0005 | k_im= 0.0386 +/- 0.0025  | k_im= 0.0533 +/- 0.0018  | k_im= -0.0009 +/- 0.0005 | k_im= -0.0016 +/- 0.0009 | k_im= -0.0016 +/- 0.0008 |
| corr= [-0.06]            | corr= [ 0.15]            | corr= [ 0.11]            | corr= [-0.06]            | corr= [-0.04]            | corr= [-0.04]            |

  

| eta8:eta1/1^P_1              | f8:eta8/3^S_1                | h8:eta8/3^S_1(*)             | omega8:eta8/3^P_1             | omega8:omega1/1^P_1          | omega8:omega1/3^P_1            | omega8:omega1/5^P_1          | omega8:omega8/3^P_1          |
|------------------------------|------------------------------|------------------------------|-------------------------------|------------------------------|--------------------------------|------------------------------|------------------------------|
| g = 0.0258 +/- 0.0121        | g = 0.0000 +/- 0.0000        | g = 0.3565 +/- 0.0448        | g = 0.0315 +/- 0.0096         | g = 0.0000 +/- 0.0000        | g = 0.0006 +/- 0.0095          | g = 0.0000 +/- 0.0000        | g = 0.0000 +/- 0.0000        |
| arg(g)/pi= 0.0283 +/- 0.0104 | arg(g)/pi= 0.4963 +/- 0.0027 | arg(g)/pi= 0.0037 +/- 0.0027 | arg(g)/pi= -0.0524 +/- 0.0094 | arg(g)/pi= 0.4963 +/- 0.0027 | arg(g)/pi= -0.4778 +/- 11.1679 | arg(g)/pi= 0.4963 +/- 0.0027 | arg(g)/pi= 0.4963 +/- 0.0027 |
| g_re= 0.0257 +/- 0.0121      | g_re= 0.0000 +/- 0.0000      | g_re= 0.3564 +/- 0.0447      | g_re= 0.0311 +/- 0.0094       | g_re= 0.0000 +/- 0.0000      | g_re= -0.0000 +/- 0.0156       | g_re= 0.0000 +/- 0.0000      | g_re= 0.0000 +/- 0.0000      |
| g_im= 0.0023 +/- 0.0013      | g_im= 0.0000 +/- 0.0000      | g_im= 0.0041 +/- 0.0034      | g_im= -0.0052 +/- 0.0022      | g_im= 0.0000 +/- 0.0000      | g_im= -0.0000 +/- 0.0015       | g_im= 0.0000 +/- 0.0000      | g_im= 0.0000 +/- 0.0000      |
| corr= [ 0.76]                | corr= [-0.51]                | corr= [ 0.71]                | corr= [-0.93]                 | corr= [-0.51]                | corr= [ 1.00]                  | corr= [-0.51]                | corr= [-0.51]                |

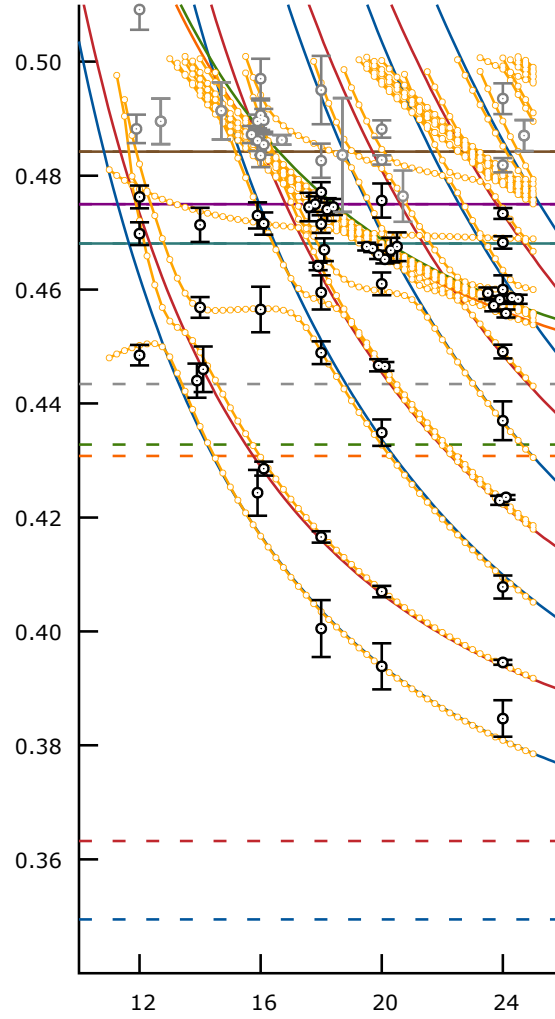

Figure 1.21: Similar to Figure 6 in the manuscript, the finite-volume spectrum, plotted as  $a_t E_{\text{cm}}$ , as a function of spatial extent  $L/a_s$ . Orange points/curves show the spectrum calculated from the amplitude given above (no uncertainties are shown). Black and grey points are the computed lattice energies on each volume, slightly displaced horizontally for clarity (black points correspond to energies used in the fit whereas grey points were not used). Two-meson non-interacting energies are shown as solid coloured curves/lines, two-meson thresholds are shown as dashed/solid horizontal lines, and the  $\eta^s \eta^s \eta^s$  threshold is shown as a dashed grey horizontal line.

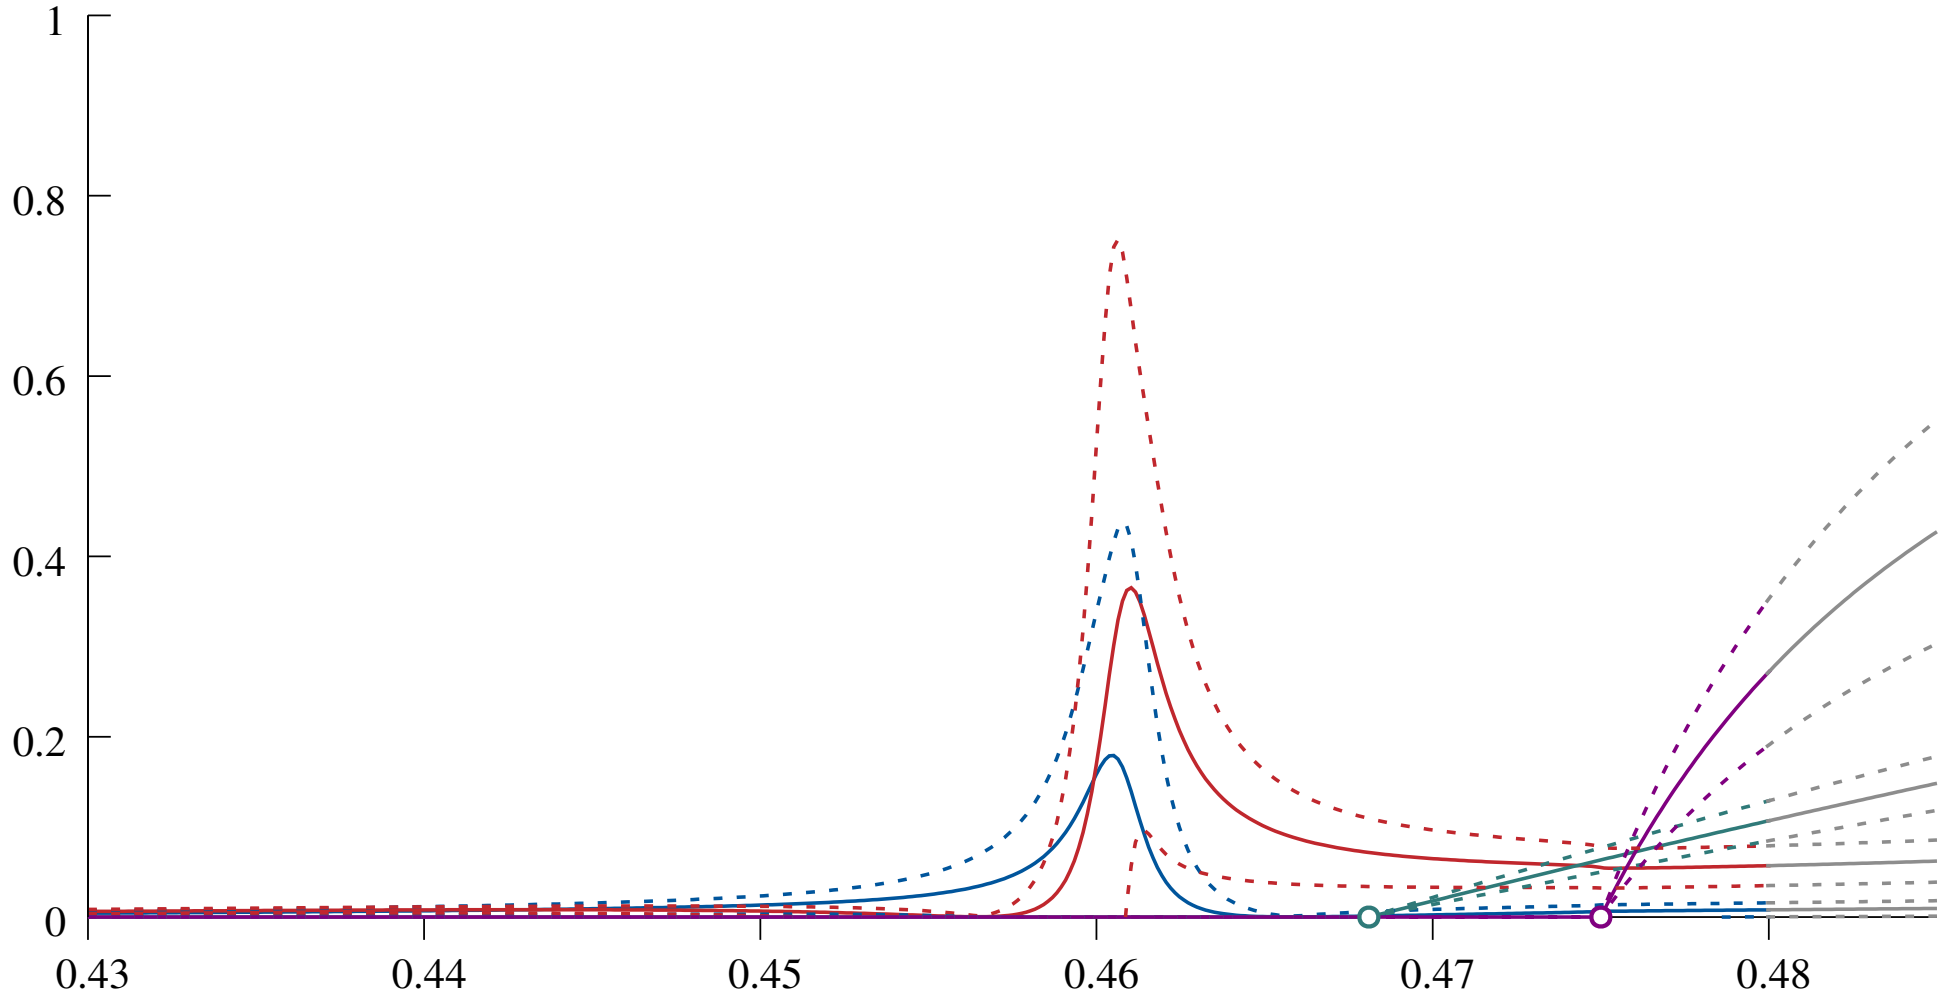

Figure 1.22: Similar to part (a) of Figure 7 in the manuscript,  $\rho_a \rho_b |t_{ab}|^2$  as a function of  $a_t E_{\text{cm}}$  for  $\eta^1 \eta^s \{^1P_1\} \rightarrow \eta^1 \eta^s \{^1P_1\}$  (blue),  $\omega^s \eta^s \{^3P_1\} \rightarrow \omega^s \eta^s \{^3P_1\}$  (red),  $f_1^s \eta^s \{^3S_1\} \rightarrow f_1^s \eta^s \{^3S_1\}$  (cyan), and  $h_1^s \eta^s \{^3S_1\} \rightarrow h_1^s \eta^s \{^3S_1\}$  (purple). Dashed lines indicate one standard deviation statistical uncertainties.

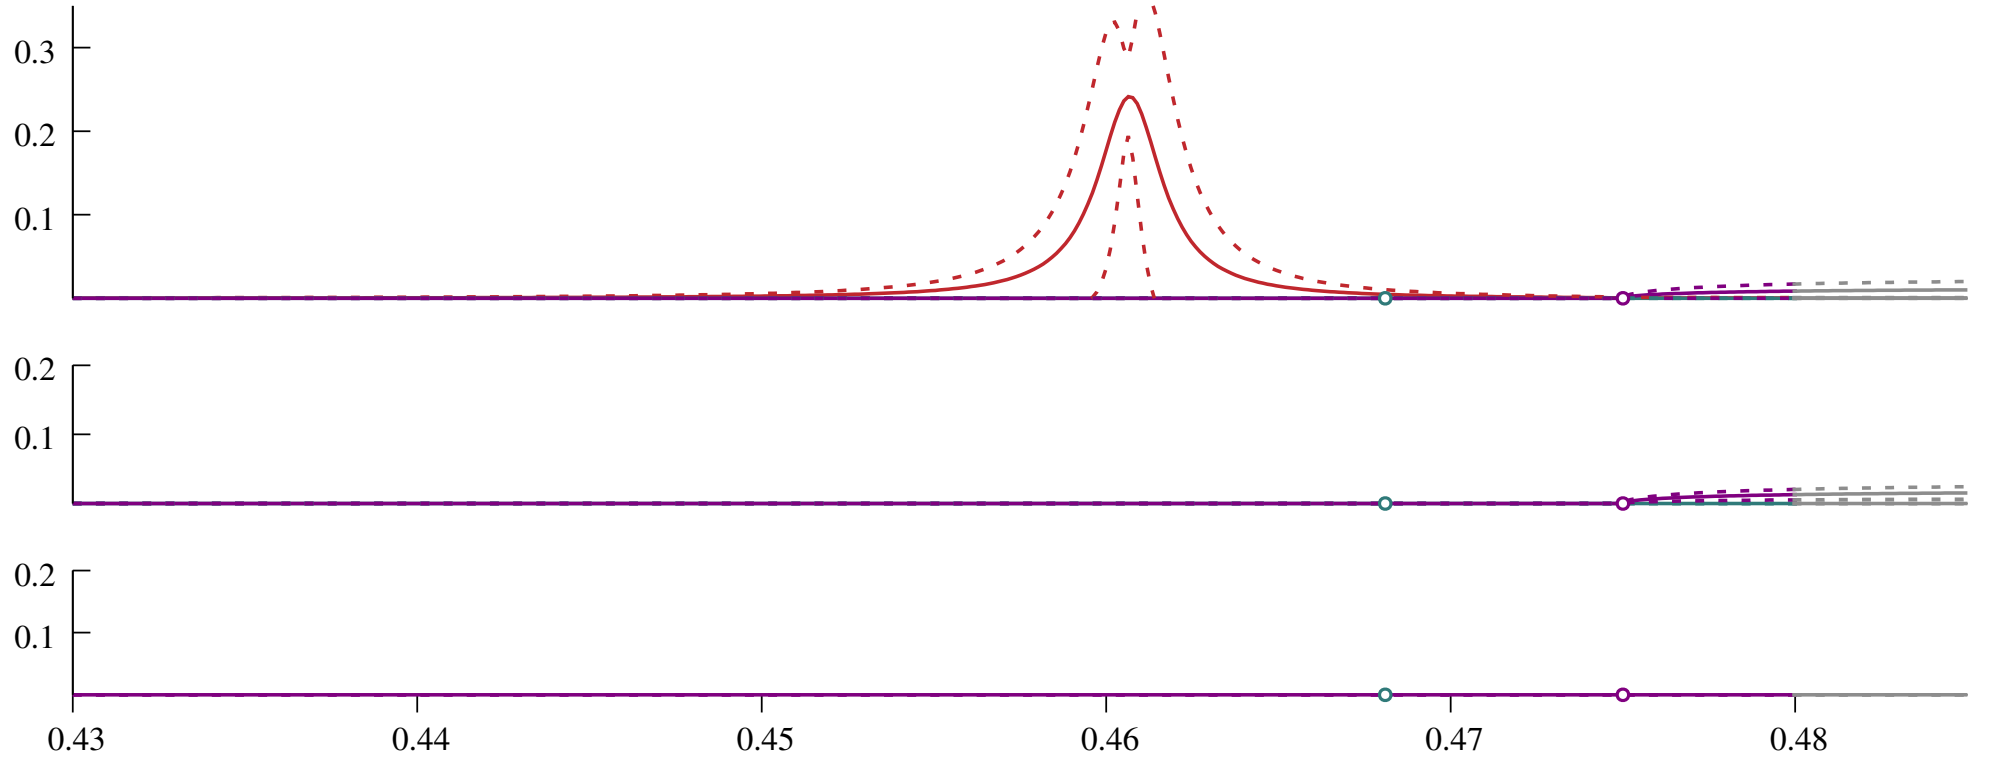

Figure 1.23: Similar to parts (b), (c) and (d) of Figure 7 in the manuscript,  $\rho_a \rho_b |t_{ab}|^2$  as a function of  $a_t E_{\text{cm}}$ . Top:  $\eta^1 \eta^s \{^1P_1\} \rightarrow \omega^s \eta^s \{^3P_1\}$  (red),  $\eta^1 \eta^s \{^1P_1\} \rightarrow f_1^s \eta^s \{^3S_1\}$  (cyan), and  $\eta^1 \eta^s \{^1P_1\} \rightarrow h_1^s \eta^s \{^3S_1\}$  (purple). Middle:  $\omega^s \eta^s \{^3P_1\} \rightarrow f_1^s \eta^s \{^3S_1\}$  (cyan), and  $\omega^s \eta^s \{^3P_1\} \rightarrow h_1^s \eta^s \{^3S_1\}$  (purple). Bottom:  $f_1^s \eta^s \{^3S_1\} \rightarrow h_1^s \eta^s \{^3S_1\}$  (purple). Dashed lines indicate one standard deviation statistical uncertainties.

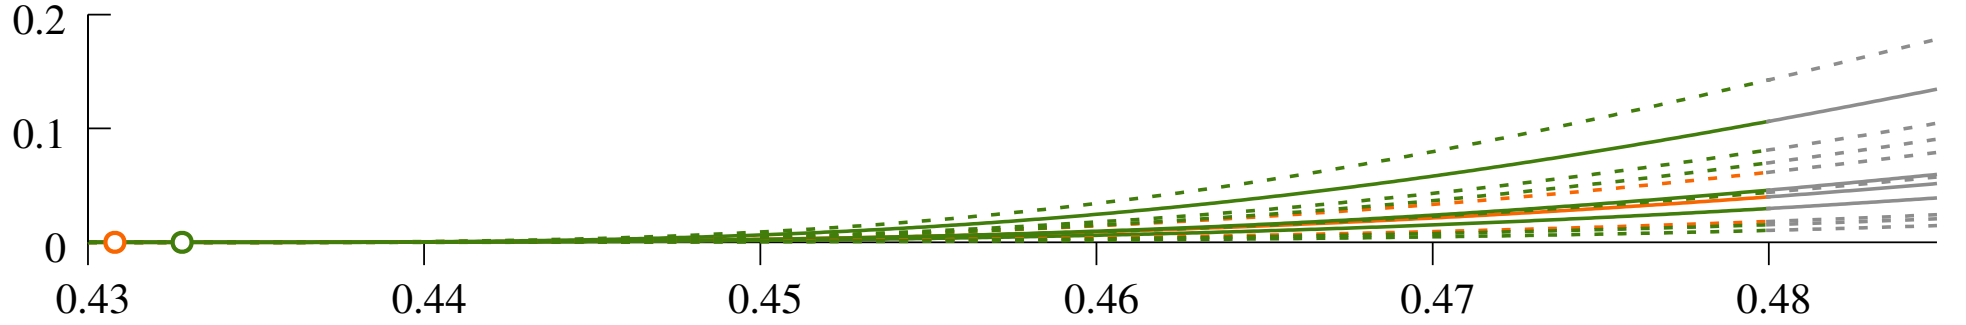

Figure 1.24: Similar to parts (e) and (f) of Figure 7 in the manuscript,  $\rho_a \rho_b |t_{ab}|^2$  as a function of  $a_t E_{cm}$  for  $\omega^s \omega^s \{^3P_1\} \rightarrow \omega^s \omega^s \{^3P_1\}$  (orange),  $\omega^1 \omega^s \{^1P_1, ^3P_1, ^5P_1\} \rightarrow \omega^s \omega^1 \{^1P_1, ^3P_1, ^5P_1\}$  (green). Dashed lines indicate one standard deviation statistical uncertainties.

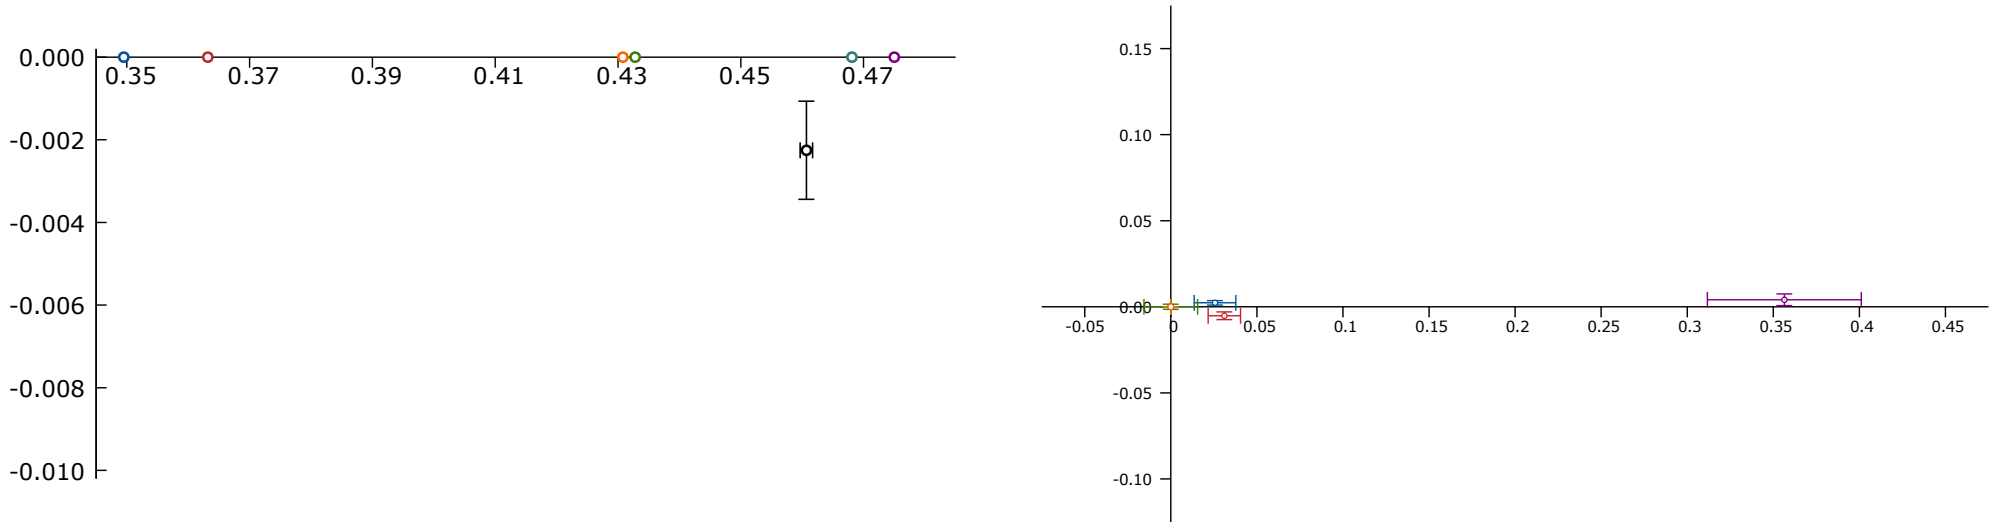

Figure 1.25: Left: Similar to Figure 13 in the manuscript, pole position on the proximal sheet (closest to physical scattering) with  $\text{Re}(a_t \sqrt{s})$  on the horizontal axis and  $2 \text{Im}(a_t \sqrt{s})$  on the vertical axis. Right: Similar to Figure 14 in the manuscript, the corresponding couplings with  $\text{Re}(a_t c)$  on the horizontal axis and  $\text{Im}(a_t c)$  on the vertical axis.

$$1.6 \quad \{m, g_{\alpha, b, \vartheta_1, \vartheta_2, \vartheta_3, f}^{(0)}, \gamma_{(\alpha, \alpha), (b, b), (c, c), (\vartheta_1, \vartheta_1), (\vartheta_2, \vartheta_2), (\vartheta_3, \vartheta_3), (c, c)}^{(0)}\}(\mathbf{CM}_m)$$

minimised with chisq/nDoF = 45.49 / (53 - 14) = 1.17

|                                                          |  |                         |  |      |      |      |      |       |      |      |      |       |       |       |       |       |       |
|----------------------------------------------------------|--|-------------------------|--|------|------|------|------|-------|------|------|------|-------|-------|-------|-------|-------|-------|
| =====                                                    |  |                         |  |      |      |      |      |       |      |      |      |       |       |       |       |       |       |
| JP1-g_eta8:eta1/1^P_1_pole0                              |  | 0.20804 +/- 0.16031     |  | 1.00 | 0.78 | 0.70 | 0.00 | 0.00  | 0.00 | 0.13 | 0.29 | -0.02 | -0.03 | 0.02  | -0.06 | -0.06 | 0.64  |
| JP1-g_h8:eta8/3^S_1_pole0                                |  | 0.85397 +/- 0.66681     |  |      | 1.00 | 0.90 | 0.00 | 0.00  | 0.00 | 0.31 | 0.43 | -0.08 | -0.00 | 0.06  | -0.00 | -0.01 | 0.51  |
| JP1-g_omega8:eta8/3^P_1_pole0                            |  | 0.27413 +/- 0.19996     |  |      |      | 1.00 | 0.00 | 0.00  | 0.00 | 0.31 | 0.39 | -0.30 | 0.02  | 0.05  | 0.01  | 0.01  | 0.39  |
| JP1-g_omega8:omega1/1^P_1_pole0                          |  | -4.2626e-06 +/- 0.38535 |  |      |      |      | 1.00 | -0.00 | 0.00 | 0.00 | 0.00 | 0.00  | 0.00  | -0.00 | 0.00  | -0.00 | -0.00 |
| JP1-g_omega8:omega1/3^P_1_pole0                          |  | 1.1836e-05 +/- 0.22387  |  |      |      |      |      | 1.00  | 0.00 | 0.00 | 0.00 | -0.00 | -0.00 | -0.00 | -0.00 | -0.00 | 0.00  |
| JP1-g_omega8:omega1/5^P_1_pole0                          |  | -5.1632e-07 +/- 0.34767 |  |      |      |      |      |       | 1.00 | 0.00 | 0.00 | -0.00 | 0.00  | 0.00  | 0.00  | 0.00  | 0.00  |
| JP1-gamma_eta8:eta1/1^P_1 eta8:eta1/1^P_1_order0         |  | 1.4411 +/- 0.57094      |  |      |      |      |      |       |      | 1.00 | 0.55 | -0.02 | 0.02  | 0.06  | 0.03  | 0.02  | -0.02 |
| JP1-gamma_f8:eta8/3^S_1 f8:eta8/3^S_1_order0             |  | -2.1023 +/- 0.30785     |  |      |      |      |      |       |      |      | 1.00 | 0.00  | 0.03  | 0.08  | 0.03  | 0.04  | 0.14  |
| JP1-gamma_omega8:eta8/3^P_1 omega8:eta8/3^P_1_order0     |  | -3.5756 +/- 0.62223     |  |      |      |      |      |       |      |      |      | 1.00  | 0.05  | 0.08  | 0.06  | 0.13  | 0.11  |
| JP1-gamma_omega8:omega1/1^P_1 omega8:omega1/1^P_1_order0 |  | 9.5810 +/- 2.3636       |  |      |      |      |      |       |      |      |      |       | 1.00  | 0.06  | 0.39  | 0.43  | -0.06 |
| JP1-gamma_omega8:omega1/3^P_1 omega8:omega1/3^P_1_order0 |  | 12.062 +/- 4.9318       |  |      |      |      |      |       |      |      |      |       |       | 1.00  | 0.13  | 0.10  | 0.05  |
| JP1-gamma_omega8:omega1/5^P_1 omega8:omega1/5^P_1_order0 |  | 19.269 +/- 3.7386       |  |      |      |      |      |       |      |      |      |       |       |       | 1.00  | 0.46  | -0.09 |
| JP1-gamma_omega8:omega8/3^P_1 omega8:omega8/3^P_1_order0 |  | 10.560 +/- 2.8998       |  |      |      |      |      |       |      |      |      |       |       |       |       | 1.00  | -0.11 |
| JP1-m_pole0                                              |  | 0.46076 +/- 0.0010259   |  |      |      |      |      |       |      |      |      |       |       |       |       |       | 1.00  |
| =====                                                    |  |                         |  |      |      |      |      |       |      |      |      |       |       |       |       |       |       |

Phase space prescription ::

pole0\_sub

eta8:eta1[-] f8:eta8[+] h8:eta8[+] omega8:eta8[-] omega8:omega1[-] omega8:omega8[-] lower half-plane

sqrt(s)\_pole = (0.46069 +/- 0.0010692)  
+ (i/2)\*(-0.0022565 +/- 0.0012685) [-0.07]

s\_pole = (0.21223 +/- 0.00098506)  
+ i\*(-0.0010395 +/- 0.00058456) [-0.07]

| eta8:eta1                | f8:eta8                  | h8:eta8                  | omega8:eta8              | omega8:omega1            | omega8:omega8            |
|--------------------------|--------------------------|--------------------------|--------------------------|--------------------------|--------------------------|
| k_re= 0.1491 +/- 0.0008  | k_re= -0.0029 +/- 0.0016 | k_re= -0.0020 +/- 0.0012 | k_re= 0.1402 +/- 0.0009  | k_re= 0.0789 +/- 0.0016  | k_re= 0.0816 +/- 0.0015  |
| k_im= -0.0009 +/- 0.0005 | k_im= 0.0386 +/- 0.0027  | k_im= 0.0533 +/- 0.0019  | k_im= -0.0009 +/- 0.0005 | k_im= -0.0016 +/- 0.0009 | k_im= -0.0016 +/- 0.0009 |
| corr= [-0.06]            | corr= [ 0.15]            | corr= [ 0.11]            | corr= [-0.06]            | corr= [-0.05]            | corr= [-0.05]            |

| eta8:eta1/1^P_1              | f8:eta8/3^S_1                | h8:eta8/3^S_1(*)             | omega8:eta8/3^P_1             | omega8:omega1/1^P_1            | omega8:omega1/3^P_1            | omega8:omega1/5^P_1            | omega8:omega8/3^P_1          |
|------------------------------|------------------------------|------------------------------|-------------------------------|--------------------------------|--------------------------------|--------------------------------|------------------------------|
| g = 0.0258 +/- 0.0126        | g = 0.0000 +/- 0.0000        | g = 0.3565 +/- 0.0449        | g = 0.0315 +/- 0.0103         | g = 0.0009 +/- 0.0158          | g = 0.0005 +/- 0.0092          | g = 0.0008 +/- 0.0146          | g = 0.0000 +/- 0.0000        |
| arg(g)/pi= 0.0283 +/- 0.0111 | arg(g)/pi= 0.4963 +/- 0.0028 | arg(g)/pi= 0.0037 +/- 0.0028 | arg(g)/pi= -0.0524 +/- 0.0089 | arg(g)/pi= -0.4826 +/- 11.1684 | arg(g)/pi= -0.4698 +/- 11.1694 | arg(g)/pi= -0.4561 +/- 11.1672 | arg(g)/pi= 0.4963 +/- 0.0028 |
| g_re= 0.0257 +/- 0.0126      | g_re= 0.0000 +/- 0.0000      | g_re= 0.3564 +/- 0.0449      | g_re= 0.0311 +/- 0.0101       | g_re= -0.0000 +/- 0.0255       | g_re= 0.0000 +/- 0.0151        | g_re= 0.0000 +/- 0.0233        | g_re= 0.0000 +/- 0.0000      |
| g_im= 0.0023 +/- 0.0014      | g_im= 0.0000 +/- 0.0000      | g_im= 0.0041 +/- 0.0035      | g_im= -0.0052 +/- 0.0022      | g_im= 0.0000 +/- 0.0019        | g_im= 0.0000 +/- 0.0014        | g_im= -0.0000 +/- 0.0037       | g_im= 0.0000 +/- 0.0000      |
| corr= [ 0.76]                | corr= [-0.47]                | corr= [ 0.69]                | corr= [-0.94]                 | corr= [ 1.00]                  | corr= [ 1.00]                  | corr= [ 1.00]                  | corr= [-0.47]                |

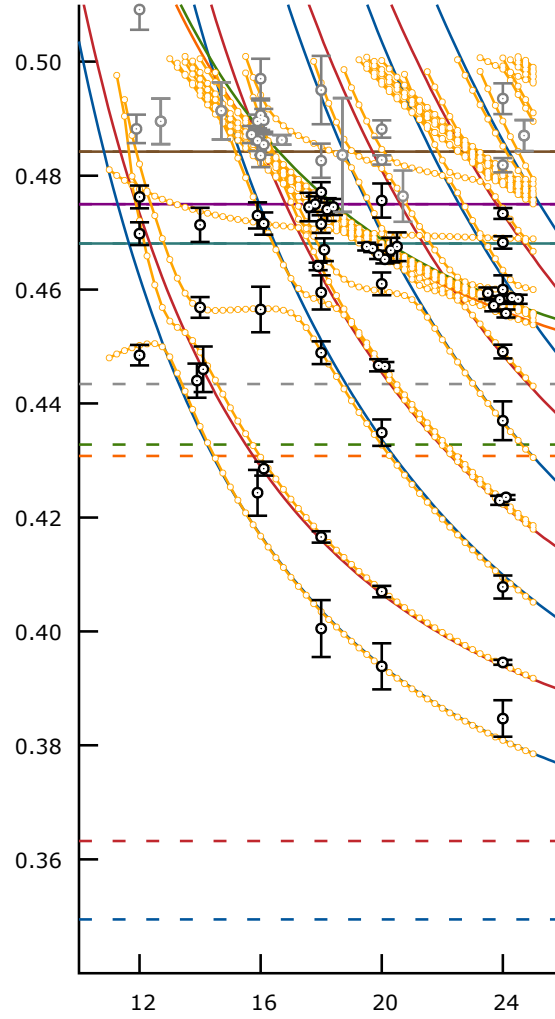

Figure 1.26: Similar to Figure 6 in the manuscript, the finite-volume spectrum, plotted as  $a_t E_{\text{cm}}$ , as a function of spatial extent  $L/a_s$ . Orange points/curves show the spectrum calculated from the amplitude given above (no uncertainties are shown). Black and grey points are the computed lattice energies on each volume, slightly displaced horizontally for clarity (black points correspond to energies used in the fit whereas grey points were not used). Two-meson non-interacting energies are shown as solid coloured curves/lines, two-meson thresholds are shown as dashed/solid horizontal lines, and the  $\eta^s \eta^s \eta^s$  threshold is shown as a dashed grey horizontal line.

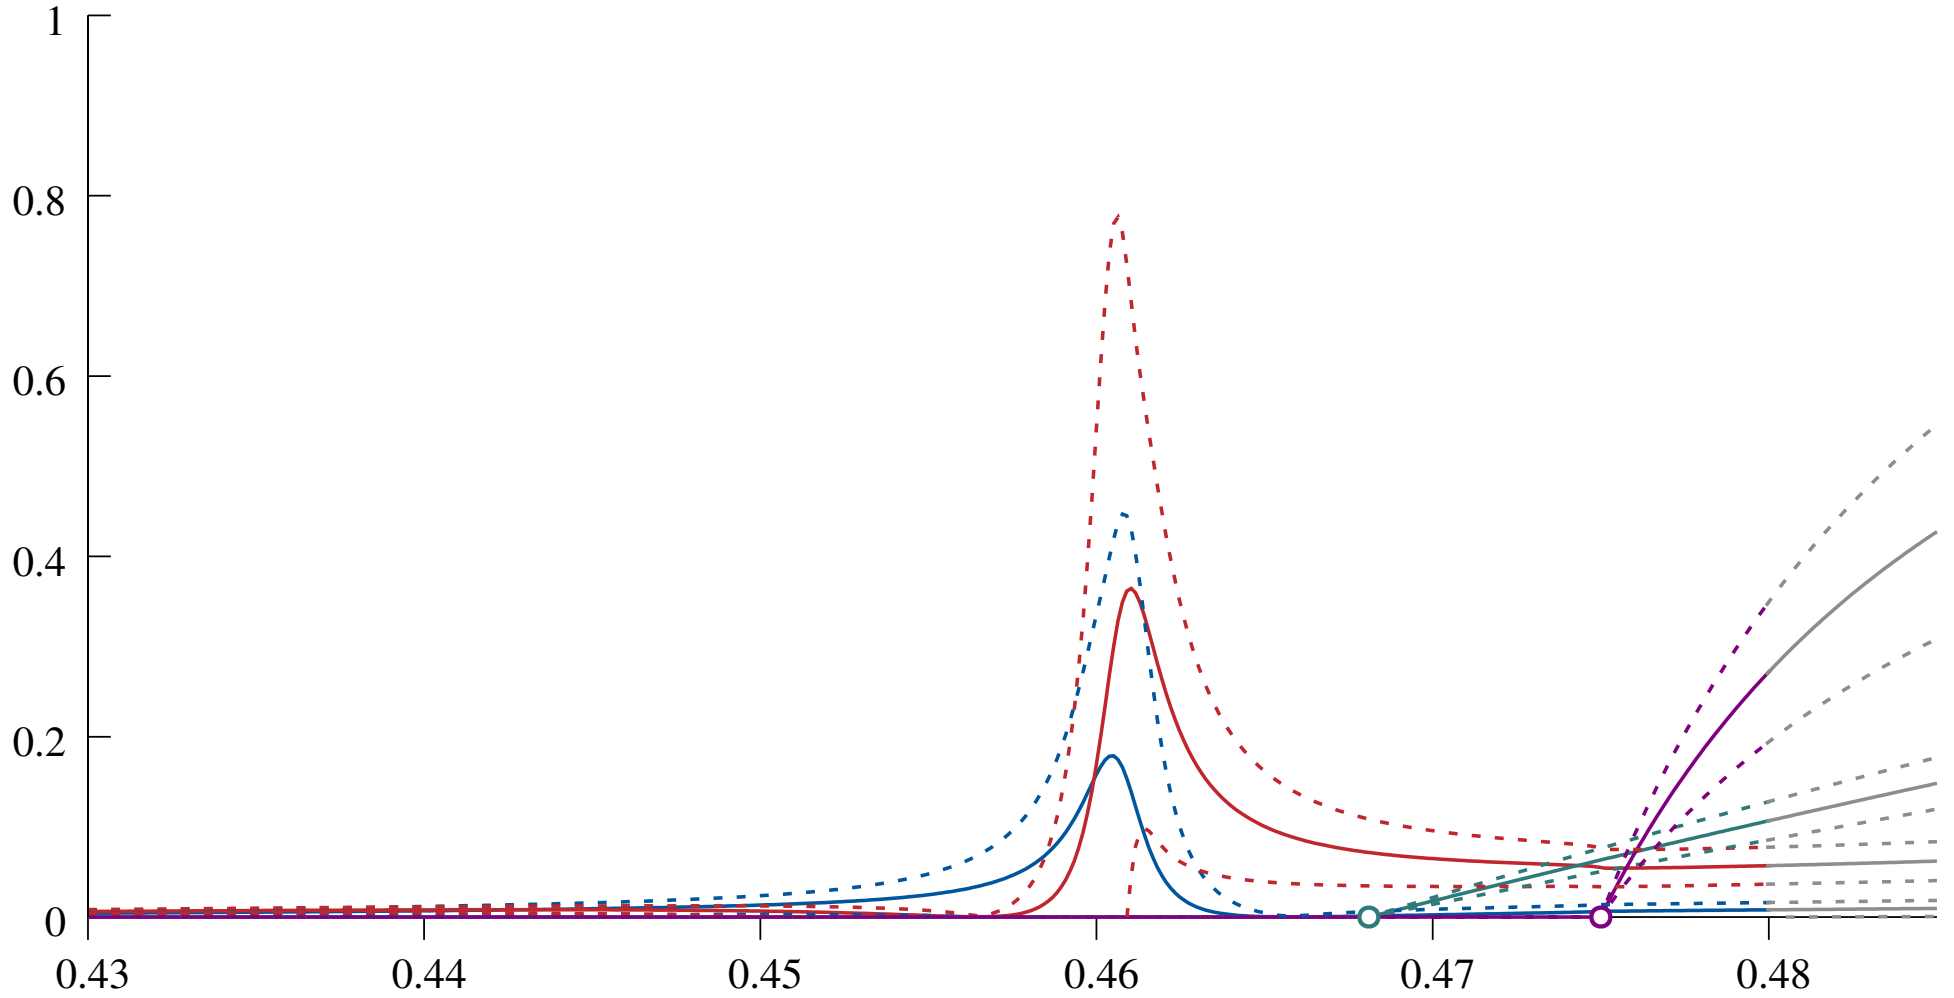

Figure 1.27: Similar to part (a) of Figure 7 in the manuscript,  $\rho_a \rho_b |t_{ab}|^2$  as a function of  $a_t E_{\text{cm}}$  for  $\eta^1 \eta^s \{^1P_1\} \rightarrow \eta^1 \eta^s \{^1P_1\}$  (blue),  $\omega^s \eta^s \{^3P_1\} \rightarrow \omega^s \eta^s \{^3P_1\}$  (red),  $f_1^s \eta^s \{^3S_1\} \rightarrow f_1^s \eta^s \{^3S_1\}$  (cyan), and  $h_1^s \eta^s \{^3S_1\} \rightarrow h_1^s \eta^s \{^3S_1\}$  (purple). Dashed lines indicate one standard deviation statistical uncertainties.

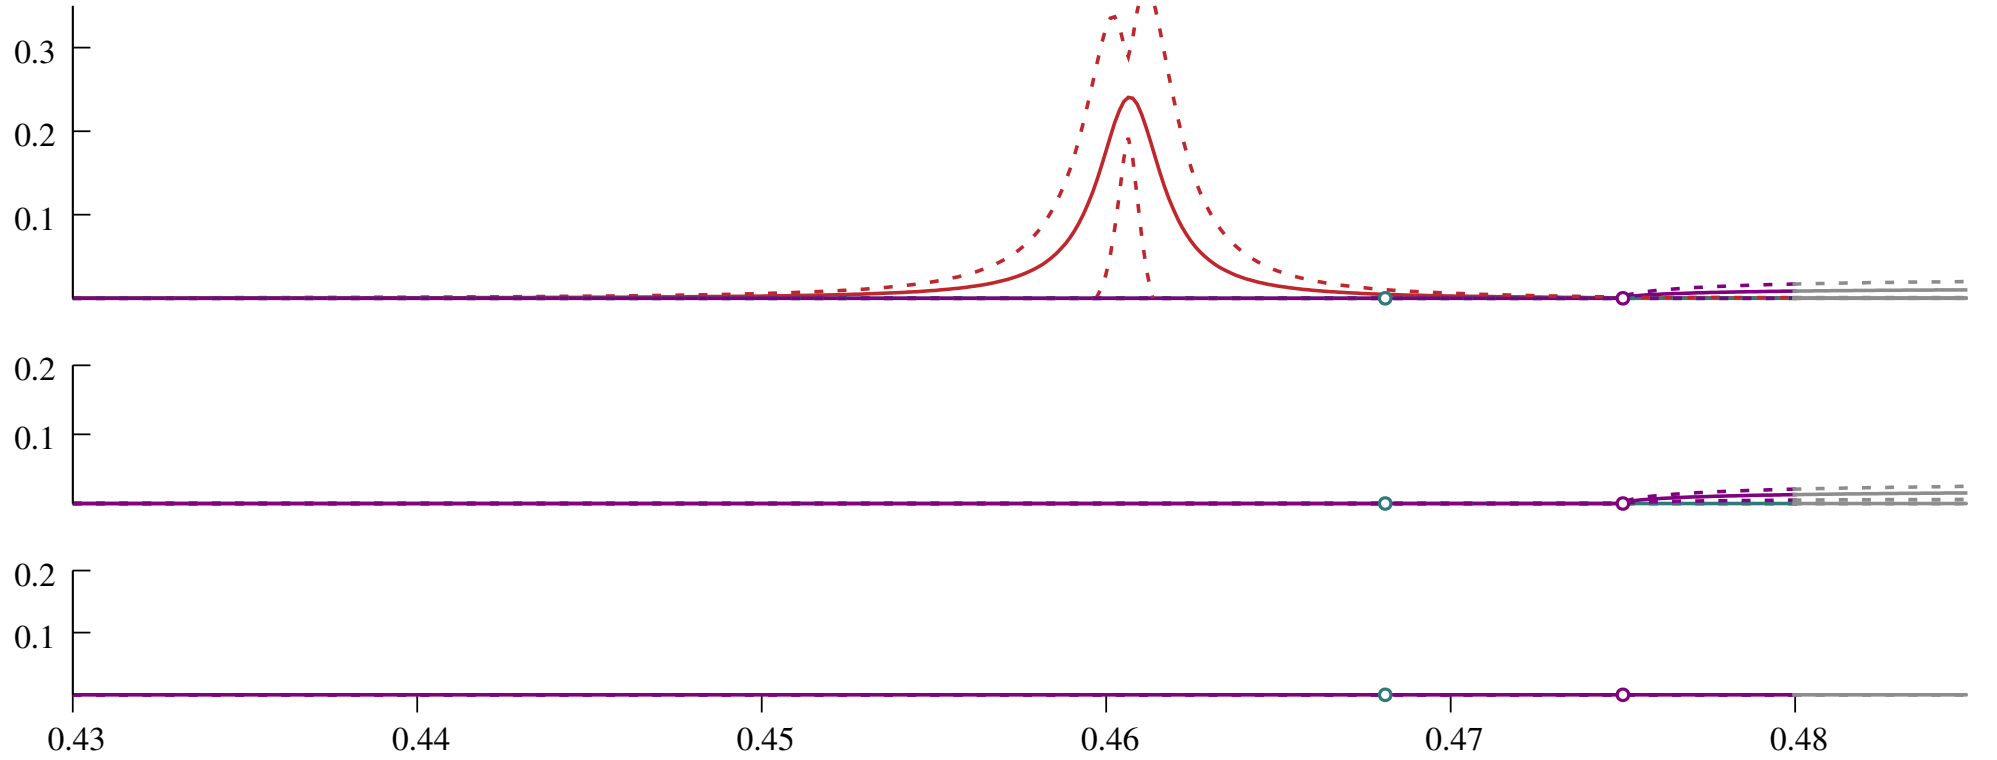

Figure 1.28: Similar to parts (b), (c) and (d) of Figure 7 in the manuscript,  $\rho_a \rho_b |t_{ab}|^2$  as a function of  $a_t E_{\text{cm}}$ . Top:  $\eta^1 \eta^s \{^1P_1\} \rightarrow \omega^s \eta^s \{^3P_1\}$  (red),  $\eta^1 \eta^s \{^1P_1\} \rightarrow f_1^s \eta^s \{^3S_1\}$  (cyan), and  $\eta^1 \eta^s \{^1P_1\} \rightarrow h_1^s \eta^s \{^3S_1\}$  (purple). Middle:  $\omega^s \eta^s \{^3P_1\} \rightarrow f_1^s \eta^s \{^3S_1\}$  (cyan), and  $\omega^s \eta^s \{^3P_1\} \rightarrow h_1^s \eta^s \{^3S_1\}$  (purple). Bottom:  $f_1^s \eta^s \{^3S_1\} \rightarrow h_1^s \eta^s \{^3S_1\}$  (purple). Dashed lines indicate one standard deviation statistical uncertainties.

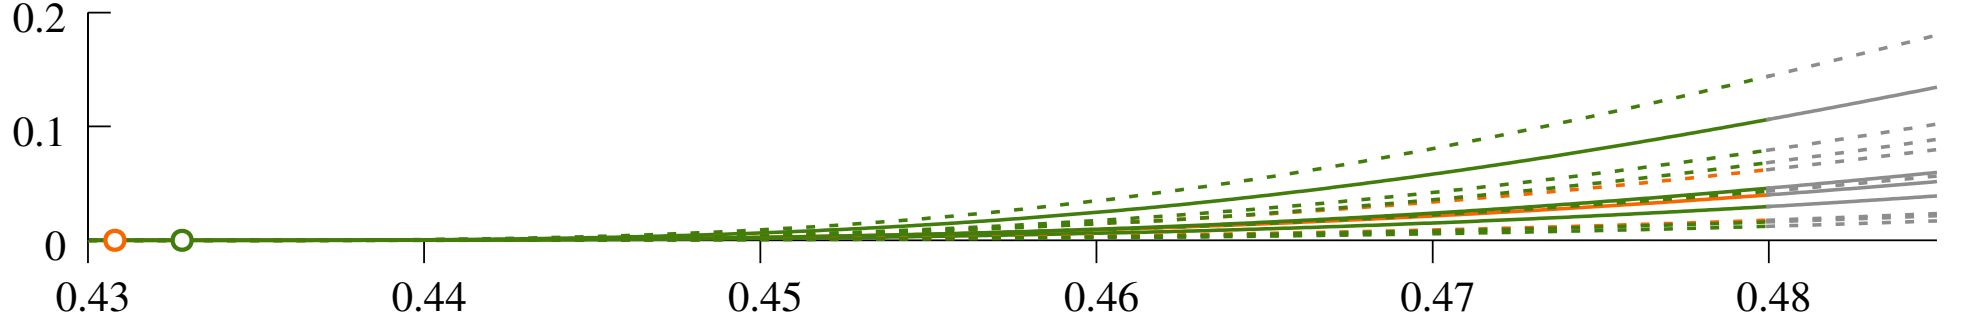

Figure 1.29: Similar to parts (e) and (f) of Figure 7 in the manuscript,  $\rho_a \rho_b |t_{ab}|^2$  as a function of  $a_t E_{cm}$  for  $\omega^s \omega^s \{^3P_1\} \rightarrow \omega^s \omega^s \{^3P_1\}$  (orange),  $\omega^1 \omega^s \{^1P_1, ^3P_1, ^5P_1\} \rightarrow \omega^s \omega^1 \{^1P_1, ^3P_1, ^5P_1\}$  (green). Dashed lines indicate one standard deviation statistical uncertainties.

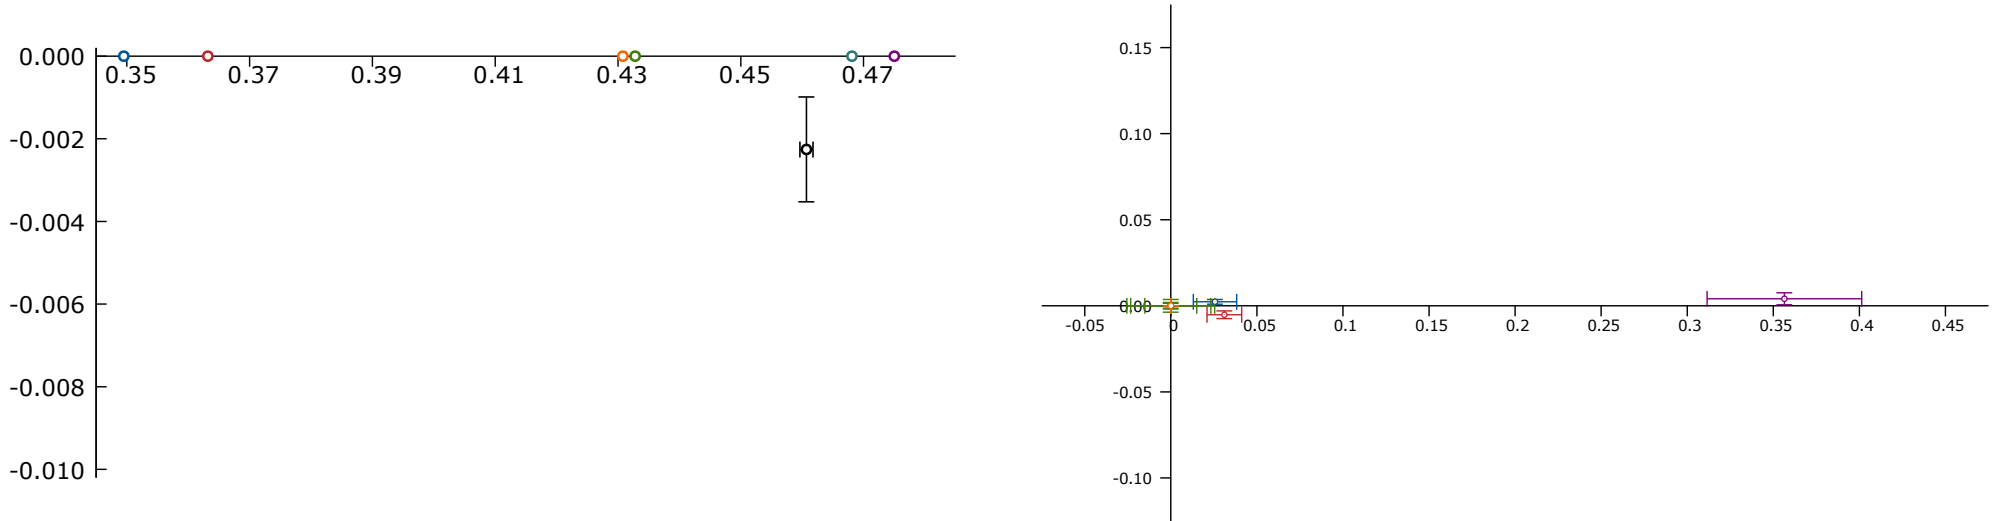

Figure 1.30: Left: Similar to Figure 13 in the manuscript, pole position on the proximal sheet (closest to physical scattering) with  $\text{Re}(a_t \sqrt{s})$  on the horizontal axis and  $2 \text{Im}(a_t \sqrt{s})$  on the vertical axis. Right: Similar to Figure 14 in the manuscript, the corresponding couplings with  $\text{Re}(a_t c)$  on the horizontal axis and  $\text{Im}(a_t c)$  on the vertical axis.

$$1.7 \quad \{m, g_{\alpha, b, c, d_1, d_2, d_3, f}^{(0)}, \gamma_{(\alpha, \alpha), (b, b), (c, c), (d_1, d_1), (d_2, d_2), (d_3, d_3), (e, e)}^{(0)}\}(\mathbf{CM}_m)$$

minimised with chisq/nDoF = 45.15 / (53 - 15) = 1.19

|                                                          |  |                         |  |      |      |      |      |       |      |      |      |      |       |       |       |       |       |      |
|----------------------------------------------------------|--|-------------------------|--|------|------|------|------|-------|------|------|------|------|-------|-------|-------|-------|-------|------|
| =====                                                    |  |                         |  |      |      |      |      |       |      |      |      |      |       |       |       |       |       |      |
| JP1-g_eta8:eta1/1^P_1_pole0                              |  | 0.21013 +/- 0.15218     |  | 1.00 | 0.78 | 0.70 | 0.00 | 0.00  | 0.00 | 0.51 | 0.13 | 0.29 | -0.01 | -0.04 | 0.02  | -0.07 | -0.05 | 0.0  |
| JP1-g_h8:eta8/3^S_1_pole0                                |  | 0.82083 +/- 0.61634     |  |      | 1.00 | 0.89 | 0.00 | 0.00  | 0.00 | 0.54 | 0.30 | 0.43 | -0.08 | 0.02  | 0.06  | 0.01  | -0.02 | 0.5  |
| JP1-g_omega8:eta8/3^P_1_pole0                            |  | 0.26842 +/- 0.18636     |  |      |      | 1.00 | 0.00 | 0.00  | 0.00 | 0.52 | 0.30 | 0.39 | -0.31 | 0.03  | 0.05  | 0.02  | 0.01  | 0.3  |
| JP1-g_omega8:omega1/1^P_1_pole0                          |  | -2.9172e-06 +/- 0.36511 |  |      |      |      | 1.00 | -0.00 | 0.00 | 0.00 | 0.00 | 0.00 | 0.00  | 0.00  | -0.00 | 0.00  | -0.00 | 0.0  |
| JP1-g_omega8:omega1/3^P_1_pole0                          |  | 1.3662e-05 +/- 0.22478  |  |      |      |      |      | 1.00  | 0.00 | 0.00 | 0.00 | 0.00 | 0.00  | -0.00 | -0.00 | -0.00 | -0.00 | 0.0  |
| JP1-g_omega8:omega1/5^P_1_pole0                          |  | 5.9145e-07 +/- 0.34995  |  |      |      |      |      |       | 1.00 | 0.00 | 0.00 | 0.00 | -0.00 | 0.00  | 0.00  | 0.00  | -0.00 | 0.0  |
| JP1-g_omega8:omega8/3^P_1_pole0                          |  | 0.24546 +/- 0.25873     |  |      |      |      |      |       |      | 1.00 | 0.18 | 0.25 | 0.02  | -0.19 | 0.03  | -0.16 | 0.08  | 0.2  |
| JP1-gamma_eta8:eta1/1^P_1 eta8:eta1/1^P_1_order0         |  | 1.4399 +/- 0.57292      |  |      |      |      |      |       |      |      | 1.00 | 0.55 | -0.02 | 0.02  | 0.06  | 0.03  | 0.01  | -0.0 |
| JP1-gamma_f8:eta8/3^S_1 f8:eta8/3^S_1_order0             |  | -2.1046 +/- 0.30943     |  |      |      |      |      |       |      |      |      | 1.00 | 0.00  | 0.03  | 0.08  | 0.03  | 0.03  | 0.3  |
| JP1-gamma_omega8:eta8/3^P_1 omega8:eta8/3^P_1_order0     |  | -3.5447 +/- 0.62675     |  |      |      |      |      |       |      |      |      |      | 1.00  | 0.03  | 0.08  | 0.04  | 0.13  | 0.3  |
| JP1-gamma_omega8:omega1/1^P_1 omega8:omega1/1^P_1_order0 |  | 9.2389 +/- 2.4264       |  |      |      |      |      |       |      |      |      |      |       | 1.00  | 0.06  | 0.42  | 0.39  | -0.0 |
| JP1-gamma_omega8:omega1/3^P_1 omega8:omega1/3^P_1_order0 |  | 12.020 +/- 4.9329       |  |      |      |      |      |       |      |      |      |      |       |       | 1.00  | 0.13  | 0.10  | 0.0  |
| JP1-gamma_omega8:omega1/5^P_1 omega8:omega1/5^P_1_order0 |  | 18.831 +/- 3.7943       |  |      |      |      |      |       |      |      |      |      |       |       |       | 1.00  | 0.42  | -0.0 |
| JP1-gamma_omega8:omega8/3^P_1 omega8:omega8/3^P_1_order0 |  | 10.750 +/- 2.981        |  |      |      |      |      |       |      |      |      |      |       |       |       |       | 1.00  | -0.0 |
| JP1-m_pole0                                              |  | 0.46065 +/- 0.0010777   |  |      |      |      |      |       |      |      |      |      |       |       |       |       |       | 1.0  |
| =====                                                    |  |                         |  |      |      |      |      |       |      |      |      |      |       |       |       |       |       |      |

Phase space prescription ::

pole0\_sub

eta8:eta1[-] f8:eta8[+] h8:eta8[+] omega8:eta8[-] omega8:omega1[-] omega8:omega8[-] lower half-plane

sqrt(s)\_pole = (0.46059 +/- 0.0011201)  
+ (1/2)\*(-0.0026091 +/- 0.001397) [ 0.06]

s\_pole = (0.21214 +/- 0.0010319)  
+ i\*(-0.0012017 +/- 0.00064327) [ 0.06]

| eta8:eta1                                                            | f8:eta8                                                              | h8:eta8                                                              | omega8:eta8                                                          | omega8:omega1                                                        | omega8:omega8                                                        |
|----------------------------------------------------------------------|----------------------------------------------------------------------|----------------------------------------------------------------------|----------------------------------------------------------------------|----------------------------------------------------------------------|----------------------------------------------------------------------|
| k_re= 0.1490 +/- 0.0009<br>k_im= -0.0010 +/- 0.0005<br>corr= [ 0.06] | k_re= -0.0033 +/- 0.0018<br>k_im= 0.0389 +/- 0.0028<br>corr= [ 0.03] | k_re= -0.0024 +/- 0.0013<br>k_im= 0.0535 +/- 0.0020<br>corr= [-0.01] | k_re= 0.1401 +/- 0.0009<br>k_im= -0.0011 +/- 0.0006<br>corr= [ 0.06] | k_re= 0.0788 +/- 0.0016<br>k_im= -0.0019 +/- 0.0010<br>corr= [ 0.08] | k_re= 0.0815 +/- 0.0016<br>k_im= -0.0018 +/- 0.0010<br>corr= [ 0.08] |

  

| eta8:eta1/1^P_1                                                     | f8:eta8/3^S_1                                                       | h8:eta8/3^S_1(*)                                                    | omega8:eta8/3^P_1                                                    | omega8:omega1/1^P_1                                                   | omega8:omega1/3^P_1                                                   | omega8:omega1/5^P_1                                                   | omega8:omega8/3^P_1                                                 |
|---------------------------------------------------------------------|---------------------------------------------------------------------|---------------------------------------------------------------------|----------------------------------------------------------------------|-----------------------------------------------------------------------|-----------------------------------------------------------------------|-----------------------------------------------------------------------|---------------------------------------------------------------------|
| g = 0.0270 +/- 0.0120<br>arg(g)/pi= 0.0278 +/- 0.0103               | g = 0.0000 +/- 0.0000<br>arg(g)/pi= 0.4965 +/- 0.0030               | g = 0.3550 +/- 0.0481<br>arg(g)/pi= 0.0035 +/- 0.0030               | g = 0.0320 +/- 0.0103<br>arg(g)/pi= -0.0524 +/- 0.0094               | g = 0.0009 +/- 0.0156<br>arg(g)/pi= -0.4648 +/- 11.1657               | g = 0.0006 +/- 0.0094<br>arg(g)/pi= -0.4713 +/- 11.1692               | g = 0.0009 +/- 0.0137<br>arg(g)/pi= -0.4427 +/- 11.1676               | g = 0.0173 +/- 0.0159<br>arg(g)/pi= 0.0289 +/- 0.0094               |
| g_re= 0.0269 +/- 0.0119<br>g_im= 0.0024 +/- 0.0012<br>corr= [ 0.71] | g_re= 0.0000 +/- 0.0000<br>g_im= 0.0000 +/- 0.0000<br>corr= [-0.59] | g_re= 0.3550 +/- 0.0481<br>g_im= 0.0039 +/- 0.0037<br>corr= [ 0.76] | g_re= 0.0315 +/- 0.0101<br>g_im= -0.0052 +/- 0.0023<br>corr= [-0.93] | g_re= -0.0000 +/- 0.0251<br>g_im= -0.0000 +/- 0.0017<br>corr= [ 1.00] | g_re= -0.0000 +/- 0.0156<br>g_im= -0.0000 +/- 0.0014<br>corr= [ 1.00] | g_re= -0.0000 +/- 0.0233<br>g_im= -0.0000 +/- 0.0035<br>corr= [ 1.00] | g_re= 0.0173 +/- 0.0158<br>g_im= 0.0016 +/- 0.0015<br>corr= [ 0.94] |

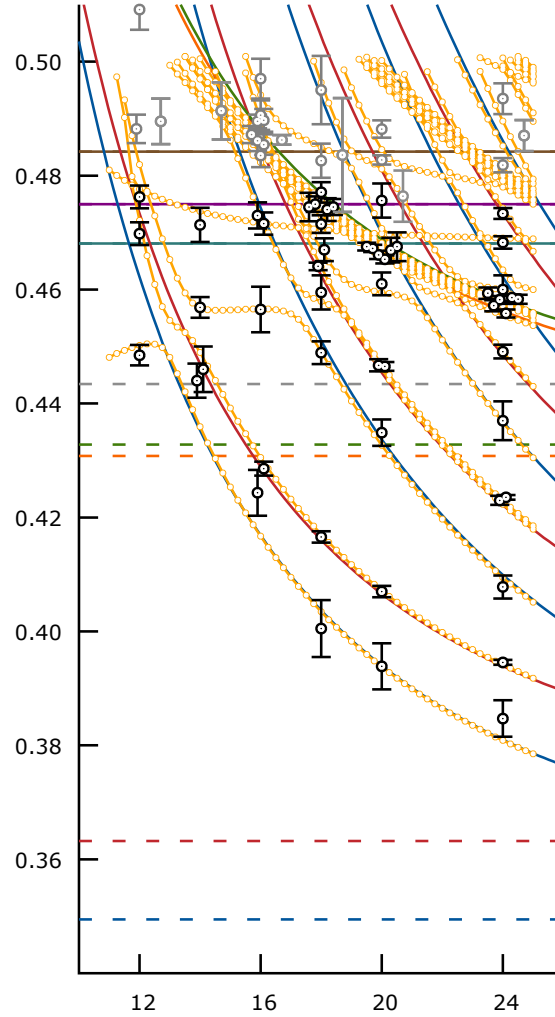

Figure 1.31: Similar to Figure 6 in the manuscript, the finite-volume spectrum, plotted as  $a_t E_{\text{cm}}$ , as a function of spatial extent  $L/a_s$ . Orange points/curves show the spectrum calculated from the amplitude given above (no uncertainties are shown). Black and grey points are the computed lattice energies on each volume, slightly displaced horizontally for clarity (black points correspond to energies used in the fit whereas grey points were not used). Two-meson non-interacting energies are shown as solid coloured curves/lines, two-meson thresholds are shown as dashed/solid horizontal lines, and the  $\eta^s \eta^s \eta^s$  threshold is shown as a dashed grey horizontal line.

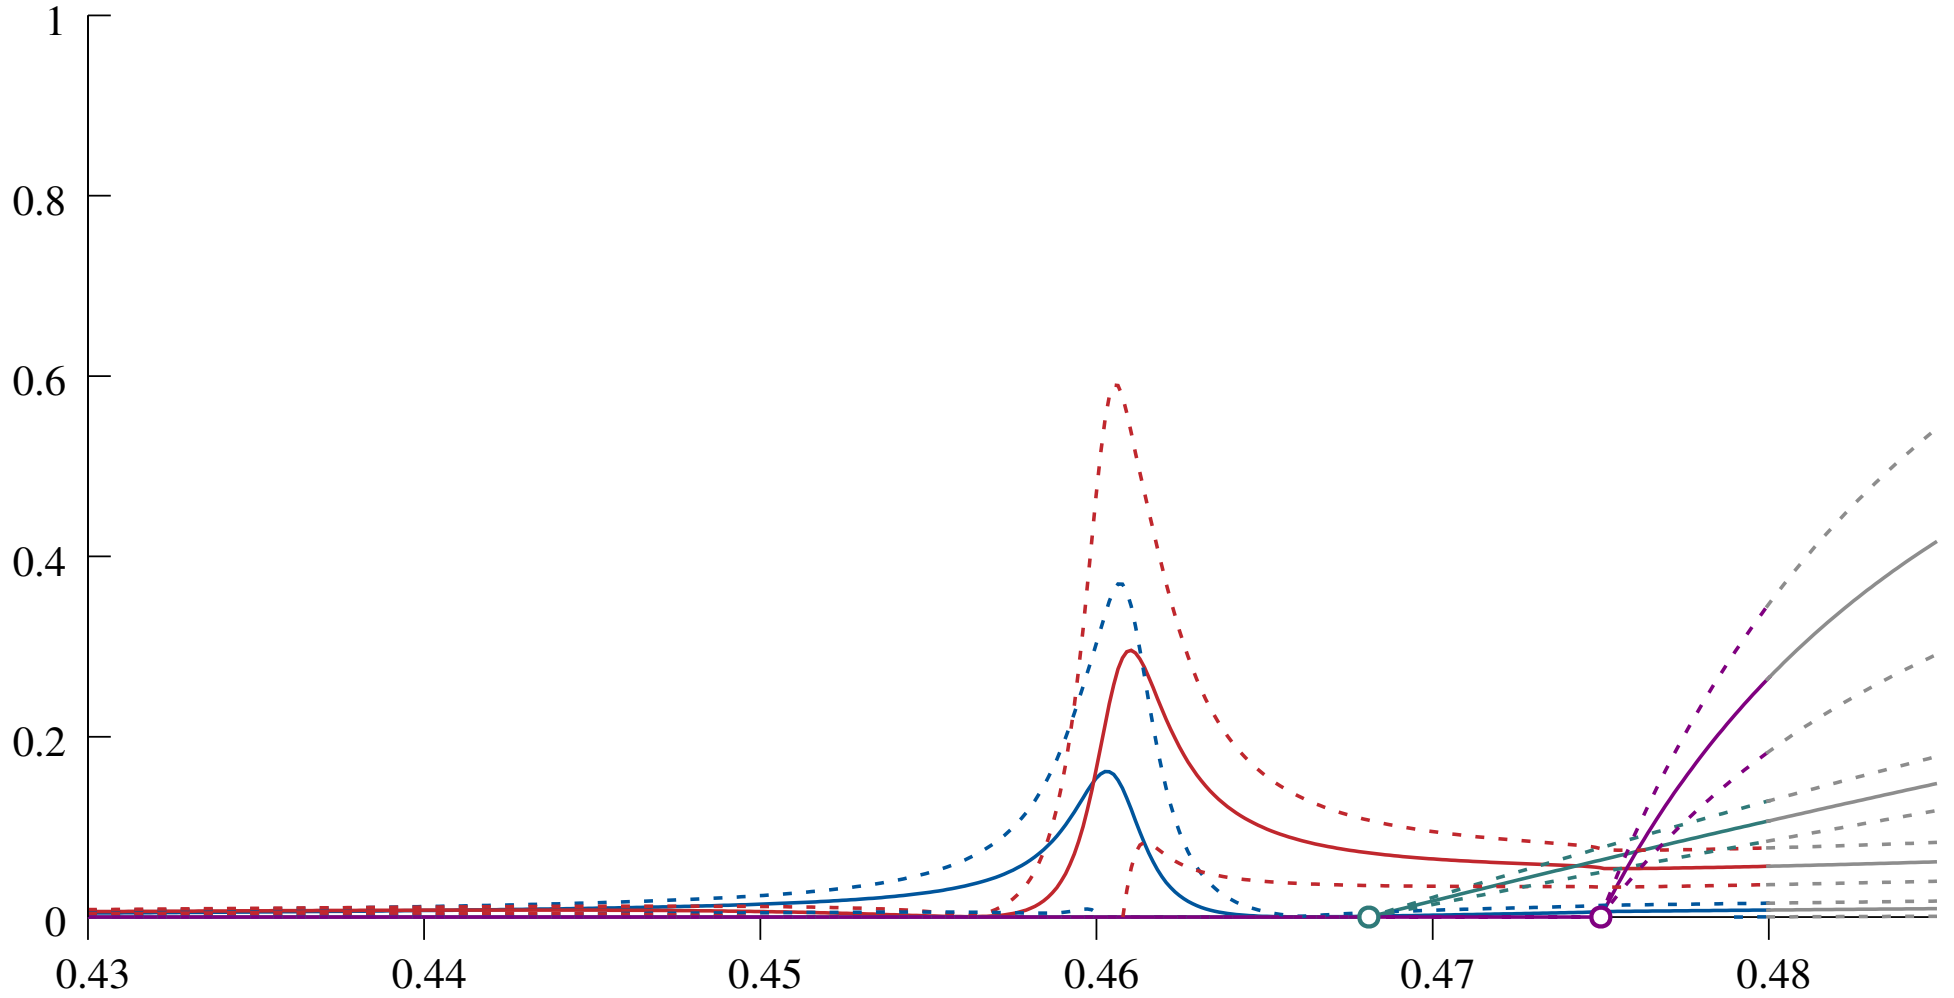

Figure 1.32: Similar to part (a) of Figure 7 in the manuscript,  $\rho_a \rho_b |t_{ab}|^2$  as a function of  $a_t E_{\text{cm}}$  for  $\eta^1 \eta^8 \{^1P_1\} \rightarrow \eta^1 \eta^8 \{^1P_1\}$  (blue),  $\omega^8 \eta^8 \{^3P_1\} \rightarrow \omega^8 \eta^8 \{^3P_1\}$  (red),  $f_1^8 \eta^8 \{^3S_1\} \rightarrow f_1^8 \eta^8 \{^3S_1\}$  (cyan), and  $h_1^8 \eta^8 \{^3S_1\} \rightarrow h_1^8 \eta^8 \{^3S_1\}$  (purple). Dashed lines indicate one standard deviation statistical uncertainties.

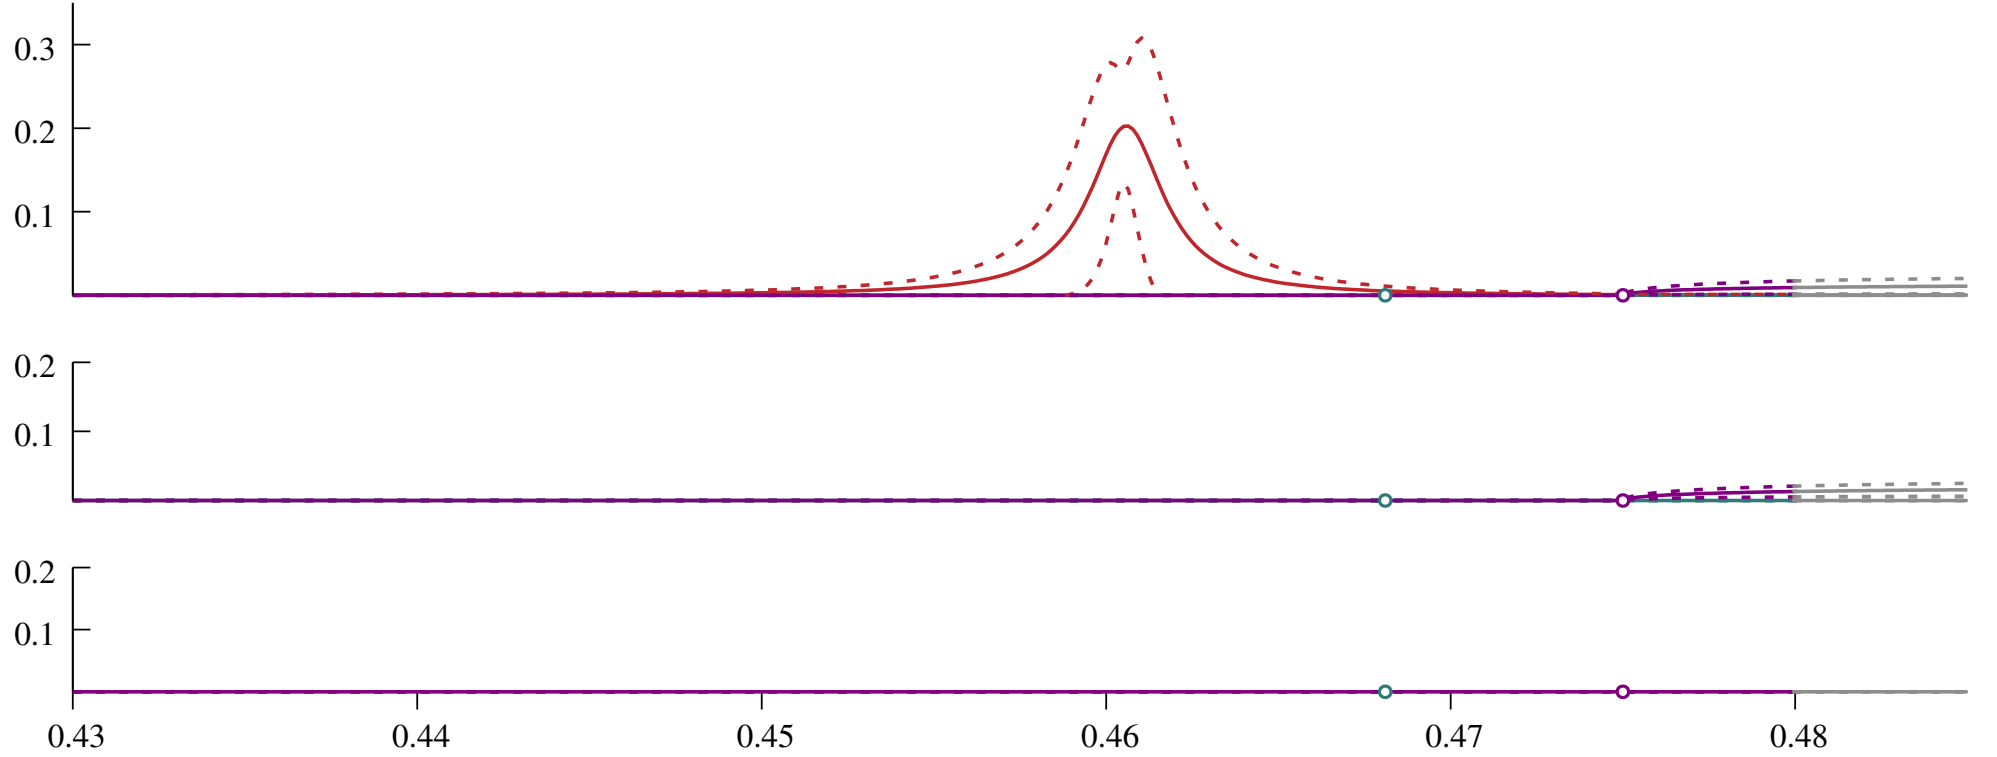

Figure 1.33: Similar to parts (b), (c) and (d) of Figure 7 in the manuscript,  $\rho_a \rho_b |t_{ab}|^2$  as a function of  $a_t E_{\text{cm}}$ . Top:  $\eta^1 \eta^s \{^1P_1\} \rightarrow \omega^s \eta^s \{^3P_1\}$  (red),  $\eta^1 \eta^s \{^1P_1\} \rightarrow f_1^s \eta^s \{^3S_1\}$  (cyan), and  $\eta^1 \eta^s \{^1P_1\} \rightarrow h_1^s \eta^s \{^3S_1\}$  (purple). Middle:  $\omega^s \eta^s \{^3P_1\} \rightarrow f_1^s \eta^s \{^3S_1\}$  (cyan), and  $\omega^s \eta^s \{^3P_1\} \rightarrow h_1^s \eta^s \{^3S_1\}$  (purple). Bottom:  $f_1^s \eta^s \{^3S_1\} \rightarrow h_1^s \eta^s \{^3S_1\}$  (purple). Dashed lines indicate one standard deviation statistical uncertainties.

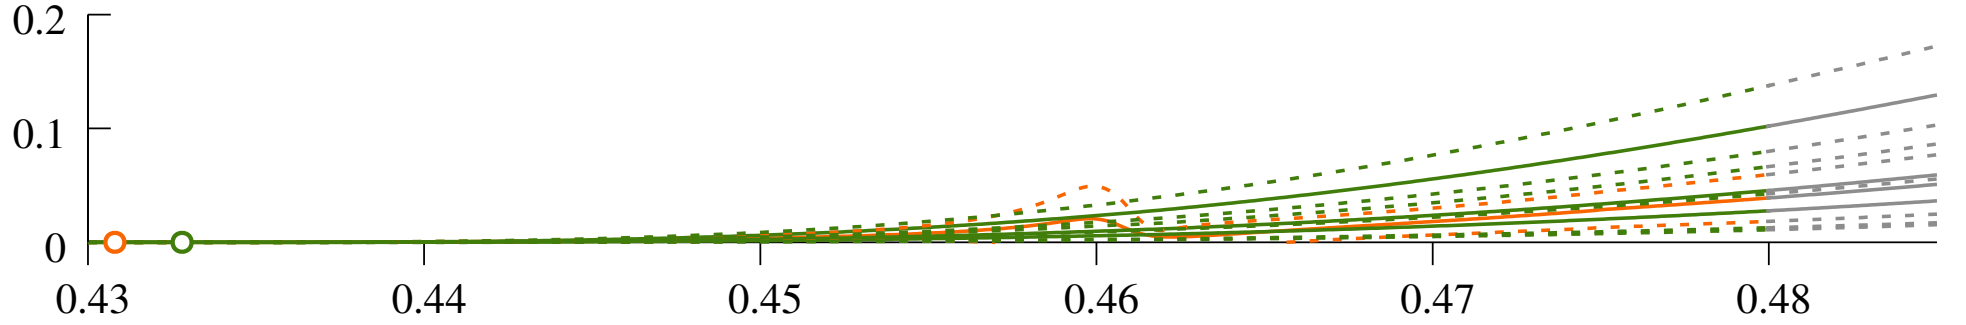

Figure 1.34: Similar to parts (e) and (f) of Figure 7 in the manuscript,  $\rho_a \rho_b |t_{ab}|^2$  as a function of  $a_t E_{cm}$  for  $\omega^s \omega^s \{^3P_1\} \rightarrow \omega^s \omega^s \{^3P_1\}$  (orange),  $\omega^1 \omega^s \{^1P_1, ^3P_1, ^5P_1\} \rightarrow \omega^s \omega^1 \{^1P_1, ^3P_1, ^5P_1\}$  (green). Dashed lines indicate one standard deviation statistical uncertainties.

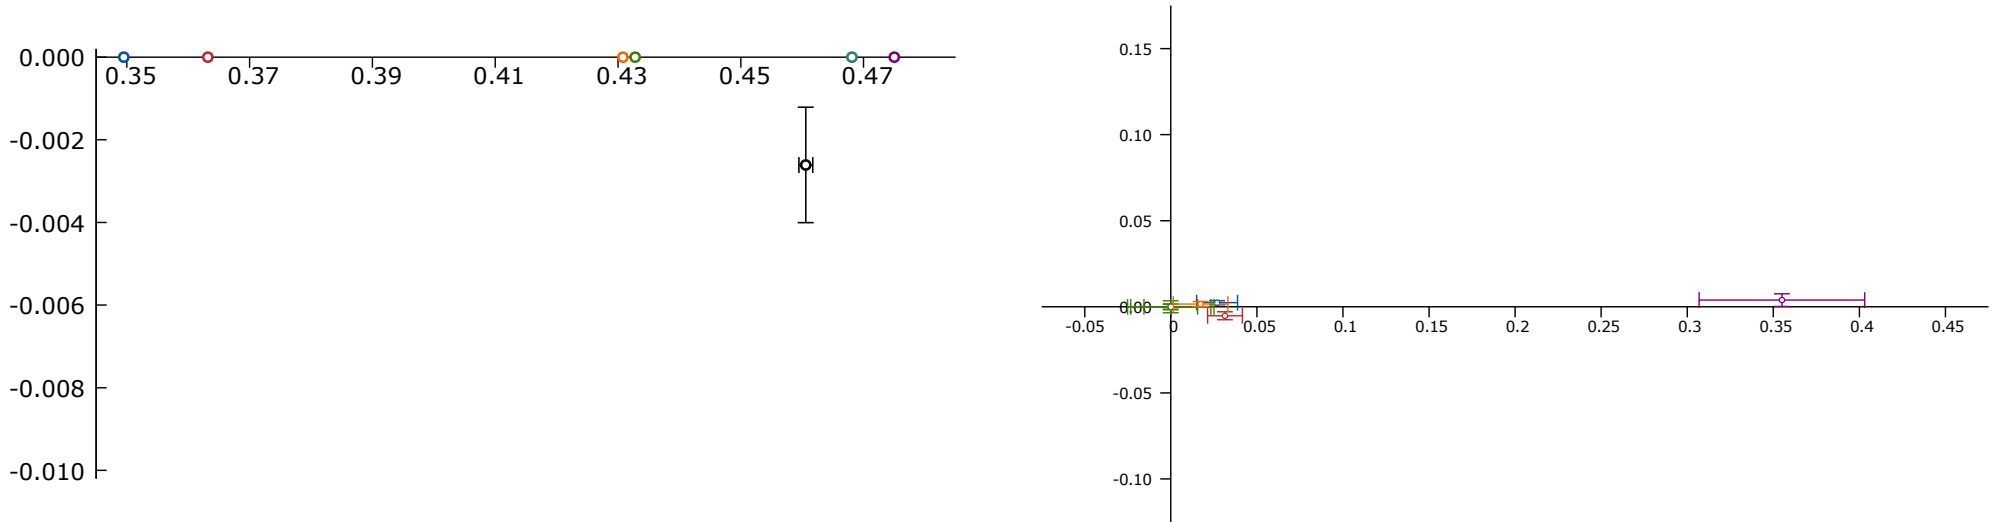

Figure 1.35: Left: Similar to Figure 13 in the manuscript, pole position on the proximal sheet (closest to physical scattering) with  $\text{Re}(a_t \sqrt{s})$  on the horizontal axis and  $2 \text{Im}(a_t \sqrt{s})$  on the vertical axis. Right: Similar to Figure 14 in the manuscript, the corresponding couplings with  $\text{Re}(a_t c)$  on the horizontal axis and  $\text{Im}(a_t c)$  on the vertical axis.

# 1.8 $\{m, g_f^{(0)}, \gamma_{(a,a),(b,b),(c,c),(\partial_1,\partial_1),(\partial_2,\partial_2),(\partial_3,\partial_3),(\epsilon,\epsilon)}^{(0)}\}(\mathbf{CM}_m)$

minimised with chisq/nDoF = 50.49 / (53 - 9) = 1.15

|                                                           |  |                        |  |      |      |      |      |      |      |       |       |       |
|-----------------------------------------------------------|--|------------------------|--|------|------|------|------|------|------|-------|-------|-------|
| =====                                                     |  |                        |  |      |      |      |      |      |      |       |       |       |
| JP1-_g_h8:eta8/3^S_1_pole0                                |  | 0.75982 +/- 0.45548    |  | 1.00 | 0.31 | 0.41 | 0.08 | 0.00 | 0.06 | -0.00 | -0.00 | 0.58  |
| JP1-_gamma_eta8:eta1/1^P_1 eta8:eta1/1^P_1_order0         |  | 1.4529 +/- 0.5324      |  |      | 1.00 | 0.54 | 0.09 | 0.01 | 0.05 | 0.01  | 0.00  | 0.05  |
| JP1-_gamma_f8:eta8/3^S_1 f8:eta8/3^S_1_order0             |  | -2.1059 +/- 0.30469    |  |      |      | 1.00 | 0.09 | 0.03 | 0.07 | 0.03  | 0.03  | 0.16  |
| JP1-_gamma_omega8:eta8/3^P_1 omega8:eta8/3^P_1_order0     |  | -3.0657 +/- 0.51232    |  |      |      |      | 1.00 | 0.10 | 0.10 | 0.10  | 0.18  | 0.02  |
| JP1-_gamma_omega8:omega1/1^P_1 omega8:omega1/1^P_1_order0 |  | 9.5152 +/- 2.356       |  |      |      |      |      | 1.00 | 0.05 | 0.39  | 0.43  | -0.04 |
| JP1-_gamma_omega8:omega1/3^P_1 omega8:omega1/3^P_1_order0 |  | 12.427 +/- 4.9469      |  |      |      |      |      |      | 1.00 | 0.13  | 0.10  | 0.06  |
| JP1-_gamma_omega8:omega1/5^P_1 omega8:omega1/5^P_1_order0 |  | 19.475 +/- 3.7272      |  |      |      |      |      |      |      | 1.00  | 0.45  | -0.05 |
| JP1-_gamma_omega8:omega8/3^P_1 omega8:omega8/3^P_1_order0 |  | 10.607 +/- 2.8873      |  |      |      |      |      |      |      |       | 1.00  | -0.07 |
| JP1-_m_pole0                                              |  | 0.46066 +/- 0.00076931 |  |      |      |      |      |      |      |       |       | 1.00  |
| =====                                                     |  |                        |  |      |      |      |      |      |      |       |       |       |

Phase space prescription ::

pole0\_sub

eta8:eta1[-] f8:eta8[+] h8:eta8[+] omega8:eta8[-] omega8:omega1[-] omega8:omega8[-] lower half-plane

sqrt(s)\_pole = (0.46066 +/- 0.00077007)  
+ (i/2)\*(-1.6974e-13 +/- 7.0092e-11) [ 0.00]

s\_pole = ( 0.2122 +/- 0.00070947)  
+ i\*(-7.8186e-14 +/- 3.2287e-11) [ 0.00]

| eta8:eta1                | f8:eta8                  | h8:eta8                  | omega8:eta8              | omega8:omega1            | omega8:omega8            |
|--------------------------|--------------------------|--------------------------|--------------------------|--------------------------|--------------------------|
| k_re= -0.0692 +/- 2.9491 | k_re= -0.0000 +/- 0.0000 | k_re= -0.0000 +/- 0.0000 | k_re= -0.0650 +/- 2.7730 | k_re= -0.0366 +/- 1.5605 | k_re= -0.0379 +/- 1.6138 |
| k_im= -0.0000 +/- 0.0000 | k_im= 0.0385 +/- 0.0020  | k_im= 0.0534 +/- 0.0014  | k_im= -0.0000 +/- 0.0000 | k_im= -0.0000 +/- 0.0000 | k_im= -0.0000 +/- 0.0000 |
| corr= [ 0.00]            | corr= [ 0.00]            | corr= [ 0.00]            | corr= [ 0.00]            | corr= [ 0.00]            | corr= [ 0.00]            |

  

| eta8:eta1/1^P_1              | f8:eta8/3^S_1                | h8:eta8/3^S_1(*)             | omega8:eta8/3^P_1            | omega8:omega1/1^P_1          | omega8:omega1/3^P_1          | omega8:omega1/5^P_1          | omega8:omega8/3^P_1          |
|------------------------------|------------------------------|------------------------------|------------------------------|------------------------------|------------------------------|------------------------------|------------------------------|
| g = 0.0000 +/- 0.0000        | g = 0.0000 +/- 0.0000        | g = 0.3481 +/- 0.0426        | g = 0.0000 +/- 0.0000        | g = 0.0000 +/- 0.0000        | g = 0.0000 +/- 0.0000        | g = 0.0000 +/- 0.0000        | g = 0.0000 +/- 0.0000        |
| arg(g)/pi= 0.5000 +/- 0.0000 | arg(g)/pi= 0.5000 +/- 0.0000 | arg(g)/pi= 0.0000 +/- 0.0000 | arg(g)/pi= 0.5000 +/- 0.0000 | arg(g)/pi= 0.5000 +/- 0.0000 | arg(g)/pi= 0.5000 +/- 0.0000 | arg(g)/pi= 0.5000 +/- 0.0000 | arg(g)/pi= 0.5000 +/- 0.0000 |
| g_re= 0.0000 +/- 0.0000      | g_re= 0.0000 +/- 0.0000      | g_re= 0.3481 +/- 0.0426      | g_re= 0.0000 +/- 0.0000      | g_re= 0.0000 +/- 0.0000      | g_re= 0.0000 +/- 0.0000      | g_re= 0.0000 +/- 0.0000      | g_re= 0.0000 +/- 0.0000      |
| g_im= 0.0000 +/- 0.0000      | g_im= 0.0000 +/- 0.0000      | g_im= 0.0000 +/- 0.0000      | g_im= 0.0000 +/- 0.0000      | g_im= 0.0000 +/- 0.0000      | g_im= 0.0000 +/- 0.0000      | g_im= 0.0000 +/- 0.0000      | g_im= 0.0000 +/- 0.0000      |
| corr= [ 0.00]                | corr= [ 0.00]                | corr= [-1.00]                | corr= [ 0.00]                | corr= [ 0.00]                | corr= [ 0.00]                | corr= [ 0.00]                | corr= [ 0.00]                |

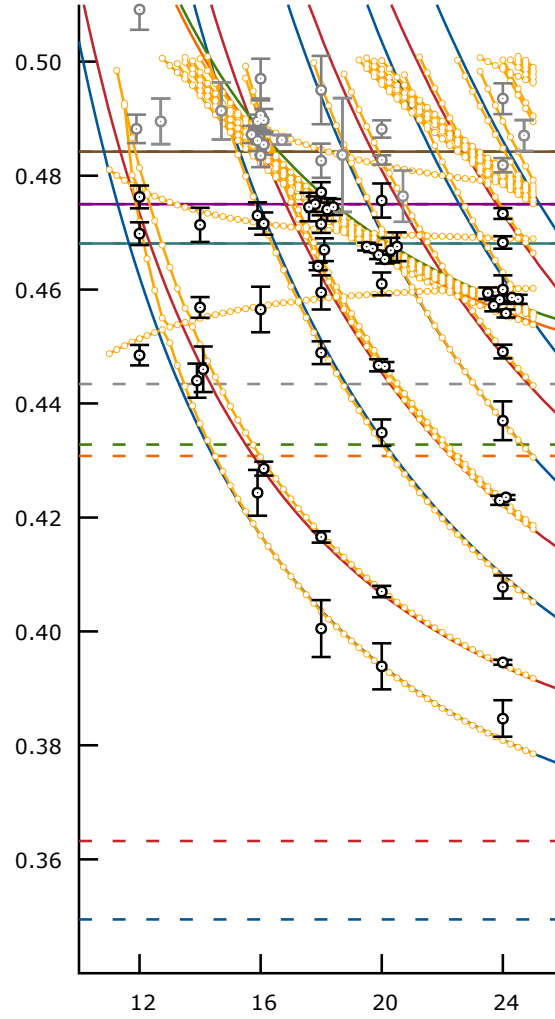

Figure 1.36: Similar to Figure 6 in the manuscript, the finite-volume spectrum, plotted as  $a_t E_{\text{cm}}$ , as a function of spatial extent  $L/a_s$ . Orange points/curves show the spectrum calculated from the amplitude given above (no uncertainties are shown). Black and grey points are the computed lattice energies on each volume, slightly displaced horizontally for clarity (black points correspond to energies used in the fit whereas grey points were not used). Two-meson non-interacting energies are shown as solid coloured curves/lines, two-meson thresholds are shown as dashed/solid horizontal lines, and the  $\eta^s \eta^s \eta^s$  threshold is shown as a dashed grey horizontal line.

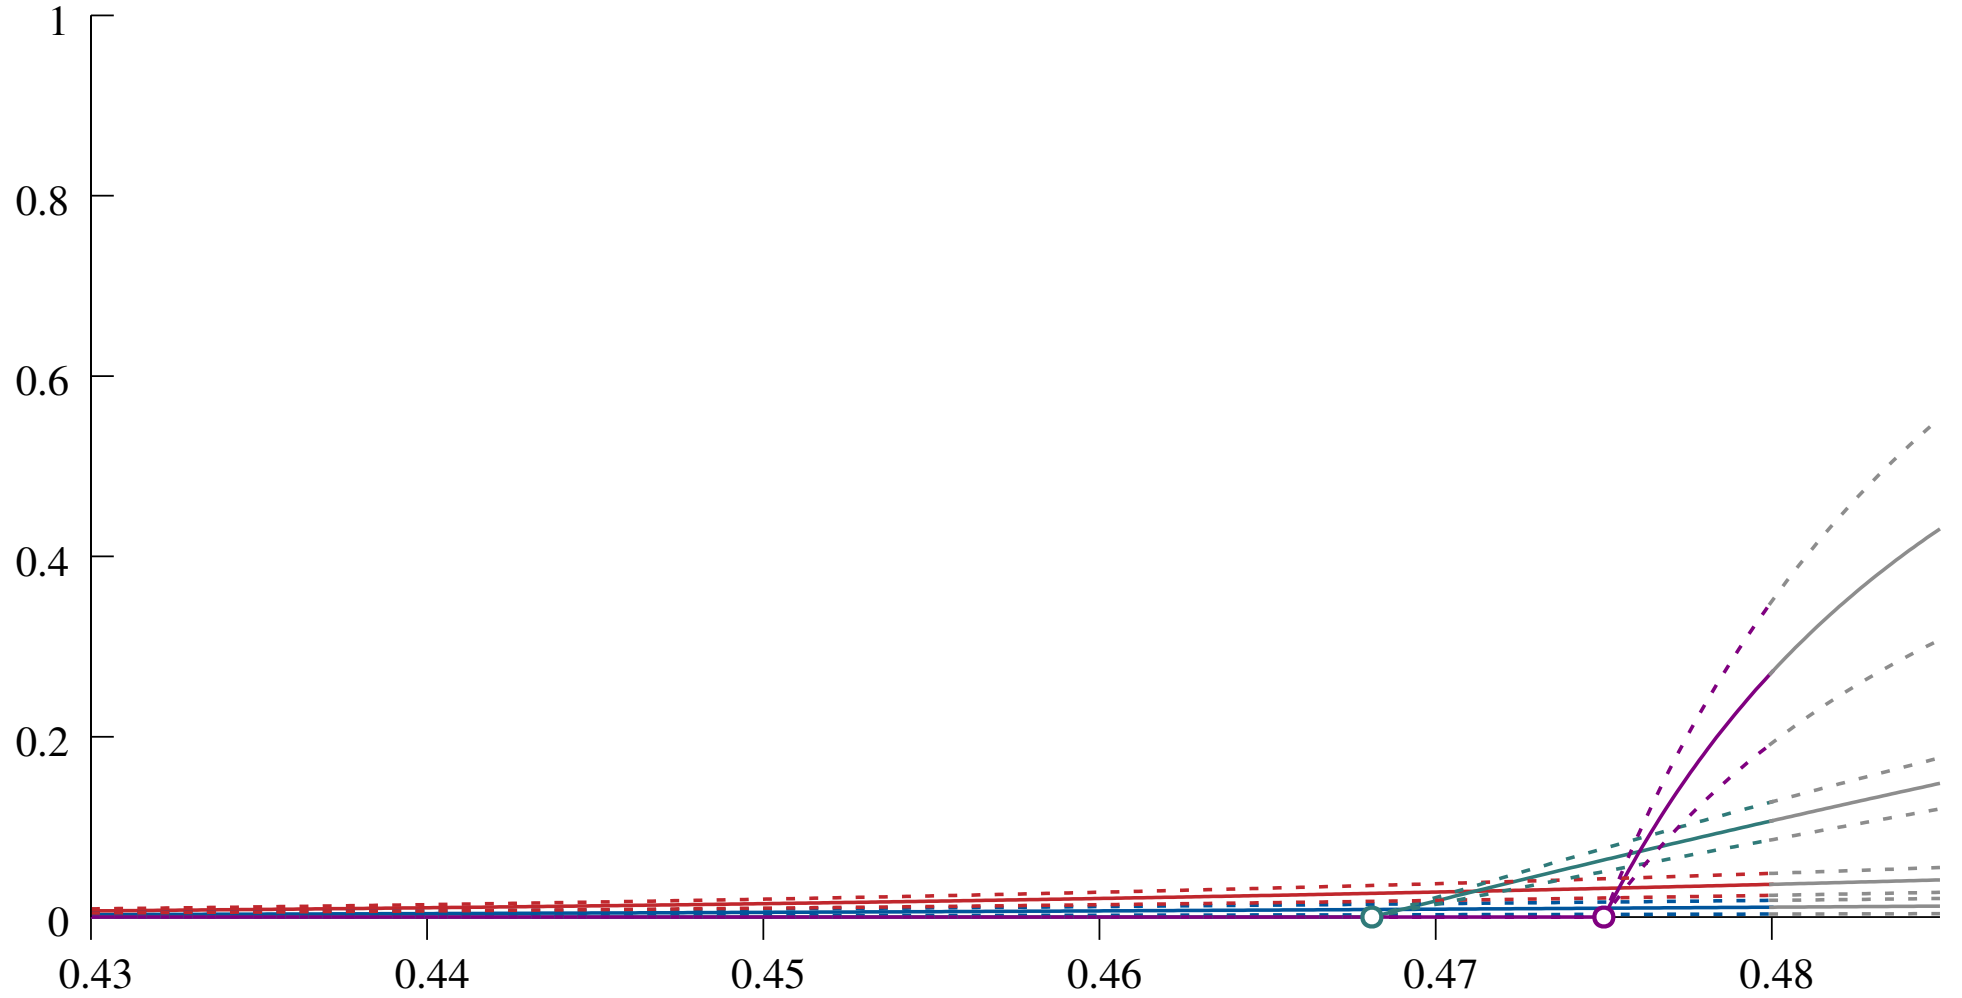

Figure 1.37: Similar to part (a) of Figure 7 in the manuscript,  $\rho_a \rho_b |t_{ab}|^2$  as a function of  $a_t E_{cm}$  for  $\eta^1 \eta^s \{^1P_1\} \rightarrow \eta^1 \eta^s \{^1P_1\}$  (blue),  $\omega^s \eta^s \{^3P_1\} \rightarrow \omega^s \eta^s \{^3P_1\}$  (red),  $f_1^s \eta^s \{^3S_1\} \rightarrow f_1^s \eta^s \{^3S_1\}$  (cyan), and  $h_1^s \eta^s \{^3S_1\} \rightarrow h_1^s \eta^s \{^3S_1\}$  (purple). Dashed lines indicate one standard deviation statistical uncertainties.

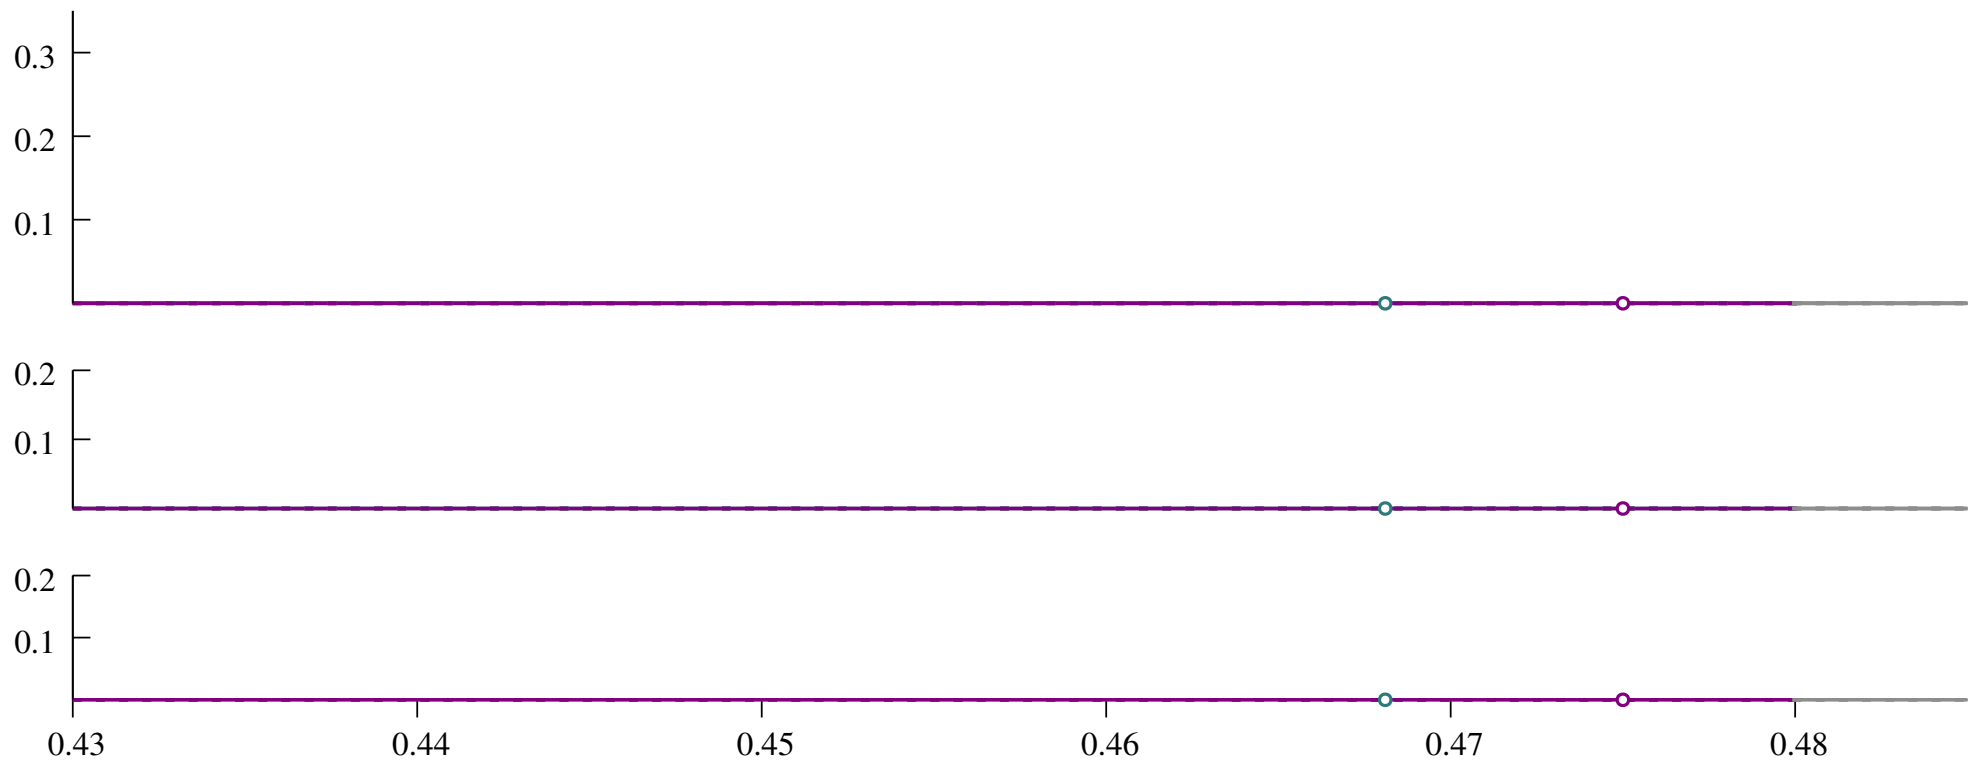

Figure 1.38: Similar to parts (b), (c) and (d) of Figure 7 in the manuscript,  $\rho_a \rho_b |t_{ab}|^2$  as a function of  $a_t E_{\text{cm}}$ . Top:  $\eta^1 \eta^s \{^1P_1\} \rightarrow \omega^s \eta^s \{^3P_1\}$  (red),  $\eta^1 \eta^s \{^1P_1\} \rightarrow f_1^s \eta^s \{^3S_1\}$  (cyan), and  $\eta^1 \eta^s \{^1P_1\} \rightarrow h_1^s \eta^s \{^3S_1\}$  (purple). Middle:  $\omega^s \eta^s \{^3P_1\} \rightarrow f_1^s \eta^s \{^3S_1\}$  (cyan), and  $\omega^s \eta^s \{^3P_1\} \rightarrow h_1^s \eta^s \{^3S_1\}$  (purple). Bottom:  $f_1^s \eta^s \{^3S_1\} \rightarrow h_1^s \eta^s \{^3S_1\}$  (purple). Dashed lines indicate one standard deviation statistical uncertainties.

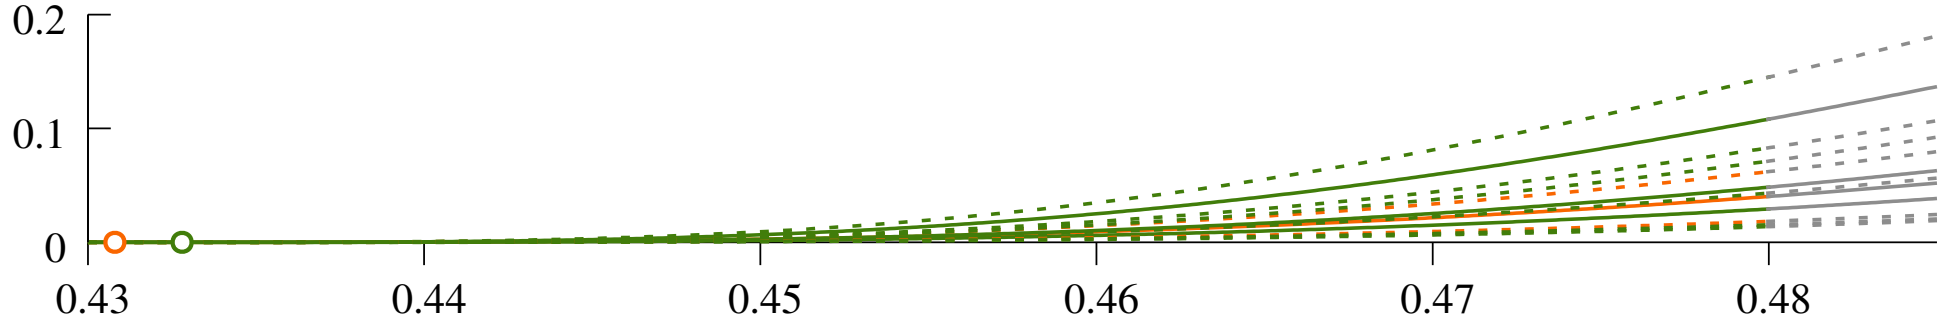

Figure 1.39: Similar to parts (e) and (f) of Figure 7 in the manuscript,  $\rho_a \rho_b |t_{ab}|^2$  as a function of  $a_t E_{cm}$  for  $\omega^s \omega^s \{^3P_1\} \rightarrow \omega^s \omega^s \{^3P_1\}$  (orange),  $\omega^1 \omega^s \{^1P_1, ^3P_1, ^5P_1\} \rightarrow \omega^s \omega^1 \{^1P_1, ^3P_1, ^5P_1\}$  (green). Dashed lines indicate one standard deviation statistical uncertainties.

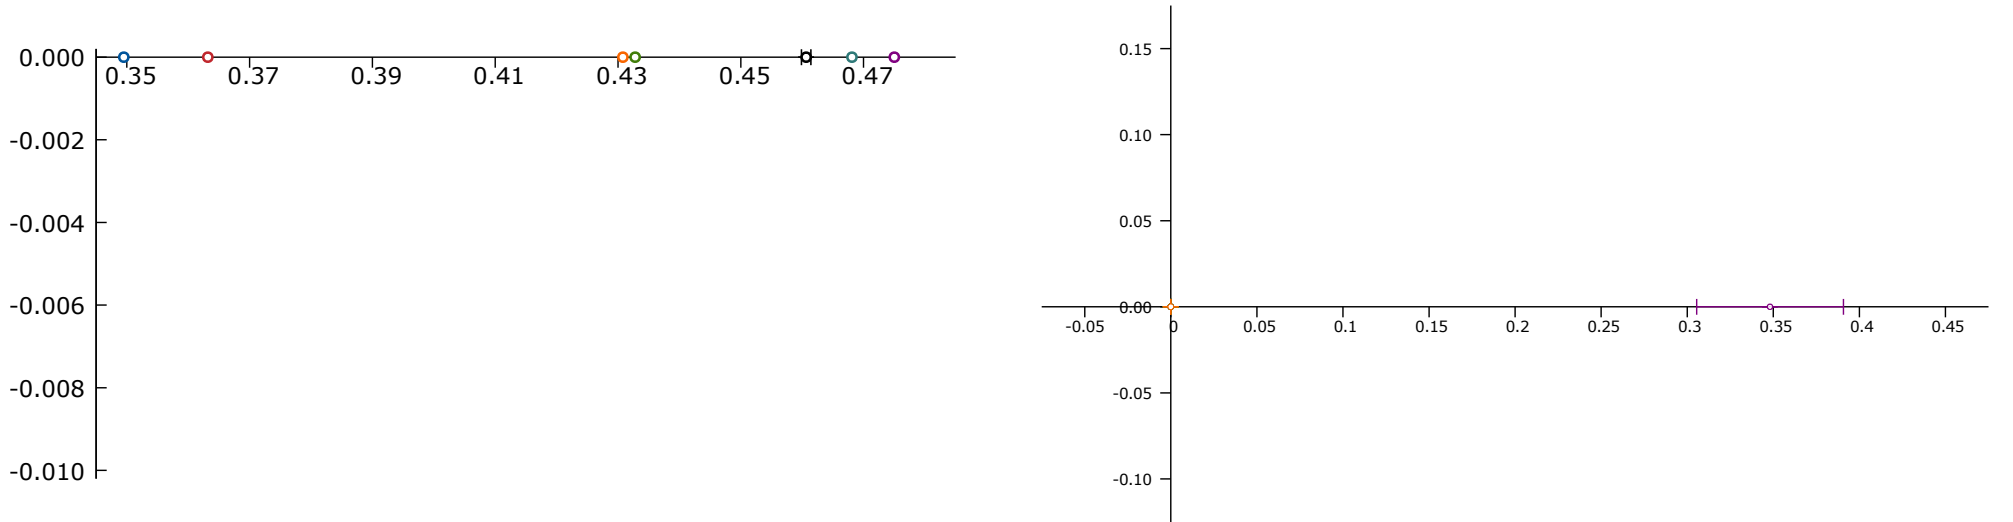

Figure 1.40: Left: Similar to Figure 13 in the manuscript, pole position on the proximal sheet (closest to physical scattering) with  $\text{Re}(a_t \sqrt{s})$  on the horizontal axis and  $2 \text{Im}(a_t \sqrt{s})$  on the vertical axis. Right: Similar to Figure 14 in the manuscript, the corresponding couplings with  $\text{Re}(a_t c)$  on the horizontal axis and  $\text{Im}(a_t c)$  on the vertical axis.

# 1.9 $\{m, g_{a,b,f}^{(0)}, \gamma_{(a,a),(b,b),(c,c),(\partial_1,\partial_1),(\partial_2,\partial_2),(\partial_3,\partial_3),(e,e)}\}(\mathbf{CM}_m)$

minimised with chisq/nDoF = 45.49 / (53 - 11) = 1.08

|                                                          |  |                       |  |      |      |      |      |       |       |       |      |                  |
|----------------------------------------------------------|--|-----------------------|--|------|------|------|------|-------|-------|-------|------|------------------|
| =====                                                    |  |                       |  |      |      |      |      |       |       |       |      |                  |
| JP1-g_eta8:eta1/1^P_1_pole0                              |  | 0.20802 +/- 0.16029   |  | 1.00 | 0.78 | 0.70 | 0.13 | 0.29  | -0.02 | -0.03 | 0.02 | -0.06 -0.06 0.64 |
| JP1-g_h8:eta8/3^S_1_pole0                                |  | 0.85392 +/- 0.66675   |  |      | 1.00 | 0.90 | 0.31 | 0.43  | -0.08 | -0.00 | 0.06 | -0.00 -0.01 0.51 |
| JP1-g_omega8:eta8/3^P_1_pole0                            |  | 0.27412 +/- 0.19994   |  |      | 1.00 | 0.31 | 0.39 | -0.30 | 0.02  | 0.05  | 0.01 | 0.01 0.39        |
| JP1-gamma_eta8:eta1/1^P_1 eta8:eta1/1^P_1_order0         |  | 1.4411 +/- 0.57094    |  |      |      | 1.00 | 0.55 | -0.02 | 0.02  | 0.06  | 0.03 | 0.02 -0.02       |
| JP1-gamma_f8:eta8/3^S_1 f8:eta8/3^S_1_order0             |  | -2.1023 +/- 0.30786   |  |      |      |      | 1.00 | 0.00  | 0.03  | 0.08  | 0.03 | 0.04 0.14        |
| JP1-gamma_omega8:eta8/3^P_1 omega8:eta8/3^P_1_order0     |  | -3.5756 +/- 0.62223   |  |      |      |      |      | 1.00  | 0.05  | 0.08  | 0.06 | 0.13 0.11        |
| JP1-gamma_omega8:omega1/1^P_1 omega8:omega1/1^P_1_order0 |  | 9.5810 +/- 2.3636     |  |      |      |      |      |       | 1.00  | 0.06  | 0.39 | 0.43 -0.06       |
| JP1-gamma_omega8:omega1/3^P_1 omega8:omega1/3^P_1_order0 |  | 12.062 +/- 4.9317     |  |      |      |      |      |       |       | 1.00  | 0.13 | 0.10 0.05        |
| JP1-gamma_omega8:omega1/5^P_1 omega8:omega1/5^P_1_order0 |  | 19.269 +/- 3.7386     |  |      |      |      |      |       |       |       | 1.00 | 0.46 -0.09       |
| JP1-gamma_omega8:omega8/3^P_1 omega8:omega8/3^P_1_order0 |  | 10.560 +/- 2.8998     |  |      |      |      |      |       |       |       |      | 1.00 -0.11       |
| JP1-m_pole0                                              |  | 0.46076 +/- 0.0010259 |  |      |      |      |      |       |       |       |      | 1.00             |
| =====                                                    |  |                       |  |      |      |      |      |       |       |       |      |                  |

Phase space prescription ::

pole0\_sub

eta8:eta1[-] f8:eta8[+] h8:eta8[+] omega8:eta8[-] omega8:omega1[-] omega8:omega8[-] lower half-plane

sqrt(s)\_pole = (0.46069 +/- 0.0010122)  
+ (i/2)\*(-0.0022542 +/- 0.001239) [ 0.01]

s\_pole = (0.21223 +/- 0.00093267)  
+ i\*(-0.0010385 +/- 0.00057077) [ 0.00]

| eta8:eta1                | f8:eta8                  | h8:eta8                  | omega8:eta8              | omega8:omega1            | omega8:omega8            |
|--------------------------|--------------------------|--------------------------|--------------------------|--------------------------|--------------------------|
| k_re= 0.1491 +/- 0.0008  | k_re= -0.0029 +/- 0.0016 | k_re= -0.0020 +/- 0.0011 | k_re= 0.1402 +/- 0.0008  | k_re= 0.0789 +/- 0.0015  | k_re= 0.0816 +/- 0.0014  |
| k_im= -0.0009 +/- 0.0005 | k_im= 0.0386 +/- 0.0026  | k_im= 0.0533 +/- 0.0018  | k_im= -0.0009 +/- 0.0005 | k_im= -0.0016 +/- 0.0009 | k_im= -0.0016 +/- 0.0009 |
| corr= [ 0.01]            | corr= [ 0.07]            | corr= [ 0.04]            | corr= [ 0.01]            | corr= [ 0.03]            | corr= [ 0.02]            |

  

| eta8:eta1/1^P_1              | f8:eta8/3^S_1                | h8:eta8/3^S_1(*)             | omega8:eta8/3^P_1             | omega8:omega1/1^P_1          | omega8:omega1/3^P_1          | omega8:omega1/5^P_1          | omega8:omega8/3^P_1          |
|------------------------------|------------------------------|------------------------------|-------------------------------|------------------------------|------------------------------|------------------------------|------------------------------|
| g = 0.0258 +/- 0.0122        | g = 0.0000 +/- 0.0000        | g = 0.3564 +/- 0.0466        | g = 0.0315 +/- 0.0104         | g = 0.0000 +/- 0.0000        | g = 0.0000 +/- 0.0000        | g = 0.0000 +/- 0.0000        | g = 0.0000 +/- 0.0000        |
| arg(g)/pi= 0.0283 +/- 0.0112 | arg(g)/pi= 0.4963 +/- 0.0027 | arg(g)/pi= 0.0037 +/- 0.0027 | arg(g)/pi= -0.0524 +/- 0.0091 | arg(g)/pi= 0.4963 +/- 0.0027 | arg(g)/pi= 0.4963 +/- 0.0027 | arg(g)/pi= 0.4963 +/- 0.0027 | arg(g)/pi= 0.4963 +/- 0.0027 |
| g_re= 0.0257 +/- 0.0122      | g_re= 0.0000 +/- 0.0000      | g_re= 0.3564 +/- 0.0466      | g_re= 0.0311 +/- 0.0102       | g_re= 0.0000 +/- 0.0000      | g_re= 0.0000 +/- 0.0000      | g_re= 0.0000 +/- 0.0000      | g_re= 0.0000 +/- 0.0000      |
| g_im= 0.0023 +/- 0.0013      | g_im= 0.0000 +/- 0.0000      | g_im= 0.0041 +/- 0.0034      | g_im= -0.0052 +/- 0.0022      | g_im= 0.0000 +/- 0.0000      | g_im= 0.0000 +/- 0.0000      | g_im= 0.0000 +/- 0.0000      | g_im= 0.0000 +/- 0.0000      |
| corr= [ 0.72]                | corr= [-0.48]                | corr= [ 0.70]                | corr= [-0.93]                 | corr= [-0.48]                | corr= [-0.48]                | corr= [-0.48]                | corr= [-0.48]                |

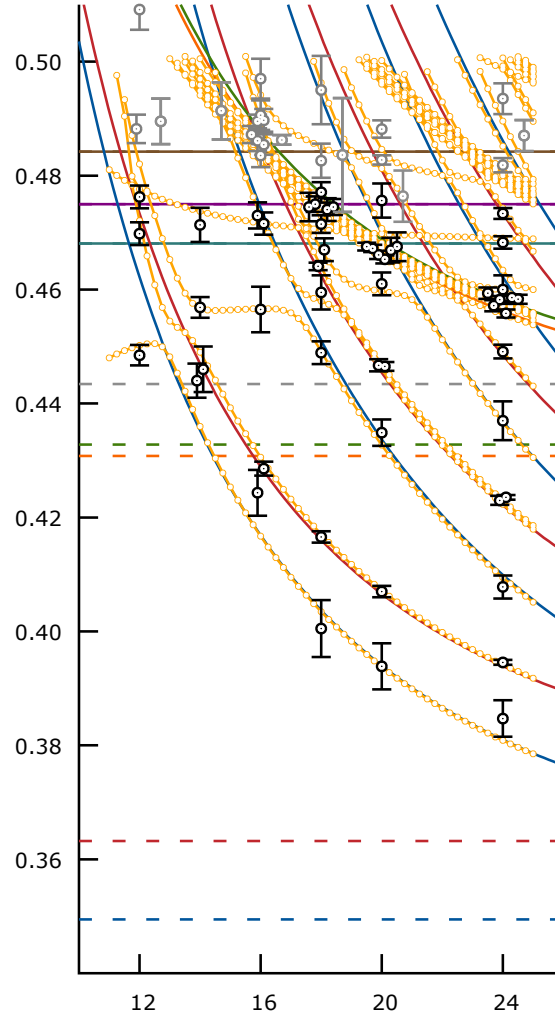

Figure 1.41: Similar to Figure 6 in the manuscript, the finite-volume spectrum, plotted as  $a_t E_{\text{cm}}$ , as a function of spatial extent  $L/a_s$ . Orange points/curves show the spectrum calculated from the amplitude given above (no uncertainties are shown). Black and grey points are the computed lattice energies on each volume, slightly displaced horizontally for clarity (black points correspond to energies used in the fit whereas grey points were not used). Two-meson non-interacting energies are shown as solid coloured curves/lines, two-meson thresholds are shown as dashed/solid horizontal lines, and the  $\eta^s \eta^s \eta^s$  threshold is shown as a dashed grey horizontal line.

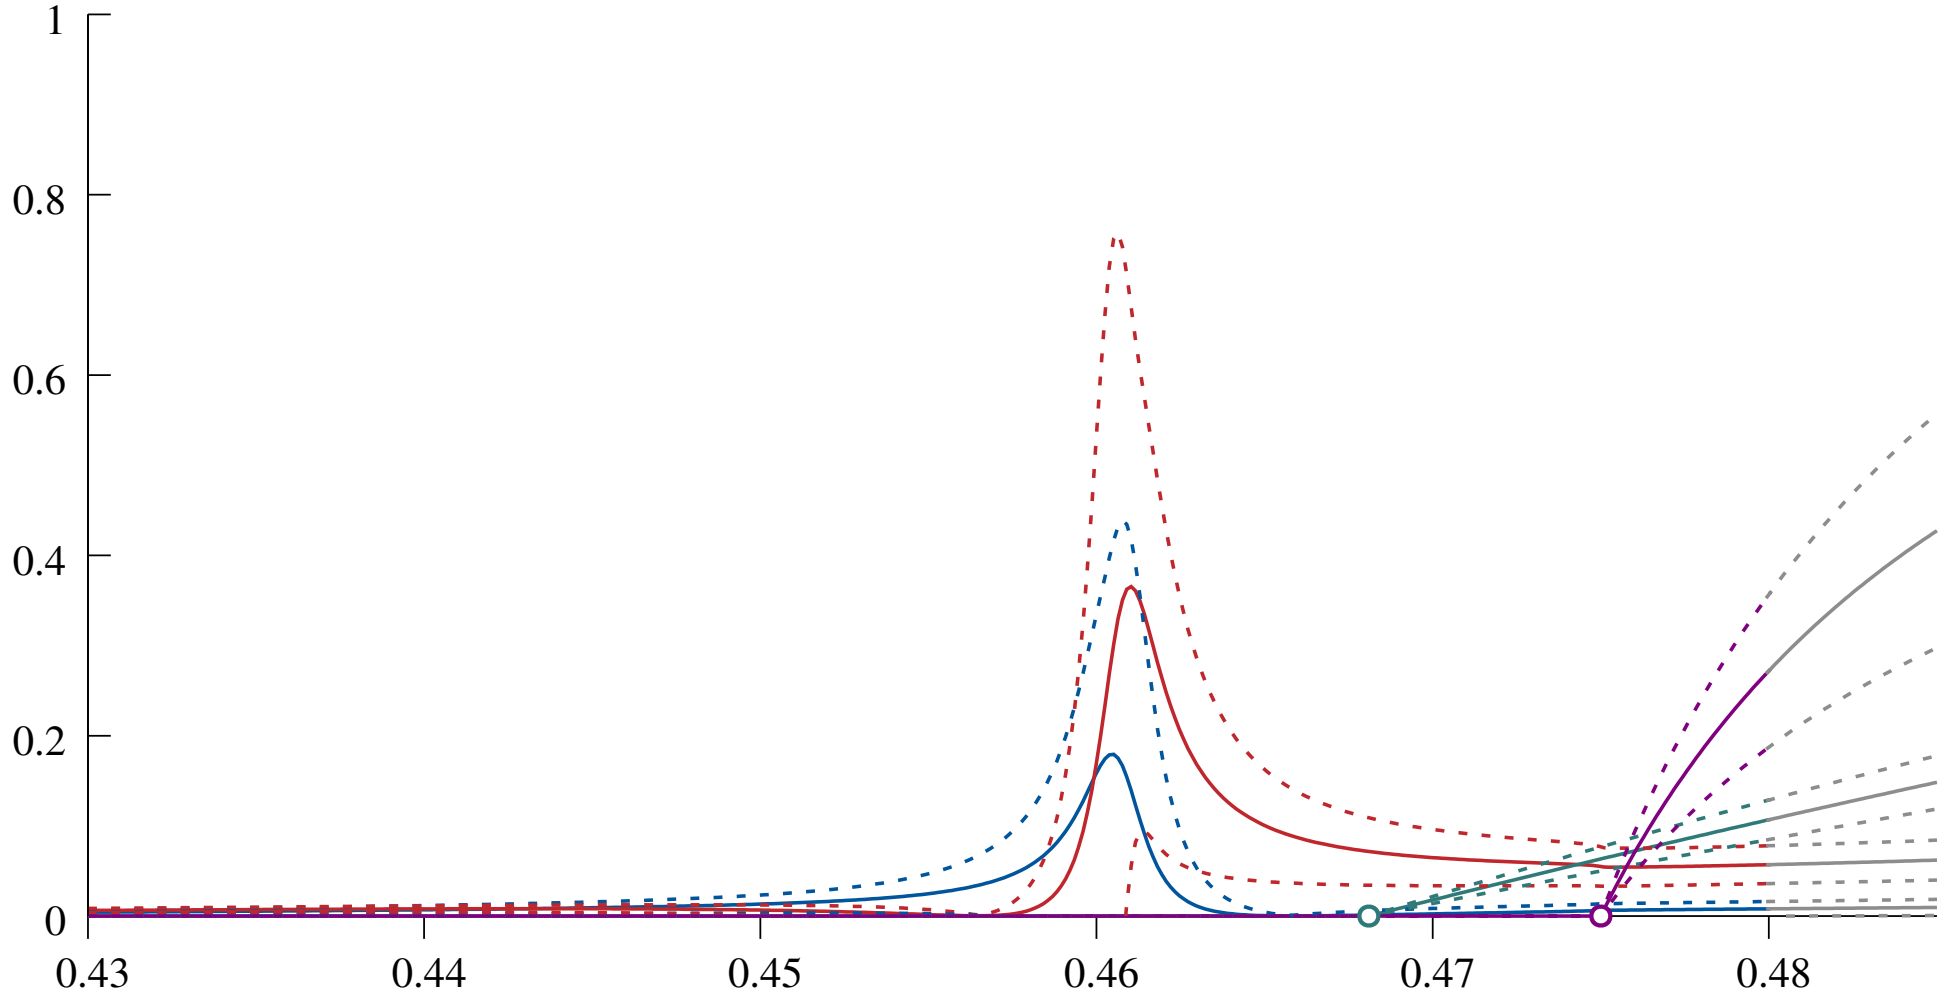

Figure 1.42: Similar to part (a) of Figure 7 in the manuscript,  $\rho_a \rho_b |t_{ab}|^2$  as a function of  $a_t E_{\text{cm}}$  for  $\eta^1 \eta^s \{^1P_1\} \rightarrow \eta^1 \eta^s \{^1P_1\}$  (blue),  $\omega^s \eta^s \{^3P_1\} \rightarrow \omega^s \eta^s \{^3P_1\}$  (red),  $f_1^s \eta^s \{^3S_1\} \rightarrow f_1^s \eta^s \{^3S_1\}$  (cyan), and  $h_1^s \eta^s \{^3S_1\} \rightarrow h_1^s \eta^s \{^3S_1\}$  (purple). Dashed lines indicate one standard deviation statistical uncertainties.

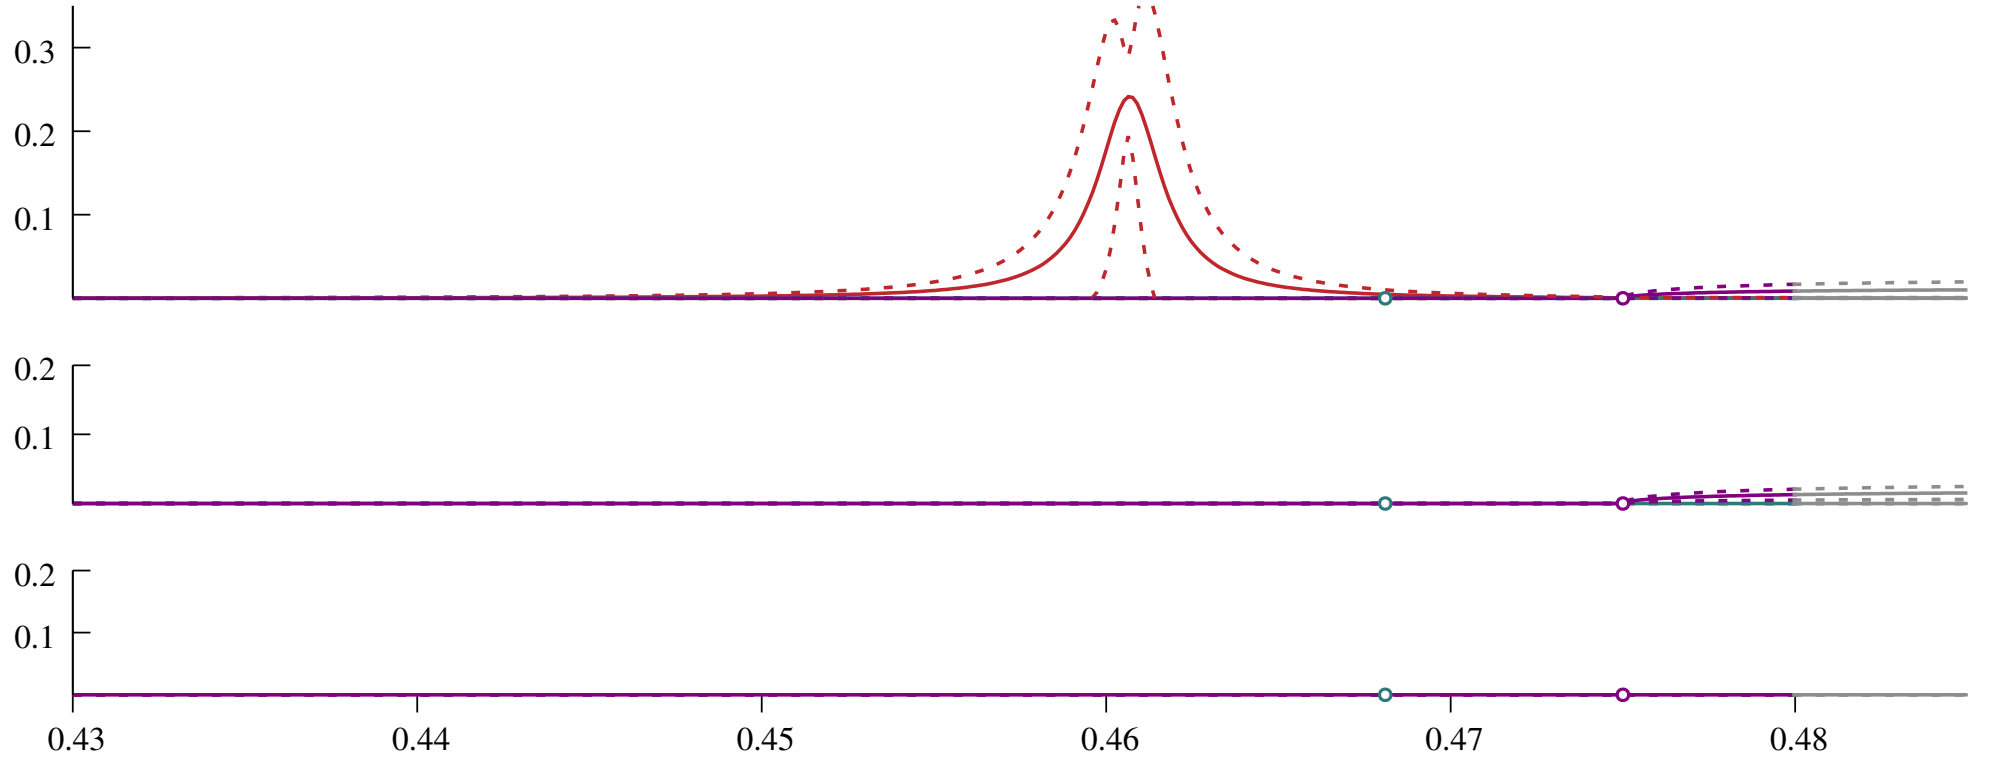

Figure 1.43: Similar to parts (b), (c) and (d) of Figure 7 in the manuscript,  $\rho_a \rho_b |t_{ab}|^2$  as a function of  $a_t E_{\text{cm}}$ . Top:  $\eta^1 \eta^s \{^1P_1\} \rightarrow \omega^s \eta^s \{^3P_1\}$  (red),  $\eta^1 \eta^s \{^1P_1\} \rightarrow f_1^s \eta^s \{^3S_1\}$  (cyan), and  $\eta^1 \eta^s \{^1P_1\} \rightarrow h_1^s \eta^s \{^3S_1\}$  (purple). Middle:  $\omega^s \eta^s \{^3P_1\} \rightarrow f_1^s \eta^s \{^3S_1\}$  (cyan), and  $\omega^s \eta^s \{^3P_1\} \rightarrow h_1^s \eta^s \{^3S_1\}$  (purple). Bottom:  $f_1^s \eta^s \{^3S_1\} \rightarrow h_1^s \eta^s \{^3S_1\}$  (purple). Dashed lines indicate one standard deviation statistical uncertainties.

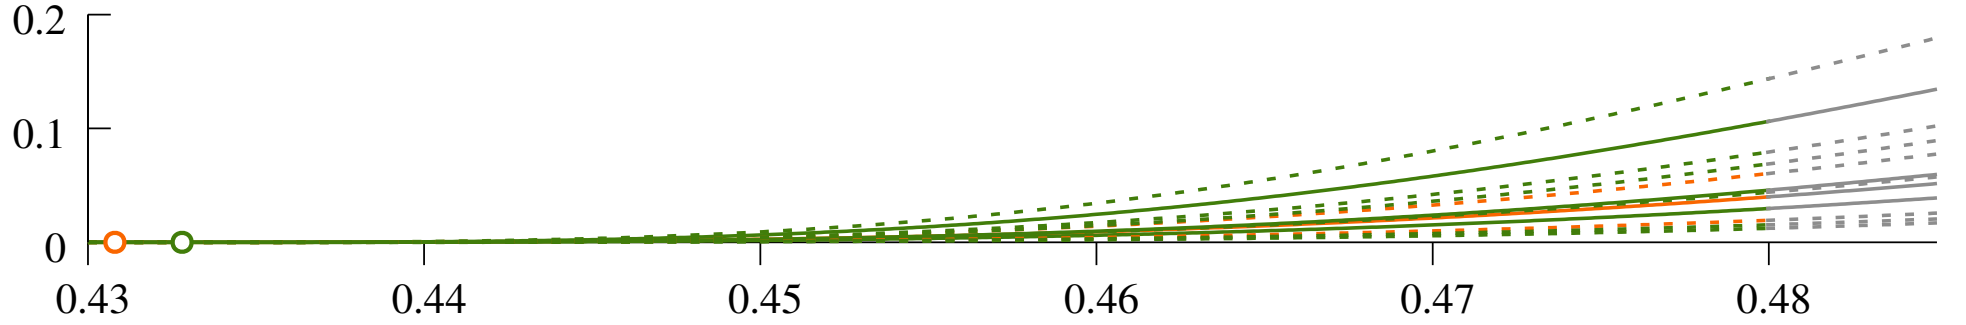

Figure 1.44: Similar to parts (e) and (f) of Figure 7 in the manuscript,  $\rho_a \rho_b |t_{ab}|^2$  as a function of  $a_t E_{cm}$  for  $\omega^s \omega^s \{^3P_1\} \rightarrow \omega^s \omega^s \{^3P_1\}$  (orange),  $\omega^1 \omega^s \{^1P_1, ^3P_1, ^5P_1\} \rightarrow \omega^s \omega^1 \{^1P_1, ^3P_1, ^5P_1\}$  (green). Dashed lines indicate one standard deviation statistical uncertainties.

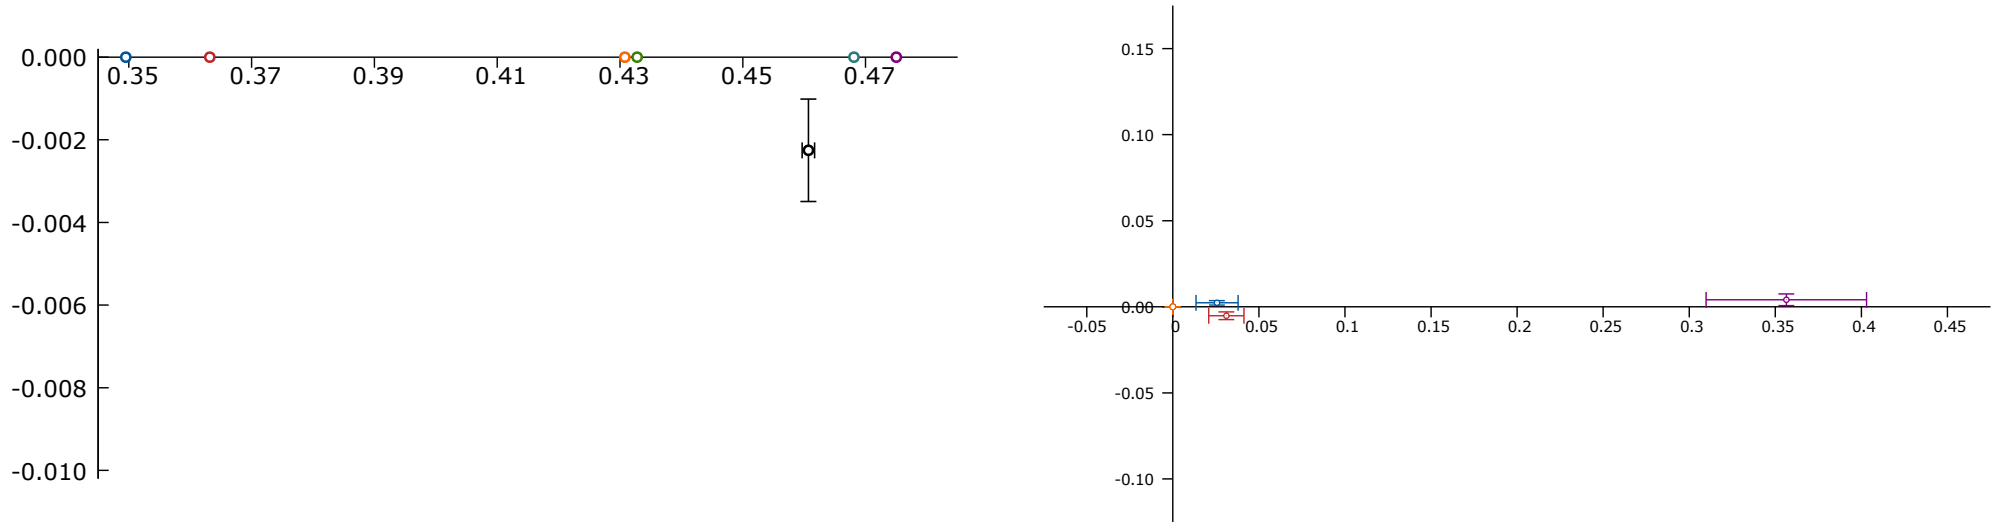

Figure 1.45: Left: Similar to Figure 13 in the manuscript, pole position on the proximal sheet (closest to physical scattering) with  $\text{Re}(a_t \sqrt{s})$  on the horizontal axis and  $2 \text{Im}(a_t \sqrt{s})$  on the vertical axis. Right: Similar to Figure 14 in the manuscript, the corresponding couplings with  $\text{Re}(a_t c)$  on the horizontal axis and  $\text{Im}(a_t c)$  on the vertical axis.

# 1.10 $\{m, g_{a,b,f}^{(0)}, \gamma_{(a,a),(b,b),(c,c),(\mathfrak{d}_1,\mathfrak{d}_1),(\mathfrak{d}_2,\mathfrak{d}_2),(\mathfrak{d}_3,\mathfrak{d}_3),(\mathfrak{e},\mathfrak{e}),(\mathfrak{f},\mathfrak{f})}\}(\mathbf{CM}_m)$

minimised with chisq/nDoF = 38.06 / (53 - 12) = 0.93

|                                                           |  |                       |  |      |      |      |       |       |       |       |       |      |       |       |       |
|-----------------------------------------------------------|--|-----------------------|--|------|------|------|-------|-------|-------|-------|-------|------|-------|-------|-------|
| =====                                                     |  |                       |  |      |      |      |       |       |       |       |       |      |       |       |       |
| JP1-_g_eta8:eta1/1^P_1_pole0                              |  | 0.30288 +/- 0.11507   |  | 1.00 | 0.79 | 0.63 | -0.51 | 0.21  | 0.67  | -0.40 | -0.04 | 0.02 | -0.06 | -0.06 | 0.50  |
| JP1-_g_h8:eta8/3^S_1_pole0                                |  | 0.72137 +/- 0.36223   |  |      | 1.00 | 0.83 | -0.17 | 0.26  | 0.94  | -0.62 | -0.03 | 0.05 | -0.02 | -0.04 | 0.35  |
| JP1-_g_omega8:eta8/3^P_1_pole0                            |  | 0.37007 +/- 0.15996   |  |      |      | 1.00 | -0.25 | 0.29  | 0.74  | -0.90 | -0.01 | 0.03 | -0.01 | -0.02 | 0.11  |
| JP1-_gamma_eta8:eta1/1^P_1 eta8:eta1/1^P_1_order0         |  | -4.1729 +/- 2.3102    |  |      |      | 1.00 | -0.08 | -0.19 | 0.25  | -0.01 |       | 0.06 | 0.02  | -0.02 | -0.09 |
| JP1-_gamma_f8:eta8/3^S_1 f8:eta8/3^S_1_order0             |  | -1.9552 +/- 0.29869   |  |      |      |      | 1.00  | 0.34  | -0.27 | 0.03  |       | 0.07 | 0.03  | 0.04  | -0.01 |
| JP1-_gamma_h8:eta8/3^S_1 h8:eta8/3^S_1_order0             |  | 14.556 +/- 8.4043     |  |      |      |      |       | 1.00  | -0.57 | -0.03 |       | 0.06 | -0.00 | -0.03 | 0.28  |
| JP1-_gamma_omega8:eta8/3^P_1 omega8:eta8/3^P_1_order0     |  | -5.6886 +/- 1.7205    |  |      |      |      |       |       | 1.00  | 0.03  |       | 0.01 | 0.03  | 0.05  | 0.08  |
| JP1-_gamma_omega8:omega1/1^P_1 omega8:omega1/1^P_1_order0 |  | 9.7178 +/- 2.3679     |  |      |      |      |       |       |       | 1.00  |       | 0.05 | 0.39  | 0.43  | -0.06 |
| JP1-_gamma_omega8:omega1/3^P_1 omega8:omega1/3^P_1_order0 |  | 11.286 +/- 4.9059     |  |      |      |      |       |       |       |       | 1.00  |      | 0.13  | 0.09  | 0.05  |
| JP1-_gamma_omega8:omega1/5^P_1 omega8:omega1/5^P_1_order0 |  | 19.158 +/- 3.7252     |  |      |      |      |       |       |       |       |       | 1.00 |       | 0.46  | -0.08 |
| JP1-_gamma_omega8:omega8/3^P_1 omega8:omega8/3^P_1_order0 |  | 10.860 +/- 2.913      |  |      |      |      |       |       |       |       |       |      | 1.00  |       | -0.11 |
| JP1-_m_pole0                                              |  | 0.46051 +/- 0.0010836 |  |      |      |      |       |       |       |       |       |      |       |       | 1.00  |
| =====                                                     |  |                       |  |      |      |      |       |       |       |       |       |      |       |       |       |

Phase space prescription ::

pole0\_sub

eta8:eta1[-] f8:eta8[+] h8:eta8[+] omega8:eta8[-] omega8:omega1[-] omega8:omega8[-] lower half-plane

sqrt(s)\_pole = (0.46033 +/- 0.0012263)  
+ (i/2)\*(-0.0060198 +/- 0.002065) [ 0.33]

s\_pole = ( 0.2119 +/- 0.0011311)  
+ i\*(-0.0027711 +/- 0.00094815) [ 0.33]

| eta8:eta1                | f8:eta8                  | h8:eta8                  | omega8:eta8              | omega8:omega1            | omega8:omega8            |
|--------------------------|--------------------------|--------------------------|--------------------------|--------------------------|--------------------------|
| k_re= 0.1488 +/- 0.0009  | k_re= -0.0074 +/- 0.0023 | k_re= -0.0054 +/- 0.0018 | k_re= 0.1399 +/- 0.0010  | k_re= 0.0785 +/- 0.0018  | k_re= 0.0812 +/- 0.0017  |
| k_im= -0.0023 +/- 0.0008 | k_im= 0.0401 +/- 0.0031  | k_im= 0.0542 +/- 0.0022  | k_im= -0.0024 +/- 0.0008 | k_im= -0.0044 +/- 0.0015 | k_im= -0.0043 +/- 0.0015 |
| corr= [ 0.34]            | corr= [-0.25]            | corr= [-0.29]            | corr= [ 0.34]            | corr= [ 0.35]            | corr= [ 0.35]            |

  

| eta8:eta1/1^P_1               | f8:eta8/3^S_1                | h8:eta8/3^S_1(*)              | omega8:eta8/3^P_1             | omega8:omega1/1^P_1          | omega8:omega1/3^P_1          | omega8:omega1/5^P_1          | omega8:omega8/3^P_1          |
|-------------------------------|------------------------------|-------------------------------|-------------------------------|------------------------------|------------------------------|------------------------------|------------------------------|
| g = 0.0448 +/- 0.0102         | g = 0.0000 +/- 0.0000        | g = 0.3500 +/- 0.0421         | g = 0.0510 +/- 0.0125         | g = 0.0000 +/- 0.0000        | g = 0.0000 +/- 0.0000        | g = 0.0000 +/- 0.0000        | g = 0.0000 +/- 0.0000        |
| arg(g)/pi= -0.0138 +/- 0.0521 | arg(g)/pi= 0.5120 +/- 0.0115 | arg(g)/pi= -0.0120 +/- 0.0115 | arg(g)/pi= -0.0237 +/- 0.0356 | arg(g)/pi= 0.5120 +/- 0.0115 | arg(g)/pi= 0.5120 +/- 0.0115 | arg(g)/pi= 0.5120 +/- 0.0115 | arg(g)/pi= 0.5120 +/- 0.0115 |
| g_re= 0.0448 +/- 0.0101       | g_re= -0.0000 +/- 0.0000     | g_re= 0.3498 +/- 0.0425       | g_re= 0.0508 +/- 0.0124       | g_re= -0.0000 +/- 0.0000     | g_re= -0.0000 +/- 0.0000     | g_re= -0.0000 +/- 0.0000     | g_re= -0.0000 +/- 0.0000     |
| g_im= -0.0019 +/- 0.0076      | g_im= 0.0000 +/- 0.0000      | g_im= -0.0132 +/- 0.0113      | g_im= -0.0038 +/- 0.0060      | g_im= 0.0000 +/- 0.0000      | g_im= 0.0000 +/- 0.0000      | g_im= 0.0000 +/- 0.0000      | g_im= 0.0000 +/- 0.0000      |
| corr= [-0.54]                 | corr= [-0.87]                | corr= [ 0.80]                 | corr= [-0.39]                 | corr= [-0.87]                | corr= [-0.87]                | corr= [-0.87]                | corr= [-0.87]                |

eta8:eta1[-] f8:eta8[+] h8:eta8[+] omega8:eta8[-] omega8:omega1[-] omega8:omega8[-] lower half-plane

sqrt(s)\_pole = (0.49379 +/- 0.0098872)  
+ (i/2)\*(-0.013062 +/- 0.023605) [-0.70]

s\_pole = (0.24379 +/- 0.0096565)  
+ i\*(-0.0064501 +/- 0.011748) [-0.70]

| eta8:eta1                | f8:eta8                  | h8:eta8                  | omega8:eta8              | omega8:omega1            | omega8:omega8            |
|--------------------------|--------------------------|--------------------------|--------------------------|--------------------------|--------------------------|
| k_re= 0.1734 +/- 0.0071  | k_re= -0.0742 +/- 0.0158 | k_re= -0.0637 +/- 0.0186 | k_re= 0.1657 +/- 0.0074  | k_re= 0.1190 +/- 0.0106  | k_re= 0.1208 +/- 0.0104  |
| k_im= -0.0046 +/- 0.0083 | k_im= 0.0097 +/- 0.0162  | k_im= 0.0111 +/- 0.0179  | k_im= -0.0048 +/- 0.0086 | k_im= -0.0068 +/- 0.0119 | k_im= -0.0067 +/- 0.0117 |
| corr= [-0.71]            | corr= [-0.71]            | corr= [-0.71]            | corr= [-0.71]            | corr= [-0.71]            | corr= [-0.71]            |

  

| eta8:eta1/1^P_1              | f8:eta8/3^S_1                | h8:eta8/3^S_1(*)             | omega8:eta8/3^P_1            | omega8:omega1/1^P_1          | omega8:omega1/3^P_1          | omega8:omega1/5^P_1          | omega8:omega8/3^P_1          |
|------------------------------|------------------------------|------------------------------|------------------------------|------------------------------|------------------------------|------------------------------|------------------------------|
| g = 0.0888 +/- 0.0342        | g = 0.0000 +/- 0.0000        | g = 0.1770 +/- 0.0239        | g = 0.1014 +/- 0.0395        | g = 0.0000 +/- 0.0000        | g = 0.0000 +/- 0.0000        | g = 0.0000 +/- 0.0000        | g = 0.0000 +/- 0.0000        |
| arg(g)/pi= 0.8304 +/- 0.0746 | arg(g)/pi= 0.1101 +/- 0.0660 | arg(g)/pi= 0.3899 +/- 0.0660 | arg(g)/pi= 0.8102 +/- 0.0639 | arg(g)/pi= 0.1101 +/- 0.0660 | arg(g)/pi= 0.1101 +/- 0.0660 | arg(g)/pi= 0.1101 +/- 0.0660 | arg(g)/pi= 0.1101 +/- 0.0660 |
| g_re= -0.0765 +/- 0.0248     | g_re= 0.0000 +/- 0.0000      | g_re= 0.0600 +/- 0.0383      | g_re= -0.0839 +/- 0.0219     | g_re= 0.0000 +/- 0.0000      | g_re= 0.0000 +/- 0.0000      | g_re= 0.0000 +/- 0.0000      | g_re= 0.0000 +/- 0.0000      |
| g_im= 0.0451 +/- 0.0314      | g_im= 0.0000 +/- 0.0000      | g_im= 0.1665 +/- 0.0212      | g_im= 0.0570 +/- 0.0386      | g_im= 0.0000 +/- 0.0000      | g_im= 0.0000 +/- 0.0000      | g_im= 0.0000 +/- 0.0000      | g_im= 0.0000 +/- 0.0000      |
| corr= [-0.67]                | corr= [-0.53]                | corr= [ 0.01]                | corr= [-0.96]                | corr= [-0.53]                | corr= [-0.53]                | corr= [-0.53]                | corr= [-0.53]                |

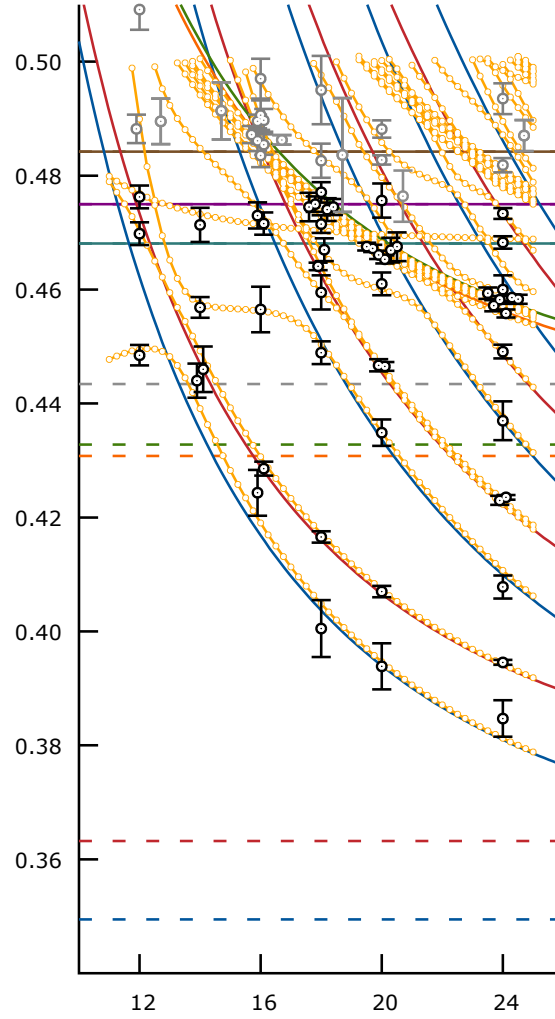

Figure 1.46: Similar to Figure 6 in the manuscript, the finite-volume spectrum, plotted as  $a_t E_{\text{cm}}$ , as a function of spatial extent  $L/a_s$ . Orange points/curves show the spectrum calculated from the amplitude given above (no uncertainties are shown). Black and grey points are the computed lattice energies on each volume, slightly displaced horizontally for clarity (black points correspond to energies used in the fit whereas grey points were not used). Two-meson non-interacting energies are shown as solid coloured curves/lines, two-meson thresholds are shown as dashed/solid horizontal lines, and the  $\eta^s \eta^s \eta^s$  threshold is shown as a dashed grey horizontal line.

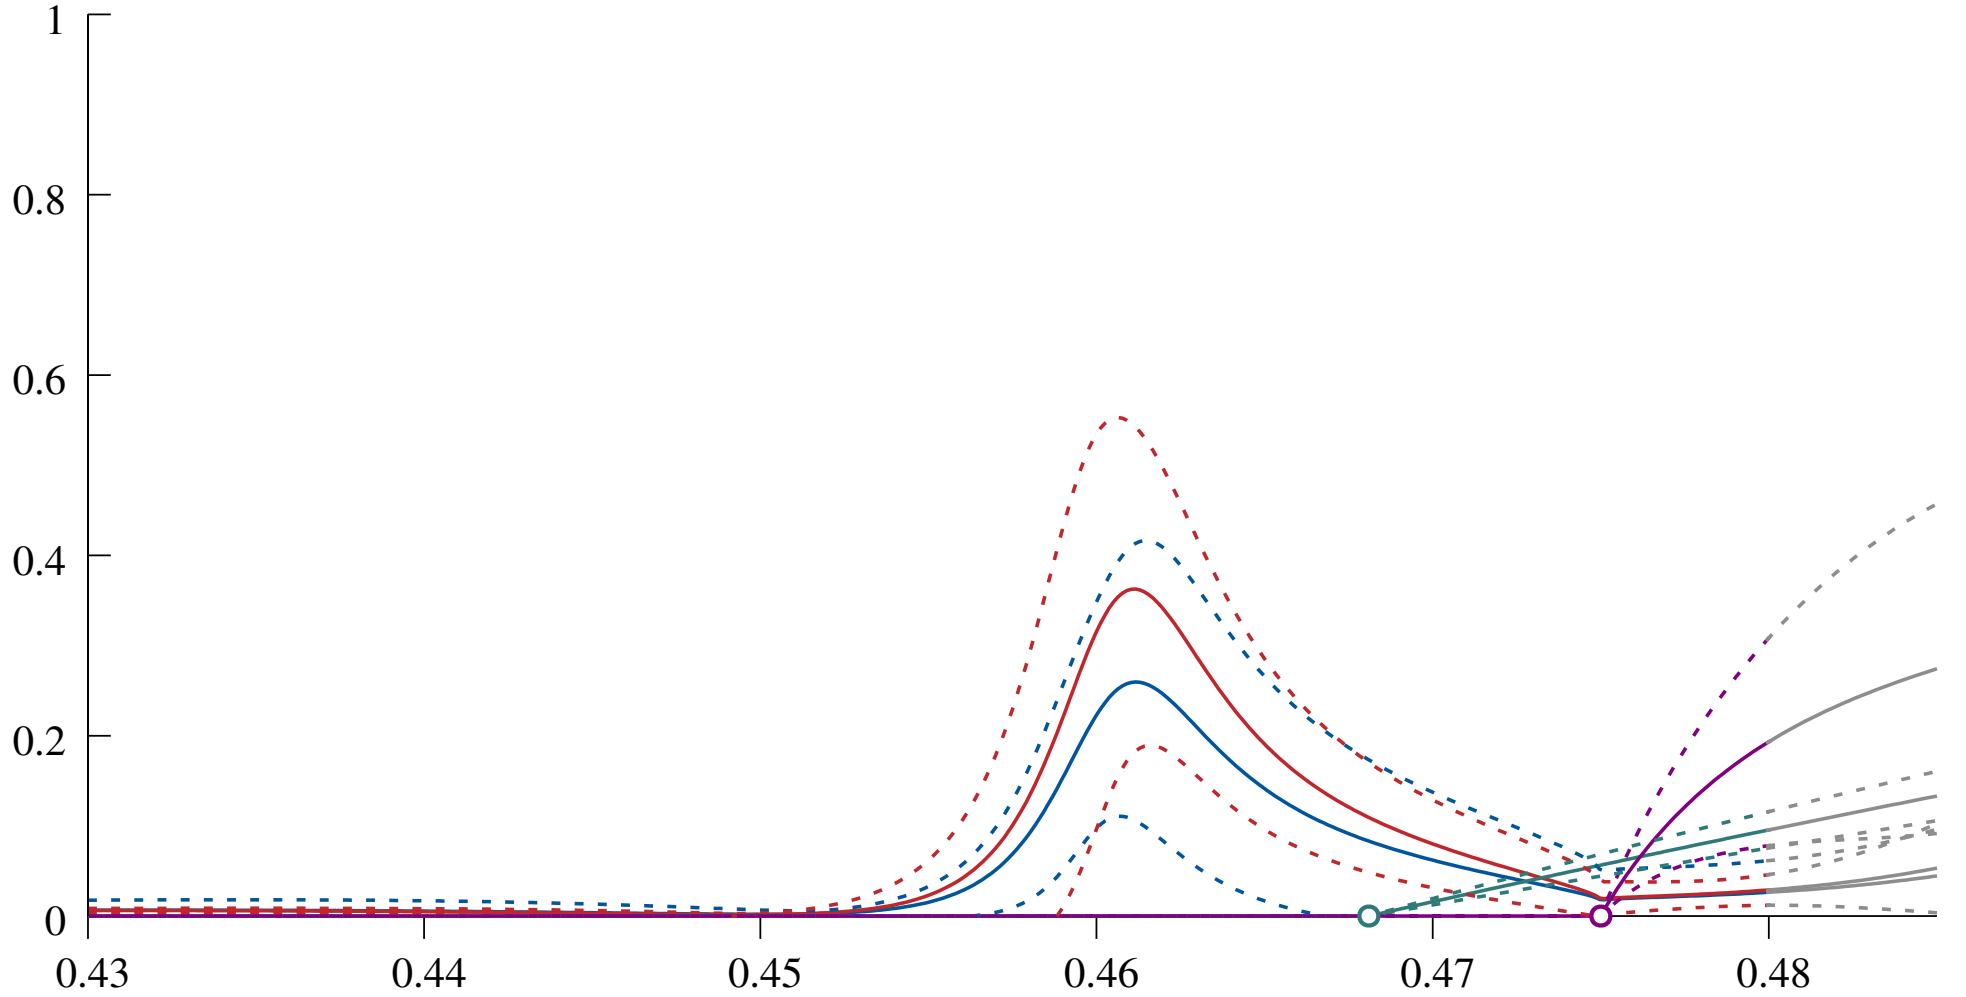

Figure 1.47: Similar to part (a) of Figure 7 in the manuscript,  $\rho_a \rho_b |t_{ab}|^2$  as a function of  $a_t E_{\text{cm}}$  for  $\eta^1 \eta^s \{^1P_1\} \rightarrow \eta^1 \eta^s \{^1P_1\}$  (blue),  $\omega^s \eta^s \{^3P_1\} \rightarrow \omega^s \eta^s \{^3P_1\}$  (red),  $f_1^s \eta^s \{^3S_1\} \rightarrow f_1^s \eta^s \{^3S_1\}$  (cyan), and  $h_1^s \eta^s \{^3S_1\} \rightarrow h_1^s \eta^s \{^3S_1\}$  (purple). Dashed lines indicate one standard deviation statistical uncertainties.

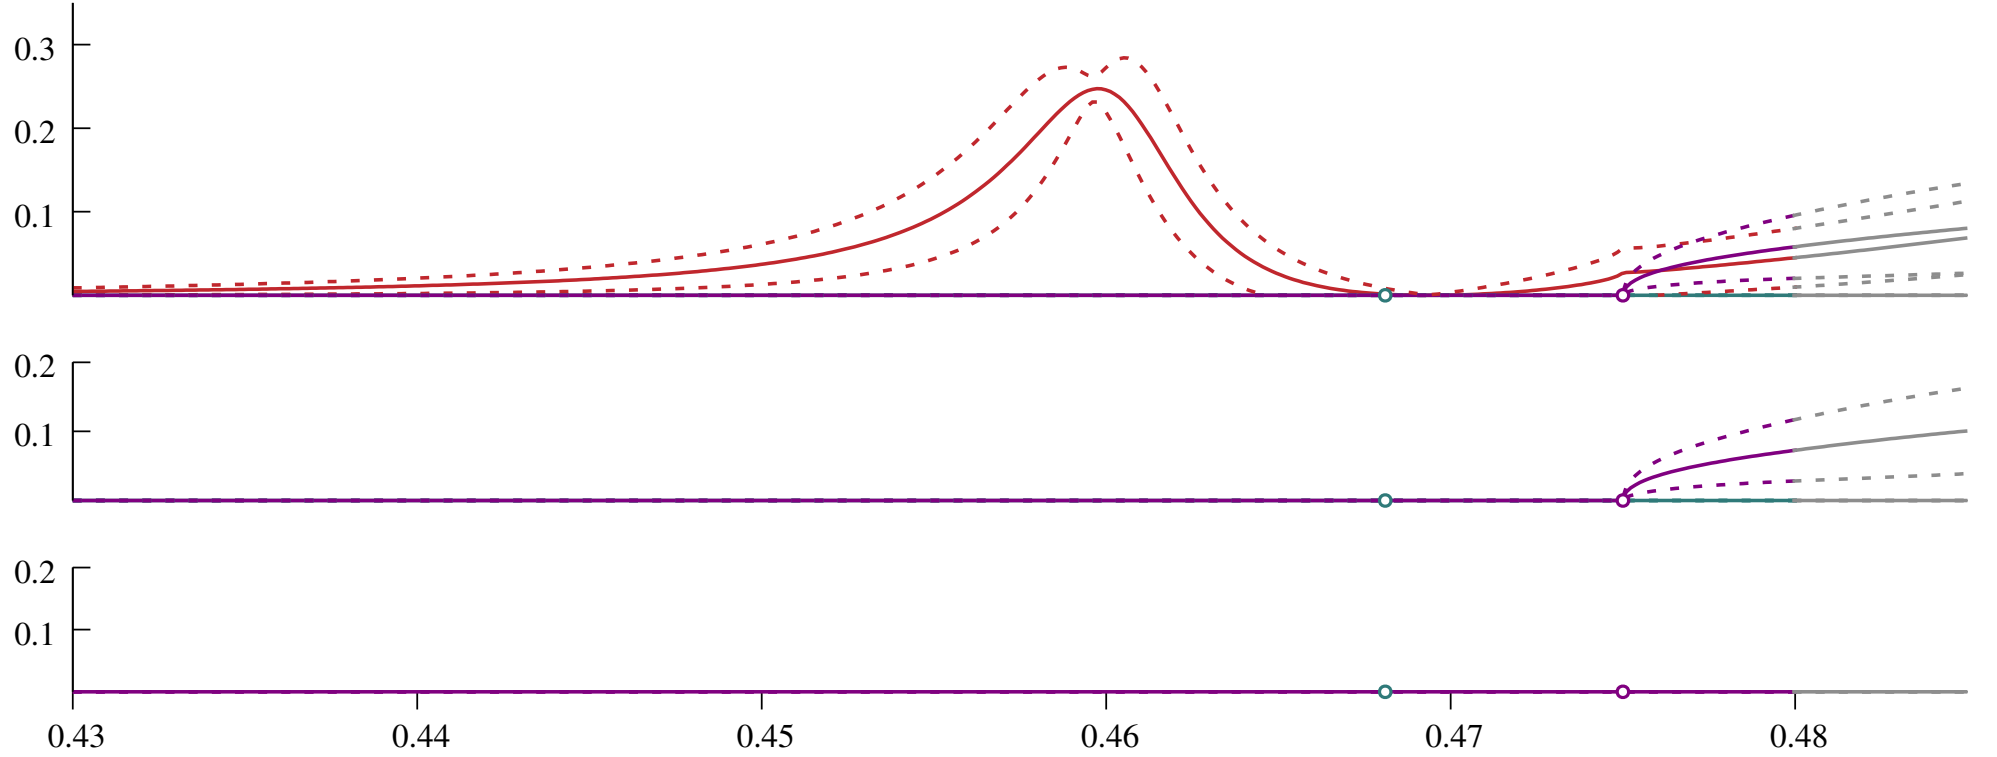

Figure 1.48: Similar to parts (b), (c) and (d) of Figure 7 in the manuscript,  $\rho_a \rho_b |t_{ab}|^2$  as a function of  $a_t E_{\text{cm}}$ . Top:  $\eta^1 \eta^s \{^1P_1\} \rightarrow \omega^s \eta^s \{^3P_1\}$  (red),  $\eta^1 \eta^s \{^1P_1\} \rightarrow f_1^s \eta^s \{^3S_1\}$  (cyan), and  $\eta^1 \eta^s \{^1P_1\} \rightarrow h_1^s \eta^s \{^3S_1\}$  (purple). Middle:  $\omega^s \eta^s \{^3P_1\} \rightarrow f_1^s \eta^s \{^3S_1\}$  (cyan), and  $\omega^s \eta^s \{^3P_1\} \rightarrow h_1^s \eta^s \{^3S_1\}$  (purple). Bottom:  $f_1^s \eta^s \{^3S_1\} \rightarrow h_1^s \eta^s \{^3S_1\}$  (purple). Dashed lines indicate one standard deviation statistical uncertainties.

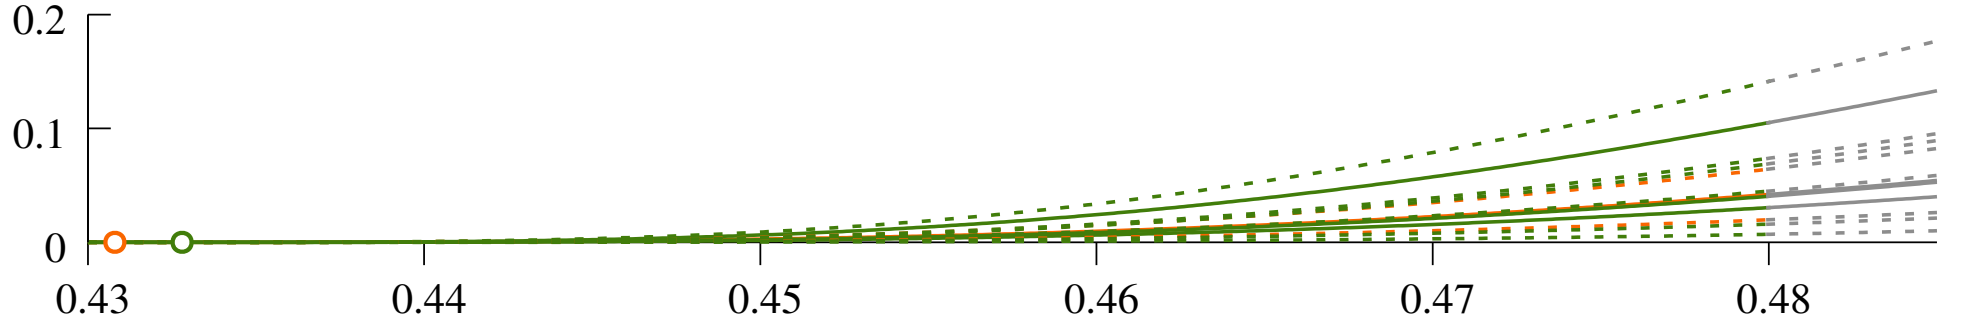

Figure 1.49: Similar to parts (e) and (f) of Figure 7 in the manuscript,  $\rho_a \rho_b |t_{ab}|^2$  as a function of  $a_t E_{cm}$  for  $\omega^s \omega^s \{^3P_1\} \rightarrow \omega^s \omega^s \{^3P_1\}$  (orange),  $\omega^1 \omega^s \{^1P_1, ^3P_1, ^5P_1\} \rightarrow \omega^s \omega^1 \{^1P_1, ^3P_1, ^5P_1\}$  (green). Dashed lines indicate one standard deviation statistical uncertainties.

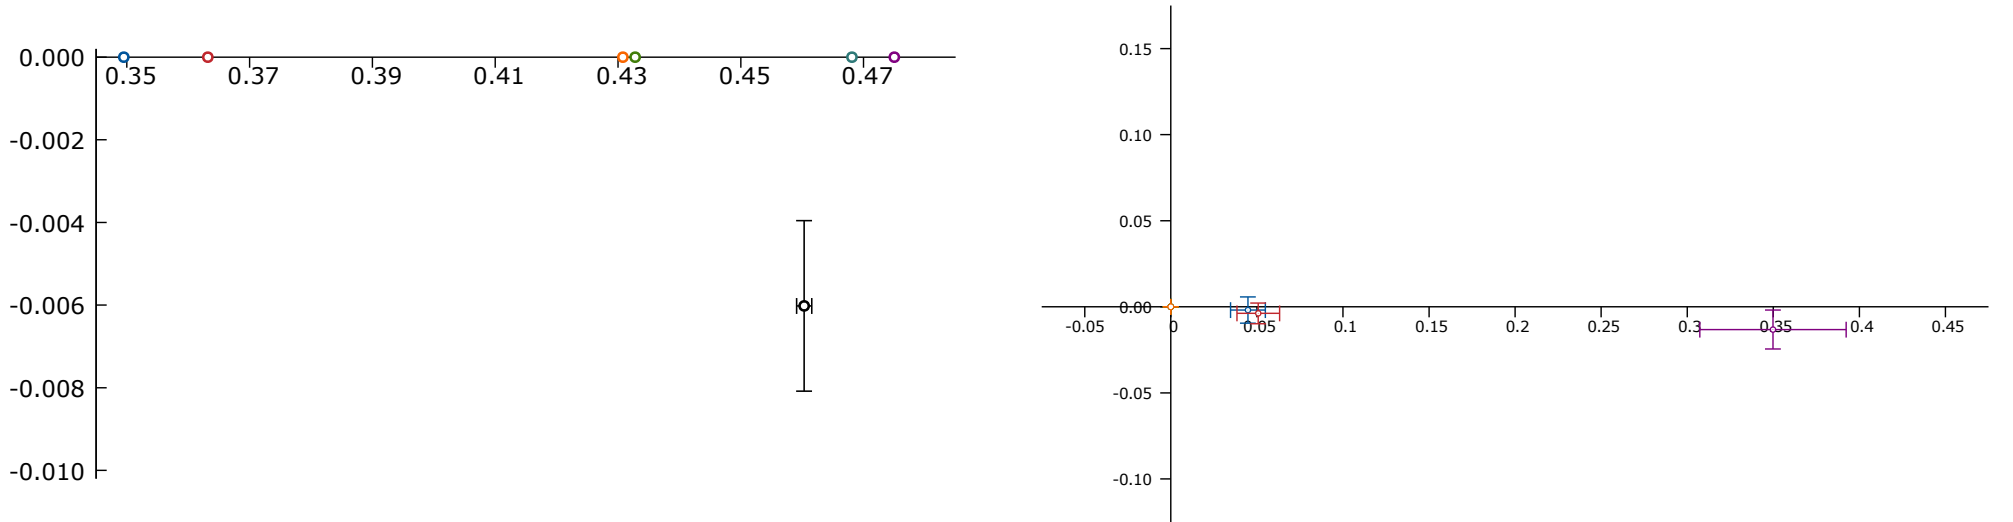

Figure 1.50: Left: Similar to Figure 13 in the manuscript, pole position on the proximal sheet (closest to physical scattering) with  $\text{Re}(a_t \sqrt{s})$  on the horizontal axis and  $2 \text{Im}(a_t \sqrt{s})$  on the vertical axis. Right: Similar to Figure 14 in the manuscript, the corresponding couplings with  $\text{Re}(a_t c)$  on the horizontal axis and  $\text{Im}(a_t c)$  on the vertical axis.

# 1.11 $\{m, g_{a,b,f}^{(0)}, \gamma_{(b,b),(c,c),(\partial_1,\partial_1),(\partial_2,\partial_2),(\partial_3,\partial_3),(\epsilon,\epsilon),(f,f)}^{(0)}\}(\mathbf{CM}_m)$

minimised with chisq/nDoF = 41.55 / (53 - 11) = 0.99

|                                                          |  |                        |  |      |      |      |      |      |       |       |      |       |       |       |
|----------------------------------------------------------|--|------------------------|--|------|------|------|------|------|-------|-------|------|-------|-------|-------|
| JP1-g_eta8:eta1/1^P_1_pole0                              |  | 0.18835 +/- 0.083034   |  | 1.00 | 0.63 | 0.49 | 0.18 | 0.20 | -0.20 | -0.03 | 0.01 | -0.05 | -0.06 | 0.43  |
| JP1-g_h8:eta8/3^S_1_pole0                                |  | 0.68648 +/- 0.35021    |  |      | 1.00 | 0.83 | 0.26 | 0.83 | -0.61 | -0.02 | 0.04 | -0.01 | -0.03 | 0.38  |
| JP1-g_omega8:eta8/3^P_1_pole0                            |  | 0.31275 +/- 0.14569    |  |      |      | 1.00 | 0.31 | 0.68 | -0.88 | -0.00 | 0.03 | -0.00 | -0.01 | 0.16  |
| JP1-gamma_f8:eta8/3^S_1 f8:eta8/3^S_1_order0             |  | -1.9801 +/- 0.3034     |  |      |      |      | 1.00 | 0.37 | -0.30 | 0.03  | 0.06 | 0.03  | 0.04  | -0.01 |
| JP1-gamma_h8:eta8/3^S_1 h8:eta8/3^S_1_order0             |  | 13.132 +/- 8.5605      |  |      |      |      |      | 1.00 | -0.61 | -0.02 | 0.06 | 0.01  | -0.00 | 0.21  |
| JP1-gamma_omega8:eta8/3^P_1 omega8:eta8/3^P_1_order0     |  | -4.9803 +/- 1.4702     |  |      |      |      |      |      | 1.00  | 0.03  | 0.00 | 0.02  | 0.06  | 0.04  |
| JP1-gamma_omega8:omega1/1^P_1 omega8:omega1/1^P_1_order0 |  | 9.6430 +/- 2.3648      |  |      |      |      |      |      |       | 1.00  | 0.05 | 0.39  | 0.43  | -0.06 |
| JP1-gamma_omega8:omega1/3^P_1 omega8:omega1/3^P_1_order0 |  | 11.964 +/- 4.9216      |  |      |      |      |      |      |       |       | 1.00 | 0.13  | 0.10  | 0.05  |
| JP1-gamma_omega8:omega1/5^P_1 omega8:omega1/5^P_1_order0 |  | 19.345 +/- 3.7349      |  |      |      |      |      |      |       |       |      | 1.00  | 0.46  | -0.08 |
| JP1-gamma_omega8:omega8/3^P_1 omega8:omega8/3^P_1_order0 |  | 10.731 +/- 2.9062      |  |      |      |      |      |      |       |       |      |       | 1.00  | -0.11 |
| JP1-m_pole0                                              |  | 0.46034 +/- 0.00094855 |  |      |      |      |      |      |       |       |      |       |       | 1.00  |

Phase space prescription ::

pole0\_sub

eta8:eta1[-] f8:eta8[+] h8:eta8[+] omega8:eta8[-] omega8:omega1[-] omega8:omega8[-] lower half-plane

sqrt(s)\_pole = (0.46024 +/- 0.0010022)  
+ (i/2)\*(-0.0035928 +/- 0.0015477) [ 0.35]

s\_pole = (0.21181 +/- 0.00092345)  
+ i\*(-0.0016535 +/- 0.00071105) [ 0.35]

| eta8:eta1                | f8:eta8                  | h8:eta8                  | omega8:eta8              | omega8:omega1            | omega8:omega8            |
|--------------------------|--------------------------|--------------------------|--------------------------|--------------------------|--------------------------|
| k_re= 0.1487 +/- 0.0008  | k_re= -0.0044 +/- 0.0018 | k_re= -0.0032 +/- 0.0013 | k_re= 0.1398 +/- 0.0008  | k_re= 0.0783 +/- 0.0015  | k_re= 0.0810 +/- 0.0014  |
| k_im= -0.0014 +/- 0.0006 | k_im= 0.0399 +/- 0.0025  | k_im= 0.0542 +/- 0.0018  | k_im= -0.0015 +/- 0.0006 | k_im= -0.0026 +/- 0.0012 | k_im= -0.0026 +/- 0.0011 |
| corr= [ 0.35]            | corr= [-0.29]            | corr= [-0.32]            | corr= [ 0.35]            | corr= [ 0.36]            | corr= [ 0.36]            |

  

| eta8:eta1/1^P_1              | f8:eta8/3^S_1                | h8:eta8/3^S_1(*)              | omega8:eta8/3^P_1             | omega8:omega1/1^P_1          | omega8:omega1/3^P_1          | omega8:omega1/5^P_1          | omega8:omega8/3^P_1          |
|------------------------------|------------------------------|-------------------------------|-------------------------------|------------------------------|------------------------------|------------------------------|------------------------------|
| lg = 0.0287 +/- 0.0098       | lg = 0.0000 +/- 0.0000       | lg = 0.3437 +/- 0.0443        | lg = 0.0433 +/- 0.0121        | lg = 0.0000 +/- 0.0000       | lg = 0.0000 +/- 0.0000       | lg = 0.0000 +/- 0.0000       | lg = 0.0000 +/- 0.0000       |
| arg(g)/pi= 0.0337 +/- 0.0299 | arg(g)/pi= 0.5066 +/- 0.0069 | arg(g)/pi= -0.0066 +/- 0.0069 | arg(g)/pi= -0.0406 +/- 0.0179 | arg(g)/pi= 0.5066 +/- 0.0069 | arg(g)/pi= 0.5066 +/- 0.0069 | arg(g)/pi= 0.5066 +/- 0.0069 | arg(g)/pi= 0.5066 +/- 0.0069 |
| g_re= 0.0285 +/- 0.0098      | g_re= -0.0000 +/- 0.0000     | g_re= 0.3436 +/- 0.0444       | g_re= 0.0429 +/- 0.0119       | g_re= -0.0000 +/- 0.0000     | g_re= -0.0000 +/- 0.0000     | g_re= -0.0000 +/- 0.0000     | g_re= -0.0000 +/- 0.0000     |
| g_im= 0.0030 +/- 0.0025      | g_im= 0.0000 +/- 0.0000      | g_im= -0.0072 +/- 0.0068      | g_im= -0.0055 +/- 0.0032      | g_im= 0.0000 +/- 0.0000      | g_im= 0.0000 +/- 0.0000      | g_im= 0.0000 +/- 0.0000      | g_im= 0.0000 +/- 0.0000      |
| corr= [ 0.03]                | corr= [-0.80]                | corr= [ 0.70]                 | corr= [-0.66]                 | corr= [-0.80]                | corr= [-0.80]                | corr= [-0.80]                | corr= [-0.80]                |

eta8:eta1[-] f8:eta8[+] h8:eta8[+] omega8:eta8[-] omega8:omega1[-] omega8:omega8[-] lower half-plane

sqrt(s)\_pole = (0.49834 +/- 0.017205)  
+ (i/2)\*(-0.0021297 +/- 0.019707) [-0.51]

s\_pole = (0.24834 +/- 0.017139)  
+ i\*(-0.0010617 +/- 0.00984) [-0.51]

| eta8:eta1                | f8:eta8                  | h8:eta8                  | omega8:eta8              | omega8:omega1            | omega8:omega8            |
|--------------------------|--------------------------|--------------------------|--------------------------|--------------------------|--------------------------|
| k_re= 0.1724 +/- 0.8568  | k_re= -0.0783 +/- 0.3860 | k_re= -0.0687 +/- 0.3376 | k_re= 0.1650 +/- 0.8198  | k_re= 0.1206 +/- 0.5976  | k_re= 0.1223 +/- 0.6061  |
| k_im= -0.0007 +/- 0.0068 | k_im= 0.0015 +/- 0.0133  | k_im= 0.0017 +/- 0.0148  | k_im= -0.0008 +/- 0.0071 | k_im= -0.0011 +/- 0.0097 | k_im= -0.0011 +/- 0.0096 |
| corr= [-0.24]            | corr= [-0.27]            | corr= [-0.27]            | corr= [-0.25]            | corr= [-0.25]            | corr= [-0.25]            |

  

| eta8:eta1/1^P_1              | f8:eta8/3^S_1                | h8:eta8/3^S_1(*)             | omega8:eta8/3^P_1            | omega8:omega1/1^P_1          | omega8:omega1/3^P_1          | omega8:omega1/5^P_1          | omega8:omega8/3^P_1          |
|------------------------------|------------------------------|------------------------------|------------------------------|------------------------------|------------------------------|------------------------------|------------------------------|
| lg = 0.0610 +/- 0.0320       | lg = 0.0000 +/- 0.0000       | lg = 0.1665 +/- 0.0329       | lg = 0.0939 +/- 0.0438       | lg = 0.0000 +/- 0.0000       | lg = 0.0000 +/- 0.0000       | lg = 0.0000 +/- 0.0000       | lg = 0.0000 +/- 0.0000       |
| arg(g)/pi= 0.9541 +/- 2.2690 | arg(g)/pi= 0.1168 +/- 1.8971 | arg(g)/pi= 0.3832 +/- 1.8971 | arg(g)/pi= 0.8342 +/- 1.6831 | arg(g)/pi= 0.1168 +/- 1.8971 | arg(g)/pi= 0.1168 +/- 1.8971 | arg(g)/pi= 0.1168 +/- 1.8971 | arg(g)/pi= 0.1168 +/- 1.8971 |
| g_re= -0.0592 +/- 0.2900     | g_re= 0.0000 +/- 0.0000      | g_re= 0.0551 +/- 0.0355      | g_re= -0.0807 +/- 0.3962     | g_re= 0.0000 +/- 0.0000      | g_re= 0.0000 +/- 0.0000      | g_re= 0.0000 +/- 0.0000      | g_re= 0.0000 +/- 0.0000      |
| g_im= 0.0066 +/- 0.0074      | g_im= 0.0000 +/- 0.0000      | g_im= 0.1533 +/- 0.7663      | g_im= 0.0446 +/- 0.0380      | g_im= 0.0000 +/- 0.0000      | g_im= 0.0000 +/- 0.0000      | g_im= 0.0000 +/- 0.0000      | g_im= 0.0000 +/- 0.0000      |
| corr= [-0.32]                | corr= [-0.13]                | corr= [-0.25]                | corr= [-0.30]                | corr= [-0.13]                | corr= [-0.13]                | corr= [-0.13]                | corr= [-0.13]                |

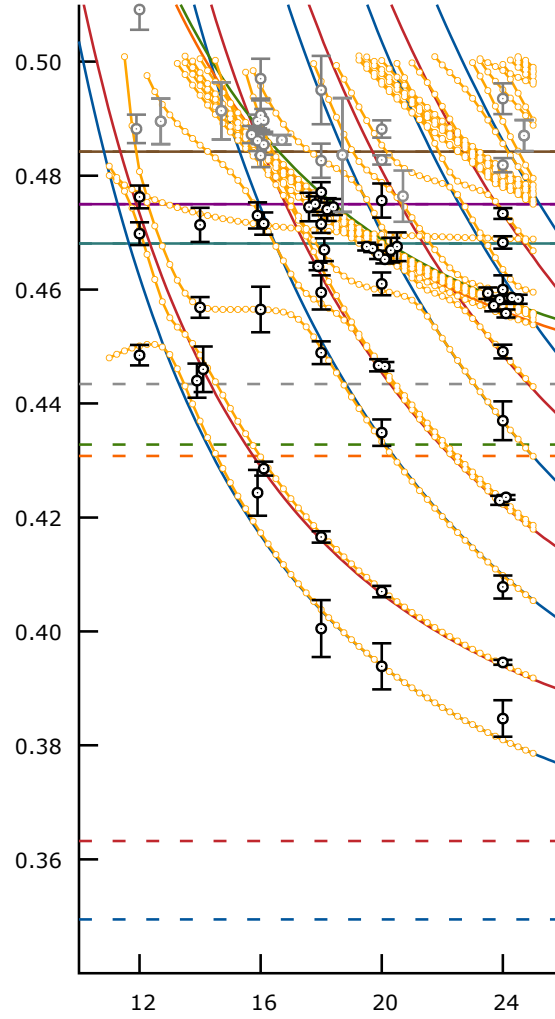

Figure 1.51: Similar to Figure 6 in the manuscript, the finite-volume spectrum, plotted as  $a_t E_{\text{cm}}$ , as a function of spatial extent  $L/a_s$ . Orange points/curves show the spectrum calculated from the amplitude given above (no uncertainties are shown). Black and grey points are the computed lattice energies on each volume, slightly displaced horizontally for clarity (black points correspond to energies used in the fit whereas grey points were not used). Two-meson non-interacting energies are shown as solid coloured curves/lines, two-meson thresholds are shown as dashed/solid horizontal lines, and the  $\eta^s \eta^s \eta^s$  threshold is shown as a dashed grey horizontal line.

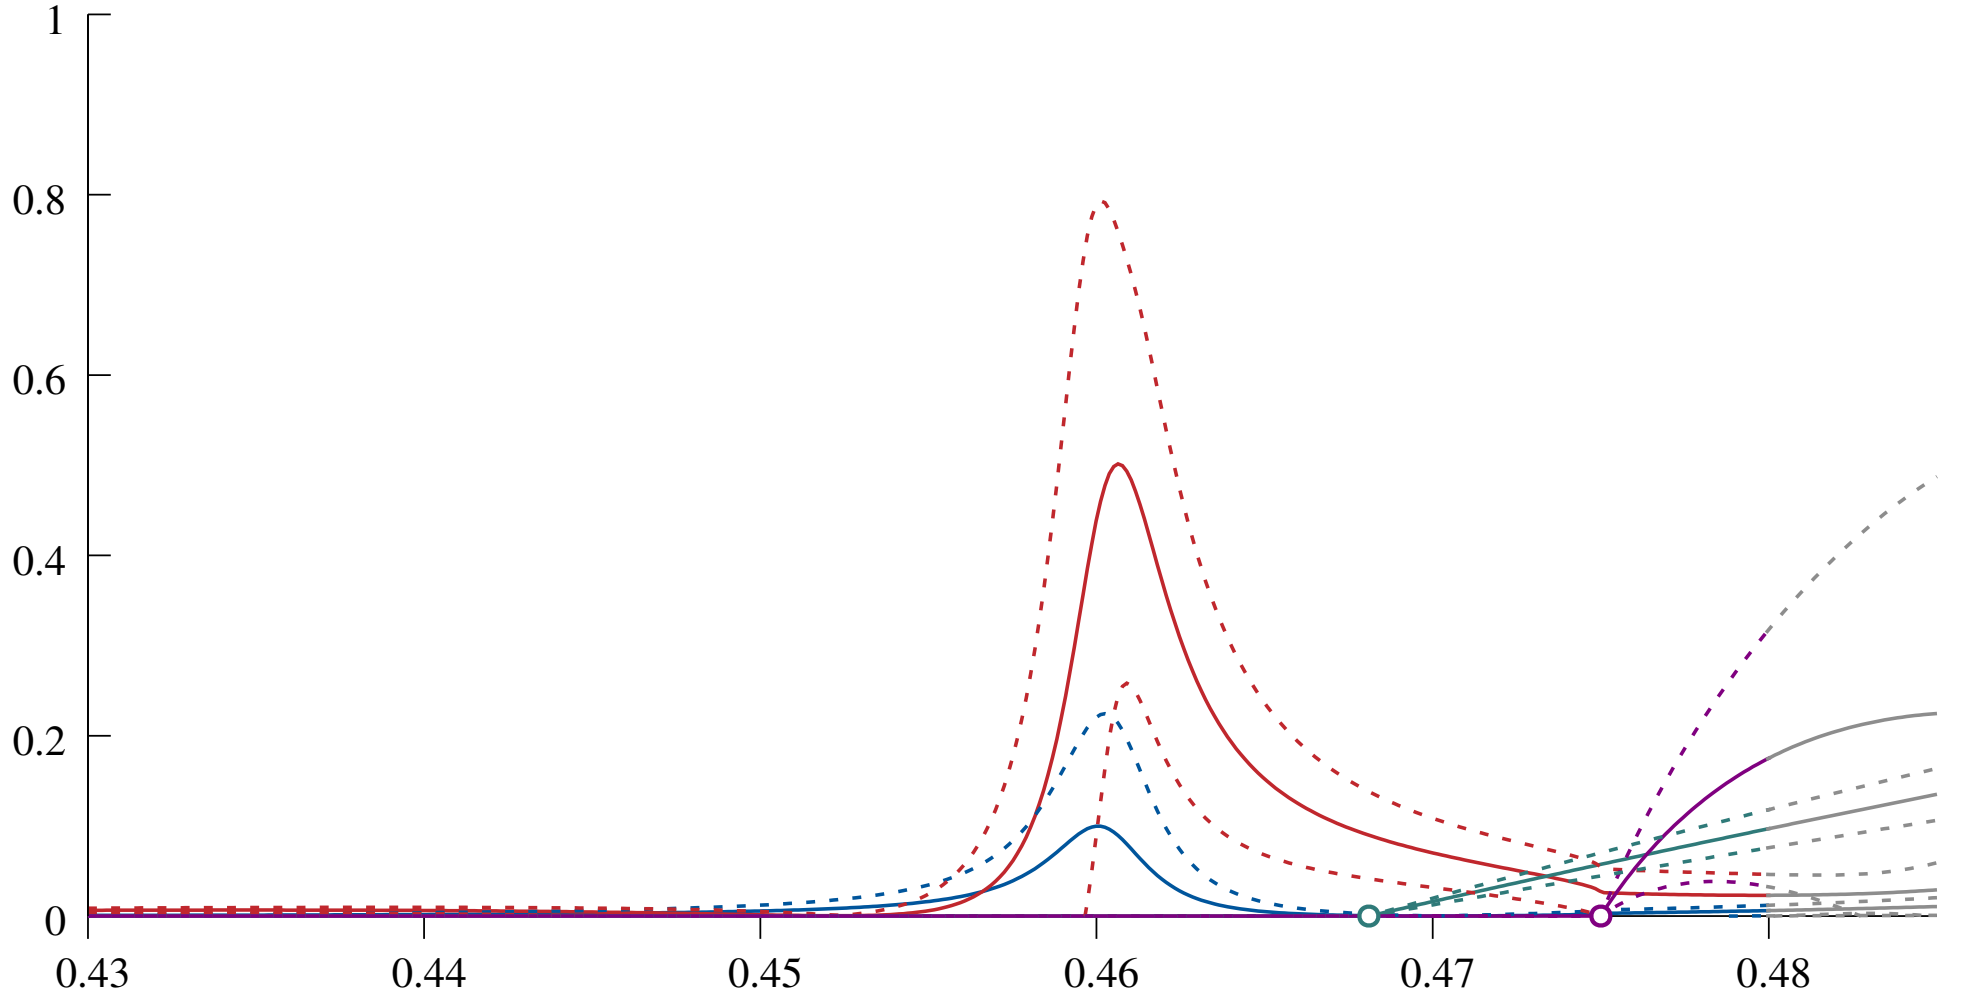

Figure 1.52: Similar to part (a) of Figure 7 in the manuscript,  $\rho_a \rho_b |t_{ab}|^2$  as a function of  $a_t E_{\text{cm}}$  for  $\eta^1 \eta^8 \{^1P_1\} \rightarrow \eta^1 \eta^8 \{^1P_1\}$  (blue),  $\omega^8 \eta^8 \{^3P_1\} \rightarrow \omega^8 \eta^8 \{^3P_1\}$  (red),  $f_1^8 \eta^8 \{^3S_1\} \rightarrow f_1^8 \eta^8 \{^3S_1\}$  (cyan), and  $h_1^8 \eta^8 \{^3S_1\} \rightarrow h_1^8 \eta^8 \{^3S_1\}$  (purple). Dashed lines indicate one standard deviation statistical uncertainties.

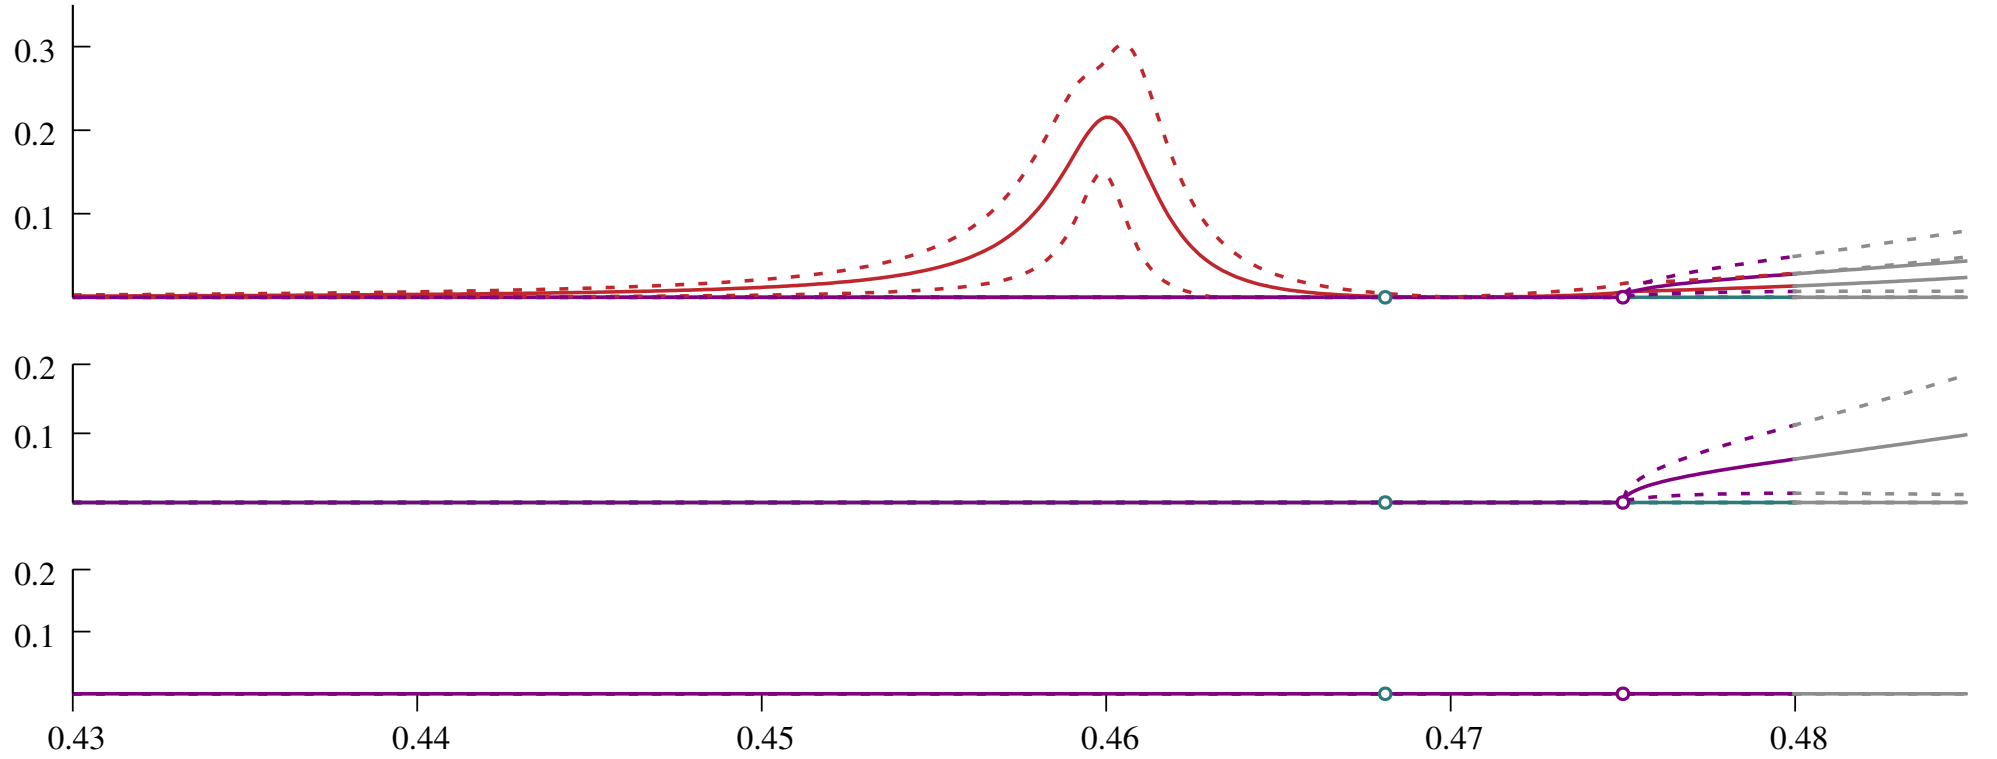

Figure 1.53: Similar to parts (b), (c) and (d) of Figure 7 in the manuscript,  $\rho_a \rho_b |t_{ab}|^2$  as a function of  $a_t E_{\text{cm}}$ . Top:  $\eta^1 \eta^s \{^1P_1\} \rightarrow \omega^s \eta^s \{^3P_1\}$  (red),  $\eta^1 \eta^s \{^1P_1\} \rightarrow f_1^s \eta^s \{^3S_1\}$  (cyan), and  $\eta^1 \eta^s \{^1P_1\} \rightarrow h_1^s \eta^s \{^3S_1\}$  (purple). Middle:  $\omega^s \eta^s \{^3P_1\} \rightarrow f_1^s \eta^s \{^3S_1\}$  (cyan), and  $\omega^s \eta^s \{^3P_1\} \rightarrow h_1^s \eta^s \{^3S_1\}$  (purple). Bottom:  $f_1^s \eta^s \{^3S_1\} \rightarrow h_1^s \eta^s \{^3S_1\}$  (purple). Dashed lines indicate one standard deviation statistical uncertainties.

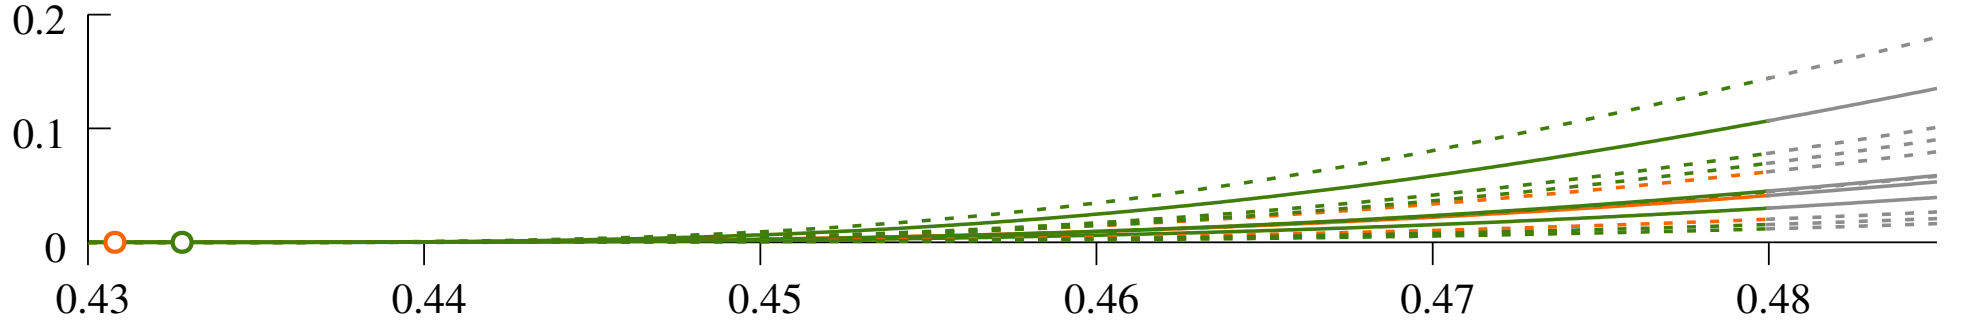

Figure 1.54: Similar to parts (e) and (f) of Figure 7 in the manuscript,  $\rho_a \rho_b |t_{ab}|^2$  as a function of  $a_t E_{cm}$  for  $\omega^s \omega^s \{^3P_1\} \rightarrow \omega^s \omega^s \{^3P_1\}$  (orange),  $\omega^1 \omega^s \{^1P_1, ^3P_1, ^5P_1\} \rightarrow \omega^s \omega^1 \{^1P_1, ^3P_1, ^5P_1\}$  (green). Dashed lines indicate one standard deviation statistical uncertainties.

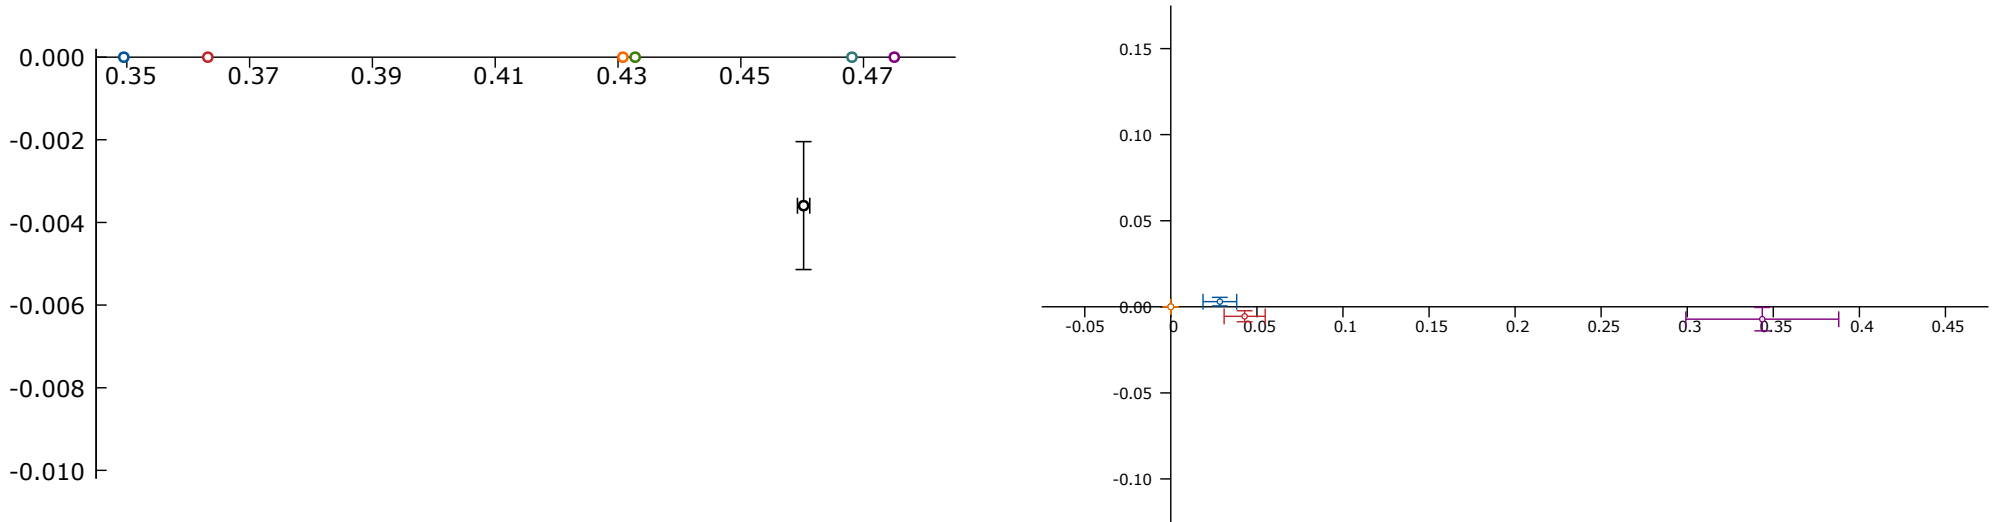

Figure 1.55: Left: Similar to Figure 13 in the manuscript, pole position on the proximal sheet (closest to physical scattering) with  $\text{Re}(a_t \sqrt{s})$  on the horizontal axis and  $2 \text{Im}(a_t \sqrt{s})$  on the vertical axis. Right: Similar to Figure 14 in the manuscript, the corresponding couplings with  $\text{Re}(a_t c)$  on the horizontal axis and  $\text{Im}(a_t c)$  on the vertical axis.

## 1.12 $\{m, g_{a,b,f}^{(0)}, \gamma_{(b,b),(c,c),(\partial_1,\partial_1),(\partial_2,\partial_2),(\partial_3,\partial_3),(\epsilon,\epsilon)}^{(0)}\}(\mathbf{CM}_m)$

minimised with chisq/ndof = 52.09 / (53 - 10) = 1.21

|                                                          |  |                       |  |      |      |      |      |       |       |      |                  |
|----------------------------------------------------------|--|-----------------------|--|------|------|------|------|-------|-------|------|------------------|
| =====                                                    |  |                       |  |      |      |      |      |       |       |      |                  |
| JP1-g_eta8:eta1/1^P_1_pole0                              |  | 0.19235 +/- 0.075795  |  | 1.00 | 0.68 | 0.41 | 0.31 | 0.03  | -0.04 | 0.01 | -0.08 -0.06 0.63 |
| JP1-g_h8:eta8/3^S_1_pole0                                |  | 0.50846 +/- 0.21994   |  |      | 1.00 | 0.61 | 0.33 | -0.05 | -0.01 | 0.04 | -0.01 -0.02 0.56 |
| JP1-g_omega8:eta8/3^P_1_pole0                            |  | 0.17589 +/- 0.079381  |  |      |      | 1.00 | 0.19 | -0.42 | 0.03  | 0.02 | 0.02 0.02 0.21   |
| JP1-gamma_f8:eta8/3^S_1 f8:eta8/3^S_1_order0             |  | -2.5438 +/- 0.25869   |  |      |      |      | 1.00 | 0.04  | 0.02  | 0.05 | 0.01 0.02 0.27   |
| JP1-gamma_omega8:eta8/3^P_1 omega8:eta8/3^P_1_order0     |  | -3.5436 +/- 0.5985    |  |      |      |      |      | 1.00  | 0.06  | 0.08 | 0.06 0.14 0.11   |
| JP1-gamma_omega8:omega1/1^P_1 omega8:omega1/1^P_1_order0 |  | 9.4488 +/- 2.3595     |  |      |      |      |      |       | 1.00  | 0.05 | 0.39 0.43 -0.06  |
| JP1-gamma_omega8:omega1/3^P_1 omega8:omega1/3^P_1_order0 |  | 11.229 +/- 4.8949     |  |      |      |      |      |       |       | 1.00 | 0.13 0.10 0.05   |
| JP1-gamma_omega8:omega1/5^P_1 omega8:omega1/5^P_1_order0 |  | 18.927 +/- 3.7179     |  |      |      |      |      |       |       |      | 1.00 0.46 -0.09  |
| JP1-gamma_omega8:omega8/3^P_1 omega8:omega8/3^P_1_order0 |  | 10.387 +/- 2.8915     |  |      |      |      |      |       |       |      | 1.00 -0.10       |
| JP1-m_pole0                                              |  | 0.46081 +/- 0.0010515 |  |      |      |      |      |       |       |      | 1.00             |
| =====                                                    |  |                       |  |      |      |      |      |       |       |      |                  |

Phase space prescription ::

pole0\_sub

eta8:eta1[-] f8:eta8[+] h8:eta8[+] omega8:eta8[-] omega8:omega1[-] omega8:omega8[-] lower half-plane

sqrt(s)\_pole = (0.46071 +/- 0.0010778)  
+ (1/2)\*(-0.0028896 +/- 0.0013283) [-0.09]

s\_pole = (0.21226 +/- 0.00099294)  
+ i\*(-0.0013313 +/- 0.00061226) [-0.10]

| eta8:eta1                                                            | f8:eta8                                                              | h8:eta8                                                              | omega8:eta8                                                          | omega8:omega1                                                        | omega8:omega8                                                        |
|----------------------------------------------------------------------|----------------------------------------------------------------------|----------------------------------------------------------------------|----------------------------------------------------------------------|----------------------------------------------------------------------|----------------------------------------------------------------------|
| k_re= 0.1491 +/- 0.0008<br>k_im= -0.0011 +/- 0.0005<br>corr= [-0.09] | k_re= -0.0037 +/- 0.0017<br>k_im= 0.0386 +/- 0.0027<br>corr= [ 0.19] | k_re= -0.0026 +/- 0.0012<br>k_im= 0.0533 +/- 0.0019<br>corr= [ 0.15] | k_re= 0.1402 +/- 0.0009<br>k_im= -0.0012 +/- 0.0005<br>corr= [-0.09] | k_re= 0.0790 +/- 0.0016<br>k_im= -0.0021 +/- 0.0010<br>corr= [-0.07] | k_re= 0.0817 +/- 0.0015<br>k_im= -0.0020 +/- 0.0009<br>corr= [-0.07] |

  

| eta8:eta1/1^P_1                                                     | f8:eta8/3^S_1                                                       | h8:eta8/3^S_1(*)                                                    | omega8:eta8/3^P_1                                                    | omega8:omega1/1^P_1                                                 | omega8:omega1/3^P_1                                                 | omega8:omega1/5^P_1                                                 | omega8:omega8/3^P_1                                                 |
|---------------------------------------------------------------------|---------------------------------------------------------------------|---------------------------------------------------------------------|----------------------------------------------------------------------|---------------------------------------------------------------------|---------------------------------------------------------------------|---------------------------------------------------------------------|---------------------------------------------------------------------|
| g = 0.0351 +/- 0.0100<br>arg(g)/pi= 0.0005 +/- 0.0024               | g = 0.0000 +/- 0.0000<br>arg(g)/pi= 0.4972 +/- 0.0028               | g = 0.3108 +/- 0.0498<br>arg(g)/pi= 0.0028 +/- 0.0028               | g = 0.0296 +/- 0.0106<br>arg(g)/pi= -0.0534 +/- 0.0087               | g = 0.0000 +/- 0.0000<br>arg(g)/pi= 0.4972 +/- 0.0028               | g = 0.0000 +/- 0.0000<br>arg(g)/pi= 0.4972 +/- 0.0028               | g = 0.0000 +/- 0.0000<br>arg(g)/pi= 0.4972 +/- 0.0028               | g = 0.0000 +/- 0.0000<br>arg(g)/pi= 0.4972 +/- 0.0028               |
| g_re= 0.0351 +/- 0.0100<br>g_im= 0.0001 +/- 0.0003<br>corr= [ 0.26] | g_re= 0.0000 +/- 0.0000<br>g_im= 0.0000 +/- 0.0000<br>corr= [-0.79] | g_re= 0.3108 +/- 0.0498<br>g_im= 0.0028 +/- 0.0031<br>corr= [ 0.88] | g_re= 0.0292 +/- 0.0104<br>g_im= -0.0049 +/- 0.0022<br>corr= [-0.95] | g_re= 0.0000 +/- 0.0000<br>g_im= 0.0000 +/- 0.0000<br>corr= [-0.79] | g_re= 0.0000 +/- 0.0000<br>g_im= 0.0000 +/- 0.0000<br>corr= [-0.79] | g_re= 0.0000 +/- 0.0000<br>g_im= 0.0000 +/- 0.0000<br>corr= [-0.79] | g_re= 0.0000 +/- 0.0000<br>g_im= 0.0000 +/- 0.0000<br>corr= [-0.79] |

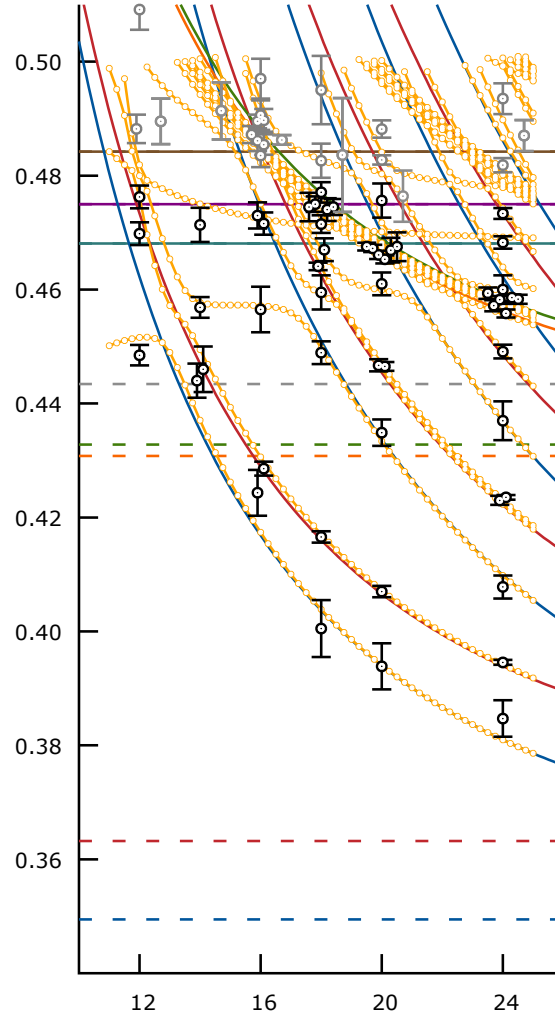

Figure 1.56: Similar to Figure 6 in the manuscript, the finite-volume spectrum, plotted as  $a_t E_{\text{cm}}$ , as a function of spatial extent  $L/a_s$ . Orange points/curves show the spectrum calculated from the amplitude given above (no uncertainties are shown). Black and grey points are the computed lattice energies on each volume, slightly displaced horizontally for clarity (black points correspond to energies used in the fit whereas grey points were not used). Two-meson non-interacting energies are shown as solid coloured curves/lines, two-meson thresholds are shown as dashed/solid horizontal lines, and the  $\eta^s \eta^s \eta^s$  threshold is shown as a dashed grey horizontal line.

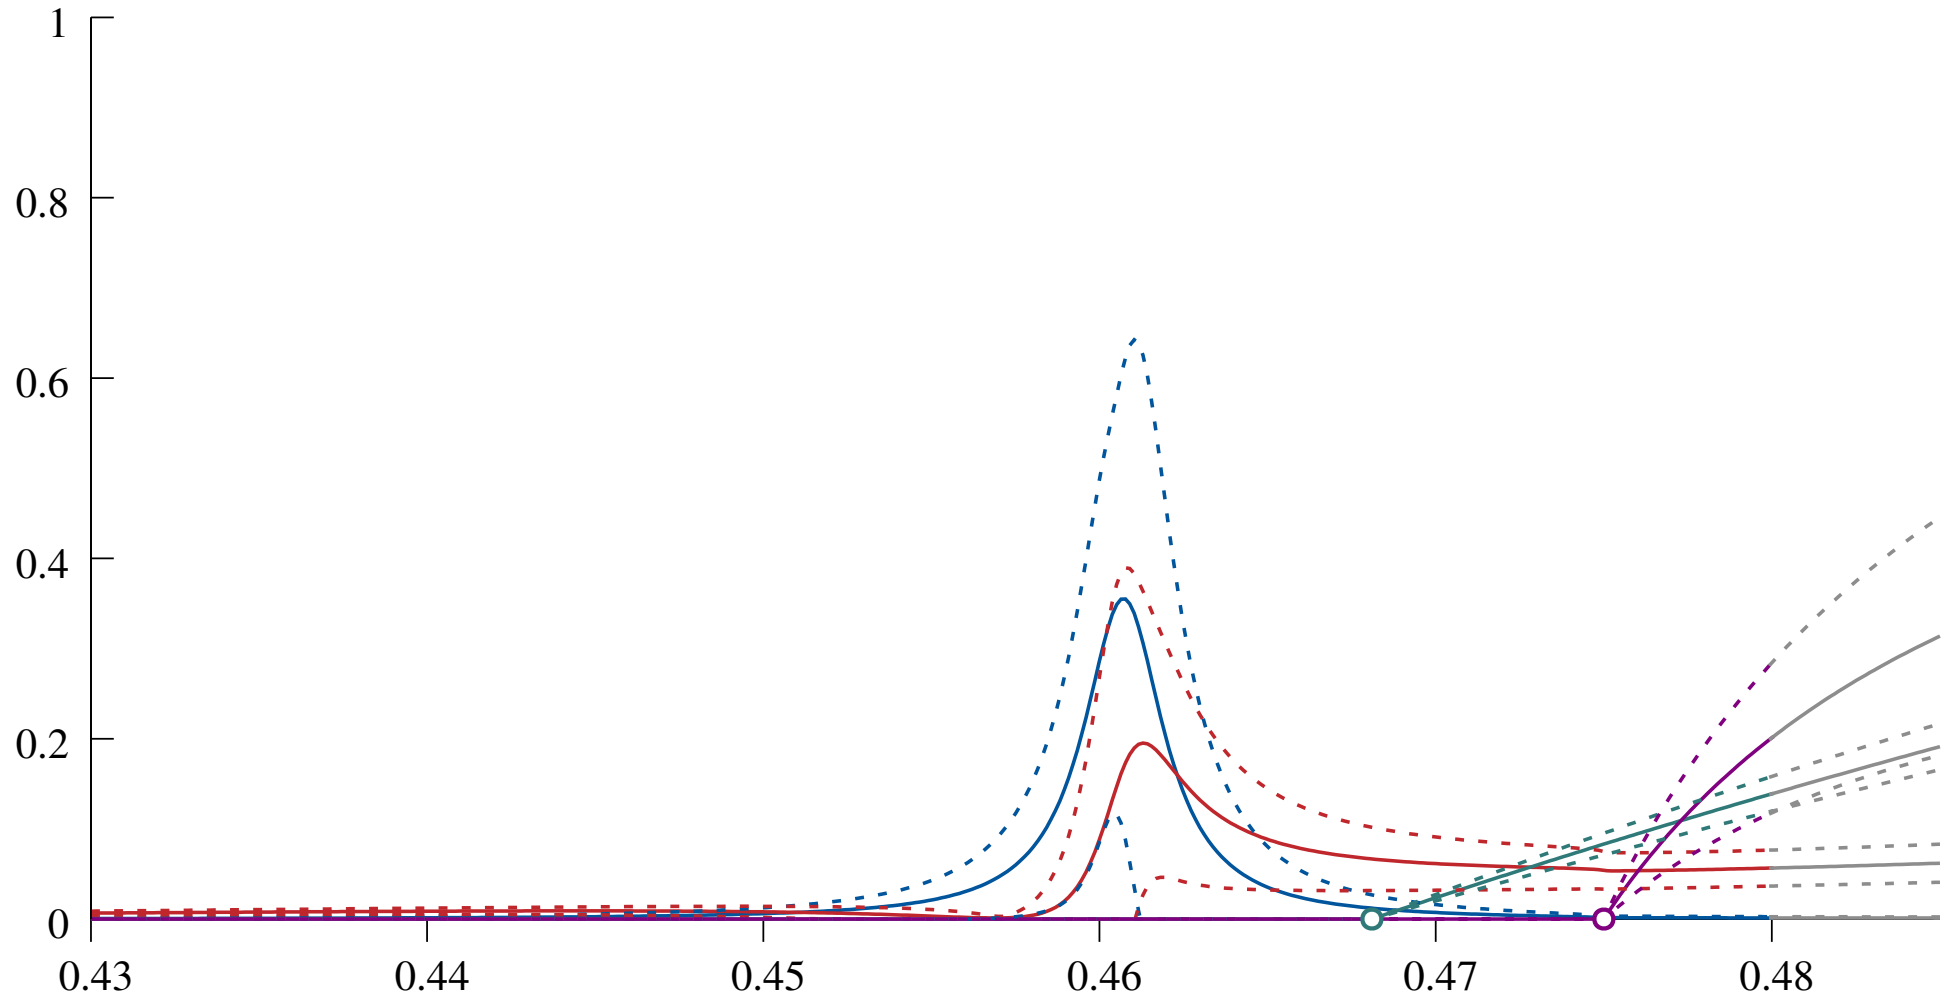

Figure 1.57: Similar to part (a) of Figure 7 in the manuscript,  $\rho_a \rho_b |t_{ab}|^2$  as a function of  $a_t E_{\text{cm}}$  for  $\eta^1 \eta^s \{^1P_1\} \rightarrow \eta^1 \eta^s \{^1P_1\}$  (blue),  $\omega^s \eta^s \{^3P_1\} \rightarrow \omega^s \eta^s \{^3P_1\}$  (red),  $f_1^s \eta^s \{^3S_1\} \rightarrow f_1^s \eta^s \{^3S_1\}$  (cyan), and  $h_1^s \eta^s \{^3S_1\} \rightarrow h_1^s \eta^s \{^3S_1\}$  (purple). Dashed lines indicate one standard deviation statistical uncertainties.

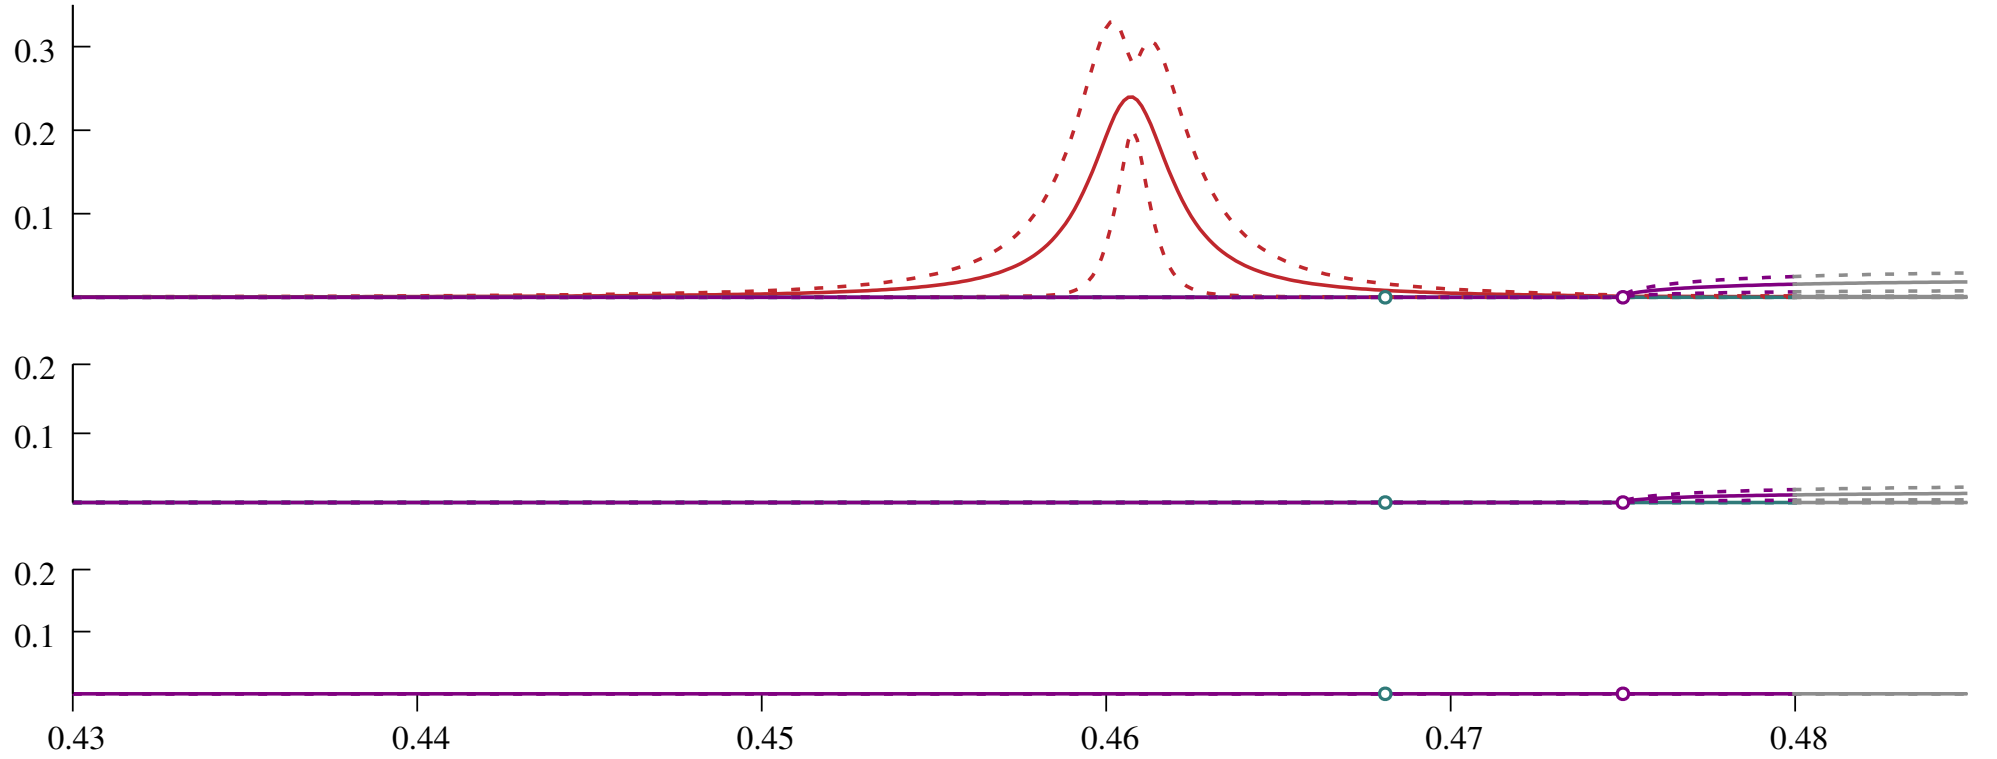

Figure 1.58: Similar to parts (b), (c) and (d) of Figure 7 in the manuscript,  $\rho_a \rho_b |t_{ab}|^2$  as a function of  $a_t E_{cm}$ . Top:  $\eta^1 \eta^s \{^1P_1\} \rightarrow \omega^s \eta^s \{^3P_1\}$  (red),  $\eta^1 \eta^s \{^1P_1\} \rightarrow f_1^s \eta^s \{^3S_1\}$  (cyan), and  $\eta^1 \eta^s \{^1P_1\} \rightarrow h_1^s \eta^s \{^3S_1\}$  (purple). Middle:  $\omega^s \eta^s \{^3P_1\} \rightarrow f_1^s \eta^s \{^3S_1\}$  (cyan), and  $\omega^s \eta^s \{^3P_1\} \rightarrow h_1^s \eta^s \{^3S_1\}$  (purple). Bottom:  $f_1^s \eta^s \{^3S_1\} \rightarrow h_1^s \eta^s \{^3S_1\}$  (purple). Dashed lines indicate one standard deviation statistical uncertainties.

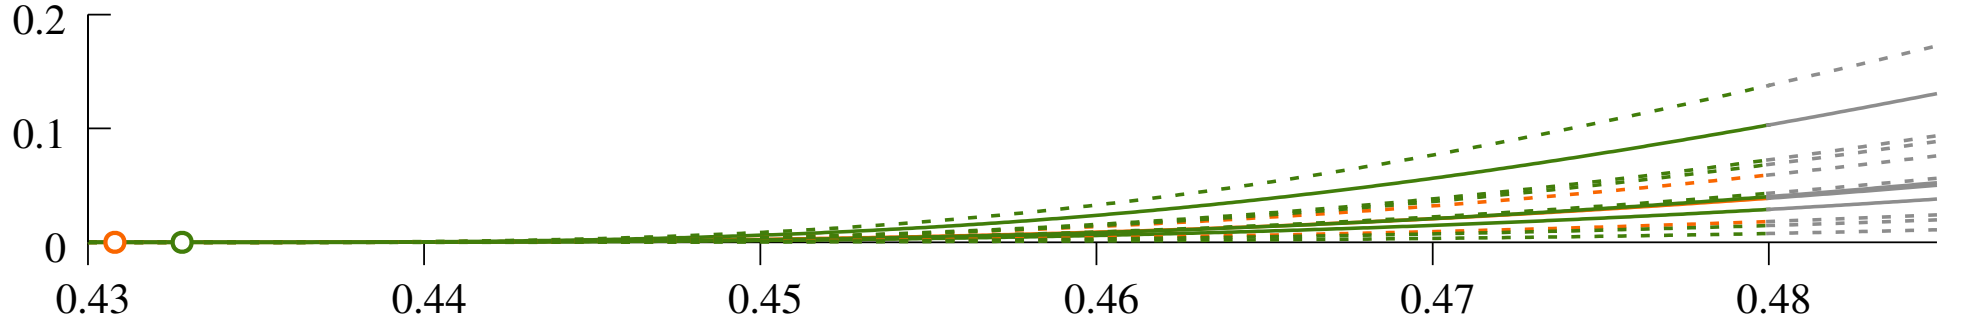

Figure 1.59: Similar to parts (e) and (f) of Figure 7 in the manuscript,  $\rho_a \rho_b |t_{ab}|^2$  as a function of  $a_t E_{cm}$  for  $\omega^s \omega^s \{^3P_1\} \rightarrow \omega^s \omega^s \{^3P_1\}$  (orange),  $\omega^1 \omega^s \{^1P_1, ^3P_1, ^5P_1\} \rightarrow \omega^s \omega^1 \{^1P_1, ^3P_1, ^5P_1\}$  (green). Dashed lines indicate one standard deviation statistical uncertainties.

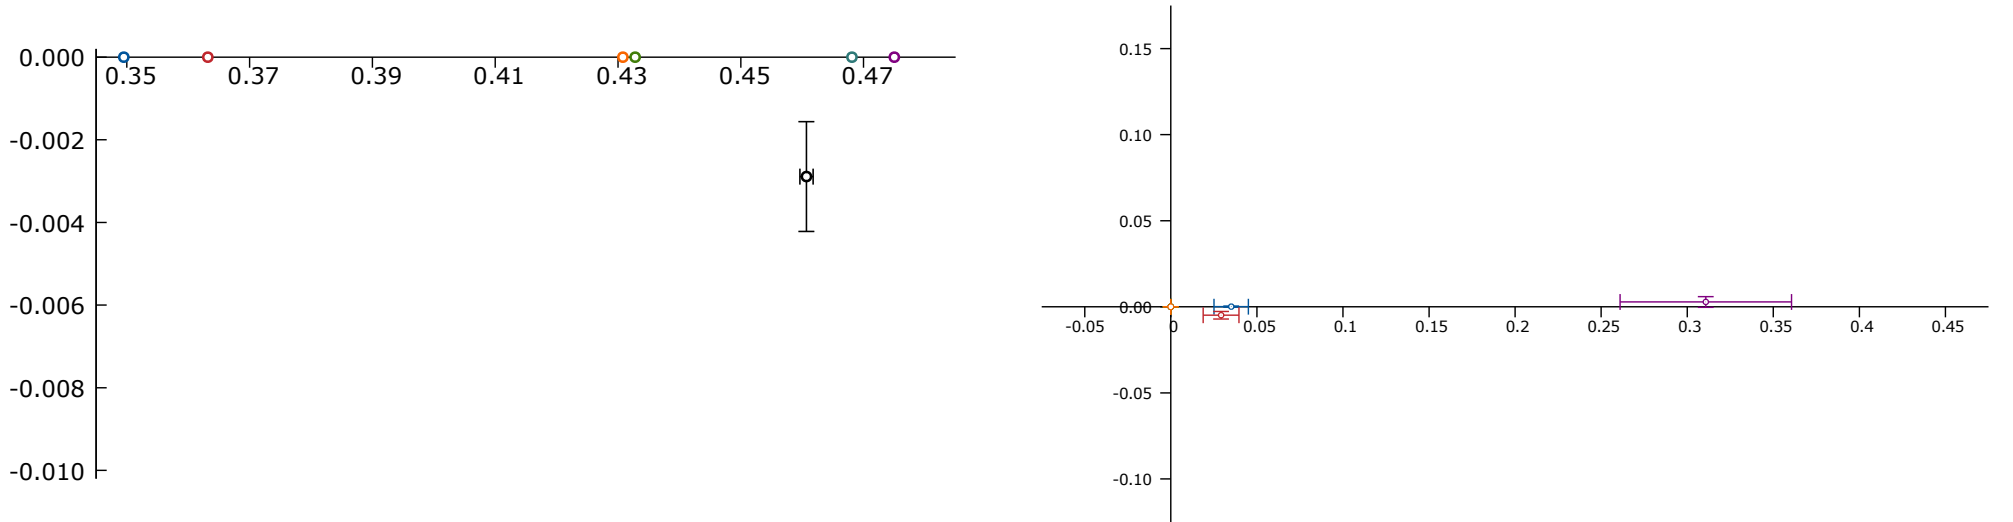

Figure 1.60: Left: Similar to Figure 13 in the manuscript, pole position on the proximal sheet (closest to physical scattering) with  $\text{Re}(a_t \sqrt{s})$  on the horizontal axis and  $2 \text{Im}(a_t \sqrt{s})$  on the vertical axis. Right: Similar to Figure 14 in the manuscript, the corresponding couplings with  $\text{Re}(a_t c)$  on the horizontal axis and  $\text{Im}(a_t c)$  on the vertical axis.

# 1.13 $\{m, g_{a,b,c,f}^{(0)}, \gamma_{(a,a),(b,b),(c,c),(\partial_1,\partial_1),(\partial_2,\partial_2),(\partial_3,\partial_3)}^{(0)}\}(\mathbf{CM}_m)$

minimised with chisq/nDoF = 43.57 / (53 - 11) = 1.04

|                                                          |  |                       |  |      |      |      |      |      |       |       |      |       |       |       |
|----------------------------------------------------------|--|-----------------------|--|------|------|------|------|------|-------|-------|------|-------|-------|-------|
| JP1-g_eta8:eta1/1^P_1_pole0                              |  | 0.27146 +/- 0.17179   |  | 1.00 | 0.89 | 0.89 | 0.80 | 0.28 | 0.00  | -0.01 | 0.08 | -0.03 | -0.05 | 0.68  |
| JP1-g_f8:eta8/3^S_1_pole0                                |  | 0.41184 +/- 0.27183   |  |      | 1.00 | 0.95 | 0.87 | 0.39 | -0.04 | -0.00 | 0.09 | -0.00 | -0.04 | 0.60  |
| JP1-g_h8:eta8/3^S_1_pole0                                |  | 0.57617 +/- 0.49928   |  |      |      | 1.00 | 0.88 | 0.47 | -0.02 | 0.03  | 0.13 | 0.03  | 0.00  | 0.57  |
| JP1-g_omega8:eta8/3^P_1_pole0                            |  | 0.29305 +/- 0.19511   |  |      |      |      | 1.00 | 0.42 | -0.35 | 0.02  | 0.07 | 0.01  | -0.00 | 0.44  |
| JP1-gamma_eta8:eta1/1^P_1 eta8:eta1/1^P_1_order0         |  | -0.25494 +/- 0.56059  |  |      |      |      |      | 1.00 | -0.02 | 0.03  | 0.10 | 0.05  | 0.03  | 0.11  |
| JP1-gamma_omega8:eta8/3^P_1 omega8:eta8/3^P_1_order0     |  | -3.9338 +/- 0.74043   |  |      |      |      |      |      | 1.00  | 0.07  | 0.11 | 0.07  | 0.12  | 0.15  |
| JP1-gamma_omega8:omega1/1^P_1 omega8:omega1/1^P_1_order0 |  | 9.4496 +/- 2.3679     |  |      |      |      |      |      |       | 1.00  | 0.07 | 0.39  | 0.44  | -0.06 |
| JP1-gamma_omega8:omega1/3^P_1 omega8:omega1/3^P_1_order0 |  | 11.082 +/- 4.9465     |  |      |      |      |      |      |       |       | 1.00 | 0.14  | 0.11  | 0.08  |
| JP1-gamma_omega8:omega1/5^P_1 omega8:omega1/5^P_1_order0 |  | 18.876 +/- 3.7311     |  |      |      |      |      |      |       |       |      | 1.00  | 0.46  | -0.08 |
| JP1-gamma_omega8:omega8/3^P_1 omega8:omega8/3^P_1_order0 |  | 10.330 +/- 2.9142     |  |      |      |      |      |      |       |       |      |       | 1.00  | -0.12 |
| JP1-m_pole0                                              |  | 0.46106 +/- 0.0011811 |  |      |      |      |      |      |       |       |      |       |       | 1.00  |

Phase space prescription ::

pole0\_sub

eta8:eta1[-] f8:eta8[+] h8:eta8[+] omega8:eta8[-] omega8:omega1[-] omega8:omega8[-] lower half-plane

sqrt(s)\_pole = (0.46091 +/- 0.0011653)  
+ (i/2)\*(-0.0036704 +/- 0.0015368) [ 0.11]

s\_pole = (0.21244 +/- 0.0010745)  
+ i\*(-0.0016917 +/- 0.00070784) [ 0.11]

| eta8:eta1                | f8:eta8                  | h8:eta8                  | omega8:eta8              | omega8:omega1            | omega8:omega8            |
|--------------------------|--------------------------|--------------------------|--------------------------|--------------------------|--------------------------|
| k_re= 0.1492 +/- 0.0009  | k_re= -0.0047 +/- 0.0019 | k_re= -0.0033 +/- 0.0014 | k_re= 0.1404 +/- 0.0009  | k_re= 0.0793 +/- 0.0017  | k_re= 0.0820 +/- 0.0016  |
| k_im= -0.0014 +/- 0.0006 | k_im= 0.0382 +/- 0.0030  | k_im= 0.0530 +/- 0.0021  | k_im= -0.0015 +/- 0.0006 | k_im= -0.0027 +/- 0.0011 | k_im= -0.0026 +/- 0.0011 |
| corr= [ 0.12]            | corr= [ 0.00]            | corr= [-0.05]            | corr= [ 0.12]            | corr= [ 0.14]            | corr= [ 0.13]            |

  

| eta8:eta1/1^P_1              | f8:eta8/3^S_1                | h8:eta8/3^S_1(*)             | omega8:eta8/3^P_1             | omega8:omega1/1^P_1          | omega8:omega1/3^P_1          | omega8:omega1/5^P_1          | omega8:omega8/3^P_1          |
|------------------------------|------------------------------|------------------------------|-------------------------------|------------------------------|------------------------------|------------------------------|------------------------------|
| g = 0.0368 +/- 0.0102        | g = 0.1873 +/- 0.0253        | g = 0.2620 +/- 0.0667        | g = 0.0366 +/- 0.0114         | g = 0.0000 +/- 0.0000        | g = 0.0000 +/- 0.0000        | g = 0.0000 +/- 0.0000        | g = 0.0000 +/- 0.0000        |
| arg(g)/pi= 0.0017 +/- 0.0120 | arg(g)/pi= 0.0094 +/- 0.0057 | arg(g)/pi= 0.0094 +/- 0.0057 | arg(g)/pi= -0.0534 +/- 0.0108 | arg(g)/pi= 0.4906 +/- 0.0057 | arg(g)/pi= 0.4906 +/- 0.0057 | arg(g)/pi= 0.4906 +/- 0.0057 | arg(g)/pi= 0.4906 +/- 0.0057 |
| g_re= 0.0368 +/- 0.0102      | g_re= 0.1873 +/- 0.0252      | g_re= 0.2619 +/- 0.0666      | g_re= 0.0361 +/- 0.0112       | g_re= 0.0000 +/- 0.0000      | g_re= 0.0000 +/- 0.0000      | g_re= 0.0000 +/- 0.0000      | g_re= 0.0000 +/- 0.0000      |
| g_im= 0.0002 +/- 0.0014      | g_im= 0.0055 +/- 0.0037      | g_im= 0.0077 +/- 0.0058      | g_im= -0.0061 +/- 0.0028      | g_im= 0.0000 +/- 0.0000      | g_im= 0.0000 +/- 0.0000      | g_im= 0.0000 +/- 0.0000      | g_im= 0.0000 +/- 0.0000      |
| corr= [-0.16]                | corr= [ 0.56]                | corr= [ 0.70]                | corr= [-0.92]                 | corr= [-0.04]                | corr= [-0.04]                | corr= [-0.04]                | corr= [-0.04]                |

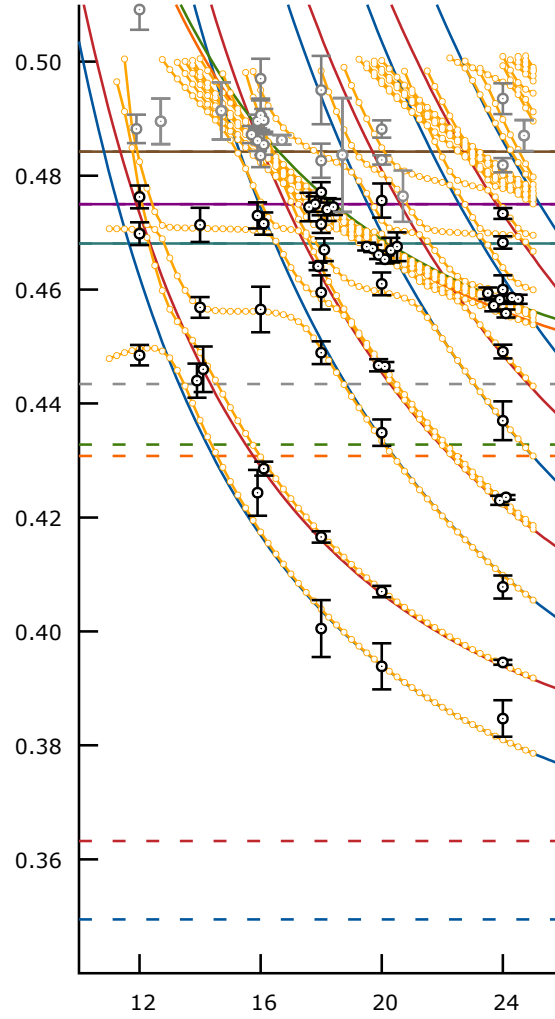

Figure 1.61: Similar to Figure 6 in the manuscript, the finite-volume spectrum, plotted as  $a_t E_{\text{cm}}$ , as a function of spatial extent  $L/a_s$ . Orange points/curves show the spectrum calculated from the amplitude given above (no uncertainties are shown). Black and grey points are the computed lattice energies on each volume, slightly displaced horizontally for clarity (black points correspond to energies used in the fit whereas grey points were not used). Two-meson non-interacting energies are shown as solid coloured curves/lines, two-meson thresholds are shown as dashed/solid horizontal lines, and the  $\eta^s \eta^s \eta^s$  threshold is shown as a dashed grey horizontal line.

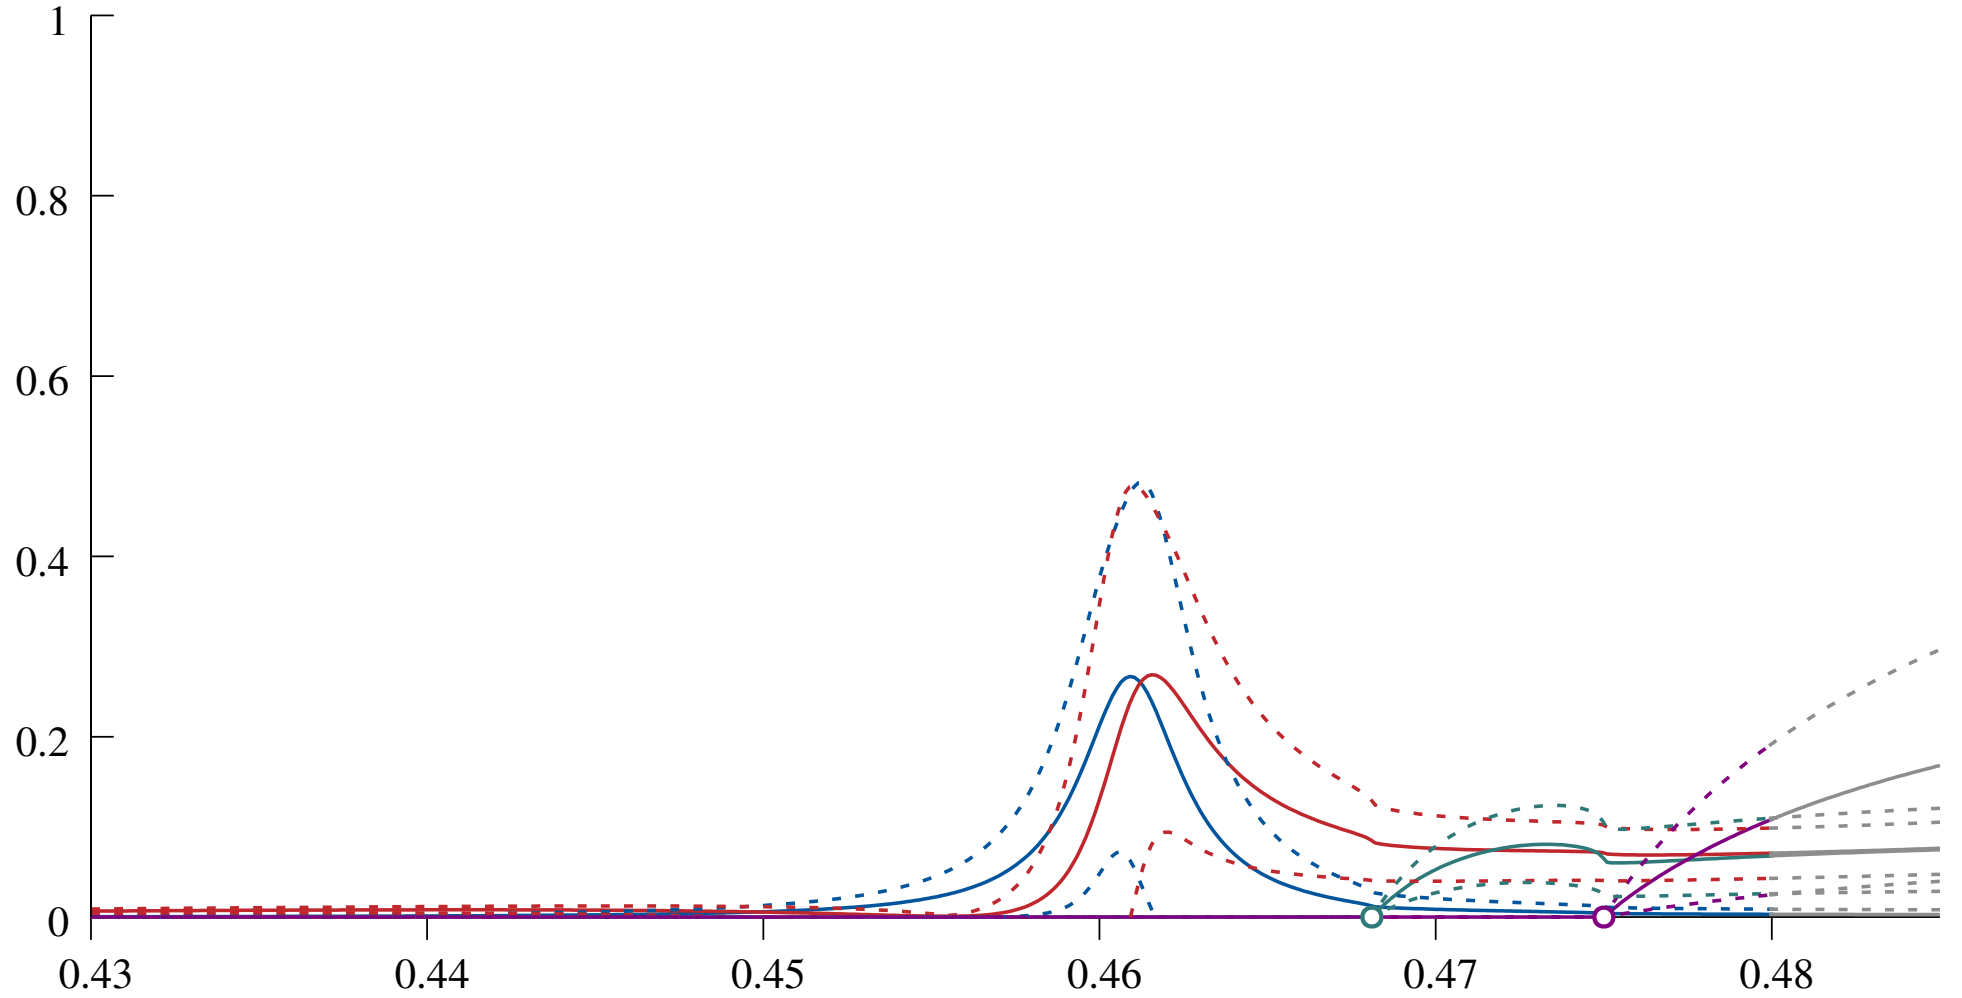

Figure 1.62: Similar to part (a) of Figure 7 in the manuscript,  $\rho_a \rho_b |t_{ab}|^2$  as a function of  $a_t E_{cm}$  for  $\eta^1 \eta^s \{^1P_1\} \rightarrow \eta^1 \eta^s \{^1P_1\}$  (blue),  $\omega^s \eta^s \{^3P_1\} \rightarrow \omega^s \eta^s \{^3P_1\}$  (red),  $f_1^s \eta^s \{^3S_1\} \rightarrow f_1^s \eta^s \{^3S_1\}$  (cyan), and  $h_1^s \eta^s \{^3S_1\} \rightarrow h_1^s \eta^s \{^3S_1\}$  (purple). Dashed lines indicate one standard deviation statistical uncertainties.

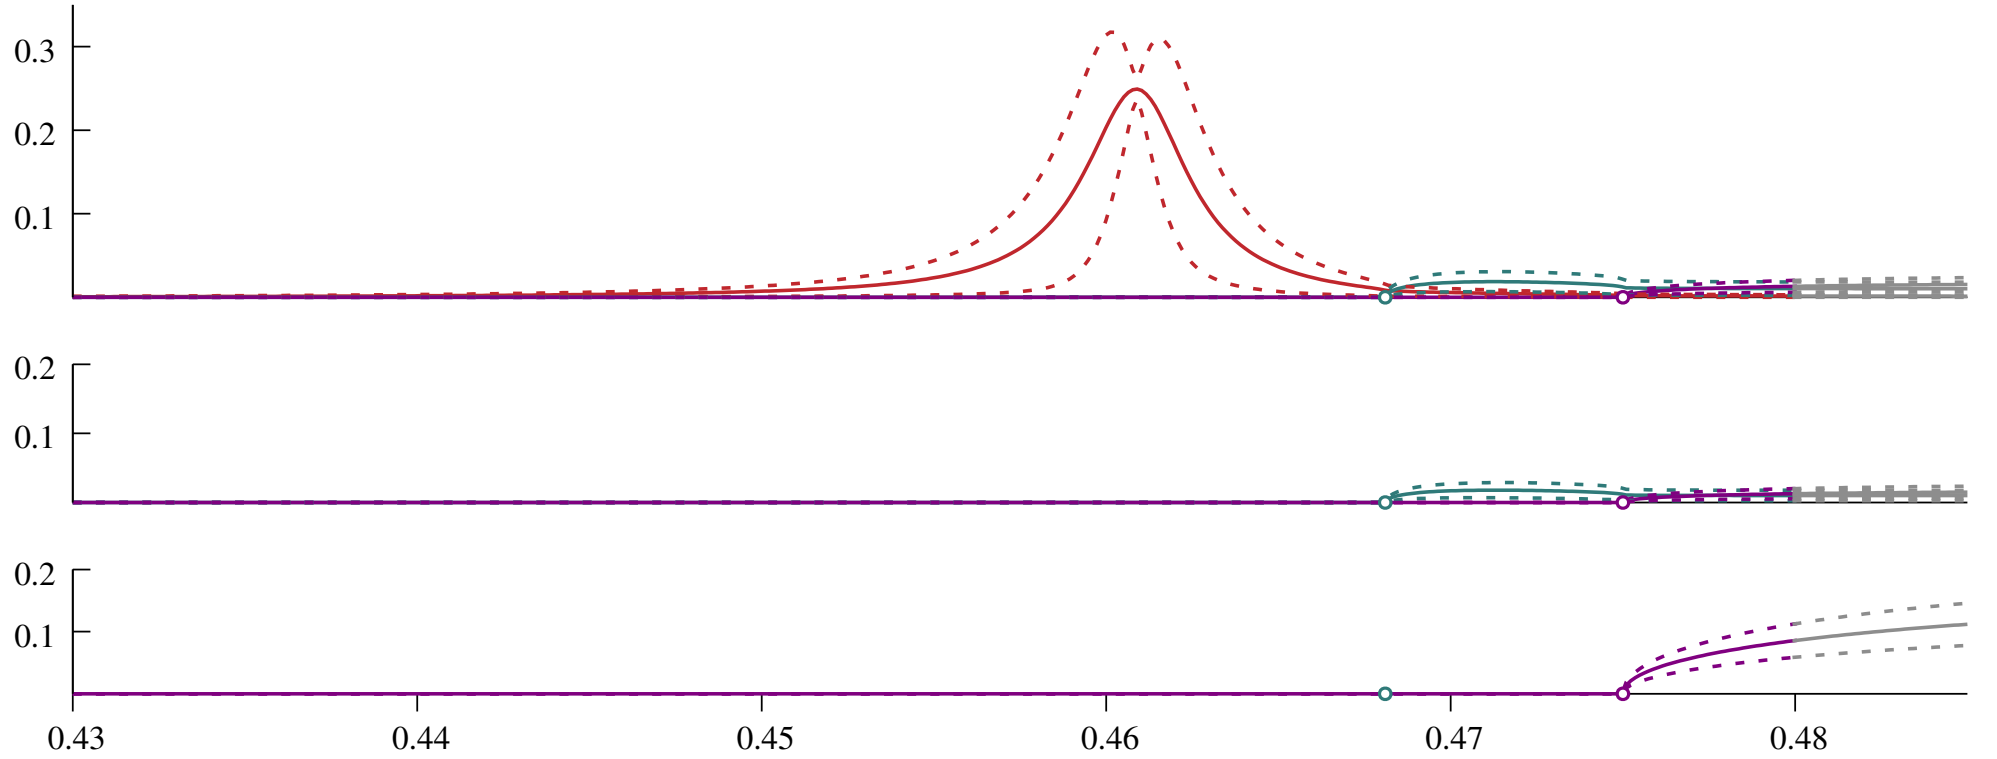

Figure 1.63: Similar to parts (b), (c) and (d) of Figure 7 in the manuscript,  $\rho_a \rho_b |t_{ab}|^2$  as a function of  $a_t E_{\text{cm}}$ . Top:  $\eta^1 \eta^s \{^1P_1\} \rightarrow \omega^s \eta^s \{^3P_1\}$  (red),  $\eta^1 \eta^s \{^1P_1\} \rightarrow f_1^s \eta^s \{^3S_1\}$  (cyan), and  $\eta^1 \eta^s \{^1P_1\} \rightarrow h_1^s \eta^s \{^3S_1\}$  (purple). Middle:  $\omega^s \eta^s \{^3P_1\} \rightarrow f_1^s \eta^s \{^3S_1\}$  (cyan), and  $\omega^s \eta^s \{^3P_1\} \rightarrow h_1^s \eta^s \{^3S_1\}$  (purple). Bottom:  $f_1^s \eta^s \{^3S_1\} \rightarrow h_1^s \eta^s \{^3S_1\}$  (purple). Dashed lines indicate one standard deviation statistical uncertainties.

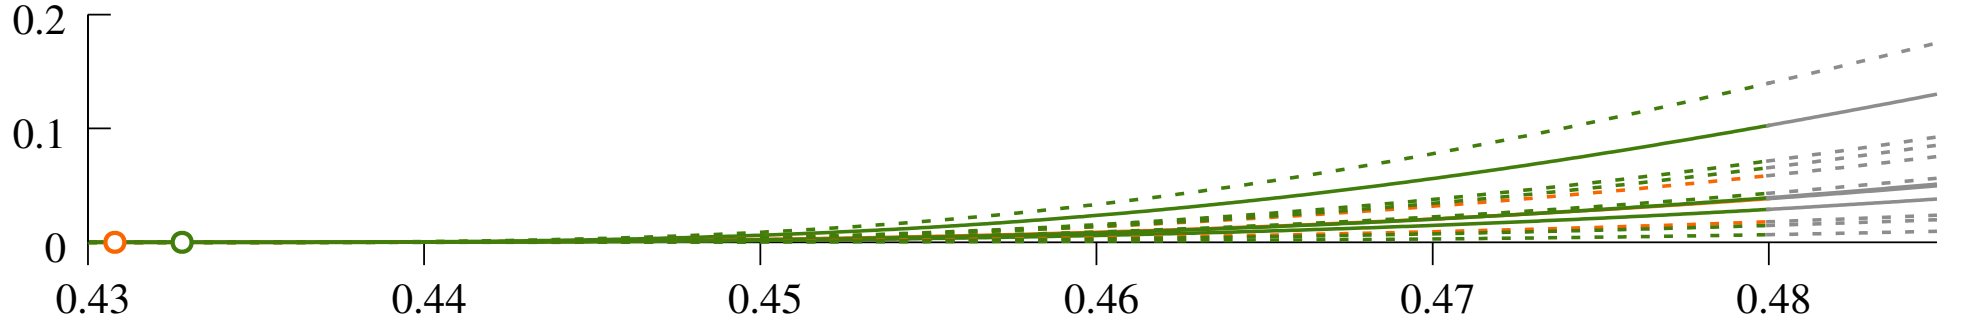

Figure 1.64: Similar to parts (e) and (f) of Figure 7 in the manuscript,  $\rho_a \rho_b |t_{ab}|^2$  as a function of  $a_t E_{cm}$  for  $\omega^s \omega^s \{^3P_1\} \rightarrow \omega^s \omega^s \{^3P_1\}$  (orange),  $\omega^1 \omega^s \{^1P_1, ^3P_1, ^5P_1\} \rightarrow \omega^s \omega^1 \{^1P_1, ^3P_1, ^5P_1\}$  (green). Dashed lines indicate one standard deviation statistical uncertainties.

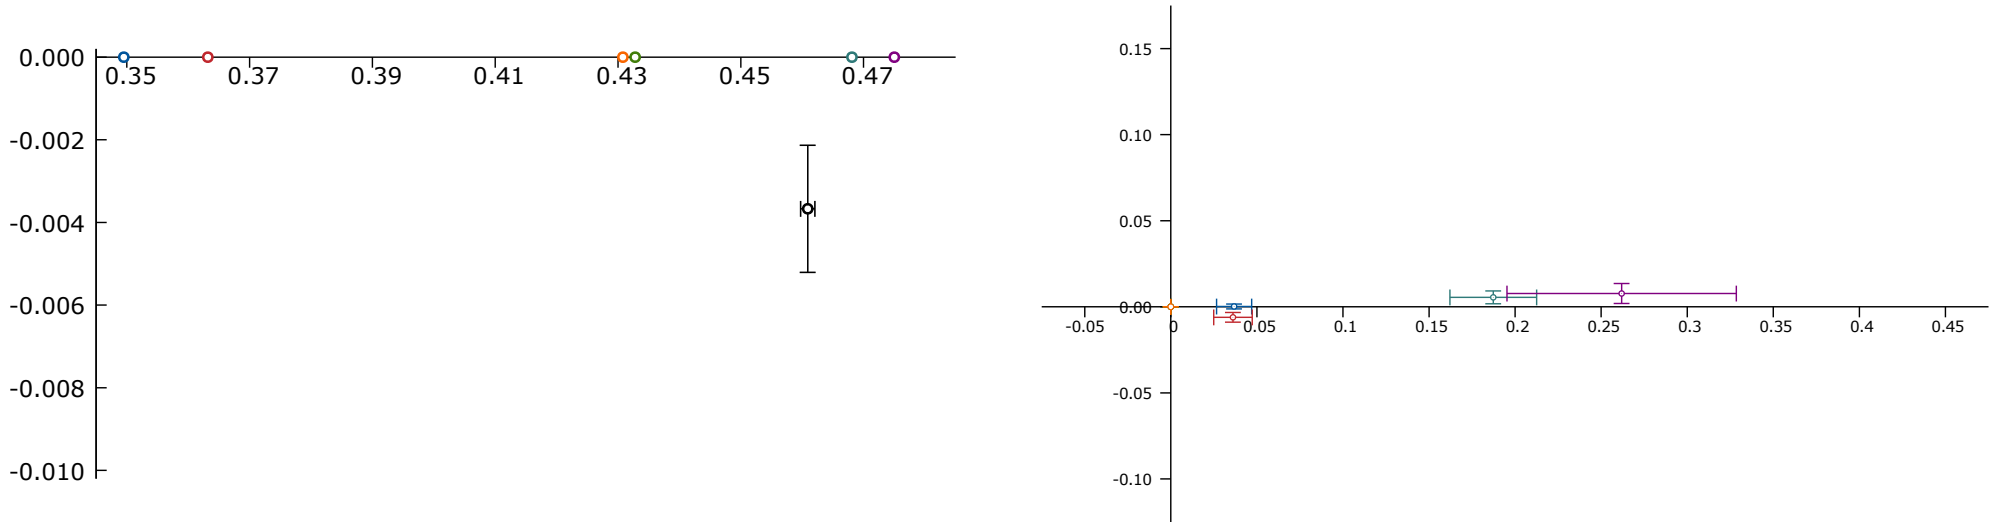

Figure 1.65: Left: Similar to Figure 13 in the manuscript, pole position on the proximal sheet (closest to physical scattering) with  $\text{Re}(a_t \sqrt{s})$  on the horizontal axis and  $2 \text{Im}(a_t \sqrt{s})$  on the vertical axis. Right: Similar to Figure 14 in the manuscript, the corresponding couplings with  $\text{Re}(a_t c)$  on the horizontal axis and  $\text{Im}(a_t c)$  on the vertical axis.

# 1.14 $\{m, g_{a,b,c,f}^{(0)}, \gamma_{(a,a),(b,b),(c,c),(\partial_1,\partial_1),(\partial_2,\partial_2),(\partial_3,\partial_3),(\epsilon,\epsilon)}^{(0)}\}(\mathbf{CM}_{thr})$

minimised with chisq/nDoF = 46.26 / (53 - 12) = 1.13

|                                                           |  |                      |  |      |       |       |       |       |       |       |       |       |       |       |       |
|-----------------------------------------------------------|--|----------------------|--|------|-------|-------|-------|-------|-------|-------|-------|-------|-------|-------|-------|
| =====                                                     |  |                      |  |      |       |       |       |       |       |       |       |       |       |       |       |
| JP1-_g_eta8:eta1/1^P_1_pole0                              |  | 0.20784 +/- 0.13912  |  | 1.00 | -0.76 | 0.66  | 0.71  | 0.15  | 0.22  | 0.00  | -0.03 | 0.03  | -0.06 | -0.04 | -0.76 |
| JP1-_g_h8:eta8/3^S_1_pole0                                |  | -0.75900 +/- 0.54818 |  |      | 1.00  | -0.88 | -0.84 | -0.32 | -0.37 | 0.07  | -0.03 | -0.07 | -0.02 | -0.02 | 1.00  |
| JP1-_g_omega8:eta8/3^P_1_pole0                            |  | 0.23147 +/- 0.15007  |  |      |       | 1.00  | 0.77  | 0.31  | 0.35  | -0.29 | 0.04  | 0.06  | 0.03  | 0.04  | -0.88 |
| JP1-_g_omega8:omega8/3^P_1_pole0                          |  | 0.37734 +/- 0.25462  |  |      |       |       | 1.00  | 0.27  | 0.32  | -0.02 | -0.08 | 0.06  | -0.08 | 0.01  | -0.84 |
| JP1-_gamma_eta8:eta1/1^P_1 eta8:eta1/1^P_1_order0         |  | 1.4861 +/- 0.62683   |  |      |       |       | 1.00  | 0.56  | -0.01 | 0.02  | 0.06  | 0.02  | 0.01  | -0.32 |       |
| JP1-_gamma_f8:eta8/3^S_1 f8:eta8/3^S_1_order0             |  | -1.6029 +/- 0.17795  |  |      |       |       |       | 1.00  | -0.01 | 0.04  | 0.07  | 0.04  | 0.03  | -0.38 |       |
| JP1-_gamma_omega8:eta8/3^P_1 omega8:eta8/3^P_1_order0     |  | -3.2790 +/- 0.54824  |  |      |       |       |       |       | 1.00  | 0.03  | 0.08  | 0.08  | 0.08  | 0.08  |       |
| JP1-_gamma_omega8:omega1/1^P_1 omega8:omega1/1^P_1_order0 |  | 9.3795 +/- 2.5323    |  |      |       |       |       |       |       | 1.00  | 0.06  | 0.49  | 0.36  | -0.03 |       |
| JP1-_gamma_omega8:omega1/3^P_1 omega8:omega1/3^P_1_order0 |  | 12.650 +/- 5.1914    |  |      |       |       |       |       |       |       | 1.00  | 0.11  | 0.12  | -0.07 |       |
| JP1-_gamma_omega8:omega1/5^P_1 omega8:omega1/5^P_1_order0 |  | 27.315 +/- 4.4064    |  |      |       |       |       |       |       |       |       | 1.00  | 0.45  | -0.02 |       |
| JP1-_gamma_omega8:omega8/3^P_1 omega8:omega8/3^P_1_order0 |  | 6.7390 +/- 3.1515    |  |      |       |       |       |       |       |       |       |       | 1.00  | -0.02 |       |
| JP1-_m_pole0                                              |  | 0.30712 +/- 0.27092  |  |      |       |       |       |       |       |       |       |       |       |       | 1.00  |
| =====                                                     |  |                      |  |      |       |       |       |       |       |       |       |       |       |       |       |

Phase space prescription ::

threshold\_sub

eta8:eta1[-] f8:eta8[+] h8:eta8[-] omega8:eta8[-] omega8:omega1[-] omega8:omega8[-] lower half-plane

sqrt(s)\_pole = (0.46045 +/- 0.0022426)  
+ (i/2)\*(-0.0030021 +/- 0.0014244) [ 0.13]

s\_pole = (0.21201 +/- 0.0020659)  
+ i\*(-0.0013823 +/- 0.00065501) [ 0.13]

| eta8:eta1                | f8:eta8                  | h8:eta8                  | omega8:eta8              | omega8:omega1            | omega8:omega8            |
|--------------------------|--------------------------|--------------------------|--------------------------|--------------------------|--------------------------|
| k_re= 0.1489 +/- 0.0017  | k_re= -0.0038 +/- 0.0018 | k_re= -0.0027 +/- 0.0013 | k_re= 0.1400 +/- 0.0018  | k_re= 0.0786 +/- 0.0033  | k_re= 0.0813 +/- 0.0032  |
| k_im= -0.0012 +/- 0.0005 | k_im= 0.0393 +/- 0.0056  | k_im= 0.0538 +/- 0.0040  | k_im= -0.0012 +/- 0.0006 | k_im= -0.0022 +/- 0.0011 | k_im= -0.0021 +/- 0.0010 |
| corr= [ 0.15]            | corr= [ 0.16]            | corr= [ 0.03]            | corr= [ 0.15]            | corr= [ 0.20]            | corr= [ 0.20]            |

  

| eta8:eta1/1^P_1               | f8:eta8/3^S_1                | h8:eta8/3^S_1(*)             | omega8:eta8/3^P_1            | omega8:omega1/1^P_1          | omega8:omega1/3^P_1          | omega8:omega1/5^P_1          | omega8:omega8/3^P_1           |
|-------------------------------|------------------------------|------------------------------|------------------------------|------------------------------|------------------------------|------------------------------|-------------------------------|
| g = 0.0275 +/- 0.0119         | g = 0.0000 +/- 0.0000        | g = 0.3524 +/- 0.0528        | g = 0.0318 +/- 0.0099        | g = 0.0000 +/- 0.0000        | g = 0.0000 +/- 0.0000        | g = 0.0000 +/- 0.0000        | g = 0.0282 +/- 0.0111         |
| arg(g)/pi= -0.9734 +/- 0.0112 | arg(g)/pi= 0.4973 +/- 0.0033 | arg(g)/pi= 0.0027 +/- 0.0033 | arg(g)/pi= 0.9465 +/- 0.0099 | arg(g)/pi= 0.4973 +/- 0.0033 | arg(g)/pi= 0.4973 +/- 0.0033 | arg(g)/pi= 0.4973 +/- 0.0033 | arg(g)/pi= -0.9854 +/- 0.0114 |
| g_re= -0.0274 +/- 0.0119      | g_re= 0.0000 +/- 0.0000      | g_re= 0.3524 +/- 0.0528      | g_re= -0.0313 +/- 0.0097     | g_re= 0.0000 +/- 0.0000      | g_re= 0.0000 +/- 0.0000      | g_re= 0.0000 +/- 0.0000      | g_re= -0.0281 +/- 0.0111      |
| g_im= -0.0023 +/- 0.0012      | g_im= 0.0000 +/- 0.0000      | g_im= 0.0030 +/- 0.0040      | g_im= 0.0053 +/- 0.0023      | g_im= 0.0000 +/- 0.0000      | g_im= 0.0000 +/- 0.0000      | g_im= 0.0000 +/- 0.0000      | g_im= -0.0013 +/- 0.0010      |
| corr= [ 0.65]                 | corr= [-0.51]                | corr= [ 0.67]                | corr= [-0.93]                | corr= [-0.51]                | corr= [-0.51]                | corr= [-0.51]                | corr= [ 0.20]                 |

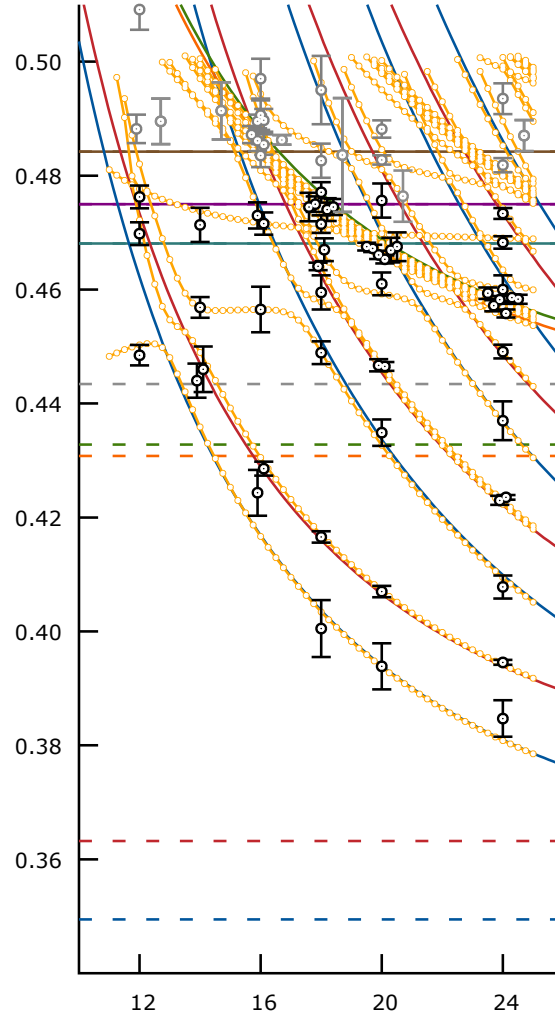

Figure 1.66: Similar to Figure 6 in the manuscript, the finite-volume spectrum, plotted as  $a_t E_{\text{cm}}$ , as a function of spatial extent  $L/a_s$ . Orange points/curves show the spectrum calculated from the amplitude given above (no uncertainties are shown). Black and grey points are the computed lattice energies on each volume, slightly displaced horizontally for clarity (black points correspond to energies used in the fit whereas grey points were not used). Two-meson non-interacting energies are shown as solid coloured curves/lines, two-meson thresholds are shown as dashed/solid horizontal lines, and the  $\eta^s \eta^s \eta^s$  threshold is shown as a dashed grey horizontal line.

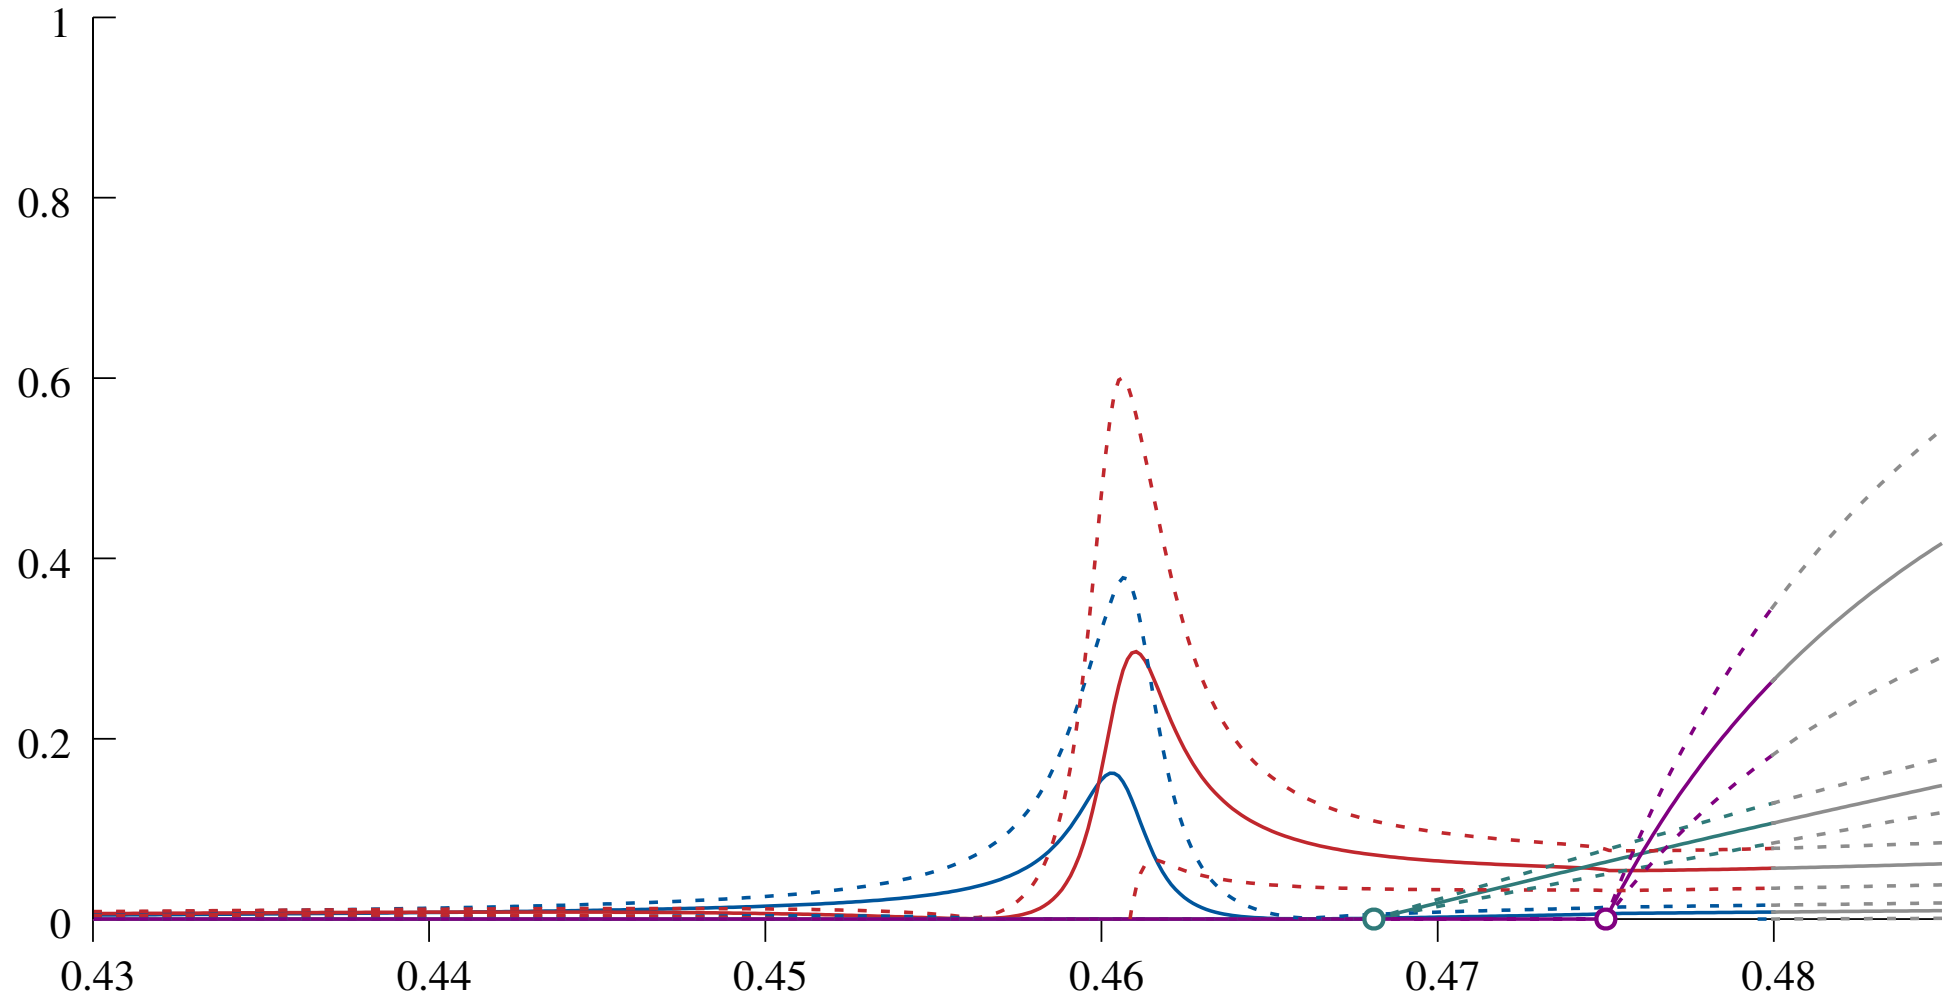

Figure 1.67: Similar to part (a) of Figure 7 in the manuscript,  $\rho_a \rho_b |t_{ab}|^2$  as a function of  $a_t E_{cm}$  for  $\eta^1 \eta^s \{^1P_1\} \rightarrow \eta^1 \eta^s \{^1P_1\}$  (blue),  $\omega^s \eta^s \{^3P_1\} \rightarrow \omega^s \eta^s \{^3P_1\}$  (red),  $f_1^s \eta^s \{^3S_1\} \rightarrow f_1^s \eta^s \{^3S_1\}$  (cyan), and  $h_1^s \eta^s \{^3S_1\} \rightarrow h_1^s \eta^s \{^3S_1\}$  (purple). Dashed lines indicate one standard deviation statistical uncertainties.

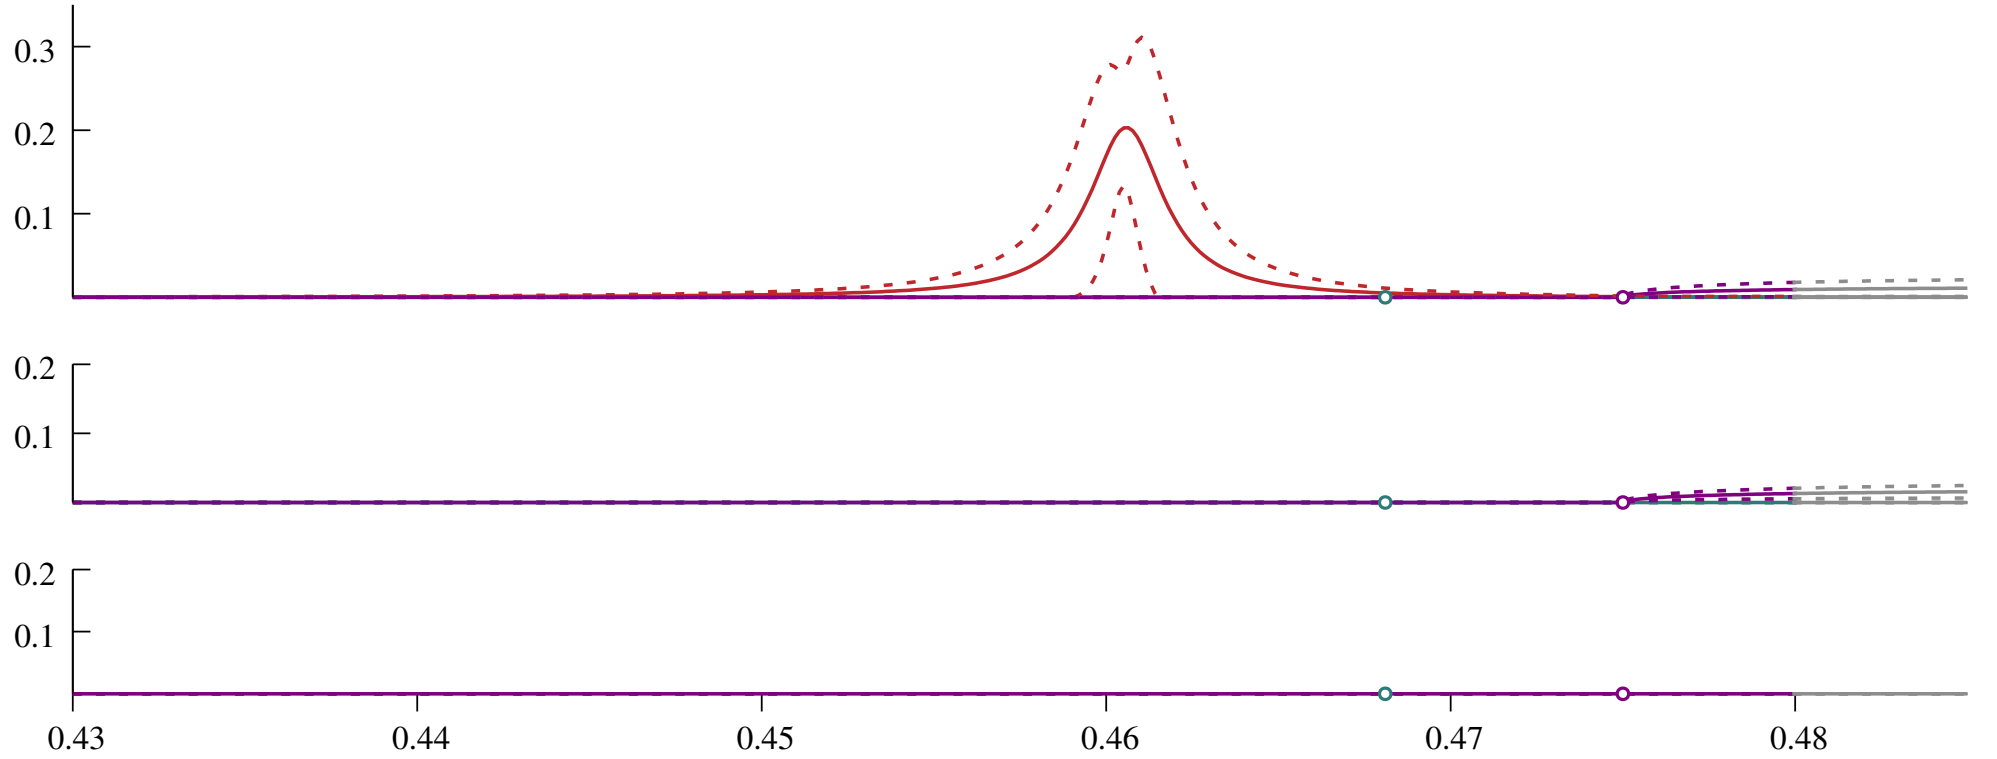

Figure 1.68: Similar to parts (b), (c) and (d) of Figure 7 in the manuscript,  $\rho_a \rho_b |t_{ab}|^2$  as a function of  $a_t E_{\text{cm}}$ . Top:  $\eta^1 \eta^s \{^1P_1\} \rightarrow \omega^s \eta^s \{^3P_1\}$  (red),  $\eta^1 \eta^s \{^1P_1\} \rightarrow f_1^s \eta^s \{^3S_1\}$  (cyan), and  $\eta^1 \eta^s \{^1P_1\} \rightarrow h_1^s \eta^s \{^3S_1\}$  (purple). Middle:  $\omega^s \eta^s \{^3P_1\} \rightarrow f_1^s \eta^s \{^3S_1\}$  (cyan), and  $\omega^s \eta^s \{^3P_1\} \rightarrow h_1^s \eta^s \{^3S_1\}$  (purple). Bottom:  $f_1^s \eta^s \{^3S_1\} \rightarrow h_1^s \eta^s \{^3S_1\}$  (purple). Dashed lines indicate one standard deviation statistical uncertainties.

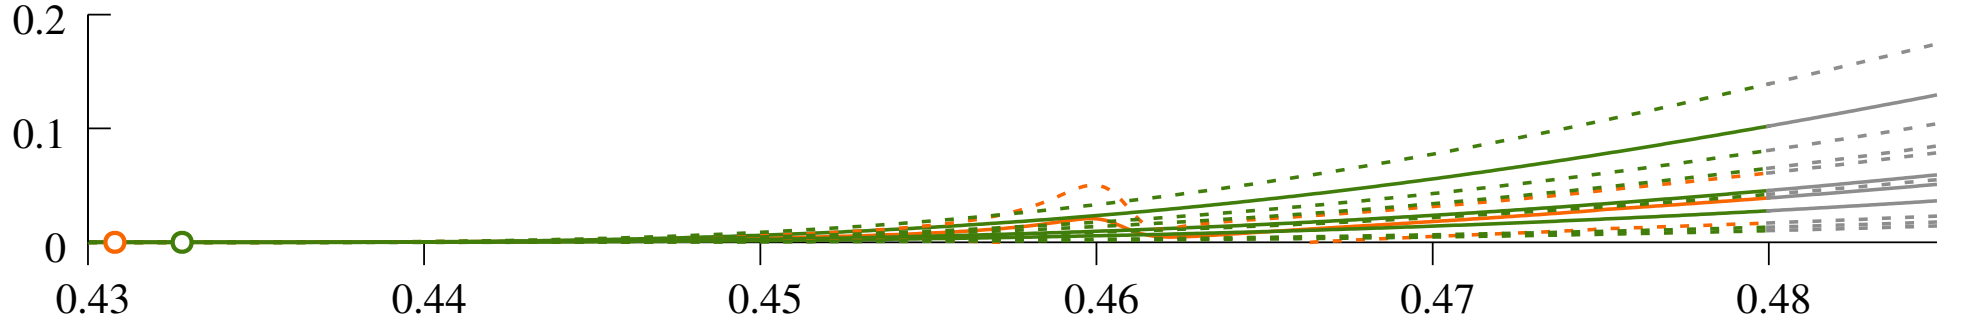

Figure 1.69: Similar to parts (e) and (f) of Figure 7 in the manuscript,  $\rho_a \rho_b |t_{ab}|^2$  as a function of  $a_t E_{cm}$  for  $\omega^s \omega^s \{^3P_1\} \rightarrow \omega^s \omega^s \{^3P_1\}$  (orange),  $\omega^1 \omega^s \{^1P_1, ^3P_1, ^5P_1\} \rightarrow \omega^s \omega^1 \{^1P_1, ^3P_1, ^5P_1\}$  (green). Dashed lines indicate one standard deviation statistical uncertainties.

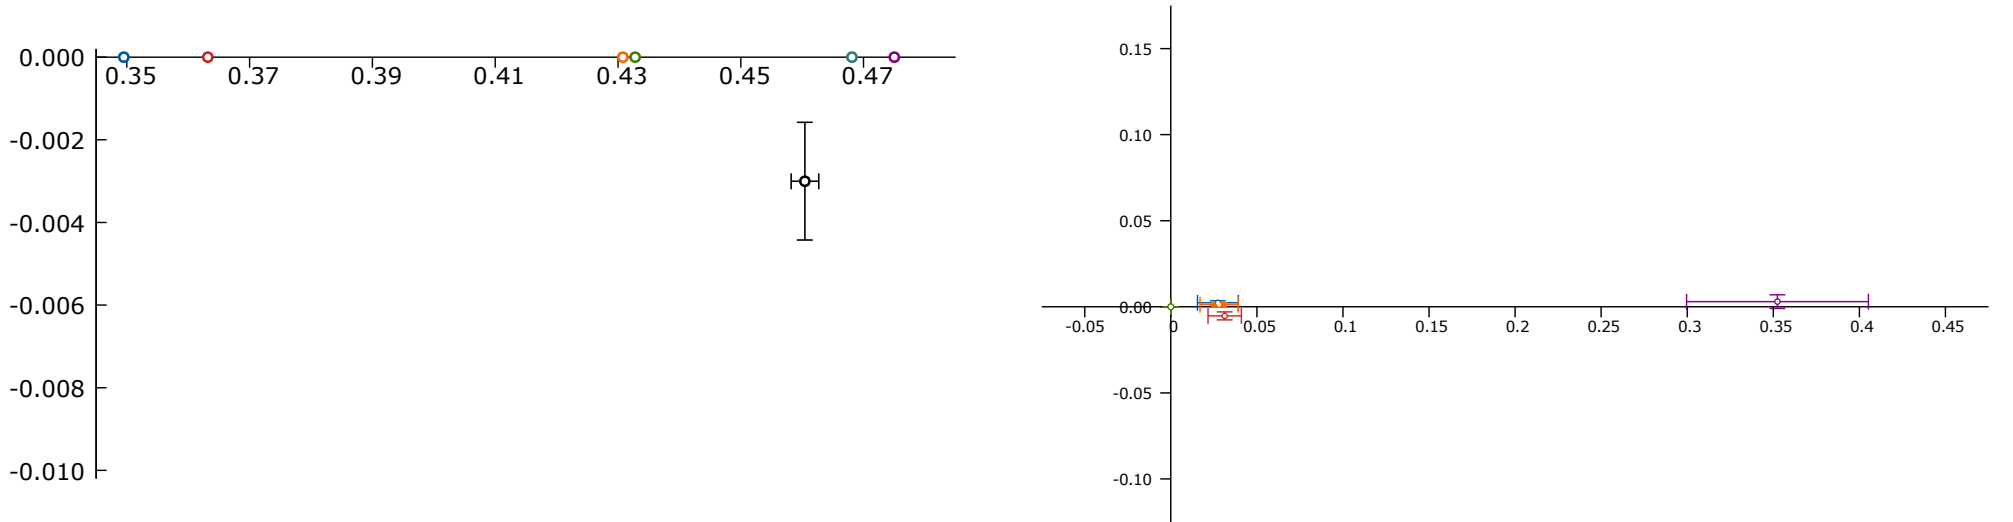

Figure 1.70: Left: Similar to Figure 13 in the manuscript, pole position on the proximal sheet (closest to physical scattering) with  $\text{Re}(a_t \sqrt{s})$  on the horizontal axis and  $2 \text{Im}(a_t \sqrt{s})$  on the vertical axis. Right: Similar to Figure 14 in the manuscript, the corresponding couplings with  $\text{Re}(a_t c)$  on the horizontal axis and  $\text{Im}(a_t c)$  on the vertical axis.

# 1.15 $\{m, g_f^{(0)}, \gamma_{(a,a),(b,b),(c,c),(\partial_1,\partial_1),(\partial_2,\partial_2),(\partial_3,\partial_3),(\epsilon,\epsilon)}^{(0)}\}(\mathbf{CM}_{thr})$

minimised with chisq/nDoF = 50.52 / (53 - 9) = 1.15

|                                                           |  |                     |  |      |      |      |      |      |      |      |       |       |
|-----------------------------------------------------------|--|---------------------|--|------|------|------|------|------|------|------|-------|-------|
| =====                                                     |  |                     |  |      |      |      |      |      |      |      |       |       |
| JP1-_g_h8:eta8/3^S_1_pole0                                |  | 0.75725 +/- 0.25536 |  | 1.00 | 0.18 | 0.21 | 0.04 | 0.00 | 0.03 | 0.00 | -0.00 | -1.00 |
| JP1-_gamma_eta8:eta1/1^P_1 eta8:eta1/1^P_1_order0         |  | 1.5137 +/- 0.5597   |  |      | 1.00 | 0.50 | 0.08 | 0.01 | 0.04 | 0.01 | 0.00  | -0.19 |
| JP1-_gamma_f8:eta8/3^S_1 f8:eta8/3^S_1_order0             |  | -1.6027 +/- 0.166   |  |      |      | 1.00 | 0.08 | 0.03 | 0.05 | 0.03 | 0.04  | -0.21 |
| JP1-_gamma_omega8:eta8/3^P_1 omega8:eta8/3^P_1_order0     |  | -2.9220 +/- 0.46498 |  |      |      |      | 1.00 | 0.09 | 0.09 | 0.10 | 0.18  | -0.04 |
| JP1-_gamma_omega8:omega1/1^P_1 omega8:omega1/1^P_1_order0 |  | 9.7661 +/- 2.4675   |  |      |      |      |      | 1.00 | 0.05 | 0.38 | 0.43  | -0.00 |
| JP1-_gamma_omega8:omega1/3^P_1 omega8:omega1/3^P_1_order0 |  | 12.699 +/- 5.1826   |  |      |      |      |      |      | 1.00 | 0.13 | 0.09  | -0.03 |
| JP1-_gamma_omega8:omega1/5^P_1 omega8:omega1/5^P_1_order0 |  | 20.491 +/- 4.094    |  |      |      |      |      |      |      | 1.00 | 0.45  | -0.00 |
| JP1-_gamma_omega8:omega8/3^P_1 omega8:omega8/3^P_1_order0 |  | 10.956 +/- 3.047    |  |      |      |      |      |      |      |      | 1.00  | -0.00 |
| JP1-_m_pole0                                              |  | 0.31379 +/- 0.12049 |  |      |      |      |      |      |      |      |       | 1.00  |
| =====                                                     |  |                     |  |      |      |      |      |      |      |      |       |       |

Phase space prescription ::

threshold\_sub

eta8:eta1[-] f8:eta8[+] h8:eta8[+] omega8:eta8[-] omega8:omega1[-] omega8:omega8[-] upper half-plane

sqrt(s)\_pole = (0.46067 +/- 0.00079956)  
+ (i/2)\*(+1.0064e-11 +/- 3.996e-10) [ 0.44]

s\_pole = (0.21222 +/- 0.00073668)  
+ i\*(+4.6363e-12 +/- 1.841e-10) [ 0.44]

| eta8:eta1                    | f8:eta8                      | h8:eta8                      | omega8:eta8                  | omega8:omega1                | omega8:omega8                |
|------------------------------|------------------------------|------------------------------|------------------------------|------------------------------|------------------------------|
| =====                        | =====                        | =====                        | =====                        | =====                        | =====                        |
| k_re= -0.1157 +/- 2.1003     | k_re= 0.0000 +/- 0.0000      | k_re= 0.0000 +/- 0.0000      | k_re= -0.1088 +/- 1.9749     | k_re= -0.0612 +/- 1.1119     | k_re= -0.0633 +/- 1.1499     |
| k_im= -0.0000 +/- 0.0000     | k_im= 0.0385 +/- 0.0020      | k_im= 0.0533 +/- 0.0014      | k_im= -0.0000 +/- 0.0000     | k_im= -0.0000 +/- 0.0000     | k_im= -0.0000 +/- 0.0000     |
| corr= [ 0.20]                | corr= [-0.44]                | corr= [-0.44]                | corr= [ 0.20]                | corr= [ 0.20]                | corr= [ 0.20]                |
|                              |                              |                              |                              |                              |                              |
| eta8:eta1/1^P_1              | f8:eta8/3^S_1                | h8:eta8/3^S_1(*)             | omega8:eta8/3^P_1            | omega8:omega1/1^P_1          | omega8:omega1/3^P_1          |
| =====                        | =====                        | =====                        | =====                        | =====                        | =====                        |
| g = 0.0000 +/- 0.0000        | g = 0.0000 +/- 0.0000        | g = 0.3478 +/- 0.0247        | g = 0.0000 +/- 0.0000        | g = 0.0000 +/- 0.0000        | g = 0.0000 +/- 0.0000        |
| arg(g)/pi= 0.5000 +/- 0.0000 | arg(g)/pi= 0.5000 +/- 0.0000 | arg(g)/pi= 0.0000 +/- 0.0000 | arg(g)/pi= 0.5000 +/- 0.0000 | arg(g)/pi= 0.5000 +/- 0.0000 | arg(g)/pi= 0.5000 +/- 0.0000 |
| -----                        | -----                        | -----                        | -----                        | -----                        | -----                        |
| g_re= 0.0000 +/- 0.0000      | g_re= 0.0000 +/- 0.0000      | g_re= 0.3478 +/- 0.0247      | g_re= 0.0000 +/- 0.0000      | g_re= 0.0000 +/- 0.0000      | g_re= 0.0000 +/- 0.0000      |
| g_im= 0.0000 +/- 0.0000      | g_im= 0.0000 +/- 0.0000      | g_im= 0.0000 +/- 0.0000      | g_im= 0.0000 +/- 0.0000      | g_im= 0.0000 +/- 0.0000      | g_im= 0.0000 +/- 0.0000      |
| corr= [ 0.00]                | corr= [ 0.00]                | corr= [-1.00]                | corr= [ 0.00]                | corr= [ 0.00]                | corr= [ 0.00]                |
| -----                        | -----                        | -----                        | -----                        | -----                        | -----                        |
| eta8:eta1/1^P_1              | f8:eta8/3^S_1                | h8:eta8/3^S_1(*)             | omega8:eta8/3^P_1            | omega8:omega1/1^P_1          | omega8:omega1/3^P_1          |
| =====                        | =====                        | =====                        | =====                        | =====                        | =====                        |
| g = 0.0000 +/- 0.0000        | g = 0.0000 +/- 0.0000        | g = 0.3478 +/- 0.0247        | g = 0.0000 +/- 0.0000        | g = 0.0000 +/- 0.0000        | g = 0.0000 +/- 0.0000        |
| arg(g)/pi= 0.5000 +/- 0.0000 | arg(g)/pi= 0.5000 +/- 0.0000 | arg(g)/pi= 0.0000 +/- 0.0000 | arg(g)/pi= 0.5000 +/- 0.0000 | arg(g)/pi= 0.5000 +/- 0.0000 | arg(g)/pi= 0.5000 +/- 0.0000 |
| -----                        | -----                        | -----                        | -----                        | -----                        | -----                        |
| g_re= 0.0000 +/- 0.0000      | g_re= 0.0000 +/- 0.0000      | g_re= 0.3478 +/- 0.0247      | g_re= 0.0000 +/- 0.0000      | g_re= 0.0000 +/- 0.0000      | g_re= 0.0000 +/- 0.0000      |
| g_im= 0.0000 +/- 0.0000      | g_im= 0.0000 +/- 0.0000      | g_im= 0.0000 +/- 0.0000      | g_im= 0.0000 +/- 0.0000      | g_im= 0.0000 +/- 0.0000      | g_im= 0.0000 +/- 0.0000      |
| corr= [ 0.00]                | corr= [ 0.00]                | corr= [-1.00]                | corr= [ 0.00]                | corr= [ 0.00]                | corr= [ 0.00]                |
| -----                        | -----                        | -----                        | -----                        | -----                        | -----                        |

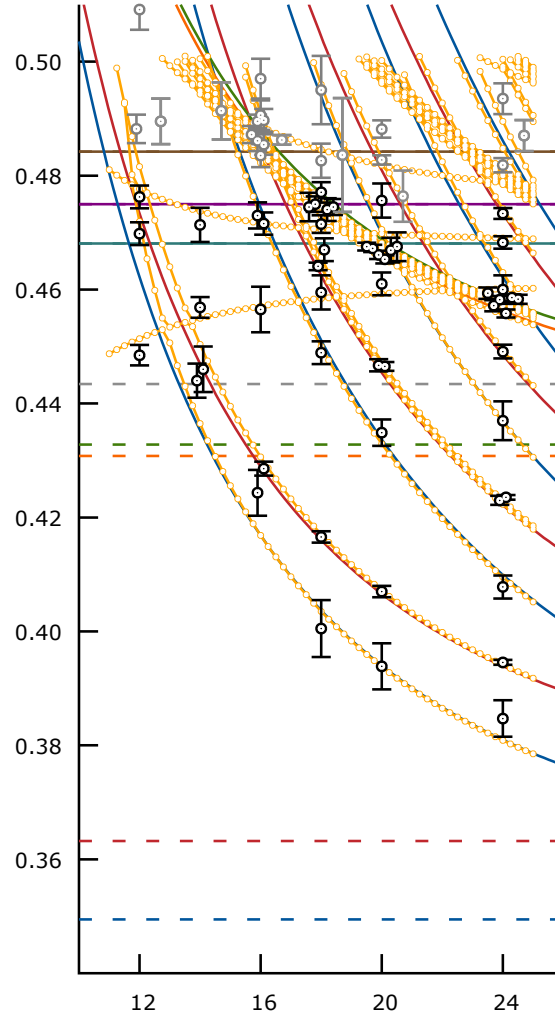

Figure 1.71: Similar to Figure 6 in the manuscript, the finite-volume spectrum, plotted as  $a_t E_{\text{cm}}$ , as a function of spatial extent  $L/a_s$ . Orange points/curves show the spectrum calculated from the amplitude given above (no uncertainties are shown). Black and grey points are the computed lattice energies on each volume, slightly displaced horizontally for clarity (black points correspond to energies used in the fit whereas grey points were not used). Two-meson non-interacting energies are shown as solid coloured curves/lines, two-meson thresholds are shown as dashed/solid horizontal lines, and the  $\eta^s \eta^s \eta^s$  threshold is shown as a dashed grey horizontal line.

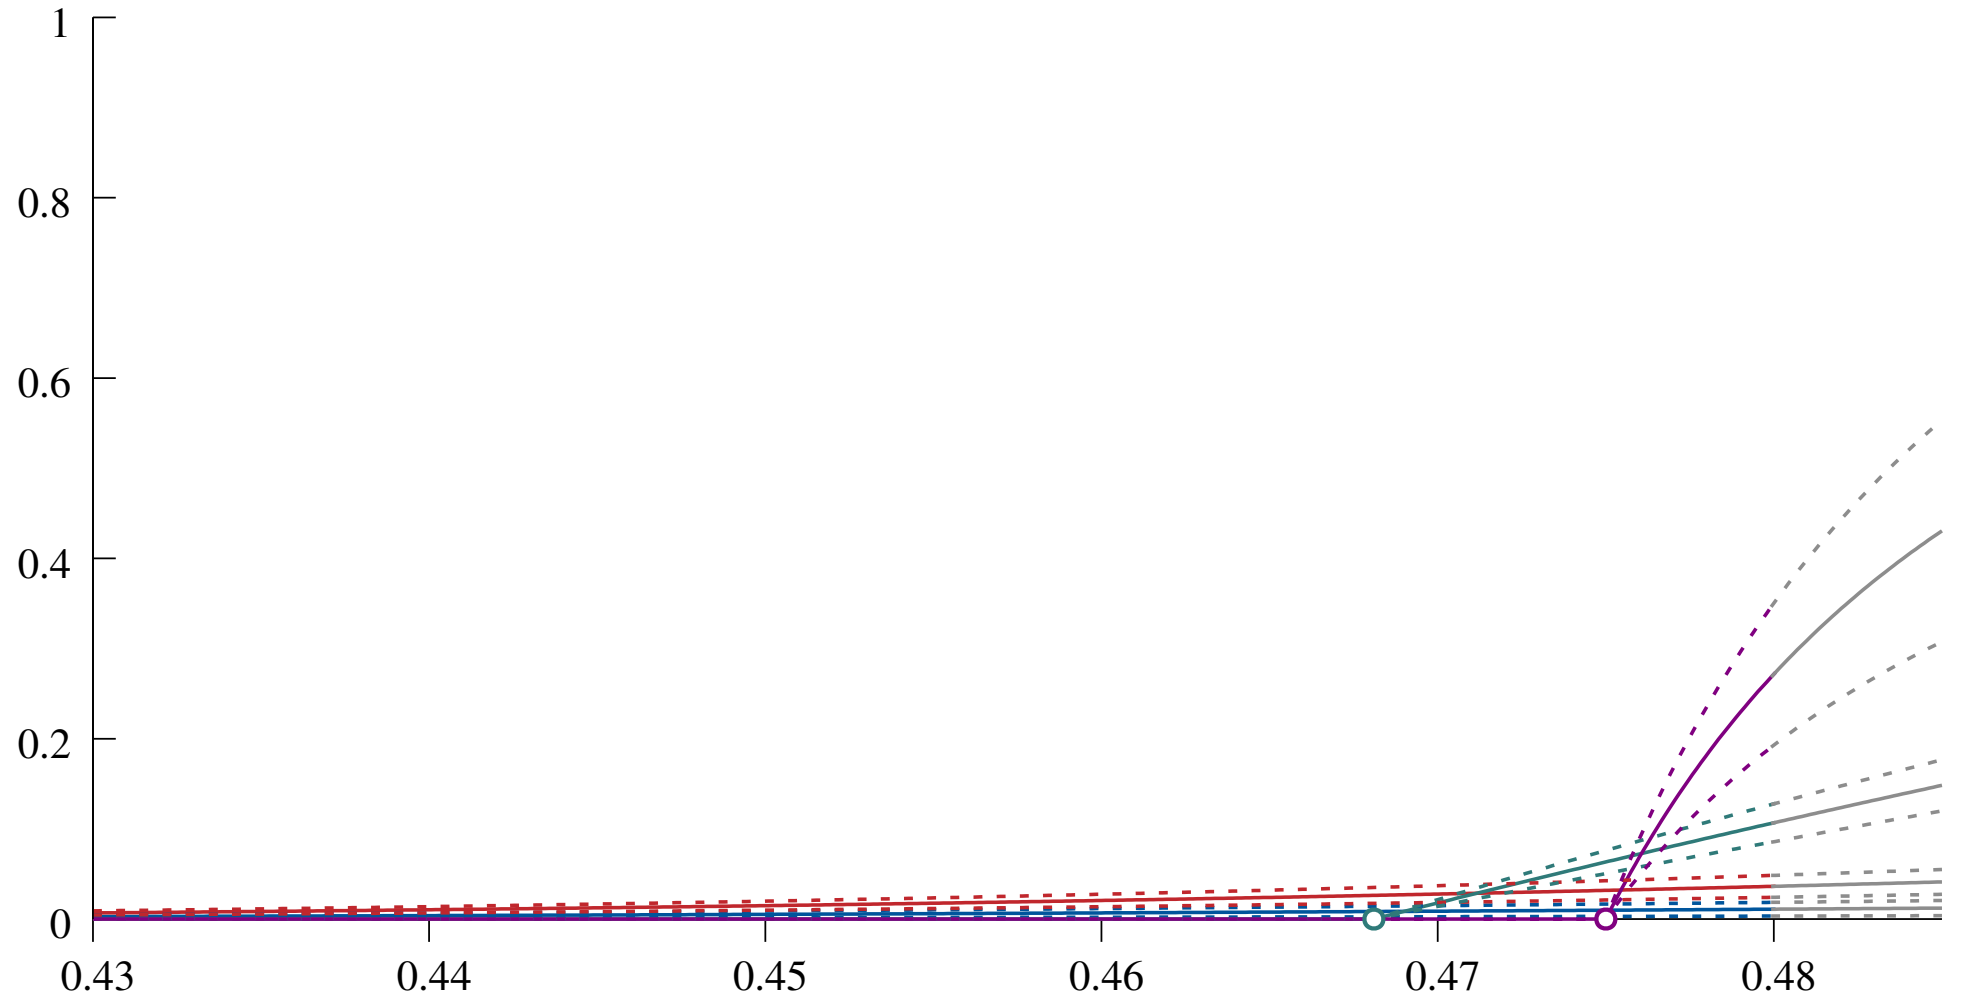

Figure 1.72: Similar to part (a) of Figure 7 in the manuscript,  $\rho_a \rho_b |t_{ab}|^2$  as a function of  $a_t E_{cm}$  for  $\eta^1 \eta^s \{^1P_1\} \rightarrow \eta^1 \eta^s \{^1P_1\}$  (blue),  $\omega^s \eta^s \{^3P_1\} \rightarrow \omega^s \eta^s \{^3P_1\}$  (red),  $f_1^s \eta^s \{^3S_1\} \rightarrow f_1^s \eta^s \{^3S_1\}$  (cyan), and  $h_1^s \eta^s \{^3S_1\} \rightarrow h_1^s \eta^s \{^3S_1\}$  (purple). Dashed lines indicate one standard deviation statistical uncertainties.

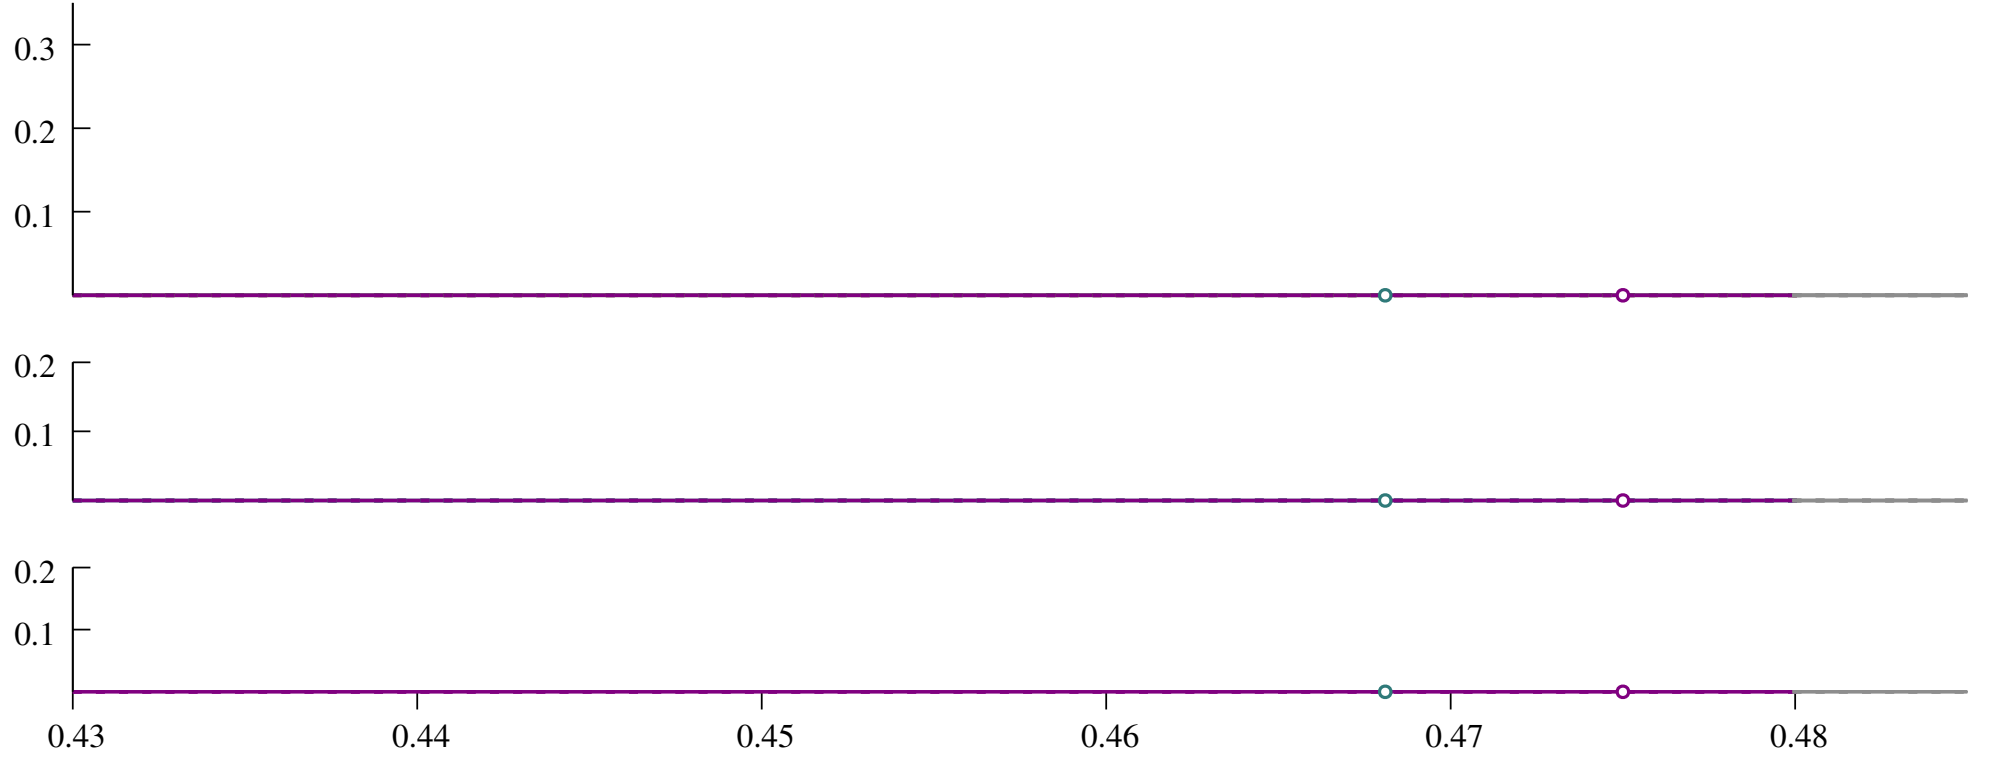

Figure 1.73: Similar to parts (b), (c) and (d) of Figure 7 in the manuscript,  $\rho_a \rho_b |t_{ab}|^2$  as a function of  $a_t E_{\text{cm}}$ . Top:  $\eta^1 \eta^s \{^1P_1\} \rightarrow \omega^s \eta^s \{^3P_1\}$  (red),  $\eta^1 \eta^s \{^1P_1\} \rightarrow f_1^s \eta^s \{^3S_1\}$  (cyan), and  $\eta^1 \eta^s \{^1P_1\} \rightarrow h_1^s \eta^s \{^3S_1\}$  (purple). Middle:  $\omega^s \eta^s \{^3P_1\} \rightarrow f_1^s \eta^s \{^3S_1\}$  (cyan), and  $\omega^s \eta^s \{^3P_1\} \rightarrow h_1^s \eta^s \{^3S_1\}$  (purple). Bottom:  $f_1^s \eta^s \{^3S_1\} \rightarrow h_1^s \eta^s \{^3S_1\}$  (purple). Dashed lines indicate one standard deviation statistical uncertainties.

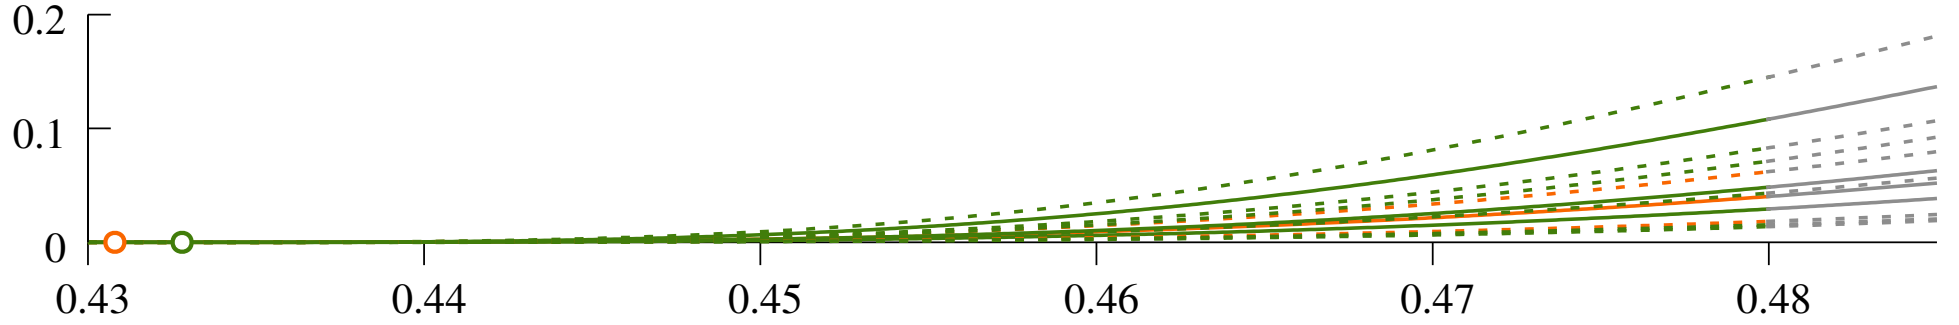

Figure 1.74: Similar to parts (e) and (f) of Figure 7 in the manuscript,  $\rho_a \rho_b |t_{ab}|^2$  as a function of  $a_t E_{cm}$  for  $\omega^s \omega^s \{^3P_1\} \rightarrow \omega^s \omega^s \{^3P_1\}$  (orange),  $\omega^1 \omega^s \{^1P_1, ^3P_1, ^5P_1\} \rightarrow \omega^s \omega^1 \{^1P_1, ^3P_1, ^5P_1\}$  (green). Dashed lines indicate one standard deviation statistical uncertainties.

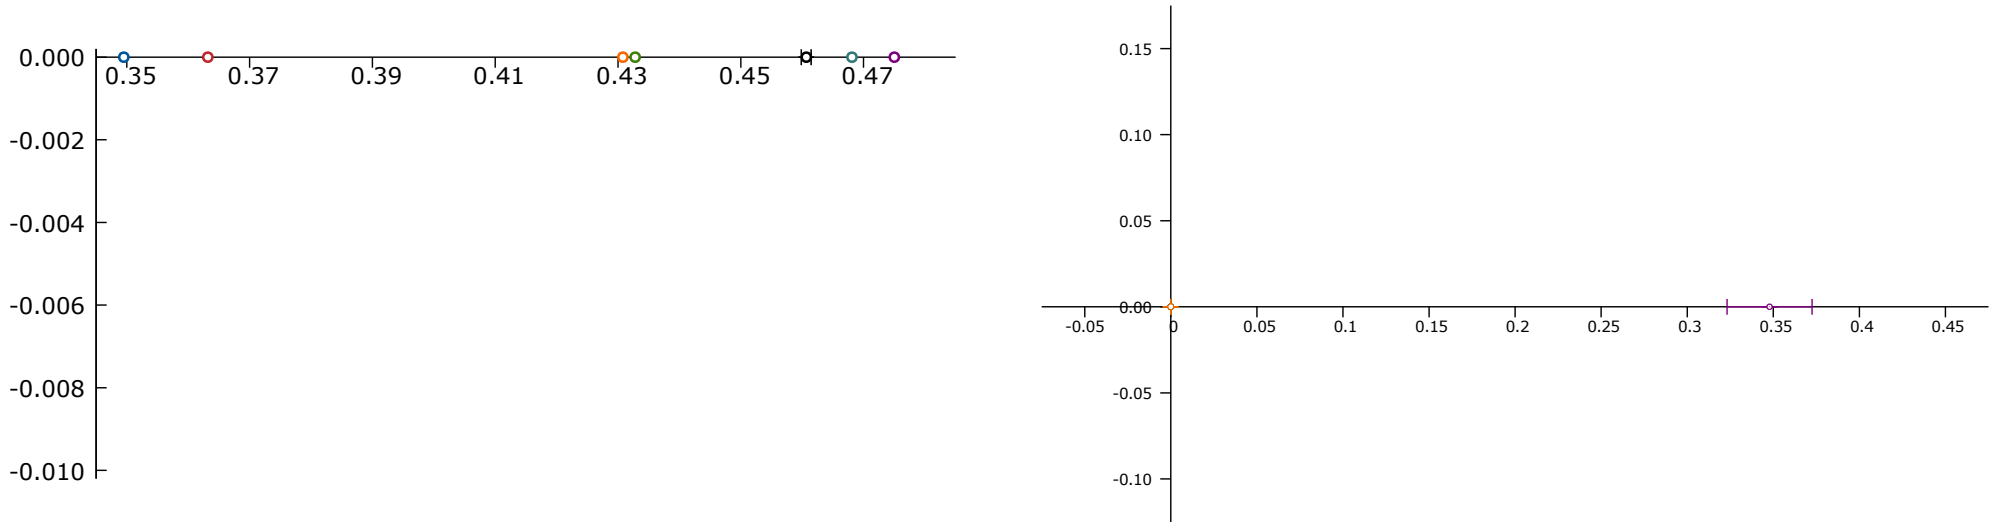

Figure 1.75: Left: Similar to Figure 13 in the manuscript, pole position on the proximal sheet (closest to physical scattering) with  $\text{Re}(a_t \sqrt{s})$  on the horizontal axis and  $2 \text{Im}(a_t \sqrt{s})$  on the vertical axis. Right: Similar to Figure 14 in the manuscript, the corresponding couplings with  $\text{Re}(a_t c)$  on the horizontal axis and  $\text{Im}(a_t c)$  on the vertical axis.

# 1.16 $\{m, g_{a,b,f}^{(0)}, \gamma_{(a,a),(b,b),(c,c),(d_1,d_1),(d_2,d_2),(d_3,d_3),(e,e),(f,f)}^{(0)}\}(\mathbf{CM}_{thr})$

minimised with chisq/nDoF = 43.18 / (53 - 12) = 1.05

|                                                          |  |                       |  |      |       |       |       |       |       |       |       |       |       |       |       |
|----------------------------------------------------------|--|-----------------------|--|------|-------|-------|-------|-------|-------|-------|-------|-------|-------|-------|-------|
| =====                                                    |  |                       |  |      |       |       |       |       |       |       |       |       |       |       |       |
| JP1-g_eta8:eta1/1^P_1_pole0                              |  | 0.19096 +/- 0.041638  |  | 1.00 | -0.41 | 0.10  | -0.28 | -0.03 | -0.41 | 0.05  | -0.04 | -0.02 | -0.08 | -0.07 | -0.01 |
| JP1-g_h8:eta8/3^S_1_pole0                                |  | 3.2057 +/- 0.42806    |  |      | 1.00  | -0.25 | -0.27 | 0.27  | 1.00  | 0.01  | 0.03  | -0.02 | 0.03  | 0.04  | -0.02 |
| JP1-g_omega8:eta8/3^P_1_pole0                            |  | 0.18596 +/- 0.04854   |  |      |       | 1.00  | -0.26 | 0.10  | -0.24 | -0.66 | 0.05  | -0.02 | 0.01  | 0.04  | -0.01 |
| JP1-gamma_eta8:eta1/1^P_1 eta8:eta1/1^P_1_order0         |  | -2.7284 +/- 1.9261    |  |      |       |       | 1.00  | -0.01 | -0.28 | 0.25  | -0.05 | 0.09  | -0.00 | -0.06 | -0.01 |
| JP1-gamma_f8:eta8/3^S_1 f8:eta8/3^S_1_order0             |  | -1.6791 +/- 0.15365   |  |      |       |       |       | 1.00  | 0.28  | -0.07 | 0.05  | 0.03  | 0.04  | 0.06  | 0.01  |
| JP1-gamma_h8:eta8/3^S_1 h8:eta8/3^S_1_order0             |  | 44.068 +/- 13.112     |  |      |       |       |       |       | 1.00  | -0.00 | 0.03  | -0.02 | 0.03  | 0.05  | 0.00  |
| JP1-gamma_omega8:eta8/3^P_1 omega8:eta8/3^P_1_order0     |  | -3.8335 +/- 0.66845   |  |      |       |       |       |       |       | 1.00  | 0.03  | 0.09  | 0.05  | 0.08  | 0.00  |
| JP1-gamma_omega8:omega1/1^P_1 omega8:omega1/1^P_1_order0 |  | 10.045 +/- 2.4879     |  |      |       |       |       |       |       |       | 1.00  | 0.05  | 0.39  | 0.43  | 0.00  |
| JP1-gamma_omega8:omega1/3^P_1 omega8:omega1/3^P_1_order0 |  | 10.899 +/- 5.0901     |  |      |       |       |       |       |       |       |       | 1.00  | 0.13  | 0.09  | -0.00 |
| JP1-gamma_omega8:omega1/5^P_1 omega8:omega1/5^P_1_order0 |  | 20.130 +/- 4.0864     |  |      |       |       |       |       |       |       |       |       | 1.00  | 0.46  | 0.00  |
| JP1-gamma_omega8:omega8/3^P_1 omega8:omega8/3^P_1_order0 |  | 11.295 +/- 3.0872     |  |      |       |       |       |       |       |       |       |       |       | 1.00  | 0.00  |
| JP1-m_pole0                                              |  | 0.0013317 +/- 0.38371 |  |      |       |       |       |       |       |       |       |       |       |       | 1.00  |
| =====                                                    |  |                       |  |      |       |       |       |       |       |       |       |       |       |       |       |

Phase space prescription ::

threshold\_sub

eta8:eta1[-] f8:eta8[+] h8:eta8[+] omega8:eta8[-] omega8:omega1[-] omega8:omega8[-] lower half-plane

\*\*\* not found on > 5% cdfs \*\*\*

sqrt(s)\_pole = (0.45967 +/- 0.0056733)  
+ (i/2)\*(-0.0056641 +/- 0.0019974) [ 0.40]

s\_pole = (0.21129 +/- 0.0052216)  
+ i\*(-0.0026036 +/- 0.00090587) [ 0.38]

| eta8:eta1                | f8:eta8                  | h8:eta8                  | omega8:eta8              | omega8:omega1            | omega8:omega8            |
|--------------------------|--------------------------|--------------------------|--------------------------|--------------------------|--------------------------|
| k_re= 0.1483 +/- 0.0044  | k_re= -0.0067 +/- 0.0025 | k_re= -0.0049 +/- 0.0016 | k_re= 0.1394 +/- 0.0046  | k_re= 0.0775 +/- 0.0083  | k_re= 0.0803 +/- 0.0080  |
| k_im= -0.0022 +/- 0.0008 | k_im= 0.0416 +/- 0.0135  | k_im= 0.0554 +/- 0.0100  | k_im= -0.0023 +/- 0.0008 | k_im= -0.0042 +/- 0.0017 | k_im= -0.0041 +/- 0.0016 |
| corr= [ 0.44]            | corr= [ 0.53]            | corr= [ 0.17]            | corr= [ 0.45]            | corr= [ 0.58]            | corr= [ 0.57]            |

  

| eta8:eta1/1^P_1               | f8:eta8/3^S_1                | h8:eta8/3^S_1(*)              | omega8:eta8/3^P_1             | omega8:omega1/1^P_1          | omega8:omega1/3^P_1          | omega8:omega1/5^P_1          | omega8:omega8/3^P_1          |
|-------------------------------|------------------------------|-------------------------------|-------------------------------|------------------------------|------------------------------|------------------------------|------------------------------|
| g = 0.0475 +/- 0.0103         | g = 0.0000 +/- 0.0000        | g = 0.2520 +/- 0.0230         | g = 0.0434 +/- 0.0111         | g = 0.0000 +/- 0.0000        | g = 0.0000 +/- 0.0000        | g = 0.0000 +/- 0.0000        | g = 0.0000 +/- 0.0000        |
| arg(g)/pi= -0.0504 +/- 0.0428 | arg(g)/pi= 0.5143 +/- 0.0071 | arg(g)/pi= -0.0143 +/- 0.0071 | arg(g)/pi= -0.0597 +/- 0.0130 | arg(g)/pi= 0.5143 +/- 0.0071 | arg(g)/pi= 0.5143 +/- 0.0071 | arg(g)/pi= 0.5143 +/- 0.0071 | arg(g)/pi= 0.5143 +/- 0.0071 |
| g_re= 0.0469 +/- 0.0097       | g_re= -0.0000 +/- 0.0000     | g_re= 0.2518 +/- 0.0232       | g_re= 0.0426 +/- 0.0106       | g_re= -0.0000 +/- 0.0000     | g_re= -0.0000 +/- 0.0000     | g_re= -0.0000 +/- 0.0000     | g_re= -0.0000 +/- 0.0000     |
| g_im= -0.0075 +/- 0.0072      | g_im= 0.0000 +/- 0.0000      | g_im= -0.0114 +/- 0.0050      | g_im= -0.0081 +/- 0.0035      | g_im= 0.0000 +/- 0.0000      | g_im= 0.0000 +/- 0.0000      | g_im= 0.0000 +/- 0.0000      | g_im= 0.0000 +/- 0.0000      |
| corr= [-0.56]                 | corr= [-0.69]                | corr= [ 0.47]                 | corr= [-0.93]                 | corr= [-0.69]                | corr= [-0.69]                | corr= [-0.69]                | corr= [-0.69]                |

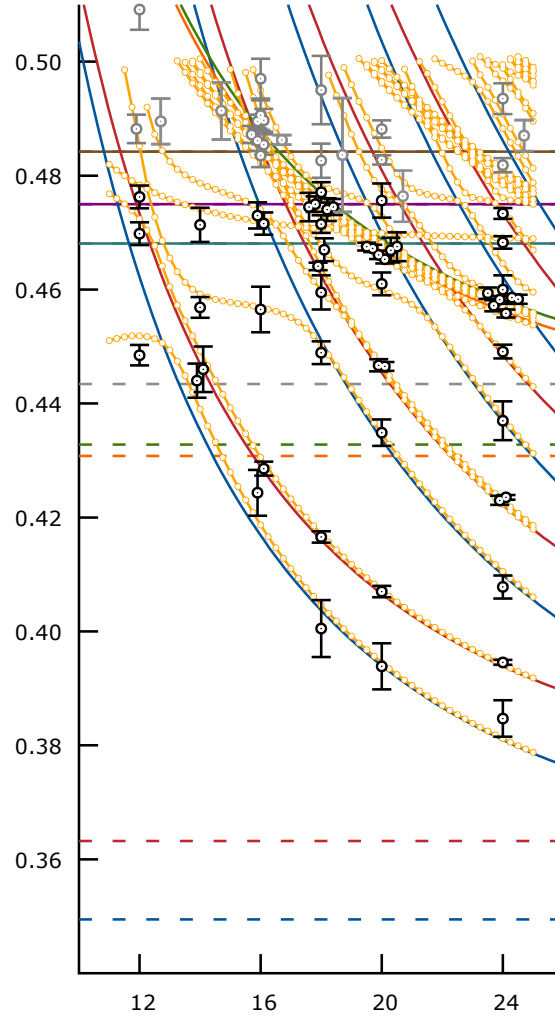

Figure 1.76: Similar to Figure 6 in the manuscript, the finite-volume spectrum, plotted as  $a_t E_{\text{cm}}$ , as a function of spatial extent  $L/a_s$ . Orange points/curves show the spectrum calculated from the amplitude given above (no uncertainties are shown). Black and grey points are the computed lattice energies on each volume, slightly displaced horizontally for clarity (black points correspond to energies used in the fit whereas grey points were not used). Two-meson non-interacting energies are shown as solid coloured curves/lines, two-meson thresholds are shown as dashed/solid horizontal lines, and the  $\eta^s \eta^s \eta^s$  threshold is shown as a dashed grey horizontal line.

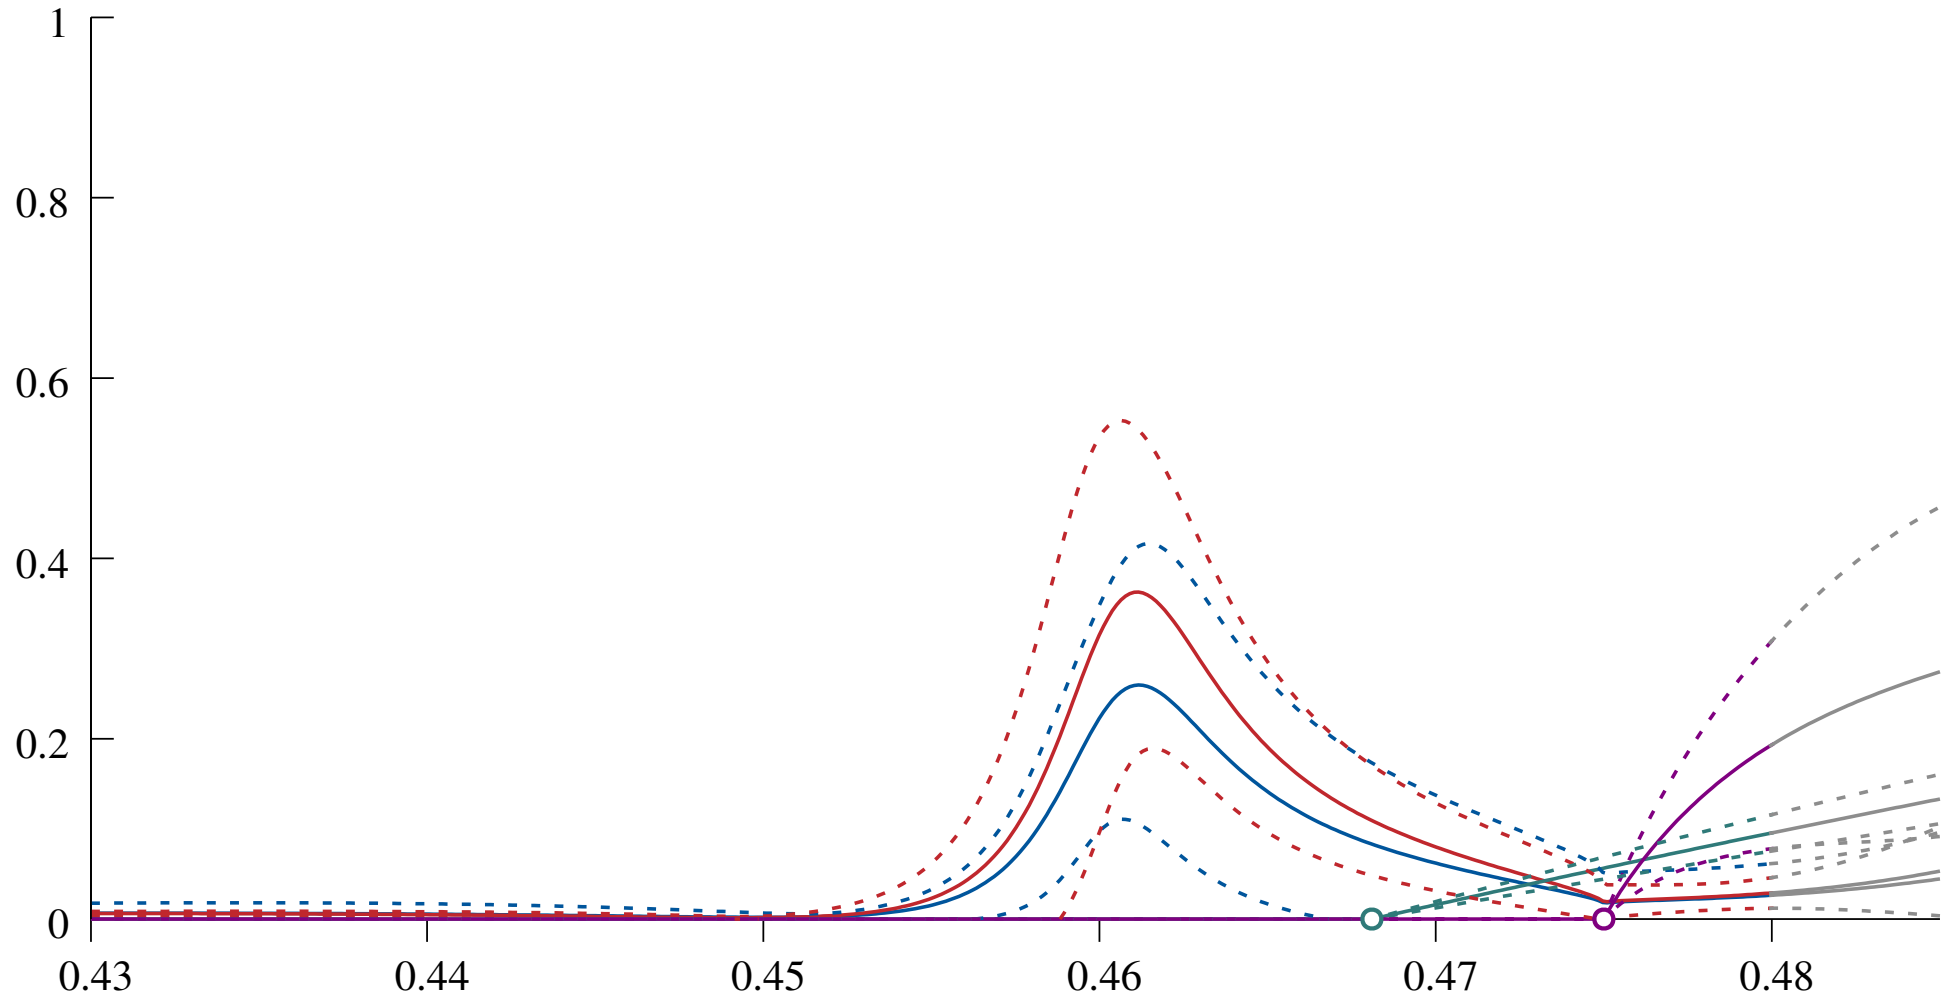

Figure 1.77: Similar to part (a) of Figure 7 in the manuscript,  $\rho_a \rho_b |t_{ab}|^2$  as a function of  $a_t E_{cm}$  for  $\eta^1 \eta^s \{^1P_1\} \rightarrow \eta^1 \eta^s \{^1P_1\}$  (blue),  $\omega^s \eta^s \{^3P_1\} \rightarrow \omega^s \eta^s \{^3P_1\}$  (red),  $f_1^s \eta^s \{^3S_1\} \rightarrow f_1^s \eta^s \{^3S_1\}$  (cyan), and  $h_1^s \eta^s \{^3S_1\} \rightarrow h_1^s \eta^s \{^3S_1\}$  (purple). Dashed lines indicate one standard deviation statistical uncertainties.

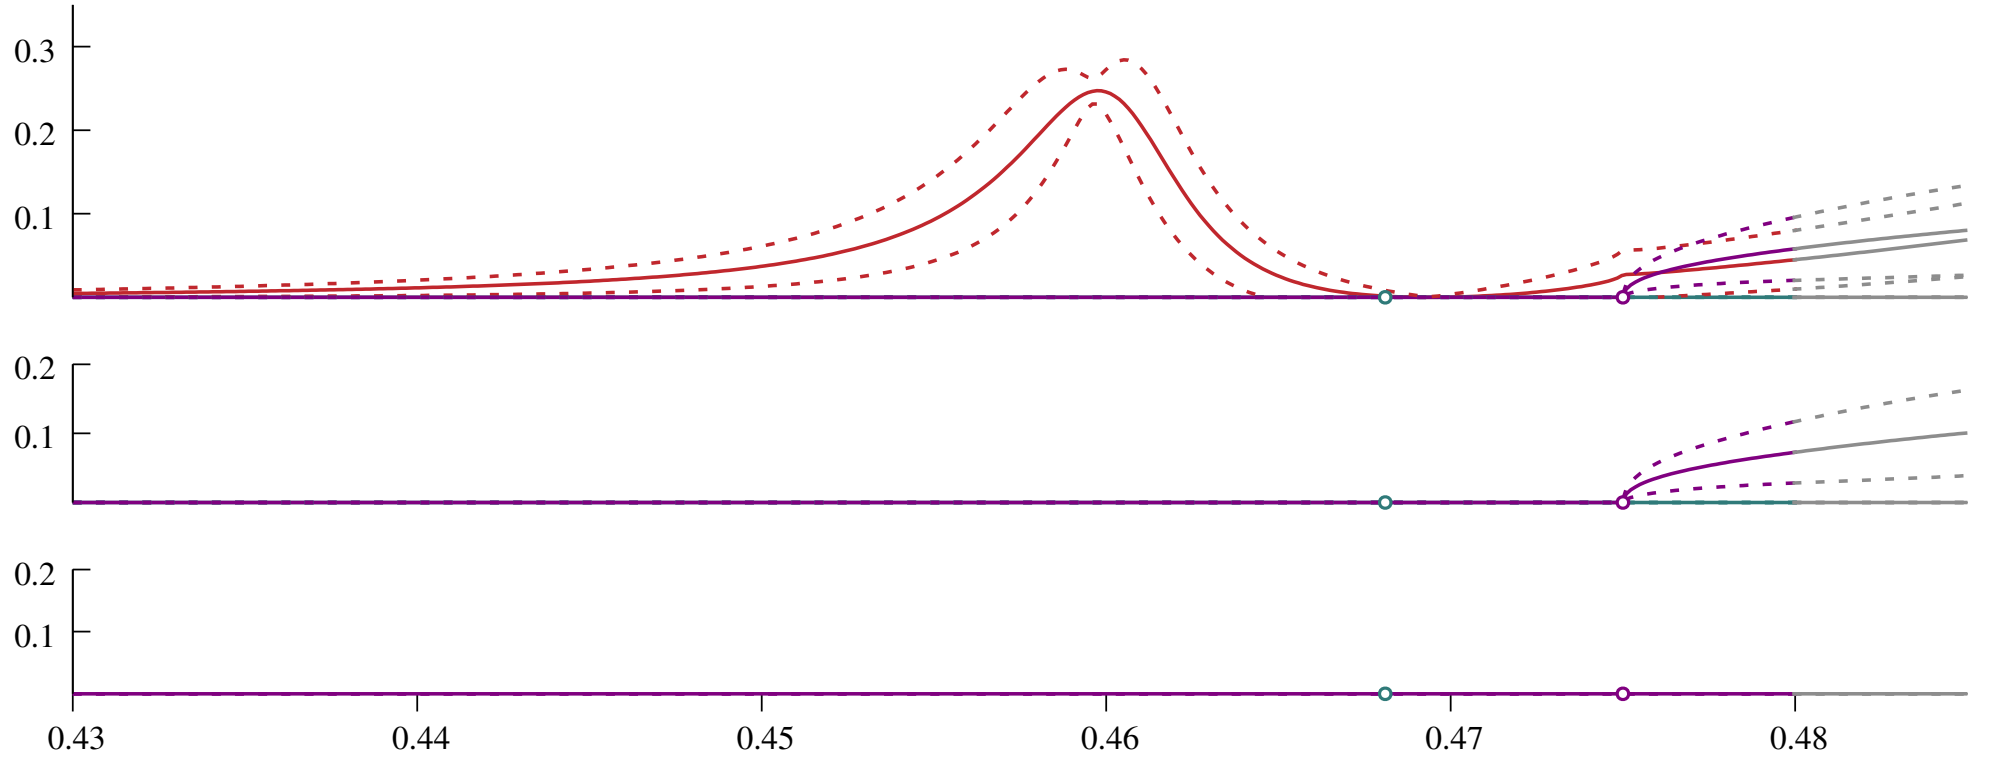

Figure 1.78: Similar to parts (b), (c) and (d) of Figure 7 in the manuscript,  $\rho_a \rho_b |t_{ab}|^2$  as a function of  $a_t E_{\text{cm}}$ . Top:  $\eta^1 \eta^s \{^1P_1\} \rightarrow \omega^s \eta^s \{^3P_1\}$  (red),  $\eta^1 \eta^s \{^1P_1\} \rightarrow f_1^s \eta^s \{^3S_1\}$  (cyan), and  $\eta^1 \eta^s \{^1P_1\} \rightarrow h_1^s \eta^s \{^3S_1\}$  (purple). Middle:  $\omega^s \eta^s \{^3P_1\} \rightarrow f_1^s \eta^s \{^3S_1\}$  (cyan), and  $\omega^s \eta^s \{^3P_1\} \rightarrow h_1^s \eta^s \{^3S_1\}$  (purple). Bottom:  $f_1^s \eta^s \{^3S_1\} \rightarrow h_1^s \eta^s \{^3S_1\}$  (purple). Dashed lines indicate one standard deviation statistical uncertainties.

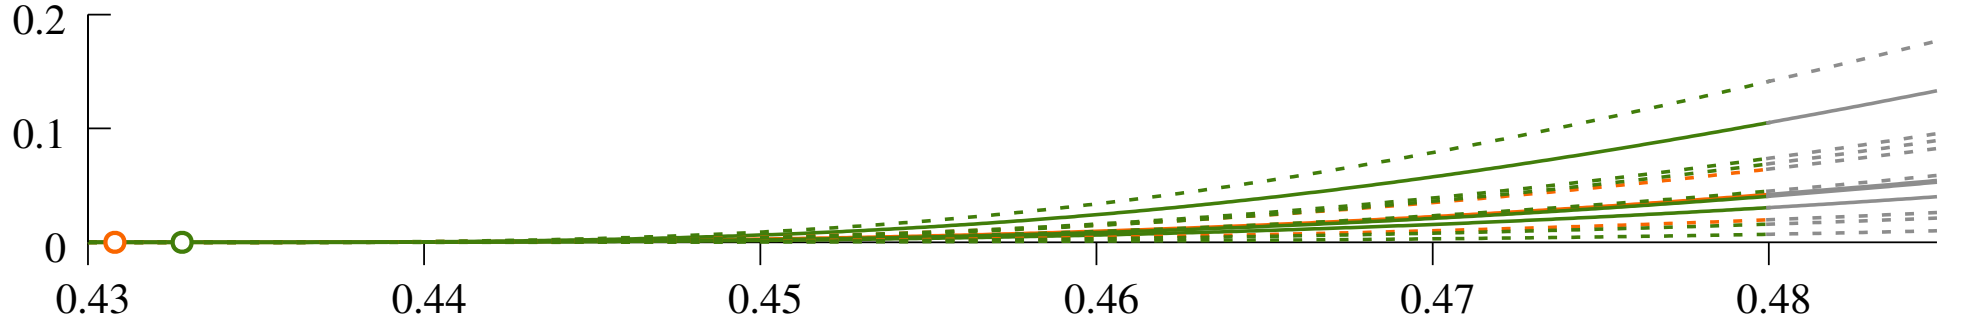

Figure 1.79: Similar to parts (e) and (f) of Figure 7 in the manuscript,  $\rho_a \rho_b |t_{ab}|^2$  as a function of  $a_t E_{cm}$  for  $\omega^s \omega^s \{^3P_1\} \rightarrow \omega^s \omega^s \{^3P_1\}$  (orange),  $\omega^1 \omega^s \{^1P_1, ^3P_1, ^5P_1\} \rightarrow \omega^s \omega^1 \{^1P_1, ^3P_1, ^5P_1\}$  (green). Dashed lines indicate one standard deviation statistical uncertainties.

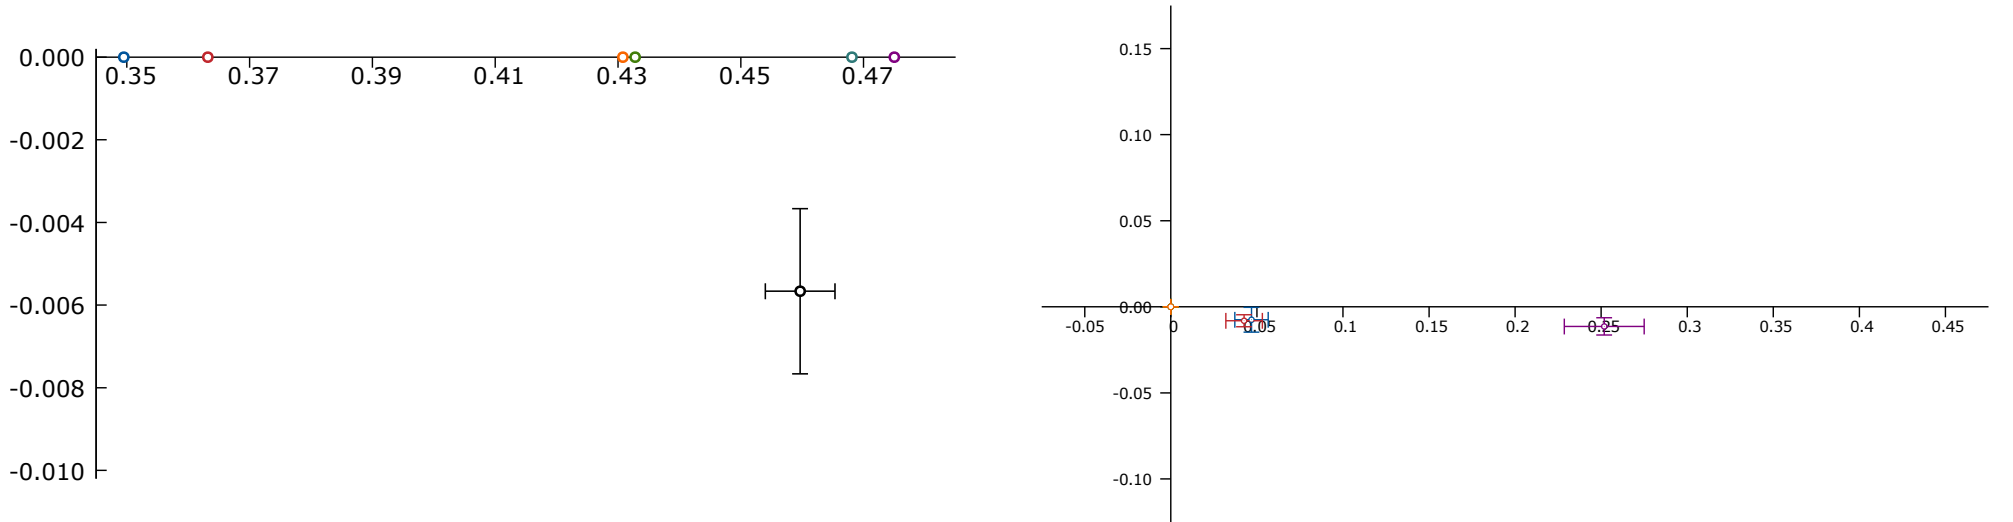

Figure 1.80: Left: Similar to Figure 13 in the manuscript, pole position on the proximal sheet (closest to physical scattering) with  $\text{Re}(a_t \sqrt{s})$  on the horizontal axis and  $2 \text{Im}(a_t \sqrt{s})$  on the vertical axis. Right: Similar to Figure 14 in the manuscript, the corresponding couplings with  $\text{Re}(a_t c)$  on the horizontal axis and  $\text{Im}(a_t c)$  on the vertical axis.

# 1.17 $\{m, g_{a,b,c,f}^{(0)}, \gamma_{(a,a),(b,b),(c,c),(\partial_1,\partial_1),(\partial_2,\partial_2),(\partial_3,\partial_3)}^{(0)}\}(\mathbf{CM}_{thr})$

minimised with chisq/nDoF = 43.64 / (53 - 11) = 1.04

|                                                           |  |                      |  |      |      |      |      |      |       |       |      |       |             |
|-----------------------------------------------------------|--|----------------------|--|------|------|------|------|------|-------|-------|------|-------|-------------|
| =====                                                     |  |                      |  |      |      |      |      |      |       |       |      |       |             |
| JP1-_g_eta8:eta1/1^P_1_pole0                              |  | 0.26449 +/- 0.11478  |  | 1.00 | 0.76 | 0.76 | 0.58 | 0.06 | 0.03  | -0.03 | 0.03 | -0.06 | -0.07 -0.77 |
| JP1-_g_f8:eta8/3^S_1_pole0                                |  | 0.40369 +/- 0.16573  |  |      | 1.00 | 0.88 | 0.71 | 0.18 | -0.04 | -0.02 | 0.03 | -0.02 | -0.05 -0.92 |
| JP1-_g_h8:eta8/3^S_1_pole0                                |  | 0.56531 +/- 0.29076  |  |      |      | 1.00 | 0.73 | 0.32 | 0.01  | 0.02  | 0.08 | 0.02  | 0.01 -0.99  |
| JP1-_g_omega8:eta8/3^P_1_pole0                            |  | 0.26415 +/- 0.12093  |  |      |      |      | 1.00 | 0.24 | -0.44 | 0.01  | 0.01 | 0.01  | 0.00 -0.76  |
| JP1-_gamma_eta8:eta1/1^P_1 eta8:eta1/1^P_1_order0         |  | -0.25509 +/- 0.51171 |  |      |      |      |      | 1.00 | -0.01 | 0.03  | 0.07 | 0.04  | 0.04 -0.30  |
| JP1-_gamma_omega8:eta8/3^P_1 omega8:eta8/3^P_1_order0     |  | -3.6601 +/- 0.6381   |  |      |      |      |      |      | 1.00  | 0.07  | 0.11 | 0.07  | 0.12 0.02   |
| JP1-_gamma_omega8:omega1/1^P_1 omega8:omega1/1^P_1_order0 |  | 9.7053 +/- 2.4802    |  |      |      |      |      |      |       | 1.00  | 0.06 | 0.39  | 0.44 -0.01  |
| JP1-_gamma_omega8:omega1/3^P_1 omega8:omega1/3^P_1_order0 |  | 11.308 +/- 5.1419    |  |      |      |      |      |      |       |       | 1.00 | 0.14  | 0.11 -0.07  |
| JP1-_gamma_omega8:omega1/5^P_1 omega8:omega1/5^P_1_order0 |  | 19.854 +/- 4.0902    |  |      |      |      |      |      |       |       |      | 1.00  | 0.46 -0.02  |
| JP1-_gamma_omega8:omega8/3^P_1 omega8:omega8/3^P_1_order0 |  | 10.680 +/- 3.0735    |  |      |      |      |      |      |       |       |      |       | 1.00 0.00   |
| JP1-_m_pole0                                              |  | 0.35005 +/- 0.11818  |  |      |      |      |      |      |       |       |      |       | 1.00        |
| =====                                                     |  |                      |  |      |      |      |      |      |       |       |      |       |             |

Phase space prescription ::

threshold\_sub

eta8:eta1[-] f8:eta8[+] h8:eta8[+] omega8:eta8[-] omega8:omega1[-] omega8:omega8[-] lower half-plane

sqrt(s)\_pole = (0.46093 +/- 0.0011586)  
+ (i/2)\*(-0.0036657 +/- 0.0015067) [ 0.02]

s\_pole = (0.21245 +/- 0.0010681)  
+ i\*(-0.0016896 +/- 0.00069439) [ 0.02]

| eta8:eta1                | f8:eta8                  | h8:eta8                  | omega8:eta8              | omega8:omega1            | omega8:omega8            |
|--------------------------|--------------------------|--------------------------|--------------------------|--------------------------|--------------------------|
| k_re= 0.1493 +/- 0.0009  | k_re= -0.0047 +/- 0.0019 | k_re= -0.0033 +/- 0.0014 | k_re= 0.1404 +/- 0.0009  | k_re= 0.0793 +/- 0.0017  | k_re= 0.0820 +/- 0.0016  |
| k_im= -0.0014 +/- 0.0006 | k_im= 0.0382 +/- 0.0030  | k_im= 0.0530 +/- 0.0021  | k_im= -0.0015 +/- 0.0006 | k_im= -0.0027 +/- 0.0011 | k_im= -0.0026 +/- 0.0011 |
| corr= [ 0.03]            | corr= [ 0.09]            | corr= [ 0.04]            | corr= [ 0.03]            | corr= [ 0.05]            | corr= [ 0.05]            |

  

| eta8:eta1/1^P_1              | f8:eta8/3^S_1                | h8:eta8/3^S_1(*)             | omega8:eta8/3^P_1             | omega8:omega1/1^P_1          | omega8:omega1/3^P_1          | omega8:omega1/5^P_1          | omega8:omega8/3^P_1          |
|------------------------------|------------------------------|------------------------------|-------------------------------|------------------------------|------------------------------|------------------------------|------------------------------|
| g = 0.0369 +/- 0.0100        | g = 0.1873 +/- 0.0252        | g = 0.2622 +/- 0.0452        | g = 0.0365 +/- 0.0115         | g = 0.0000 +/- 0.0000        | g = 0.0000 +/- 0.0000        | g = 0.0000 +/- 0.0000        | g = 0.0000 +/- 0.0000        |
| arg(g)/pi= 0.0014 +/- 0.0099 | arg(g)/pi= 0.0092 +/- 0.0049 | arg(g)/pi= 0.0092 +/- 0.0049 | arg(g)/pi= -0.0549 +/- 0.0110 | arg(g)/pi= 0.4908 +/- 0.0049 | arg(g)/pi= 0.4908 +/- 0.0049 | arg(g)/pi= 0.4908 +/- 0.0049 | arg(g)/pi= 0.4908 +/- 0.0049 |
| g_re= 0.0369 +/- 0.0100      | g_re= 0.1872 +/- 0.0252      | g_re= 0.2621 +/- 0.0452      | g_re= 0.0359 +/- 0.0112       | g_re= 0.0000 +/- 0.0000      | g_re= 0.0000 +/- 0.0000      | g_re= 0.0000 +/- 0.0000      | g_re= 0.0000 +/- 0.0000      |
| g_im= 0.0002 +/- 0.0011      | g_im= 0.0054 +/- 0.0032      | g_im= 0.0075 +/- 0.0044      | g_im= -0.0063 +/- 0.0028      | g_im= 0.0000 +/- 0.0000      | g_im= 0.0000 +/- 0.0000      | g_im= 0.0000 +/- 0.0000      | g_im= 0.0000 +/- 0.0000      |
| corr= [-0.09]                | corr= [ 0.56]                | corr= [ 0.41]                | corr= [-0.93]                 | corr= [ 0.19]                | corr= [ 0.19]                | corr= [ 0.19]                | corr= [ 0.19]                |

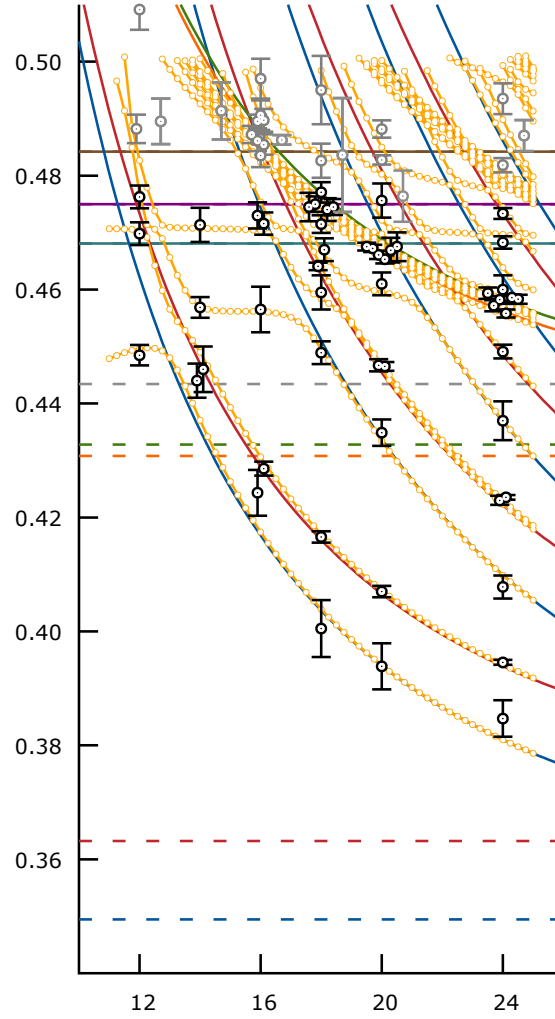

Figure 1.81: Similar to Figure 6 in the manuscript, the finite-volume spectrum, plotted as  $a_t E_{\text{cm}}$ , as a function of spatial extent  $L/a_s$ . Orange points/curves show the spectrum calculated from the amplitude given above (no uncertainties are shown). Black and grey points are the computed lattice energies on each volume, slightly displaced horizontally for clarity (black points correspond to energies used in the fit whereas grey points were not used). Two-meson non-interacting energies are shown as solid coloured curves/lines, two-meson thresholds are shown as dashed/solid horizontal lines, and the  $\eta^s \eta^s \eta^s$  threshold is shown as a dashed grey horizontal line.

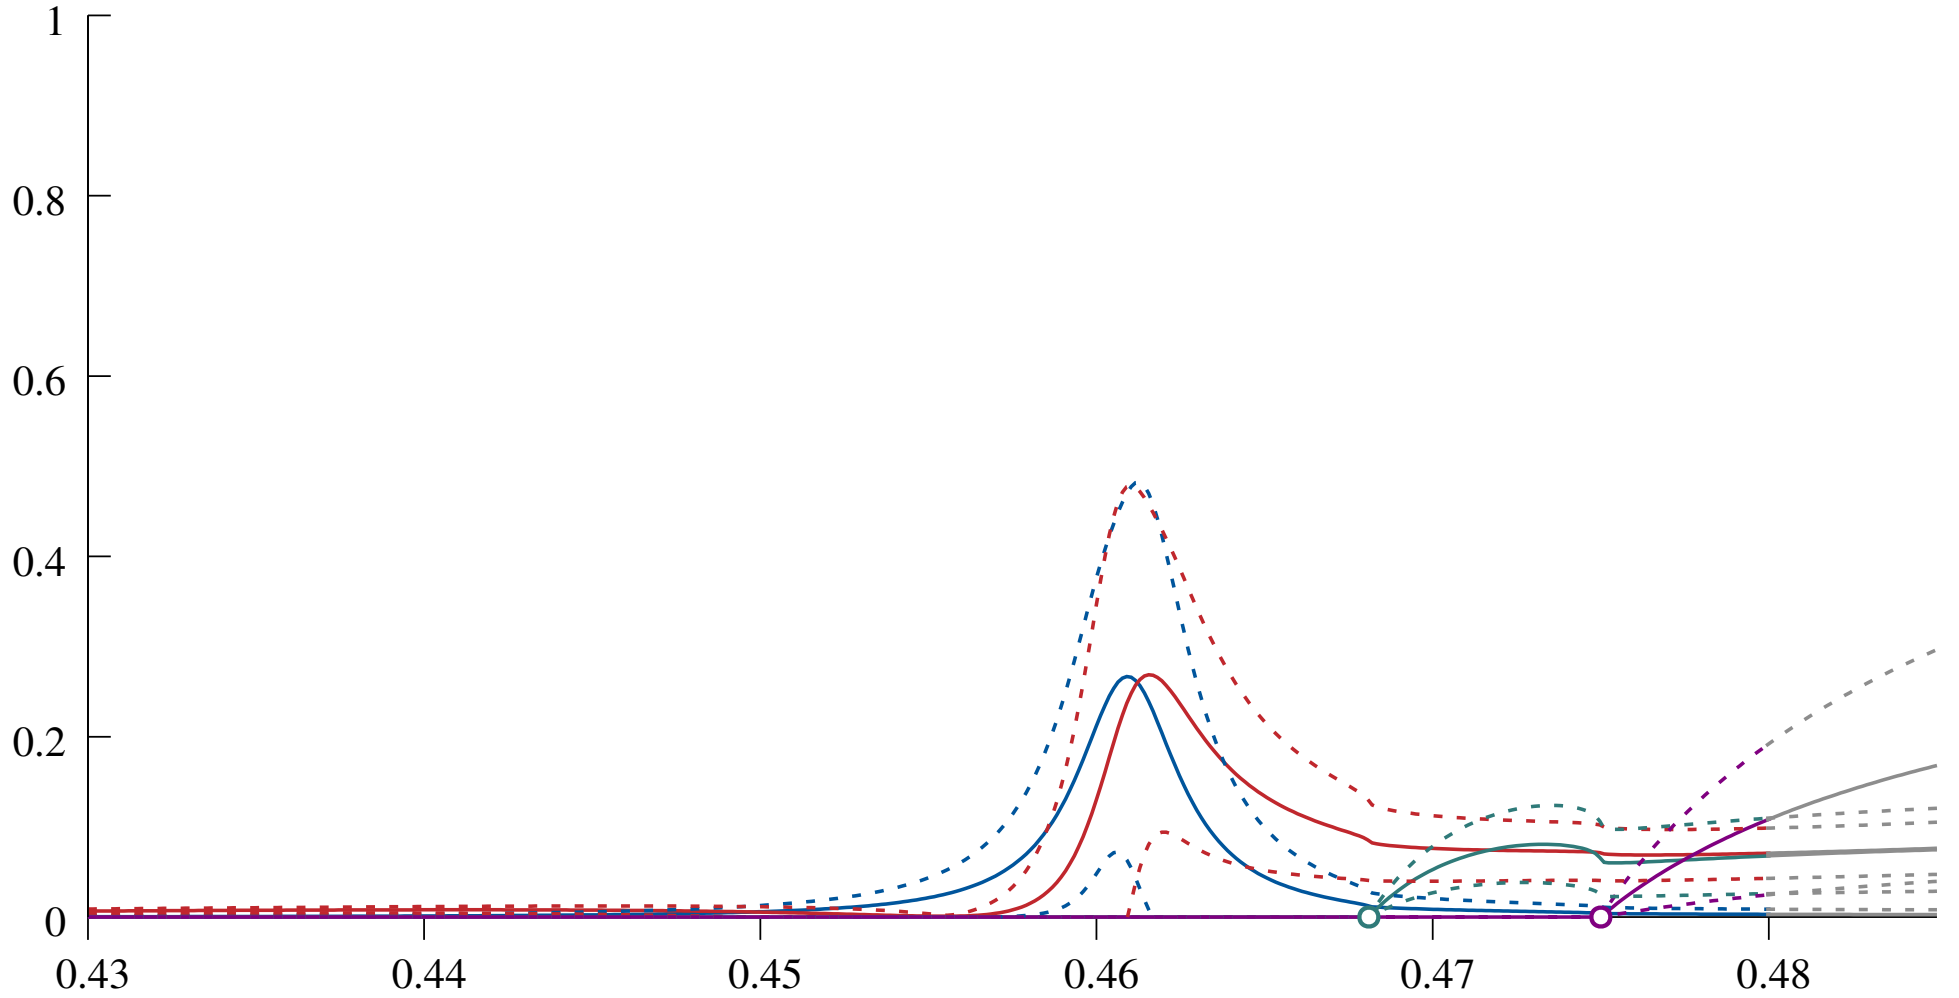

Figure 1.82: Similar to part (a) of Figure 7 in the manuscript,  $\rho_a \rho_b |t_{ab}|^2$  as a function of  $a_t E_{cm}$  for  $\eta^1 \eta^s \{^1P_1\} \rightarrow \eta^1 \eta^s \{^1P_1\}$  (blue),  $\omega^s \eta^s \{^3P_1\} \rightarrow \omega^s \eta^s \{^3P_1\}$  (red),  $f_1^s \eta^s \{^3S_1\} \rightarrow f_1^s \eta^s \{^3S_1\}$  (cyan), and  $h_1^s \eta^s \{^3S_1\} \rightarrow h_1^s \eta^s \{^3S_1\}$  (purple). Dashed lines indicate one standard deviation statistical uncertainties.

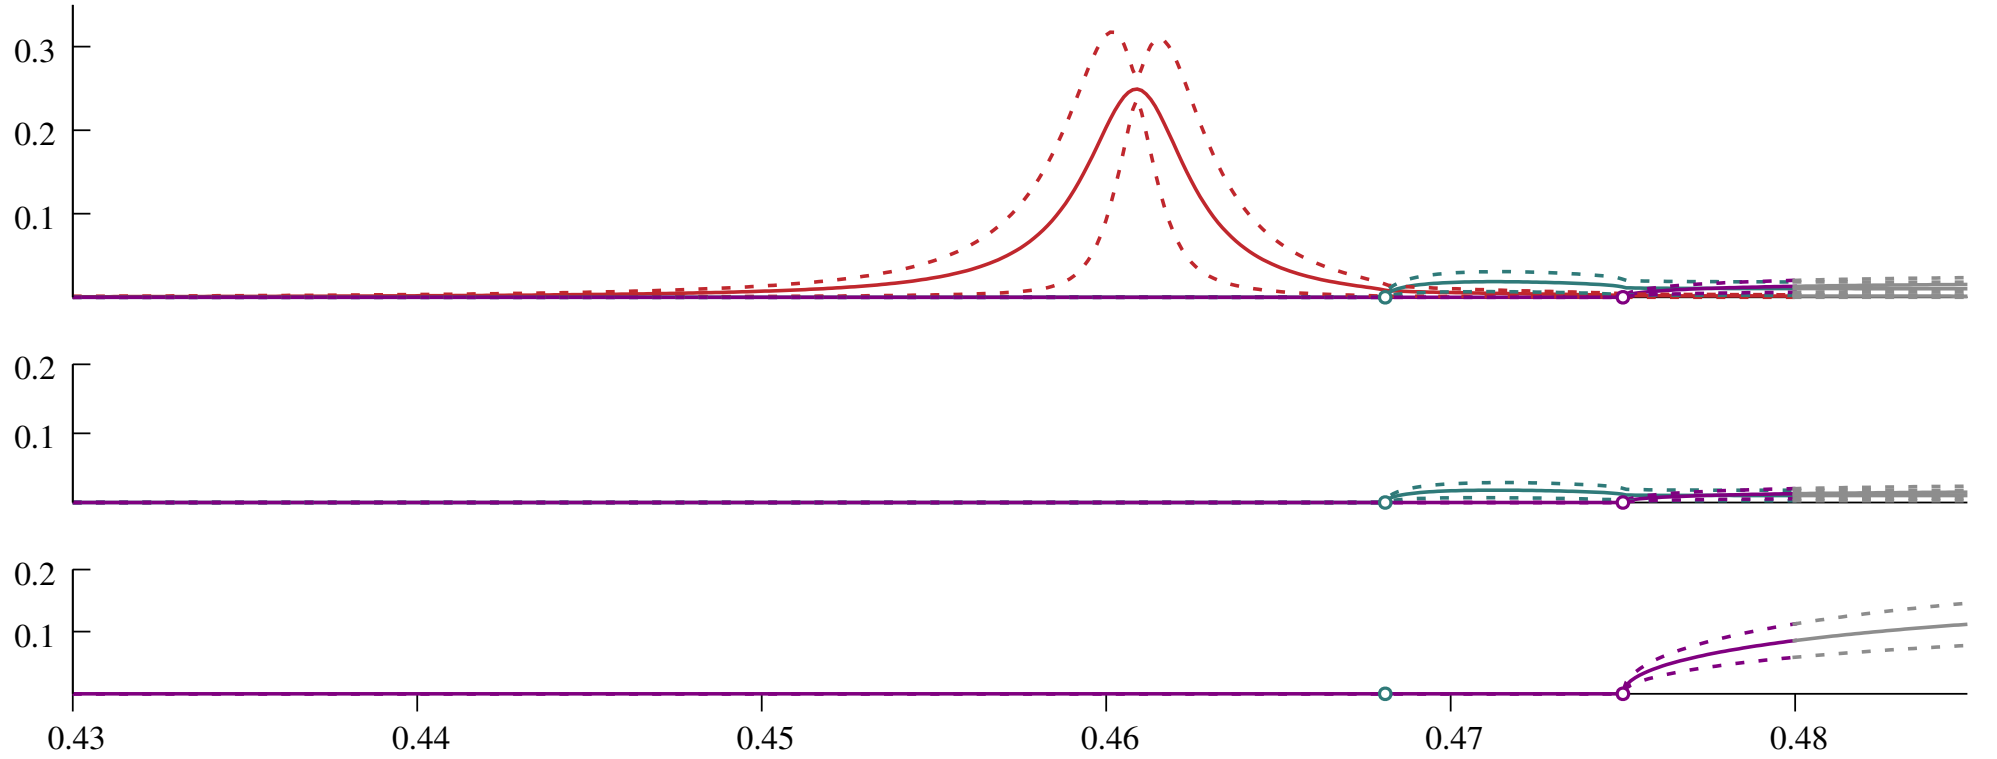

Figure 1.83: Similar to parts (b), (c) and (d) of Figure 7 in the manuscript,  $\rho_a \rho_b |t_{ab}|^2$  as a function of  $a_t E_{\text{cm}}$ . Top:  $\eta^1 \eta^s \{^1P_1\} \rightarrow \omega^s \eta^s \{^3P_1\}$  (red),  $\eta^1 \eta^s \{^1P_1\} \rightarrow f_1^s \eta^s \{^3S_1\}$  (cyan), and  $\eta^1 \eta^s \{^1P_1\} \rightarrow h_1^s \eta^s \{^3S_1\}$  (purple). Middle:  $\omega^s \eta^s \{^3P_1\} \rightarrow f_1^s \eta^s \{^3S_1\}$  (cyan), and  $\omega^s \eta^s \{^3P_1\} \rightarrow h_1^s \eta^s \{^3S_1\}$  (purple). Bottom:  $f_1^s \eta^s \{^3S_1\} \rightarrow h_1^s \eta^s \{^3S_1\}$  (purple). Dashed lines indicate one standard deviation statistical uncertainties.

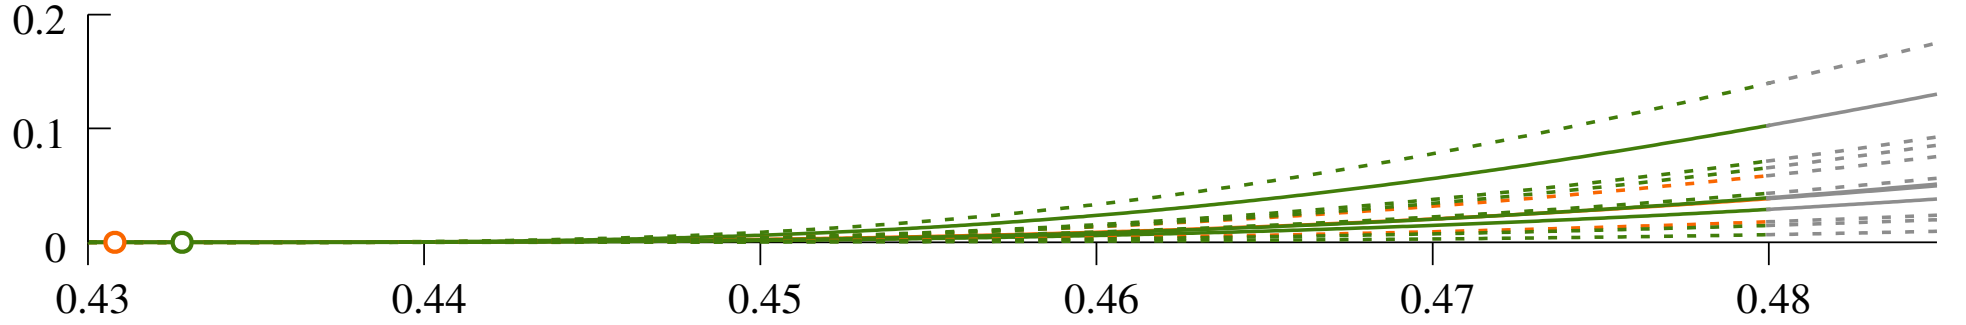

Figure 1.84: Similar to parts (e) and (f) of Figure 7 in the manuscript,  $\rho_a \rho_b |t_{ab}|^2$  as a function of  $a_t E_{cm}$  for  $\omega^s \omega^s \{^3P_1\} \rightarrow \omega^s \omega^s \{^3P_1\}$  (orange),  $\omega^1 \omega^s \{^1P_1, ^3P_1, ^5P_1\} \rightarrow \omega^s \omega^1 \{^1P_1, ^3P_1, ^5P_1\}$  (green). Dashed lines indicate one standard deviation statistical uncertainties.

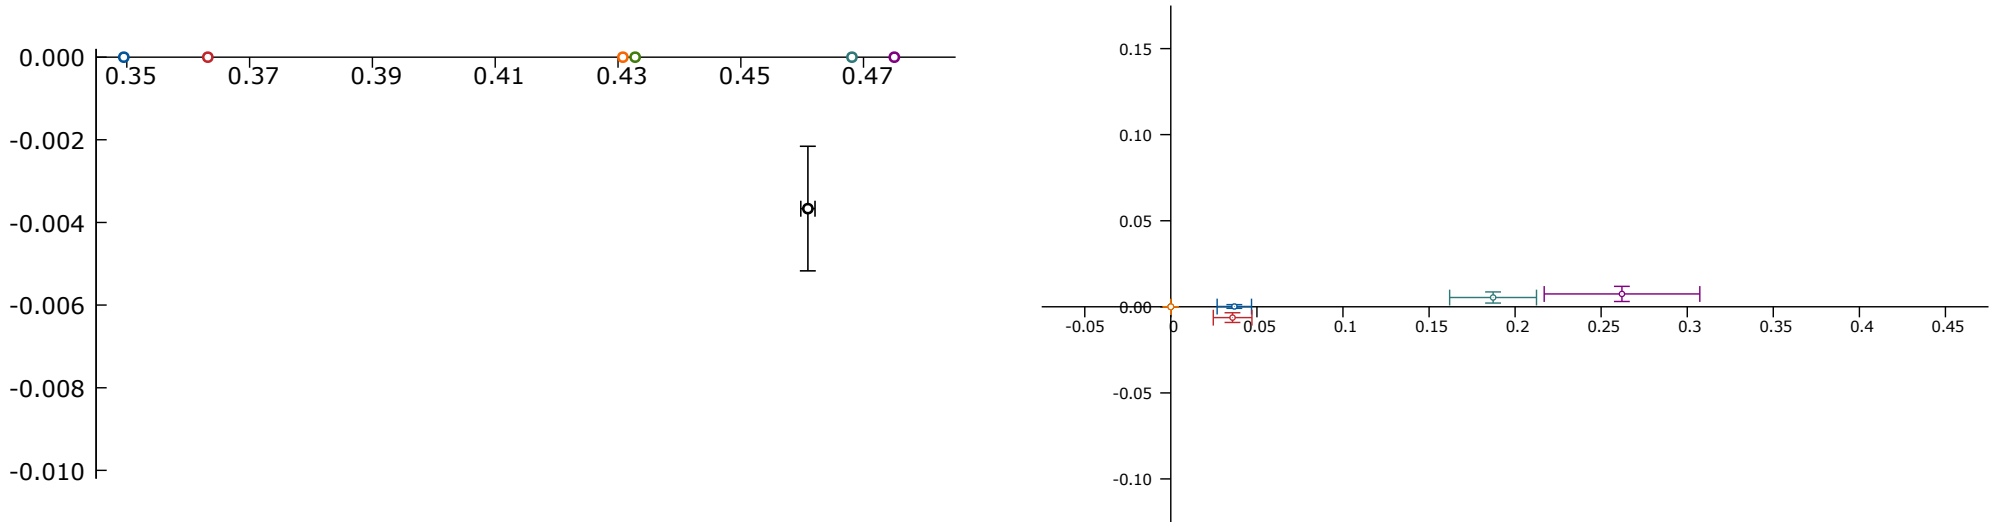

Figure 1.85: Left: Similar to Figure 13 in the manuscript, pole position on the proximal sheet (closest to physical scattering) with  $\text{Re}(a_t \sqrt{s})$  on the horizontal axis and  $2 \text{Im}(a_t \sqrt{s})$  on the vertical axis. Right: Similar to Figure 14 in the manuscript, the corresponding couplings with  $\text{Re}(a_t c)$  on the horizontal axis and  $\text{Im}(a_t c)$  on the vertical axis.

$$1.18 \quad \{m, g_{a,b,c,f}^{(0)}, \gamma_{(a,a),(b,b),(c,c),(\partial_1,\partial_1),(\partial_2,\partial_2),(\partial_3,\partial_3)}^{(0)}\}(-i\rho)$$

minimised with chisq/nDoF = 43.77 / (53 - 11) = 1.04

|                                                           |  |                       |  |      |      |       |       |       |       |       |       |                   |
|-----------------------------------------------------------|--|-----------------------|--|------|------|-------|-------|-------|-------|-------|-------|-------------------|
| =====                                                     |  |                       |  |      |      |       |       |       |       |       |       |                   |
| JP1-_g_eta8:eta1/1^P_1_pole0                              |  | 0.43454 +/- 0.12395   |  | 1.00 | 0.29 | -0.03 | 0.07  | -0.38 | 0.05  | -0.07 | -0.06 | -0.12 -0.11 -0.05 |
| JP1-_g_f8:eta8/3^S_1_pole0                                |  | 0.63277 +/- 0.09806   |  |      | 1.00 | -0.82 | 0.12  | -0.30 | -0.06 | -0.10 | -0.10 | -0.10 -0.14 -0.10 |
| JP1-_g_h8:eta8/3^S_1_pole0                                |  | 0.79484 +/- 0.055941  |  |      | 1.00 | -0.18 | 0.20  | 0.17  | 0.06  | 0.11  | 0.05  | 0.07 -0.24        |
| JP1-_g_omega8:eta8/3^P_1_pole0                            |  | 0.46460 +/- 0.14332   |  |      |      | 1.00  | -0.01 | -0.68 | -0.01 | -0.07 | -0.02 | -0.01 -0.05       |
| JP1-_gamma_eta8:eta1/1^P_1 eta8:eta1/1^P_1_order0         |  | -0.38788 +/- 0.53597  |  |      |      | 1.00  | -0.00 | 0.03  | 0.05  | 0.05  | 0.04  | -0.00             |
| JP1-_gamma_omega8:eta8/3^P_1 omega8:eta8/3^P_1_order0     |  | -3.8962 +/- 0.7193    |  |      |      |       | 1.00  | 0.07  | 0.12  | 0.07  | 0.12  | 0.00              |
| JP1-_gamma_omega8:omega1/1^P_1 omega8:omega1/1^P_1_order0 |  | 9.3532 +/- 2.3422     |  |      |      |       |       | 1.00  | 0.07  | 0.39  | 0.44  | -0.00             |
| JP1-_gamma_omega8:omega1/3^P_1 omega8:omega1/3^P_1_order0 |  | 10.832 +/- 4.8997     |  |      |      |       |       |       | 1.00  | 0.15  | 0.11  | -0.00             |
| JP1-_gamma_omega8:omega1/5^P_1 omega8:omega1/5^P_1_order0 |  | 18.577 +/- 3.6587     |  |      |      |       |       |       |       | 1.00  | 0.46  | -0.00             |
| JP1-_gamma_omega8:omega8/3^P_1 omega8:omega8/3^P_1_order0 |  | 10.248 +/- 2.8899     |  |      |      |       |       |       |       |       | 1.00  | 0.00              |
| JP1-_m_pole0                                              |  | 0.0021929 +/- 0.97081 |  |      |      |       |       |       |       |       |       | 1.00              |
| =====                                                     |  |                       |  |      |      |       |       |       |       |       |       |                   |

Phase space prescription ::

irho\_sub

eta8:eta1[-] f8:eta8[+] h8:eta8[+] omega8:eta8[-] omega8:omega1[-] omega8:omega8[-] lower half-plane

sqrt(s)\_pole = (0.46077 +/- 0.0055352)  
+ (i/2)\*(-0.0038421 +/- 0.0017103) [ 0.42]

s\_pole = ( 0.2123 +/- 0.0051059)  
+ i\*(-0.0017703 +/- 0.00077958) [ 0.40]

| eta8:eta1                | f8:eta8                  | h8:eta8                  | omega8:eta8              | omega8:omega1            | omega8:omega8            |
|--------------------------|--------------------------|--------------------------|--------------------------|--------------------------|--------------------------|
| k_re= 0.1491 +/- 0.0042  | k_re= -0.0049 +/- 0.0022 | k_re= -0.0035 +/- 0.0014 | k_re= 0.1402 +/- 0.0045  | k_re= 0.0791 +/- 0.0080  | k_re= 0.0818 +/- 0.0077  |
| k_im= -0.0015 +/- 0.0007 | k_im= 0.0386 +/- 0.0144  | k_im= 0.0533 +/- 0.0102  | k_im= -0.0016 +/- 0.0007 | k_im= -0.0028 +/- 0.0014 | k_im= -0.0027 +/- 0.0013 |
| corr= [ 0.45]            | corr= [ 0.46]            | corr= [ 0.05]            | corr= [ 0.45]            | corr= [ 0.56]            | corr= [ 0.55]            |

  

| eta8:eta1/1^P_1               | f8:eta8/3^S_1                | h8:eta8/3^S_1(*)             | omega8:eta8/3^P_1             | omega8:omega1/1^P_1          | omega8:omega1/3^P_1          | omega8:omega1/5^P_1          | omega8:omega8/3^P_1          |
|-------------------------------|------------------------------|------------------------------|-------------------------------|------------------------------|------------------------------|------------------------------|------------------------------|
| g = 0.0379 +/- 0.0103         | g = 0.1850 +/- 0.0312        | g = 0.2324 +/- 0.0339        | g = 0.0373 +/- 0.0121         | g = 0.0000 +/- 0.0000        | g = 0.0000 +/- 0.0000        | g = 0.0000 +/- 0.0000        | g = 0.0000 +/- 0.0000        |
| arg(g)/pi= -0.0023 +/- 0.0124 | arg(g)/pi= 0.0080 +/- 0.0089 | arg(g)/pi= 0.0080 +/- 0.0089 | arg(g)/pi= -0.0539 +/- 0.0113 | arg(g)/pi= 0.4920 +/- 0.0089 | arg(g)/pi= 0.4920 +/- 0.0089 | arg(g)/pi= 0.4920 +/- 0.0089 | arg(g)/pi= 0.4920 +/- 0.0089 |
| g_re= 0.0379 +/- 0.0103       | g_re= 0.1849 +/- 0.0312      | g_re= 0.2323 +/- 0.0341      | g_re= 0.0367 +/- 0.0118       | g_re= 0.0000 +/- 0.0000      | g_re= 0.0000 +/- 0.0000      | g_re= 0.0000 +/- 0.0000      | g_re= 0.0000 +/- 0.0000      |
| g_im= -0.0003 +/- 0.0015      | g_im= 0.0046 +/- 0.0047      | g_im= 0.0058 +/- 0.0057      | g_im= -0.0063 +/- 0.0030      | g_im= 0.0000 +/- 0.0000      | g_im= 0.0000 +/- 0.0000      | g_im= 0.0000 +/- 0.0000      | g_im= 0.0000 +/- 0.0000      |
| corr= [-0.37]                 | corr= [-0.37]                | corr= [-0.73]                | corr= [-0.94]                 | corr= [ 0.83]                | corr= [ 0.83]                | corr= [ 0.83]                | corr= [ 0.83]                |

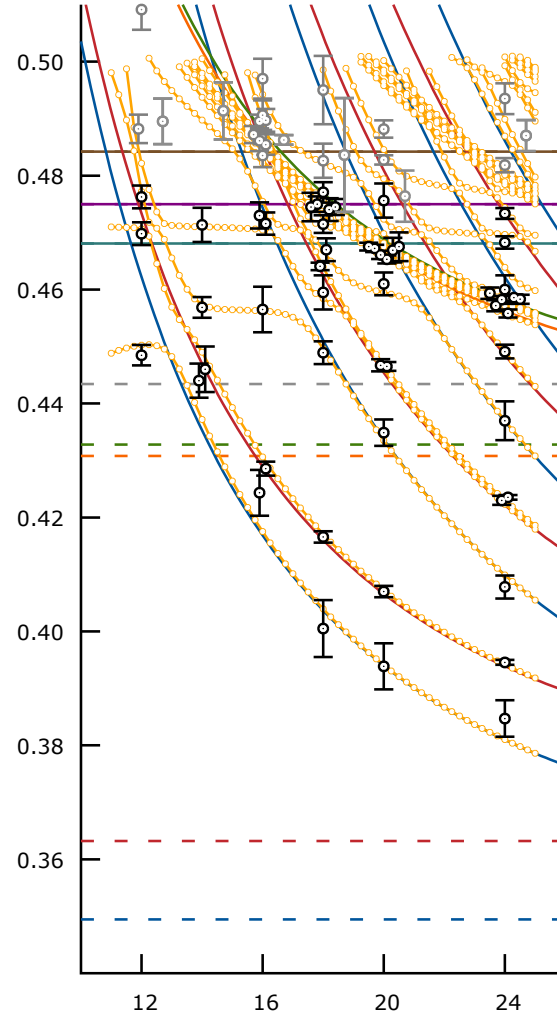

Figure 1.86: Similar to Figure 6 in the manuscript, the finite-volume spectrum, plotted as  $a_t E_{\text{cm}}$ , as a function of spatial extent  $L/a_s$ . Orange points/curves show the spectrum calculated from the amplitude given above (no uncertainties are shown). Black and grey points are the computed lattice energies on each volume, slightly displaced horizontally for clarity (black points correspond to energies used in the fit whereas grey points were not used). Two-meson non-interacting energies are shown as solid coloured curves/lines, two-meson thresholds are shown as dashed/solid horizontal lines, and the  $\eta^s \eta^s \eta^s$  threshold is shown as a dashed grey horizontal line.

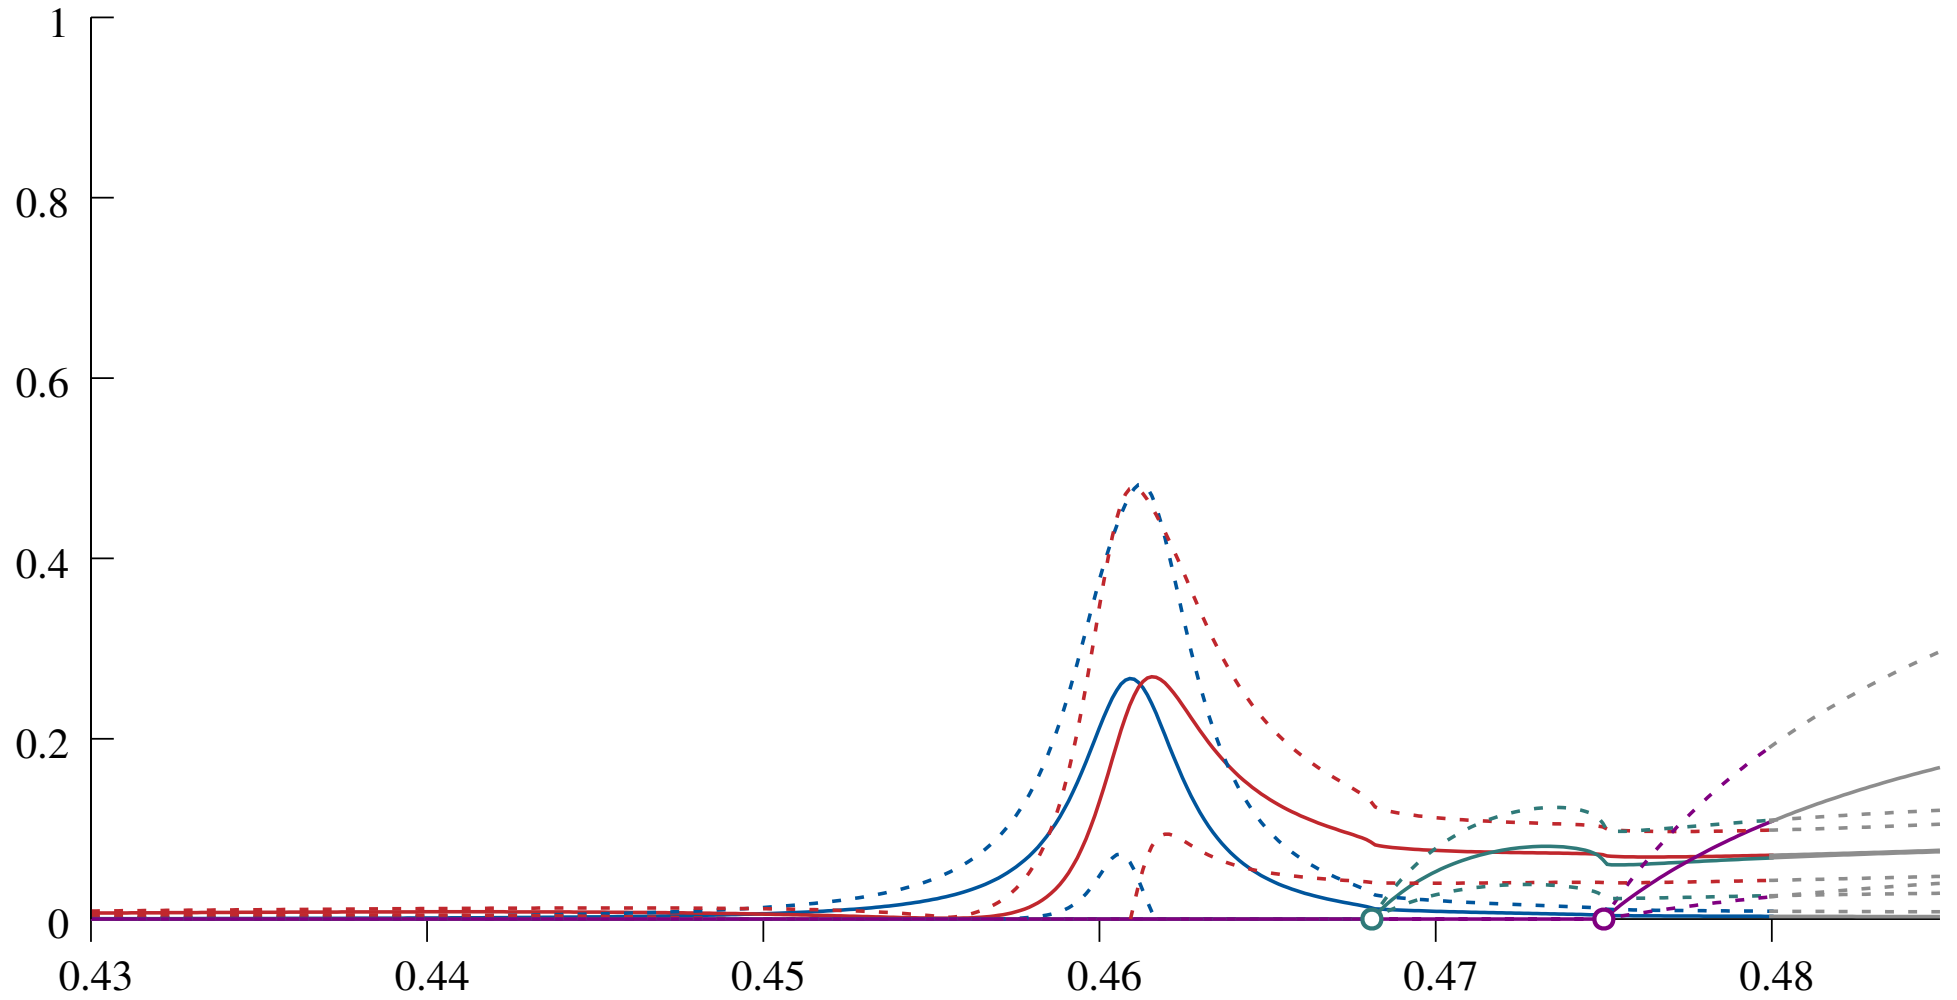

Figure 1.87: Similar to part (a) of Figure 7 in the manuscript,  $\rho_a \rho_b |t_{ab}|^2$  as a function of  $a_t E_{cm}$  for  $\eta^1 \eta^s \{^1P_1\} \rightarrow \eta^1 \eta^s \{^1P_1\}$  (blue),  $\omega^s \eta^s \{^3P_1\} \rightarrow \omega^s \eta^s \{^3P_1\}$  (red),  $f_1^s \eta^s \{^3S_1\} \rightarrow f_1^s \eta^s \{^3S_1\}$  (cyan), and  $h_1^s \eta^s \{^3S_1\} \rightarrow h_1^s \eta^s \{^3S_1\}$  (purple). Dashed lines indicate one standard deviation statistical uncertainties.

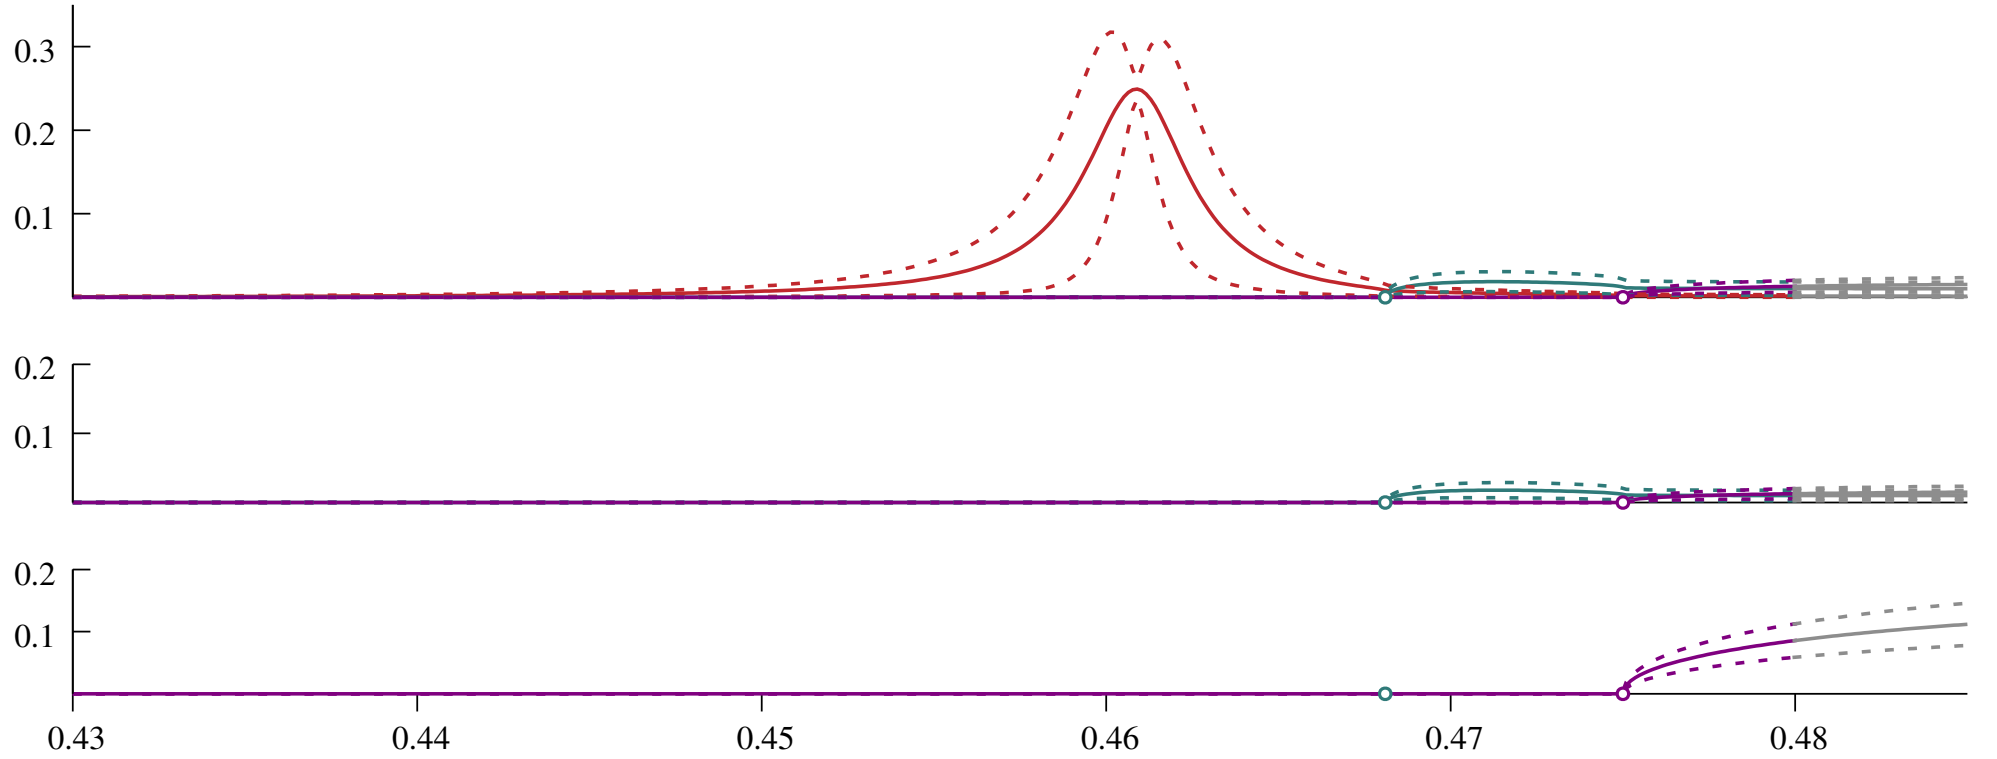

Figure 1.88: Similar to parts (b), (c) and (d) of Figure 7 in the manuscript,  $\rho_a \rho_b |t_{ab}|^2$  as a function of  $a_t E_{cm}$ . Top:  $\eta^1 \eta^s \{^1P_1\} \rightarrow \omega^s \eta^s \{^3P_1\}$  (red),  $\eta^1 \eta^s \{^1P_1\} \rightarrow f_1^s \eta^s \{^3S_1\}$  (cyan), and  $\eta^1 \eta^s \{^1P_1\} \rightarrow h_1^s \eta^s \{^3S_1\}$  (purple). Middle:  $\omega^s \eta^s \{^3P_1\} \rightarrow f_1^s \eta^s \{^3S_1\}$  (cyan), and  $\omega^s \eta^s \{^3P_1\} \rightarrow h_1^s \eta^s \{^3S_1\}$  (purple). Bottom:  $f_1^s \eta^s \{^3S_1\} \rightarrow h_1^s \eta^s \{^3S_1\}$  (purple). Dashed lines indicate one standard deviation statistical uncertainties.

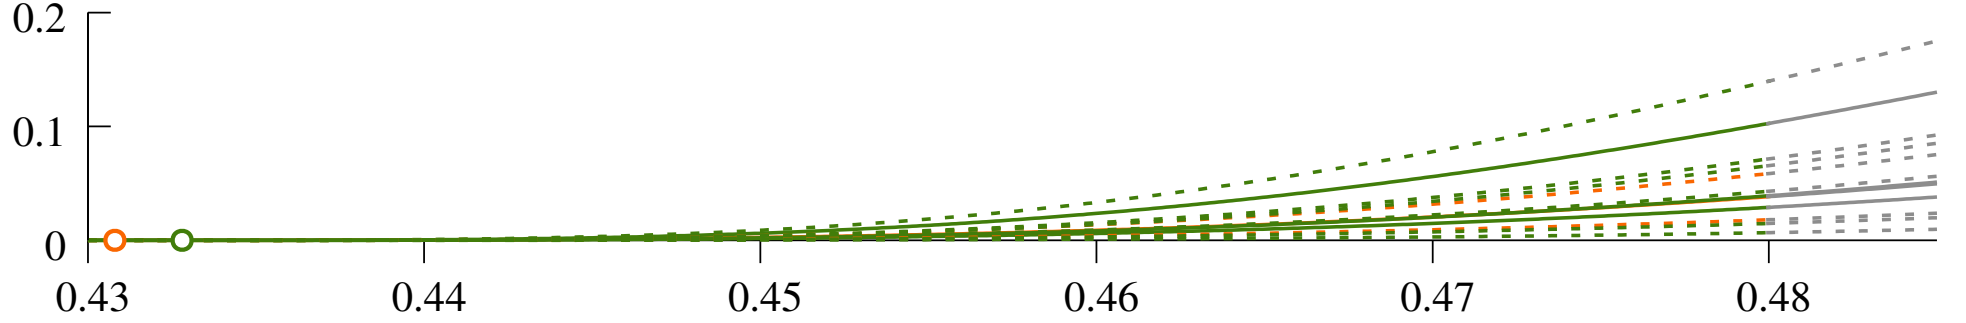

Figure 1.89: Similar to parts (e) and (f) of Figure 7 in the manuscript,  $\rho_a \rho_b |t_{ab}|^2$  as a function of  $a_t E_{cm}$  for  $\omega^s \omega^s \{^3P_1\} \rightarrow \omega^s \omega^s \{^3P_1\}$  (orange),  $\omega^1 \omega^s \{^1P_1, ^3P_1, ^5P_1\} \rightarrow \omega^s \omega^1 \{^1P_1, ^3P_1, ^5P_1\}$  (green). Dashed lines indicate one standard deviation statistical uncertainties.

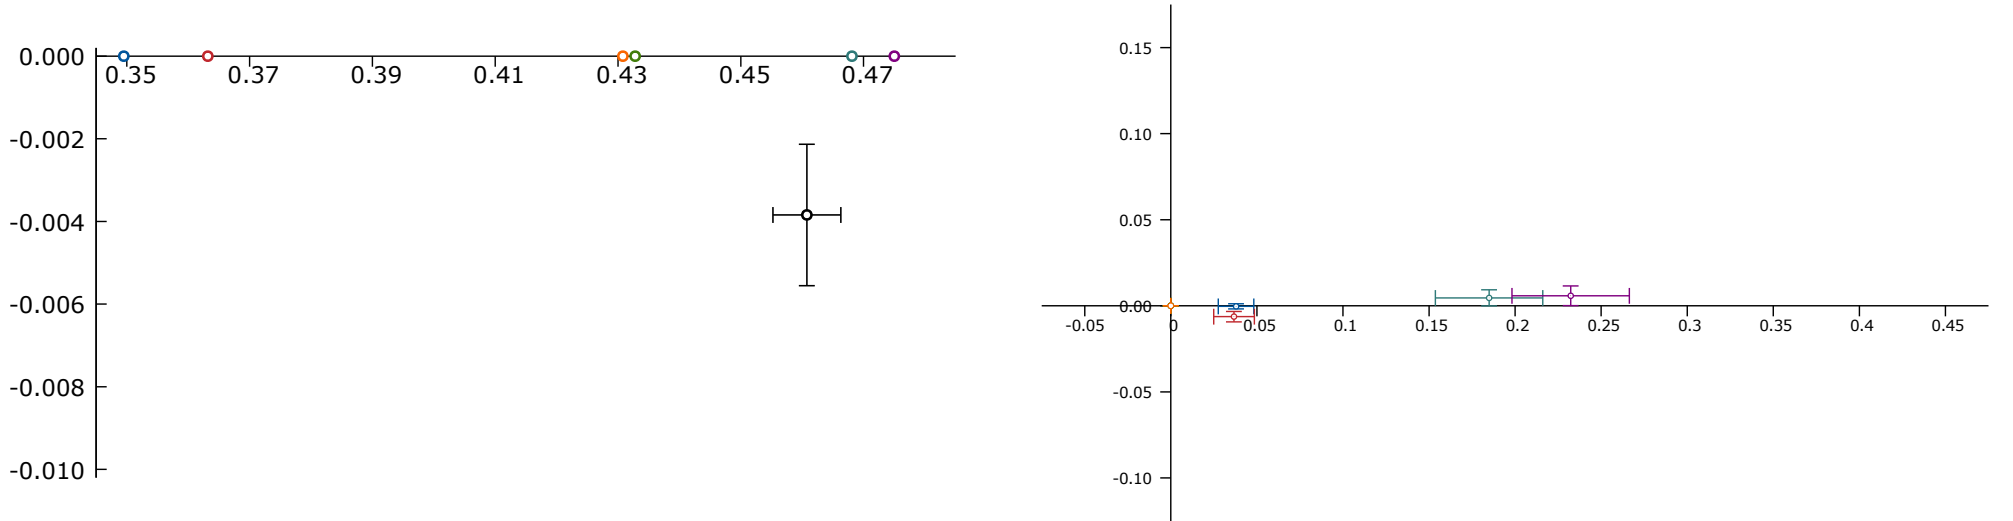

Figure 1.90: Left: Similar to Figure 13 in the manuscript, pole position on the proximal sheet (closest to physical scattering) with  $\text{Re}(a_t \sqrt{s})$  on the horizontal axis and  $2 \text{Im}(a_t \sqrt{s})$  on the vertical axis. Right: Similar to Figure 14 in the manuscript, the corresponding couplings with  $\text{Re}(a_t c)$  on the horizontal axis and  $\text{Im}(a_t c)$  on the vertical axis.

# 1.19 $\{m, g_{a,b,f}^{(0)}, \gamma_{(a,a),(b,b),(b,f),(c,c),(\partial_1,\partial_1),(\partial_2,\partial_2),(\partial_3,\partial_3),(e,e),(f,f)}^{(0)}\}(\mathbf{CM}_m)$

minimised with  $\text{chisq}/\text{nDoF} = 38.06 / (53 - 13) = 0.95$

|                                                           |  |                       |  |      |       |       |       |       |       |       |       |       |       |       |       |      |
|-----------------------------------------------------------|--|-----------------------|--|------|-------|-------|-------|-------|-------|-------|-------|-------|-------|-------|-------|------|
| JP1-_g_eta8:eta1/1^P_1_pole0                              |  | 0.29912 +/- 0.12303   |  | 1.00 | 0.83  | 0.68  | -0.59 | 0.26  | 0.70  | 0.39  | -0.07 | -0.01 | 0.03  | -0.02 | -0.04 | 0.52 |
| JP1-_g_h8:eta8/3^S_1_pole0                                |  | 0.70853 +/- 0.39151   |  | 1.00 | 0.85  | -0.32 | 0.30  | 0.86  | 0.41  | -0.21 | -0.00 | 0.06  | 0.02  | -0.02 | 0.38  |      |
| JP1-_g_omega8:eta8/3^P_1_pole0                            |  | 0.36551 +/- 0.16669   |  | 1.00 | -0.36 | 0.33  | 0.70  | 0.33  | -0.49 | 0.01  | 0.04  | 0.01  | -0.00 | 0.16  |       |      |
| JP1-_gamma_eta8:eta1/1^P_1 eta8:eta1/1^P_1_order0         |  | -4.0973 +/- 2.534     |  | 1.00 | -0.14 | -0.44 | -0.42 | -0.06 | -0.04 | 0.04  | -0.01 | -0.04 | -0.14 |       |       |      |
| JP1-_gamma_f8:eta8/3^S_1 f8:eta8/3^S_1_order0             |  | -1.9591 +/- 0.30293   |  | 1.00 | 0.34  | 0.16  | -0.13 | 0.04  | 0.07  | 0.04  | 0.04  | 0.02  |       |       |       |      |
| JP1-_gamma_h8:eta8/3^S_1 h8:eta8/3^S_1_order0             |  | 13.822 +/- 12.848     |  | 1.00 | 0.77  | 0.16  | 0.03  | 0.06  | 0.05  | 0.02  | 0.30  |       |       |       |       |      |
| JP1-_gamma_h8:eta8/3^S_1 omega8:eta8/3^P_1_order0         |  | -0.31202 +/- 4.4005   |  | 1.00 | 0.59  | 0.06  | 0.03  | 0.07  | 0.05  | 0.15  |       |       |       |       |       |      |
| JP1-_gamma_omega8:eta8/3^P_1 omega8:eta8/3^P_1_order0     |  | -5.7730 +/- 2.1265    |  | 1.00 | 0.06  | 0.03  | 0.07  | 0.07  | 0.15  |       |       |       |       |       |       |      |
| JP1-_gamma_omega8:omega1/1^P_1 omega8:omega1/1^P_1_order0 |  | 9.7045 +/- 2.3725     |  | 1.00 | 0.05  | 0.39  | 0.44  | -0.05 |       |       |       |       |       |       |       |      |
| JP1-_gamma_omega8:omega1/3^P_1 omega8:omega1/3^P_1_order0 |  | 11.270 +/- 4.9079     |  | 1.00 | 0.13  | 0.10  | 0.05  |       |       |       |       |       |       |       |       |      |
| JP1-_gamma_omega8:omega1/5^P_1 omega8:omega1/5^P_1_order0 |  | 19.139 +/- 3.734      |  | 1.00 | 0.46  | -0.06 |       |       |       |       |       |       |       |       |       |      |
| JP1-_gamma_omega8:omega8/3^P_1 omega8:omega8/3^P_1_order0 |  | 10.848 +/- 2.9158     |  | 1.00 | -0.10 |       |       |       |       |       |       |       |       |       |       |      |
| JP1-_m_pole0                                              |  | 0.46050 +/- 0.0010984 |  |      |       |       |       |       |       |       |       |       |       |       |       | 1.00 |

Phase space prescription ::

pole0\_sub

eta8:eta1[-] f8:eta8[+] h8:eta8[+] omega8:eta8[-] omega8:omega1[-] omega8:omega8[-] lower half-plane

$\text{sqrt}(s)_{\text{pole}} = (0.4943 \pm 0.012954) + (i/2) * (-0.013002 \pm 0.024845) [-0.59]$

$s_{\text{pole}} = (0.24429 \pm 0.012712) + i * (-0.0064272 \pm 0.012381) [-0.59]$

| eta8:eta1                | f8:eta8                  | h8:eta8                  | omega8:eta8              | omega8:omega1            | omega8:omega8            |
|--------------------------|--------------------------|--------------------------|--------------------------|--------------------------|--------------------------|
| k_re= 0.1738 +/- 0.0092  | k_re= -0.0749 +/- 0.0200 | k_re= -0.0645 +/- 0.0232 | k_re= 0.1661 +/- 0.0096  | k_re= 0.1195 +/- 0.0137  | k_re= 0.1213 +/- 0.0135  |
| k_im= -0.0046 +/- 0.0087 | k_im= 0.0095 +/- 0.0169  | k_im= 0.0109 +/- 0.0187  | k_im= -0.0048 +/- 0.0091 | k_im= -0.0067 +/- 0.0125 | k_im= -0.0066 +/- 0.0123 |
| corr= [-0.59]            | corr= [-0.58]            | corr= [-0.57]            | corr= [-0.59]            | corr= [-0.59]            | corr= [-0.59]            |

  

| eta8:eta1/1^P_1              | f8:eta8/3^S_1                | h8:eta8/3^S_1(*)             | omega8:eta8/3^P_1            | omega8:omega1/1^P_1          | omega8:omega1/3^P_1          | omega8:omega1/5^P_1          | omega8:omega8/3^P_1          |
|------------------------------|------------------------------|------------------------------|------------------------------|------------------------------|------------------------------|------------------------------|------------------------------|
| lg = 0.0878 +/- 0.0369       | lg = 0.0000 +/- 0.0000       | lg = 0.1801 +/- 0.0515       | lg = 0.1045 +/- 0.0630       | lg = 0.0000 +/- 0.0000       | lg = 0.0000 +/- 0.0000       | lg = 0.0000 +/- 0.0000       | lg = 0.0000 +/- 0.0000       |
| arg(g)/pi= 0.8305 +/- 0.0708 | arg(g)/pi= 0.1093 +/- 0.0672 | arg(g)/pi= 0.3907 +/- 0.0672 | arg(g)/pi= 0.8100 +/- 0.0679 | arg(g)/pi= 0.1093 +/- 0.0672 | arg(g)/pi= 0.1093 +/- 0.0672 | arg(g)/pi= 0.1093 +/- 0.0672 | arg(g)/pi= 0.1093 +/- 0.0672 |
| g_re= -0.0757 +/- 0.0274     | g_re= 0.0000 +/- 0.0000      | g_re= 0.0606 +/- 0.0401      | g_re= -0.0864 +/- 0.0444     | g_re= 0.0000 +/- 0.0000      | g_re= 0.0000 +/- 0.0000      | g_re= 0.0000 +/- 0.0000      | g_re= 0.0000 +/- 0.0000      |
| g_im= 0.0446 +/- 0.0315      | g_im= 0.0000 +/- 0.0000      | g_im= 0.1696 +/- 0.0498      | g_im= 0.0588 +/- 0.0500      | g_im= 0.0000 +/- 0.0000      | g_im= 0.0000 +/- 0.0000      | g_im= 0.0000 +/- 0.0000      | g_im= 0.0000 +/- 0.0000      |
| corr= [-0.72]                | corr= [ 0.17]                | corr= [ 0.21]                | corr= [-0.89]                | corr= [ 0.17]                | corr= [ 0.17]                | corr= [ 0.17]                | corr= [ 0.17]                |

eta8:eta1[-] f8:eta8[+] h8:eta8[+] omega8:eta8[-] omega8:omega1[-] omega8:omega8[-] lower half-plane

$\text{sqrt}(s)_{\text{pole}} = (0.46032 \pm 0.0013319) + (i/2) * (-0.0060371 \pm 0.0021155) [ 0.28]$

$s_{\text{pole}} = (0.21189 \pm 0.001228) + i * (-0.002779 \pm 0.00097159) [ 0.28]$

| eta8:eta1                | f8:eta8                  | h8:eta8                  | omega8:eta8              | omega8:omega1            | omega8:omega8            |
|--------------------------|--------------------------|--------------------------|--------------------------|--------------------------|--------------------------|
| k_re= 0.1488 +/- 0.0010  | k_re= -0.0074 +/- 0.0024 | k_re= -0.0054 +/- 0.0018 | k_re= 0.1399 +/- 0.0011  | k_re= 0.0785 +/- 0.0019  | k_re= 0.0812 +/- 0.0019  |
| k_im= -0.0023 +/- 0.0008 | k_im= 0.0401 +/- 0.0033  | k_im= 0.0543 +/- 0.0024  | k_im= -0.0024 +/- 0.0009 | k_im= -0.0044 +/- 0.0016 | k_im= -0.0043 +/- 0.0015 |
| corr= [ 0.28]            | corr= [-0.17]            | corr= [-0.22]            | corr= [ 0.28]            | corr= [ 0.30]            | corr= [ 0.30]            |

  

| eta8:eta1/1^P_1               | f8:eta8/3^S_1                | h8:eta8/3^S_1(*)              | omega8:eta8/3^P_1             | omega8:omega1/1^P_1          | omega8:omega1/3^P_1          | omega8:omega1/5^P_1          | omega8:omega8/3^P_1          |
|-------------------------------|------------------------------|-------------------------------|-------------------------------|------------------------------|------------------------------|------------------------------|------------------------------|
| lg = 0.0448 +/- 0.0106        | lg = 0.0000 +/- 0.0000       | lg = 0.3486 +/- 0.0482        | lg = 0.0510 +/- 0.0124        | lg = 0.0000 +/- 0.0000       | lg = 0.0000 +/- 0.0000       | lg = 0.0000 +/- 0.0000       | lg = 0.0000 +/- 0.0000       |
| arg(g)/pi= -0.0141 +/- 0.0536 | arg(g)/pi= 0.5123 +/- 0.0127 | arg(g)/pi= -0.0123 +/- 0.0127 | arg(g)/pi= -0.0234 +/- 0.0366 | arg(g)/pi= 0.5123 +/- 0.0127 | arg(g)/pi= 0.5123 +/- 0.0127 | arg(g)/pi= 0.5123 +/- 0.0127 | arg(g)/pi= 0.5123 +/- 0.0127 |
| g_re= 0.0448 +/- 0.0104       | g_re= -0.0000 +/- 0.0000     | g_re= 0.3483 +/- 0.0486       | g_re= 0.0509 +/- 0.0123       | g_re= -0.0000 +/- 0.0000     | g_re= -0.0000 +/- 0.0000     | g_re= -0.0000 +/- 0.0000     | g_re= -0.0000 +/- 0.0000     |
| g_im= -0.0020 +/- 0.0078      | g_im= 0.0000 +/- 0.0000      | g_im= -0.0135 +/- 0.0123      | g_im= -0.0038 +/- 0.0061      | g_im= 0.0000 +/- 0.0000      | g_im= 0.0000 +/- 0.0000      | g_im= 0.0000 +/- 0.0000      | g_im= 0.0000 +/- 0.0000      |
| corr= [-0.57]                 | corr= [-0.90]                | corr= [ 0.85]                 | corr= [-0.36]                 | corr= [-0.90]                | corr= [-0.90]                | corr= [-0.90]                | corr= [-0.90]                |

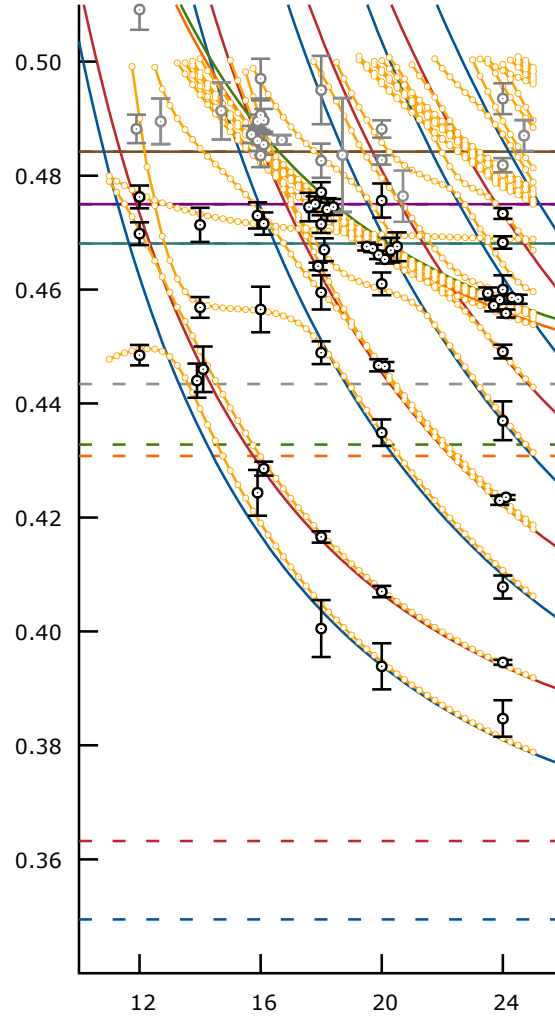

Figure 1.91: Similar to Figure 6 in the manuscript, the finite-volume spectrum, plotted as  $a_t E_{\text{cm}}$ , as a function of spatial extent  $L/a_s$ . Orange points/curves show the spectrum calculated from the amplitude given above (no uncertainties are shown). Black and grey points are the computed lattice energies on each volume, slightly displaced horizontally for clarity (black points correspond to energies used in the fit whereas grey points were not used). Two-meson non-interacting energies are shown as solid coloured curves/lines, two-meson thresholds are shown as dashed/solid horizontal lines, and the  $\eta^s \eta^s \eta^s$  threshold is shown as a dashed grey horizontal line.

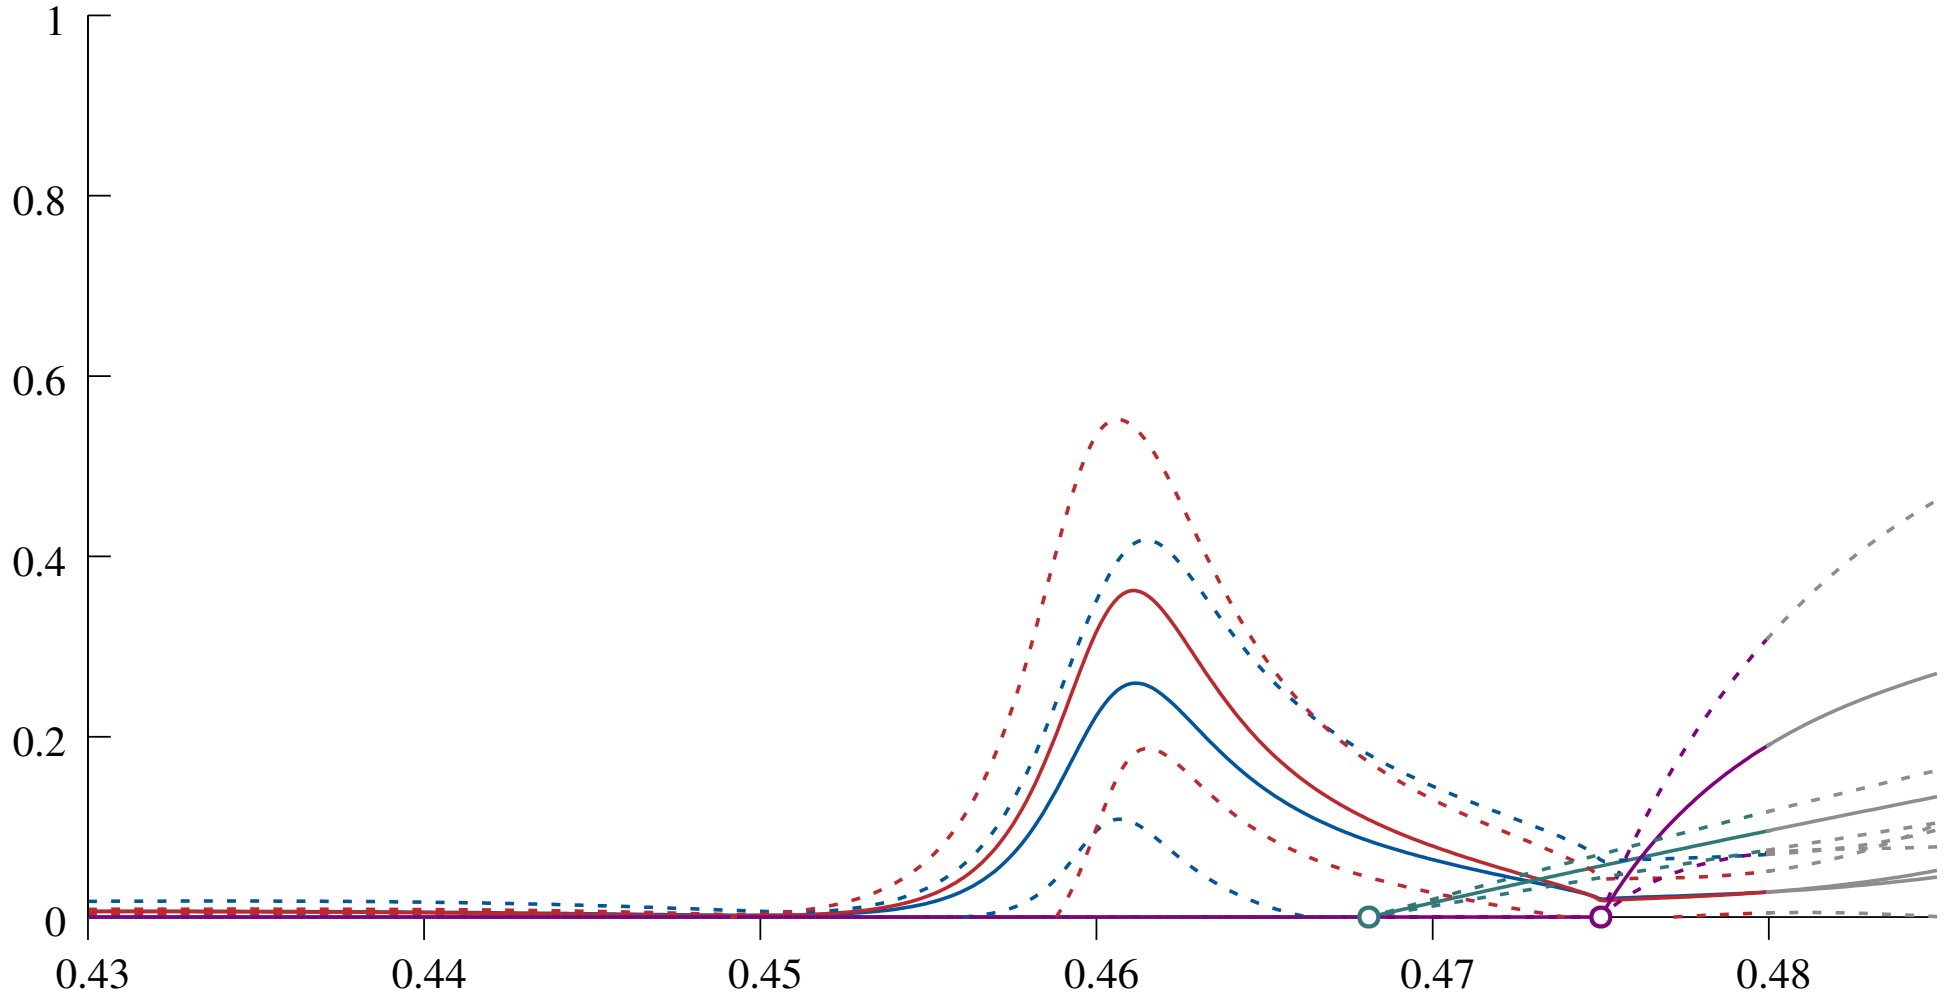

Figure 1.92: Similar to part (a) of Figure 7 in the manuscript,  $\rho_a \rho_b |t_{ab}|^2$  as a function of  $a_t E_{\text{cm}}$  for  $\eta^1 \eta^s \{^1P_1\} \rightarrow \eta^1 \eta^s \{^1P_1\}$  (blue),  $\omega^s \eta^s \{^3P_1\} \rightarrow \omega^s \eta^s \{^3P_1\}$  (red),  $f_1^s \eta^s \{^3S_1\} \rightarrow f_1^s \eta^s \{^3S_1\}$  (cyan), and  $h_1^s \eta^s \{^3S_1\} \rightarrow h_1^s \eta^s \{^3S_1\}$  (purple). Dashed lines indicate one standard deviation statistical uncertainties.

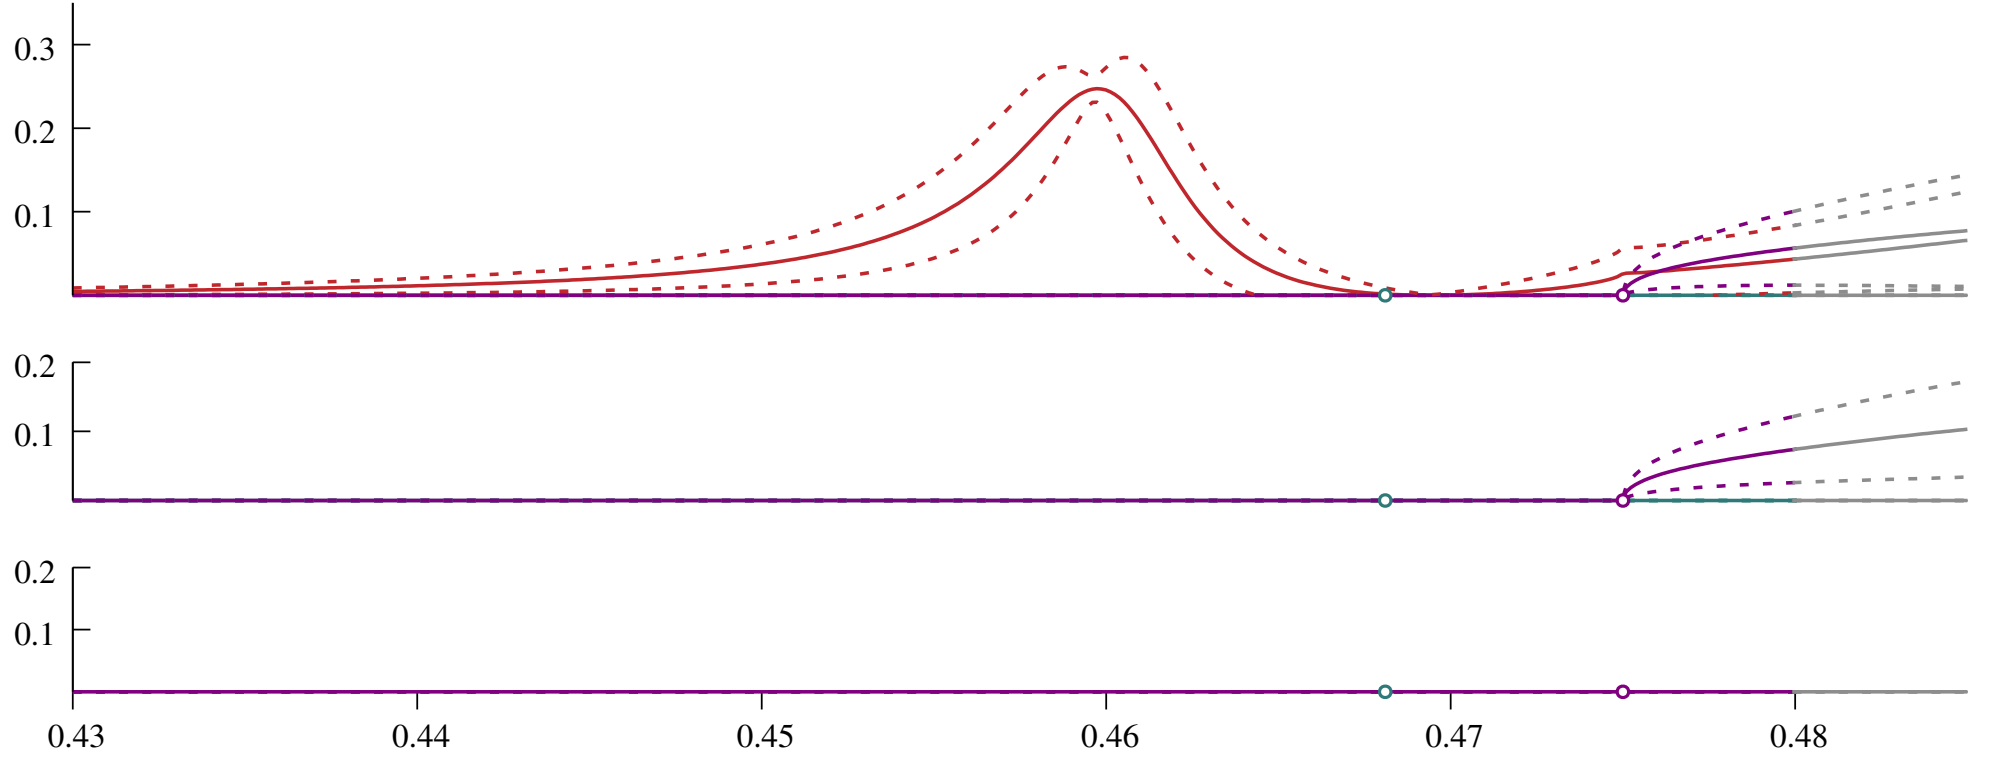

Figure 1.93: Similar to parts (b), (c) and (d) of Figure 7 in the manuscript,  $\rho_a \rho_b |t_{ab}|^2$  as a function of  $a_t E_{\text{cm}}$ . Top:  $\eta^1 \eta^s \{^1P_1\} \rightarrow \omega^s \eta^s \{^3P_1\}$  (red),  $\eta^1 \eta^s \{^1P_1\} \rightarrow f_1^s \eta^s \{^3S_1\}$  (cyan), and  $\eta^1 \eta^s \{^1P_1\} \rightarrow h_1^s \eta^s \{^3S_1\}$  (purple). Middle:  $\omega^s \eta^s \{^3P_1\} \rightarrow f_1^s \eta^s \{^3S_1\}$  (cyan), and  $\omega^s \eta^s \{^3P_1\} \rightarrow h_1^s \eta^s \{^3S_1\}$  (purple). Bottom:  $f_1^s \eta^s \{^3S_1\} \rightarrow h_1^s \eta^s \{^3S_1\}$  (purple). Dashed lines indicate one standard deviation statistical uncertainties.

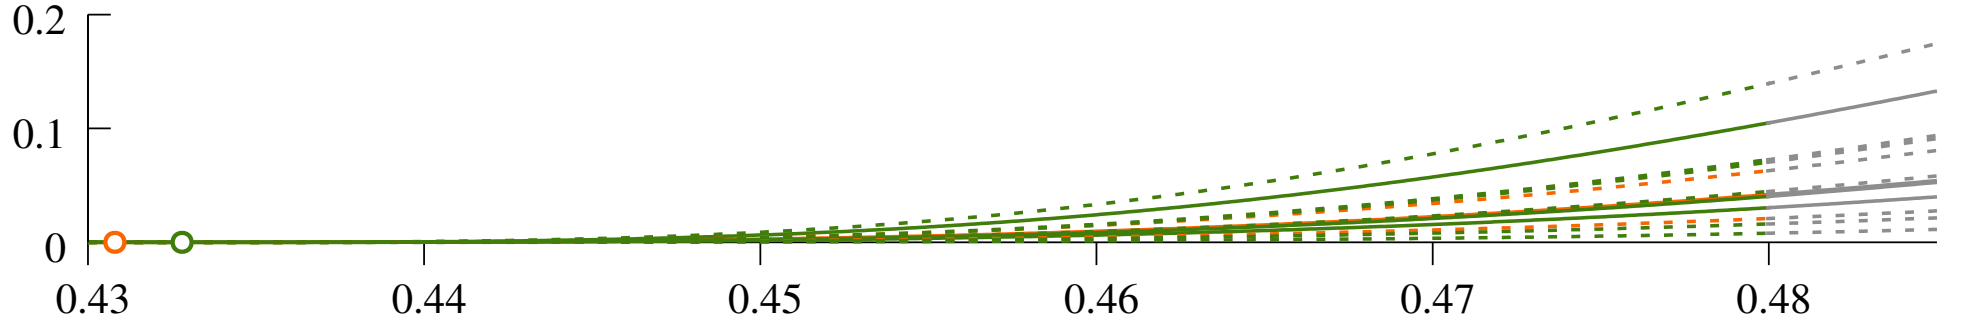

Figure 1.94: Similar to parts (e) and (f) of Figure 7 in the manuscript,  $\rho_a \rho_b |t_{ab}|^2$  as a function of  $a_t E_{cm}$  for  $\omega^s \omega^s \{^3P_1\} \rightarrow \omega^s \omega^s \{^3P_1\}$  (orange),  $\omega^1 \omega^s \{^1P_1, ^3P_1, ^5P_1\} \rightarrow \omega^s \omega^1 \{^1P_1, ^3P_1, ^5P_1\}$  (green). Dashed lines indicate one standard deviation statistical uncertainties.

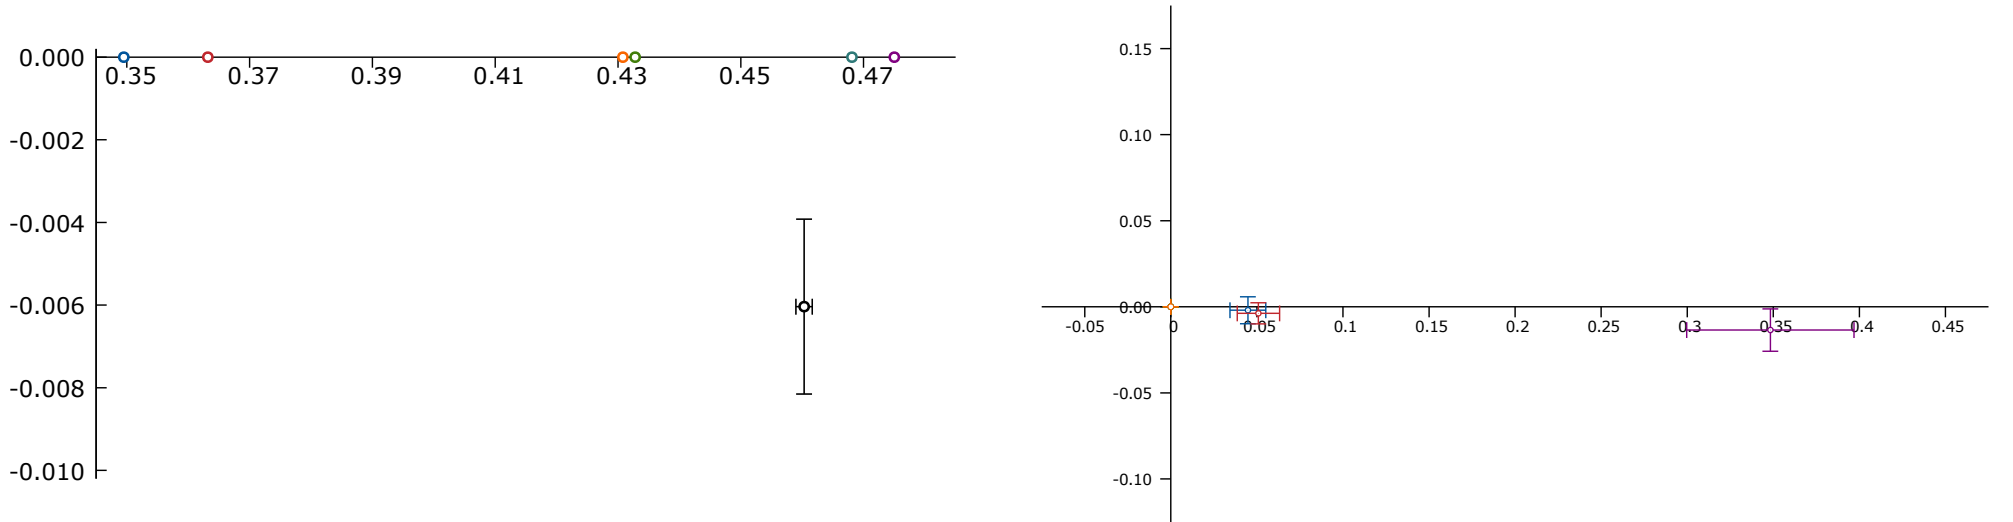

Figure 1.95: Left: Similar to Figure 13 in the manuscript, pole position on the proximal sheet (closest to physical scattering) with  $\text{Re}(a_t \sqrt{s})$  on the horizontal axis and  $2 \text{Im}(a_t \sqrt{s})$  on the vertical axis. Right: Similar to Figure 14 in the manuscript, the corresponding couplings with  $\text{Re}(a_t c)$  on the horizontal axis and  $\text{Im}(a_t c)$  on the vertical axis.

# 1.20 $\{m, g_{a,b,e,f}^{(0)}, \gamma_{(a,a),(b,b),(c,c),(\mathfrak{d}_1,\mathfrak{d}_1),(\mathfrak{d}_2,\mathfrak{d}_2),(\mathfrak{d}_3,\mathfrak{d}_3),(\mathfrak{e},f)}^{(0)}\}(\mathbf{CM}_m)$

minimised with chisq/nDoF = 43.12 / (53 - 12) = 1.05

|                                                           |  |                       |  |      |      |      |      |      |       |       |       |      |       |       |       |
|-----------------------------------------------------------|--|-----------------------|--|------|------|------|------|------|-------|-------|-------|------|-------|-------|-------|
| =====                                                     |  |                       |  |      |      |      |      |      |       |       |       |      |       |       |       |
| JP1-_g_eta8:eta1/1^P_1_pole0                              |  | 0.27430 +/- 0.16667   |  | 1.00 | 0.78 | 0.87 | 0.77 | 0.25 | -0.01 | 0.01  | -0.02 | 0.07 | -0.04 | -0.05 | 0.66  |
| JP1-_g_f8:eta8/3^S_1_pole0                                |  | 0.35276 +/- 0.25363   |  |      | 1.00 | 0.72 | 0.75 | 0.39 | -0.49 | -0.04 | -0.04 | 0.04 | -0.03 | -0.09 | 0.53  |
| JP1-_g_h8:eta8/3^S_1_pole0                                |  | 0.63048 +/- 0.51635   |  |      |      | 1.00 | 0.84 | 0.40 | 0.17  | -0.02 | 0.03  | 0.12 | 0.03  | 0.02  | 0.52  |
| JP1-_g_omega8:eta8/3^P_1_pole0                            |  | 0.28691 +/- 0.18498   |  |      |      |      | 1.00 | 0.40 | -0.04 | -0.37 | 0.01  | 0.06 | 0.01  | -0.01 | 0.39  |
| JP1-_gamma_eta8:eta1/1^P_1 eta8:eta1/1^P_1_order0         |  | -0.42567 +/- 0.60388  |  |      |      |      |      | 1.00 | -0.22 | -0.02 | 0.02  | 0.08 | 0.04  | 0.01  | 0.07  |
| JP1-_gamma_f8:eta8/3^S_1 h8:eta8/3^S_1_order0             |  | 0.61172 +/- 1.219     |  |      |      |      |      |      | 1.00  | 0.01  | 0.05  | 0.05 | 0.05  | 0.10  | -0.06 |
| JP1-_gamma_omega8:eta8/3^P_1 omega8:eta8/3^P_1_order0     |  | -3.9190 +/- 0.75271   |  |      |      |      |      |      |       | 1.00  | 0.06  | 0.11 | 0.07  | 0.12  | 0.16  |
| JP1-_gamma_omega8:omega1/1^P_1 omega8:omega1/1^P_1_order0 |  | 9.5130 +/- 2.3719     |  |      |      |      |      |      |       |       | 1.00  | 0.07 | 0.40  | 0.44  | -0.06 |
| JP1-_gamma_omega8:omega1/3^P_1 omega8:omega1/3^P_1_order0 |  | 11.196 +/- 4.9468     |  |      |      |      |      |      |       |       |       | 1.00 | 0.14  | 0.11  | 0.06  |
| JP1-_gamma_omega8:omega1/5^P_1 omega8:omega1/5^P_1_order0 |  | 18.965 +/- 3.7388     |  |      |      |      |      |      |       |       |       |      | 1.00  | 0.47  | -0.09 |
| JP1-_gamma_omega8:omega8/3^P_1 omega8:omega8/3^P_1_order0 |  | 10.476 +/- 2.9308     |  |      |      |      |      |      |       |       |       |      |       | 1.00  | -0.13 |
| JP1-_m_pole0                                              |  | 0.46107 +/- 0.0011645 |  |      |      |      |      |      |       |       |       |      |       |       | 1.00  |
| =====                                                     |  |                       |  |      |      |      |      |      |       |       |       |      |       |       |       |

Phase space prescription ::

pole0\_sub

eta8:eta1[-] f8:eta8[+] h8:eta8[+] omega8:eta8[-] omega8:omega1[-] omega8:omega8[-] lower half-plane

sqrt(s)\_pole = (0.46092 +/- 0.0011813)  
+ (i/2)\*(-0.003655 +/- 0.0015598) [ 0.19]

s\_pole = (0.21245 +/- 0.0010895)  
+ i\*(-0.0016847 +/- 0.0007181) [ 0.19]

| eta8:eta1                | f8:eta8                  | h8:eta8                  | omega8:eta8              | omega8:omega1            | omega8:omega8            |
|--------------------------|--------------------------|--------------------------|--------------------------|--------------------------|--------------------------|
| k_re= 0.1493 +/- 0.0009  | k_re= -0.0047 +/- 0.0019 | k_re= -0.0033 +/- 0.0014 | k_re= 0.1404 +/- 0.0010  | k_re= 0.0793 +/- 0.0017  | k_re= 0.0820 +/- 0.0017  |
| k_im= -0.0014 +/- 0.0006 | k_im= 0.0382 +/- 0.0031  | k_im= 0.0530 +/- 0.0022  | k_im= -0.0015 +/- 0.0006 | k_im= -0.0027 +/- 0.0011 | k_im= -0.0026 +/- 0.0011 |
| corr= [ 0.20]            | corr= [-0.08]            | corr= [-0.13]            | corr= [ 0.20]            | corr= [ 0.22]            | corr= [ 0.22]            |

  

| eta8:eta1/1^P_1               | f8:eta8/3^S_1                | h8:eta8/3^S_1(*)             | omega8:eta8/3^P_1             | omega8:omega1/1^P_1          | omega8:omega1/3^P_1          | omega8:omega1/5^P_1          | omega8:omega8/3^P_1          |
|-------------------------------|------------------------------|------------------------------|-------------------------------|------------------------------|------------------------------|------------------------------|------------------------------|
| g = 0.0373 +/- 0.0098         | g = 0.1606 +/- 0.0587        | g = 0.2872 +/- 0.0755        | g = 0.0359 +/- 0.0126         | g = 0.0000 +/- 0.0000        | g = 0.0000 +/- 0.0000        | g = 0.0000 +/- 0.0000        | g = 0.0000 +/- 0.0000        |
| arg(g)/pi= -0.0005 +/- 0.0120 | arg(g)/pi= 0.0065 +/- 0.0093 | arg(g)/pi= 0.0085 +/- 0.0057 | arg(g)/pi= -0.0523 +/- 0.0117 | arg(g)/pi= 0.4915 +/- 0.0057 | arg(g)/pi= 0.4915 +/- 0.0057 | arg(g)/pi= 0.4915 +/- 0.0057 | arg(g)/pi= 0.4915 +/- 0.0057 |
| g_re= 0.0373 +/- 0.0098       | g_re= 0.1606 +/- 0.0586      | g_re= 0.2871 +/- 0.0754      | g_re= 0.0354 +/- 0.0122       | g_re= 0.0000 +/- 0.0000      | g_re= 0.0000 +/- 0.0000      | g_re= 0.0000 +/- 0.0000      | g_re= 0.0000 +/- 0.0000      |
| g_im= -0.0001 +/- 0.0014      | g_im= 0.0033 +/- 0.0058      | g_im= 0.0077 +/- 0.0061      | g_im= -0.0059 +/- 0.0031      | g_im= 0.0000 +/- 0.0000      | g_im= 0.0000 +/- 0.0000      | g_im= 0.0000 +/- 0.0000      | g_im= 0.0000 +/- 0.0000      |
| corr= [-0.16]                 | corr= [ 0.93]                | corr= [ 0.61]                | corr= [-0.94]                 | corr= [ 0.05]                | corr= [ 0.05]                | corr= [ 0.05]                | corr= [ 0.05]                |

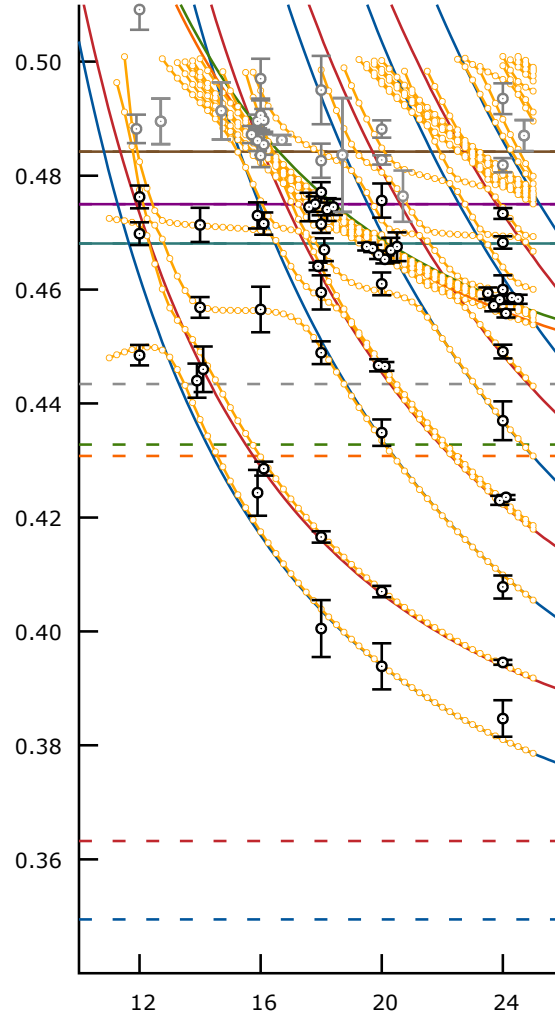

Figure 1.96: Similar to Figure 6 in the manuscript, the finite-volume spectrum, plotted as  $a_t E_{\text{cm}}$ , as a function of spatial extent  $L/a_s$ . Orange points/curves show the spectrum calculated from the amplitude given above (no uncertainties are shown). Black and grey points are the computed lattice energies on each volume, slightly displaced horizontally for clarity (black points correspond to energies used in the fit whereas grey points were not used). Two-meson non-interacting energies are shown as solid coloured curves/lines, two-meson thresholds are shown as dashed/solid horizontal lines, and the  $\eta^s \eta^s \eta^s$  threshold is shown as a dashed grey horizontal line.

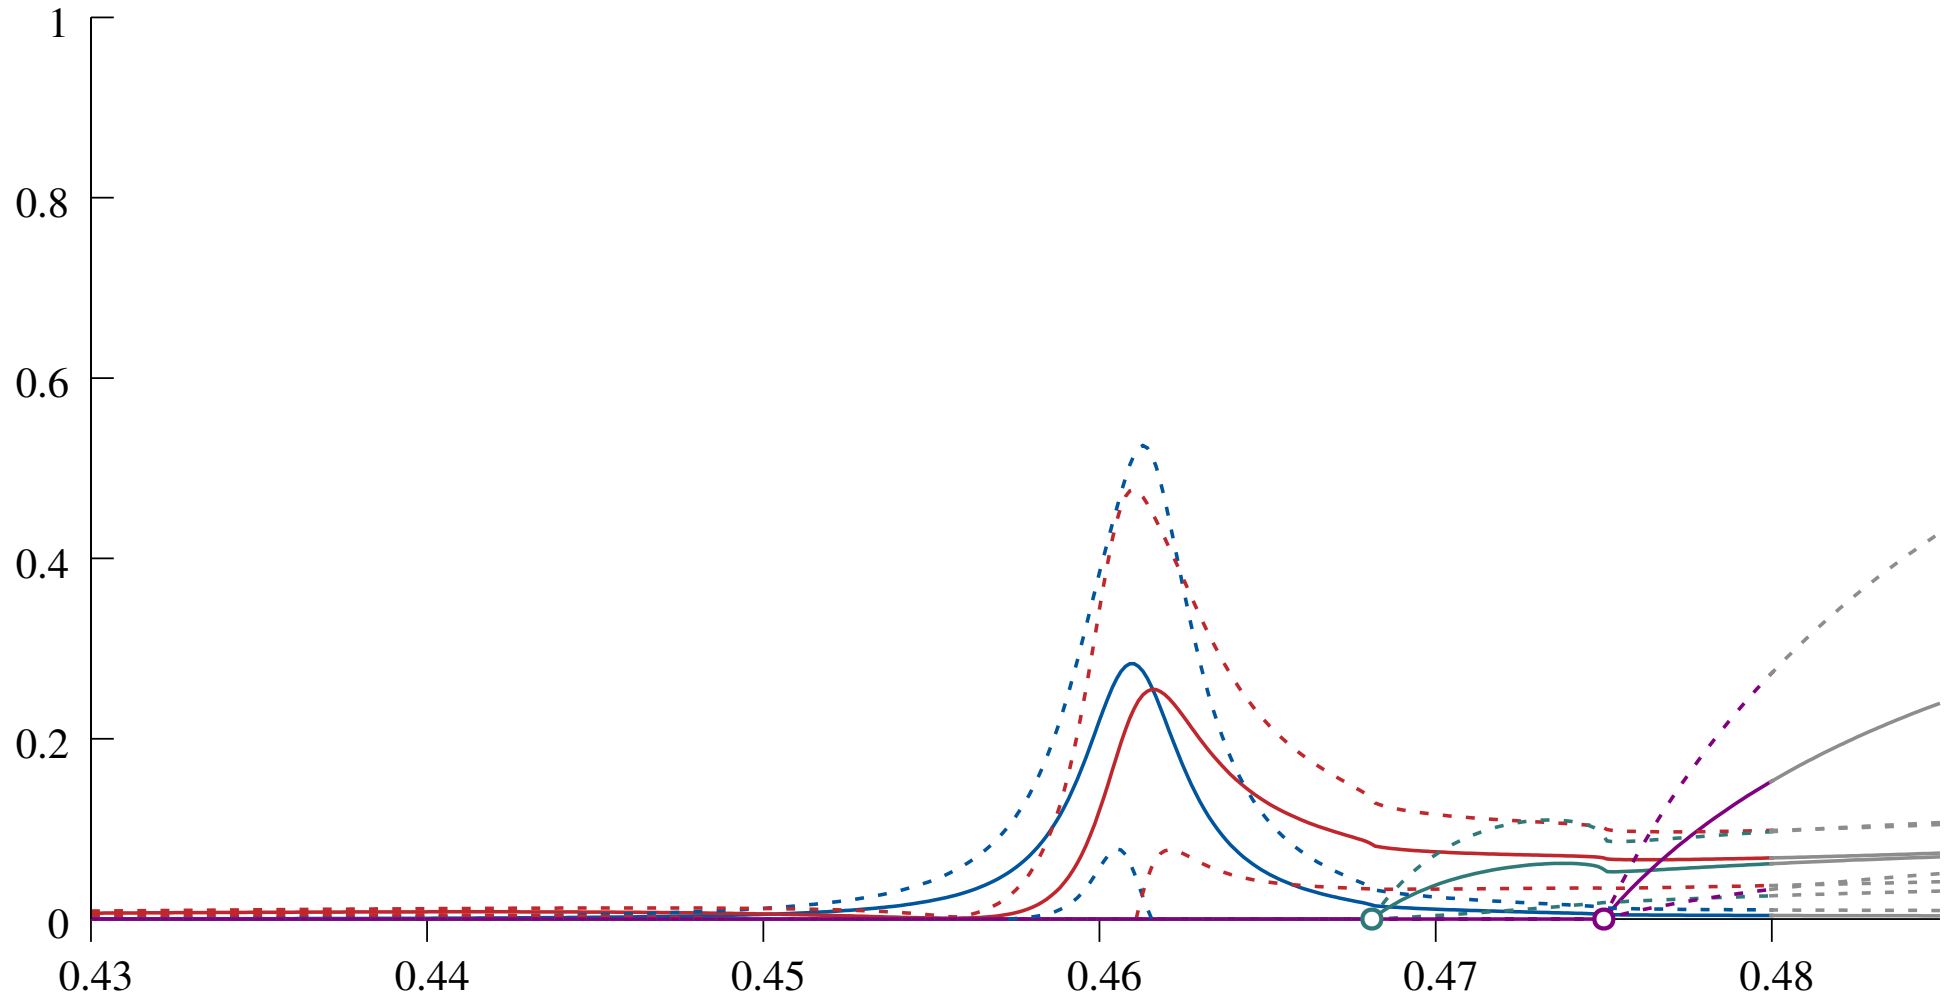

Figure 1.97: Similar to part (a) of Figure 7 in the manuscript,  $\rho_a \rho_b |t_{ab}|^2$  as a function of  $a_t E_{\text{cm}}$  for  $\eta^1 \eta^s \{^1P_1\} \rightarrow \eta^1 \eta^s \{^1P_1\}$  (blue),  $\omega^s \eta^s \{^3P_1\} \rightarrow \omega^s \eta^s \{^3P_1\}$  (red),  $f_1^s \eta^s \{^3S_1\} \rightarrow f_1^s \eta^s \{^3S_1\}$  (cyan), and  $h_1^s \eta^s \{^3S_1\} \rightarrow h_1^s \eta^s \{^3S_1\}$  (purple). Dashed lines indicate one standard deviation statistical uncertainties.

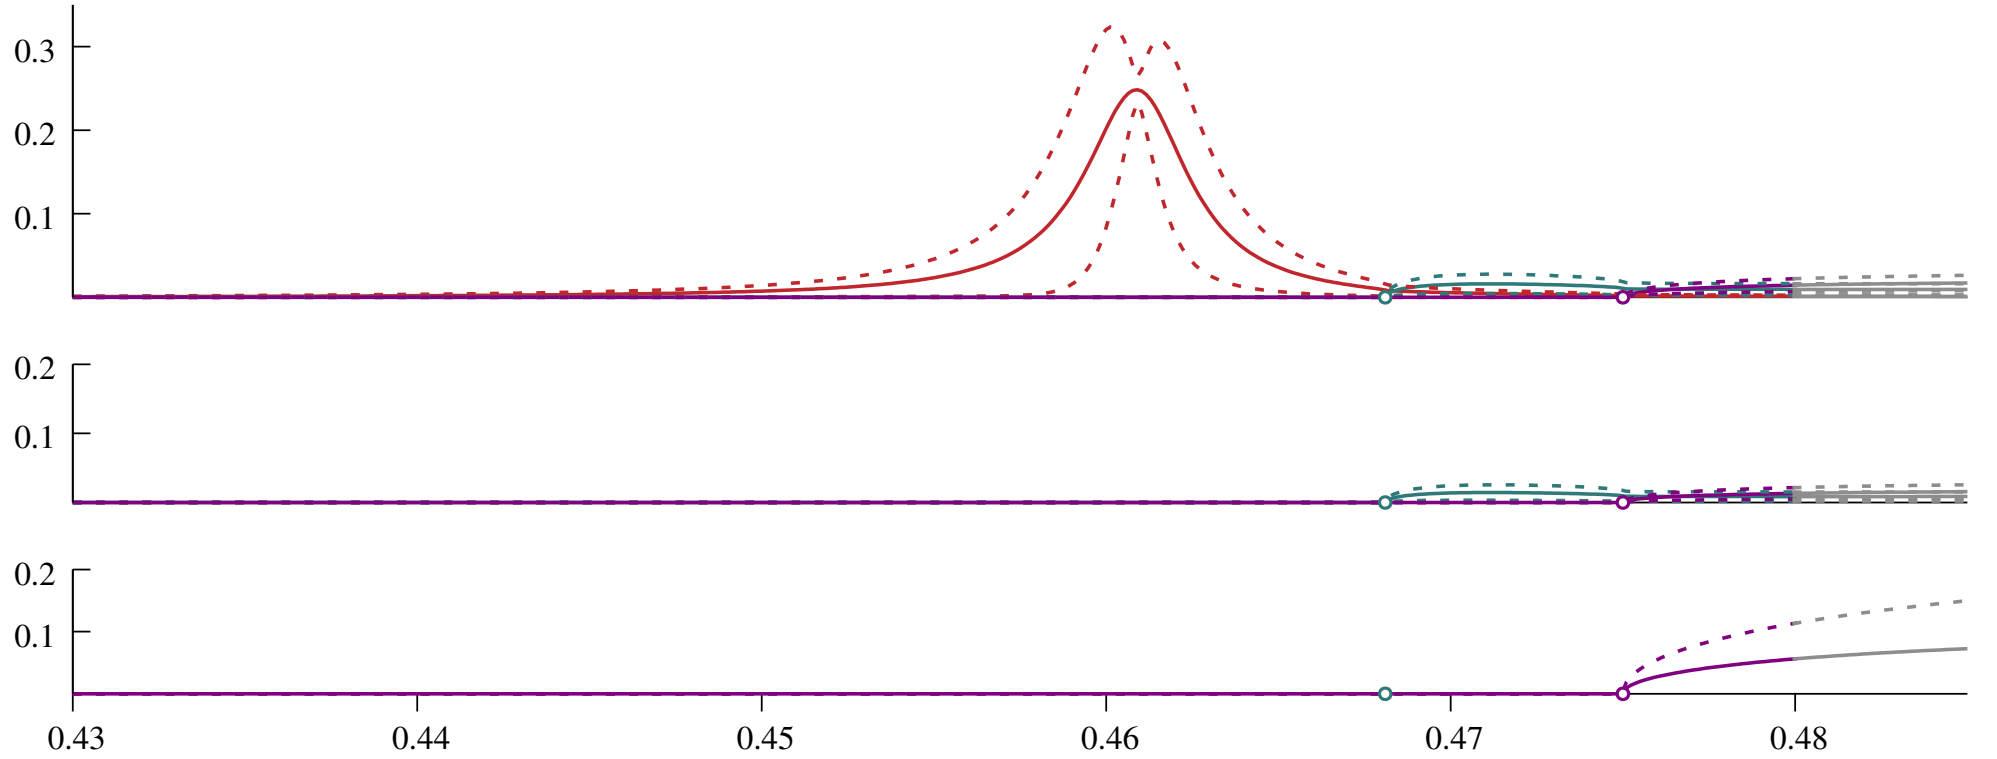

Figure 1.98: Similar to parts (b), (c) and (d) of Figure 7 in the manuscript,  $\rho_a \rho_b |t_{ab}|^2$  as a function of  $a_t E_{\text{cm}}$ . Top:  $\eta^1 \eta^s \{^1P_1\} \rightarrow \omega^s \eta^s \{^3P_1\}$  (red),  $\eta^1 \eta^s \{^1P_1\} \rightarrow f_1^s \eta^s \{^3S_1\}$  (cyan), and  $\eta^1 \eta^s \{^1P_1\} \rightarrow h_1^s \eta^s \{^3S_1\}$  (purple). Middle:  $\omega^s \eta^s \{^3P_1\} \rightarrow f_1^s \eta^s \{^3S_1\}$  (cyan), and  $\omega^s \eta^s \{^3P_1\} \rightarrow h_1^s \eta^s \{^3S_1\}$  (purple). Bottom:  $f_1^s \eta^s \{^3S_1\} \rightarrow h_1^s \eta^s \{^3S_1\}$  (purple). Dashed lines indicate one standard deviation statistical uncertainties.

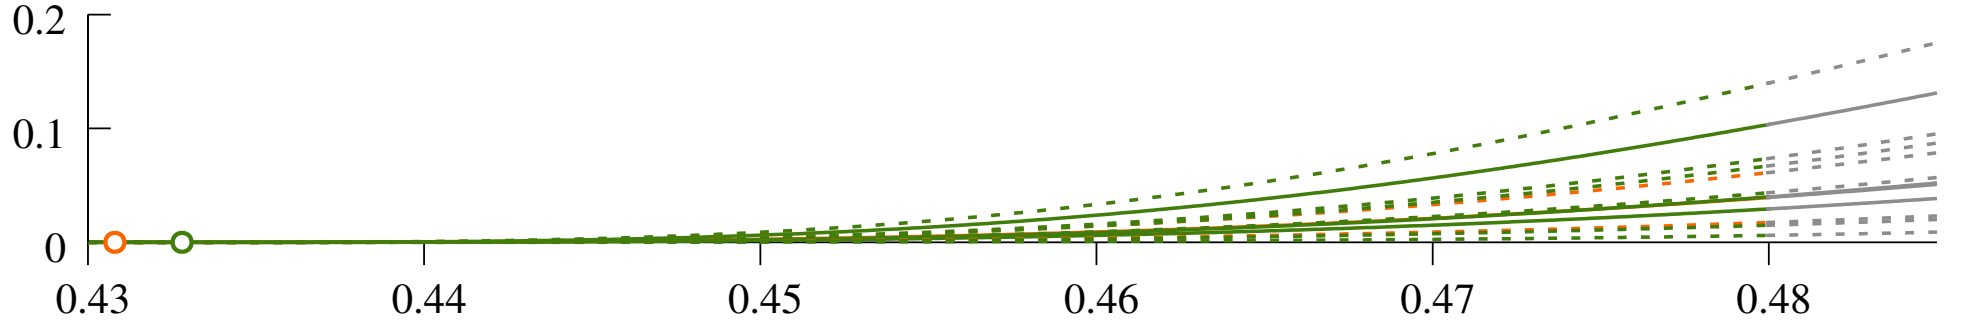

Figure 1.99: Similar to parts (e) and (f) of Figure 7 in the manuscript,  $\rho_a \rho_b |t_{ab}|^2$  as a function of  $a_t E_{cm}$  for  $\omega^s \omega^s \{^3P_1\} \rightarrow \omega^s \omega^s \{^3P_1\}$  (orange),  $\omega^1 \omega^s \{^1P_1, ^3P_1, ^5P_1\} \rightarrow \omega^s \omega^1 \{^1P_1, ^3P_1, ^5P_1\}$  (green). Dashed lines indicate one standard deviation statistical uncertainties.

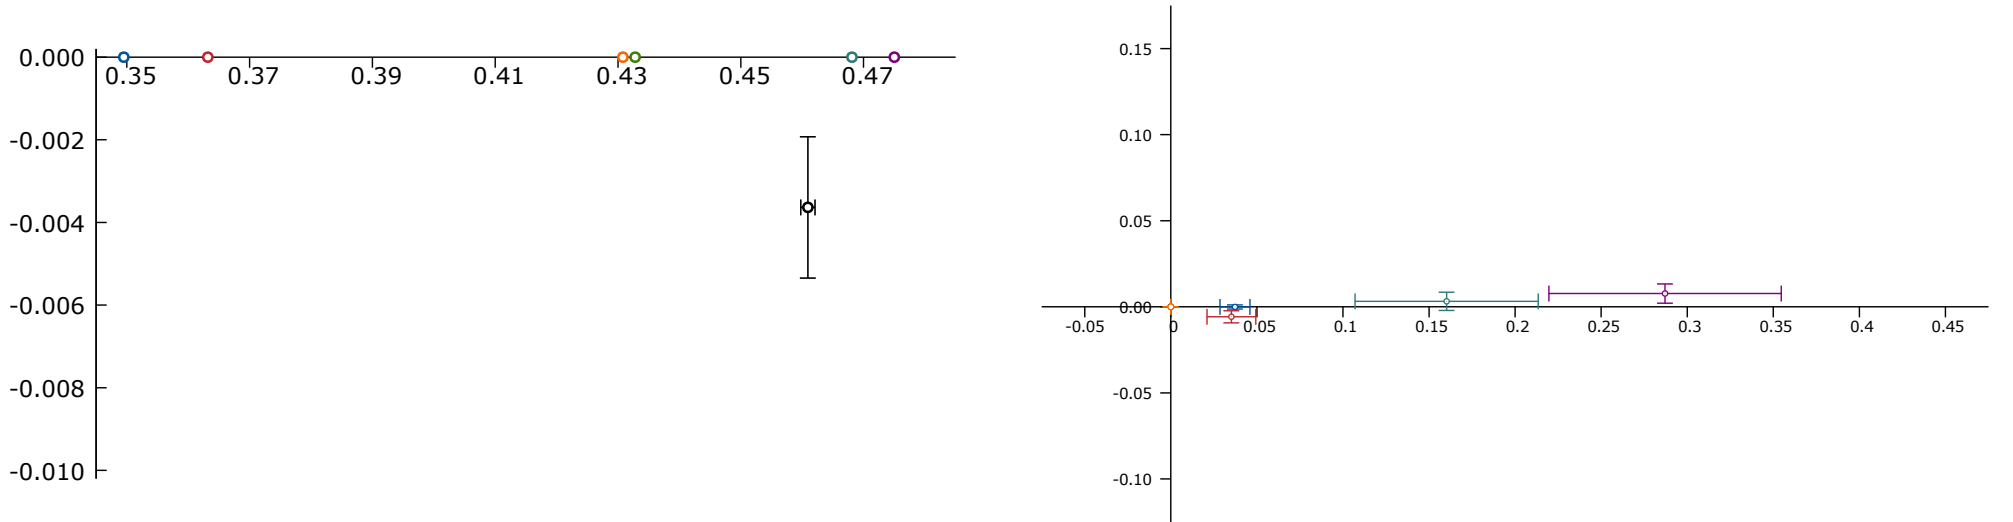

Figure 1.100: Left: Similar to Figure 13 in the manuscript, pole position on the proximal sheet (closest to physical scattering) with  $\text{Re}(a_t \sqrt{s})$  on the horizontal axis and  $2 \text{Im}(a_t \sqrt{s})$  on the vertical axis. Right: Similar to Figure 14 in the manuscript, the corresponding couplings with  $\text{Re}(a_t c)$  on the horizontal axis and  $\text{Im}(a_t c)$  on the vertical axis.

# 1.21 $\{m, g_{a,b,f}^{(0)}, \gamma_{(a,a),(b,b),(b,f),(c,c),(\partial_1,\partial_1),(\partial_2,\partial_2),(\partial_3,\partial_3),(c,c),(f,f)}^{(0)}\}(\mathbf{CM}_{thr})$

minimised with  $\text{chisq}/\text{nDoF} = 39.30 / (53 - 13) = 0.98$

|                                                           |  |                       |  |                                                                         |
|-----------------------------------------------------------|--|-----------------------|--|-------------------------------------------------------------------------|
| JP1-_g_eta8:eta1/1^P_1_pole0                              |  | 0.21668 +/- 0.058197  |  | 1.00 -0.70 -0.35 0.01 0.08 -0.70 0.26 0.36 0.02 -0.08 -0.10 -0.11 -0.04 |
| JP1-_g_h8:eta8/3^S_1_pole0                                |  | 2.3066 +/- 0.82719    |  | 1.00 0.66 -0.34 -0.10 1.00 -0.17 -0.66 -0.05 0.08 0.06 0.09 0.01        |
| JP1-_g_omega8:eta8/3^P_1_pole0                            |  | -1.1904 +/- 0.58427   |  | 1.00 -0.15 -0.35 0.66 0.62 -1.00 -0.04 0.07 0.05 0.06 0.07              |
| JP1-_gamma_eta8:eta1/1^P_1 eta8:eta1/1^P_1_order0         |  | -2.7988 +/- 1.9066    |  | 1.00 0.02 -0.34 0.19 0.16 0.10 -0.05 -0.00 -0.07 -0.02                  |
| JP1-_gamma_f8:eta8/3^S_1 f8:eta8/3^S_1_order0             |  | -1.5775 +/- 0.16764   |  | 1.00 -0.09 -0.39 0.36 0.04 0.03 0.02 0.04 -0.01                         |
| JP1-_gamma_h8:eta8/3^S_1 h8:eta8/3^S_1_order0             |  | 20.525 +/- 18.263     |  | 1.00 -0.17 -0.66 -0.05 0.08 0.06 0.09 0.03                              |
| JP1-_gamma_h8:eta8/3^S_1 omega8:eta8/3^P_1_order0         |  | -15.982 +/- 4.9665    |  | 1.00 -0.62 0.01 0.00 0.00 -0.01 0.03                                    |
| JP1-_gamma_omega8:eta8/3^P_1 omega8:eta8/3^P_1_order0     |  | 4.6465 +/- 7.7742     |  | 1.00 0.04 -0.07 -0.04 -0.05 -0.05                                       |
| JP1-_gamma_omega8:omega1/1^P_1 omega8:omega1/1^P_1_order0 |  | 11.147 +/- 5.1042     |  | 1.00 0.05 0.13 0.09 -0.00                                               |
| JP1-_gamma_omega8:omega1/3^P_1 omega8:omega1/3^P_1_order0 |  | 9.8314 +/- 2.4877     |  | 1.00 0.39 0.44 0.00                                                     |
| JP1-_gamma_omega8:omega1/5^P_1 omega8:omega1/5^P_1_order0 |  | 19.812 +/- 4.0743     |  | 1.00 0.46 0.00                                                          |
| JP1-_gamma_omega8:omega8/3^P_1 omega8:omega8/3^P_1_order0 |  | 11.099 +/- 3.0861     |  | 1.00 0.00                                                               |
| JP1-_m_pole0                                              |  | 0.0024348 +/- 0.54761 |  | 1.00                                                                    |

Phase space prescription ::

threshold\_sub

eta8:eta1[-] f8:eta8[+] h8:eta8[+] omega8:eta8[-] omega8:omega1[-] omega8:omega8[-] lower half-plane

$\sqrt{s}_{pole} = (0.46019 \pm 0.010514) + (i/2) * (-0.0065305 \pm 0.0055277) [0.93]$

$s_{pole} = (0.21176 \pm 0.0097063) + i * (-0.0030052 \pm 0.0024868) [0.92]$

| eta8:eta1                 | f8:eta8                   | h8:eta8                   | omega8:eta8               | omega8:omega1             | omega8:omega8             |
|---------------------------|---------------------------|---------------------------|---------------------------|---------------------------|---------------------------|
| k_re = 0.1487 +/- 0.0080  | k_re = -0.0079 +/- 0.0025 | k_re = -0.0058 +/- 0.0030 | k_re = 0.1398 +/- 0.0085  | k_re = 0.0783 +/- 0.0151  | k_re = 0.0810 +/- 0.0146  |
| k_im = -0.0025 +/- 0.0022 | k_im = 0.0405 +/- 0.0270  | k_im = 0.0545 +/- 0.0194  | k_im = -0.0027 +/- 0.0023 | k_im = -0.0048 +/- 0.0047 | k_im = -0.0046 +/- 0.0045 |
| corr = [0.93]             | corr = [-0.31]            | corr = [-0.80]            | corr = [0.93]             | corr = [0.94]             | corr = [0.94]             |

  

| eta8:eta1/1^P_1                | f8:eta8/3^S_1                 | h8:eta8/3^S_1(*)               | omega8:eta8/3^P_1              | omega8:omega1/1^P_1           | omega8:omega1/3^P_1           | omega8:omega1/5^P_1           | omega8:omega8/3^P_1           |
|--------------------------------|-------------------------------|--------------------------------|--------------------------------|-------------------------------|-------------------------------|-------------------------------|-------------------------------|
| g  = 0.0461 +/- 0.0147         | g  = 0.0000 +/- 0.0000        | g  = 0.3080 +/- 0.0538         | g  = 0.0532 +/- 0.0319         | g  = 0.0000 +/- 0.0000        | g  = 0.0000 +/- 0.0000        | g  = 0.0000 +/- 0.0000        | g  = 0.0000 +/- 0.0000        |
| arg(g)/pi = -0.0258 +/- 0.0533 | arg(g)/pi = 0.5201 +/- 0.0310 | arg(g)/pi = -0.0201 +/- 0.0310 | arg(g)/pi = -0.0294 +/- 0.0553 | arg(g)/pi = 0.5201 +/- 0.0310 | arg(g)/pi = 0.5201 +/- 0.0310 | arg(g)/pi = 0.5201 +/- 0.0310 | arg(g)/pi = 0.5201 +/- 0.0310 |
| g_re = 0.0459 +/- 0.0144       | g_re = -0.0000 +/- 0.0000     | g_re = 0.3074 +/- 0.0541       | g_re = 0.0529 +/- 0.0312       | g_re = -0.0000 +/- 0.0000     | g_re = -0.0000 +/- 0.0000     | g_re = -0.0000 +/- 0.0000     | g_re = -0.0000 +/- 0.0000     |
| g_im = -0.0037 +/- 0.0083      | g_im = 0.0000 +/- 0.0000      | g_im = -0.0194 +/- 0.0294      | g_im = -0.0049 +/- 0.0111      | g_im = 0.0000 +/- 0.0000      | g_im = 0.0000 +/- 0.0000      | g_im = 0.0000 +/- 0.0000      | g_im = 0.0000 +/- 0.0000      |
| corr = [-0.59]                 | corr = [-0.25]                | corr = [0.10]                  | corr = [-0.80]                 | corr = [-0.25]                | corr = [-0.25]                | corr = [-0.25]                | corr = [-0.25]                |

eta8:eta1[-] f8:eta8[+] h8:eta8[+] omega8:eta8[-] omega8:omega1[-] omega8:omega8[-] lower half-plane

$\sqrt{s}_{pole} = (0.51023 \pm 0.018872) + (i/2) * (-0.01609 \pm 0.066766) [-0.77]$

$s_{pole} = (0.26026 \pm 0.018845) + i * (-0.0082112 \pm 0.034315) [-0.76]$

| eta8:eta1                 | f8:eta8                   | h8:eta8                   | omega8:eta8               | omega8:omega1             | omega8:omega8             |
|---------------------------|---------------------------|---------------------------|---------------------------|---------------------------|---------------------------|
| k_re = 0.1849 +/- 0.0132  | k_re = -0.0959 +/- 0.0250 | k_re = -0.0877 +/- 0.0275 | k_re = 0.1776 +/- 0.0137  | k_re = 0.1353 +/- 0.0187  | k_re = 0.1368 +/- 0.0185  |
| k_im = -0.0055 +/- 0.0228 | k_im = 0.0097 +/- 0.0384  | k_im = 0.0104 +/- 0.0410  | k_im = -0.0057 +/- 0.0236 | k_im = -0.0076 +/- 0.0308 | k_im = -0.0075 +/- 0.0305 |
| corr = [-0.78]            | corr = [-0.80]            | corr = [-0.81]            | corr = [-0.78]            | corr = [-0.79]            | corr = [-0.79]            |

  

| eta8:eta1/1^P_1               | f8:eta8/3^S_1                 | h8:eta8/3^S_1(*)              | omega8:eta8/3^P_1             | omega8:omega1/1^P_1           | omega8:omega1/3^P_1           | omega8:omega1/5^P_1           | omega8:omega8/3^P_1           |
|-------------------------------|-------------------------------|-------------------------------|-------------------------------|-------------------------------|-------------------------------|-------------------------------|-------------------------------|
| g  = 0.0697 +/- 0.0188        | g  = 0.0000 +/- 0.0000        | g  = 0.2692 +/- 0.0371        | g  = 0.1849 +/- 0.0544        | g  = 0.0000 +/- 0.0000        | g  = 0.0000 +/- 0.0000        | g  = 0.0000 +/- 0.0000        | g  = 0.0000 +/- 0.0000        |
| arg(g)/pi = 0.7743 +/- 0.0860 | arg(g)/pi = 0.1035 +/- 0.0566 | arg(g)/pi = 0.3965 +/- 0.0566 | arg(g)/pi = 0.7508 +/- 0.1813 | arg(g)/pi = 0.1035 +/- 0.0566 | arg(g)/pi = 0.1035 +/- 0.0566 | arg(g)/pi = 0.1035 +/- 0.0566 | arg(g)/pi = 0.1035 +/- 0.0566 |
| g_re = -0.0529 +/- 0.0177     | g_re = 0.0000 +/- 0.0000      | g_re = 0.0860 +/- 0.0552      | g_re = -0.1310 +/- 0.0393     | g_re = 0.0000 +/- 0.0000      | g_re = 0.0000 +/- 0.0000      | g_re = 0.0000 +/- 0.0000      | g_re = 0.0000 +/- 0.0000      |
| g_im = 0.0454 +/- 0.0199      | g_im = 0.0000 +/- 0.0000      | g_im = 0.2551 +/- 0.0243      | g_im = 0.1304 +/- 0.1119      | g_im = 0.0000 +/- 0.0000      | g_im = 0.0000 +/- 0.0000      | g_im = 0.0000 +/- 0.0000      | g_im = 0.0000 +/- 0.0000      |
| corr = [-0.02]                | corr = [-0.85]                | corr = [0.70]                 | corr = [0.93]                 | corr = [-0.85]                | corr = [-0.85]                | corr = [-0.85]                | corr = [-0.85]                |

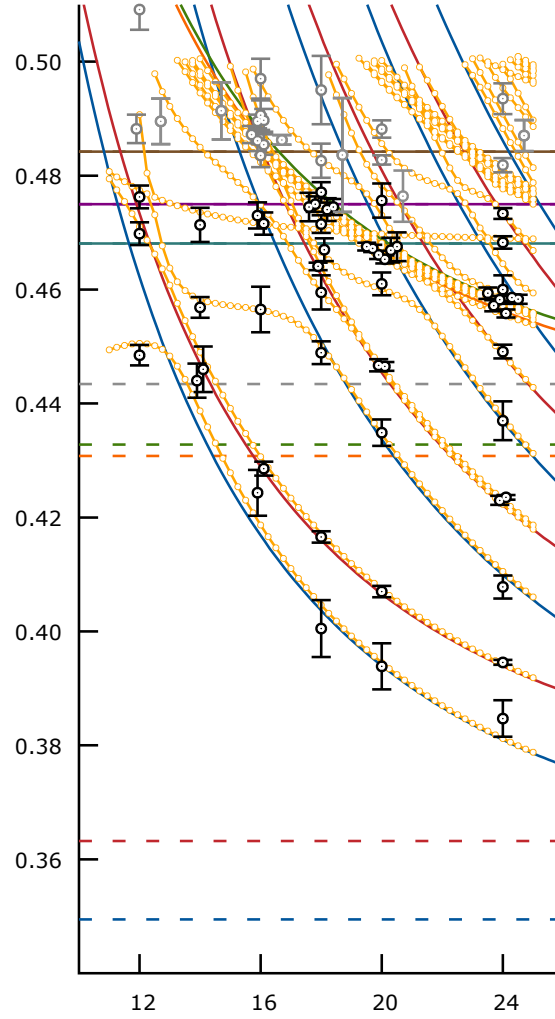

Figure 1.101: Similar to Figure 6 in the manuscript, the finite-volume spectrum, plotted as  $a_t E_{\text{cm}}$ , as a function of spatial extent  $L/a_s$ . Orange points/curves show the spectrum calculated from the amplitude given above (no uncertainties are shown). Black and grey points are the computed lattice energies on each volume, slightly displaced horizontally for clarity (black points correspond to energies used in the fit whereas grey points were not used). Two-meson non-interacting energies are shown as solid coloured curves/lines, two-meson thresholds are shown as dashed/solid horizontal lines, and the  $\eta^s \eta^s \eta^s$  threshold is shown as a dashed grey horizontal line.

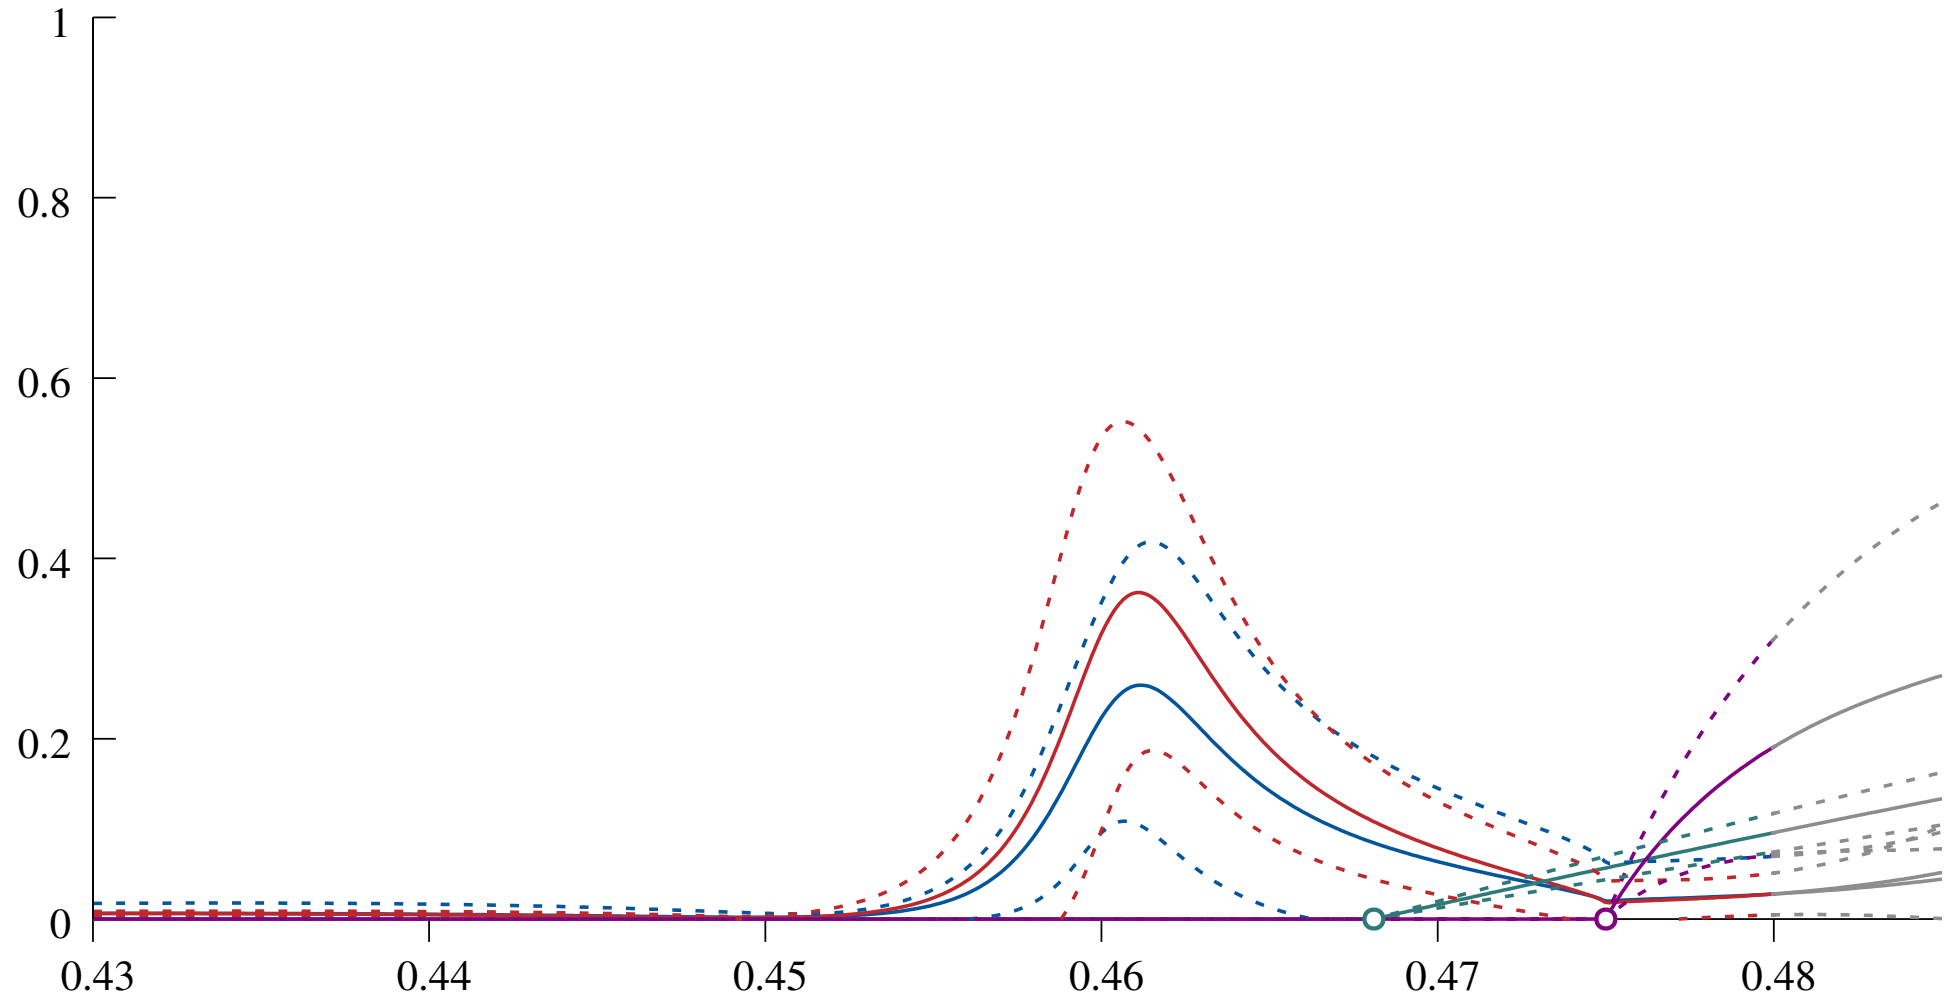

Figure 1.102: Similar to part (a) of Figure 7 in the manuscript,  $\rho_a \rho_b |t_{ab}|^2$  as a function of  $a_t E_{\text{cm}}$  for  $\eta^1 \eta^s \{^1P_1\} \rightarrow \eta^1 \eta^s \{^1P_1\}$  (blue),  $\omega^s \eta^s \{^3P_1\} \rightarrow \omega^s \eta^s \{^3P_1\}$  (red),  $f_1^s \eta^s \{^3S_1\} \rightarrow f_1^s \eta^s \{^3S_1\}$  (cyan), and  $h_1^s \eta^s \{^3S_1\} \rightarrow h_1^s \eta^s \{^3S_1\}$  (purple). Dashed lines indicate one standard deviation statistical uncertainties.

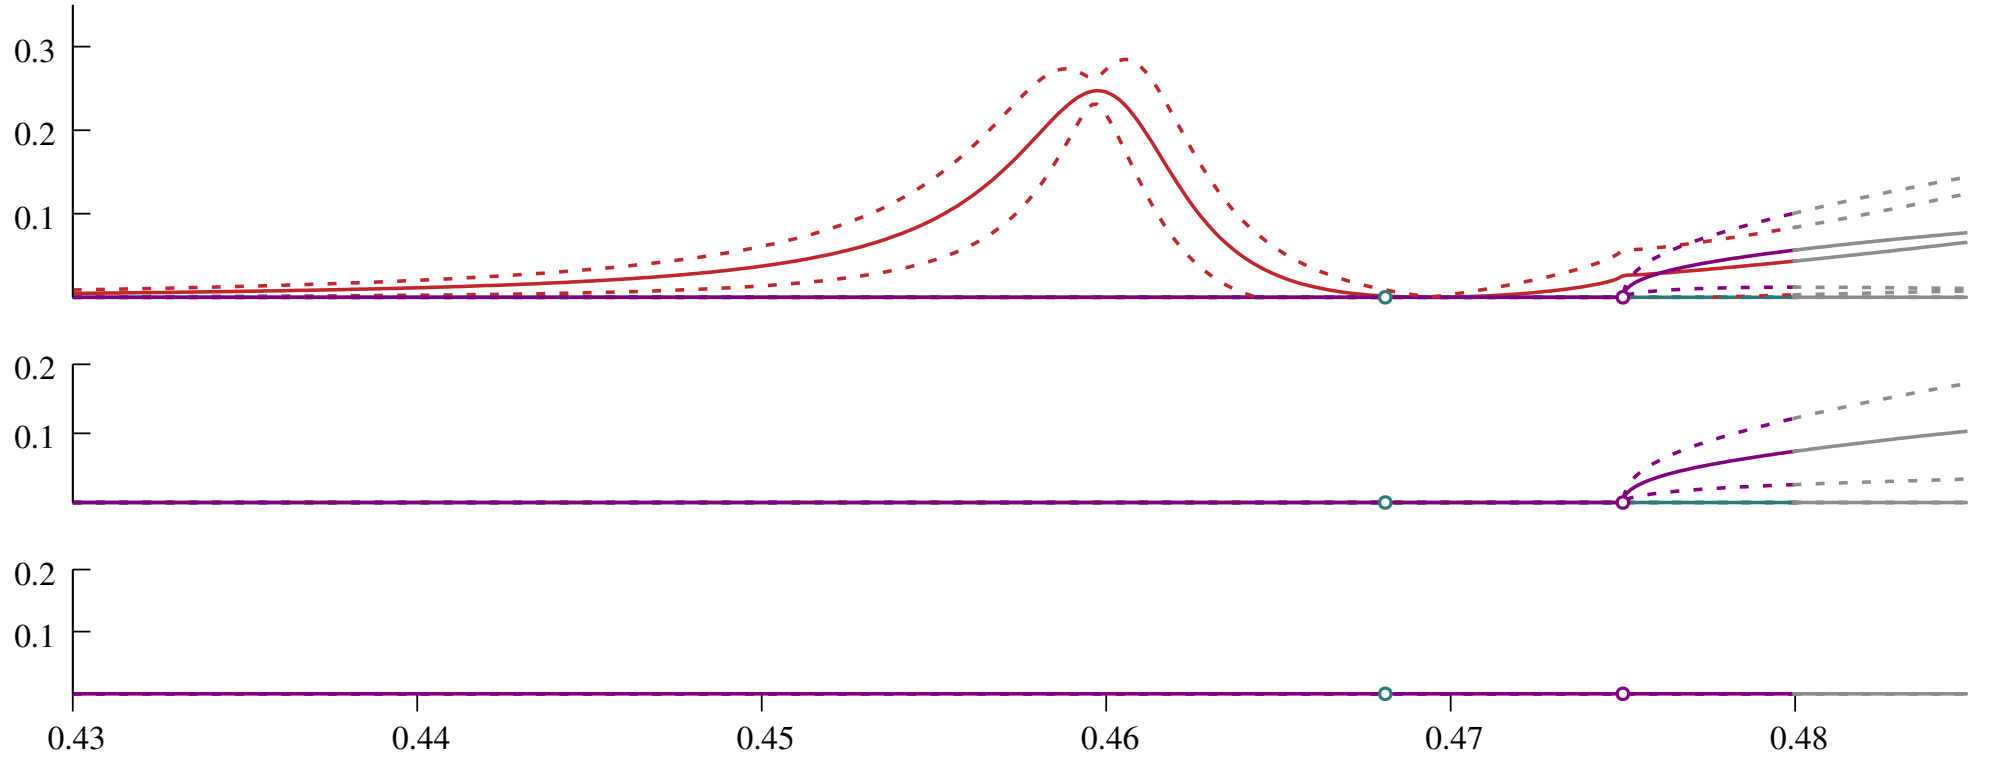

Figure 1.103: Similar to parts (b), (c) and (d) of Figure 7 in the manuscript,  $\rho_a \rho_b |t_{ab}|^2$  as a function of  $a_t E_{\text{cm}}$ . Top:  $\eta^1 \eta^s \{^1P_1\} \rightarrow \omega^s \eta^s \{^3P_1\}$  (red),  $\eta^1 \eta^s \{^1P_1\} \rightarrow f_1^s \eta^s \{^3S_1\}$  (cyan), and  $\eta^1 \eta^s \{^1P_1\} \rightarrow h_1^s \eta^s \{^3S_1\}$  (purple). Middle:  $\omega^s \eta^s \{^3P_1\} \rightarrow f_1^s \eta^s \{^3S_1\}$  (cyan), and  $\omega^s \eta^s \{^3P_1\} \rightarrow h_1^s \eta^s \{^3S_1\}$  (purple). Bottom:  $f_1^s \eta^s \{^3S_1\} \rightarrow h_1^s \eta^s \{^3S_1\}$  (purple). Dashed lines indicate one standard deviation statistical uncertainties.

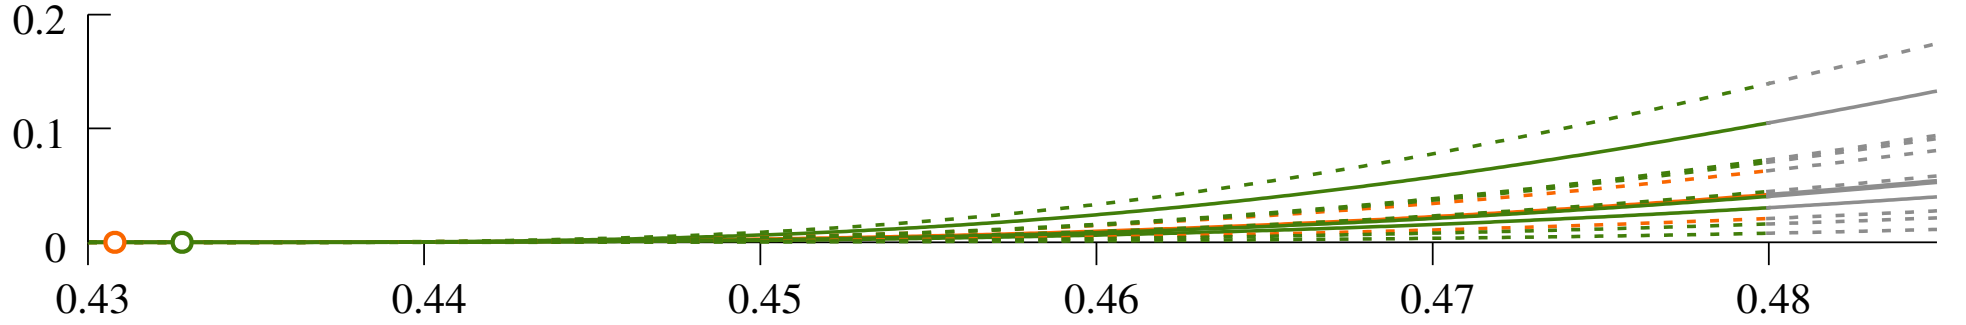

Figure 1.104: Similar to parts (e) and (f) of Figure 7 in the manuscript,  $\rho_a \rho_b |t_{ab}|^2$  as a function of  $a_t E_{cm}$  for  $\omega^s \omega^s \{^3P_1\} \rightarrow \omega^s \omega^s \{^3P_1\}$  (orange),  $\omega^1 \omega^s \{^1P_1, ^3P_1, ^5P_1\} \rightarrow \omega^s \omega^1 \{^1P_1, ^3P_1, ^5P_1\}$  (green). Dashed lines indicate one standard deviation statistical uncertainties.

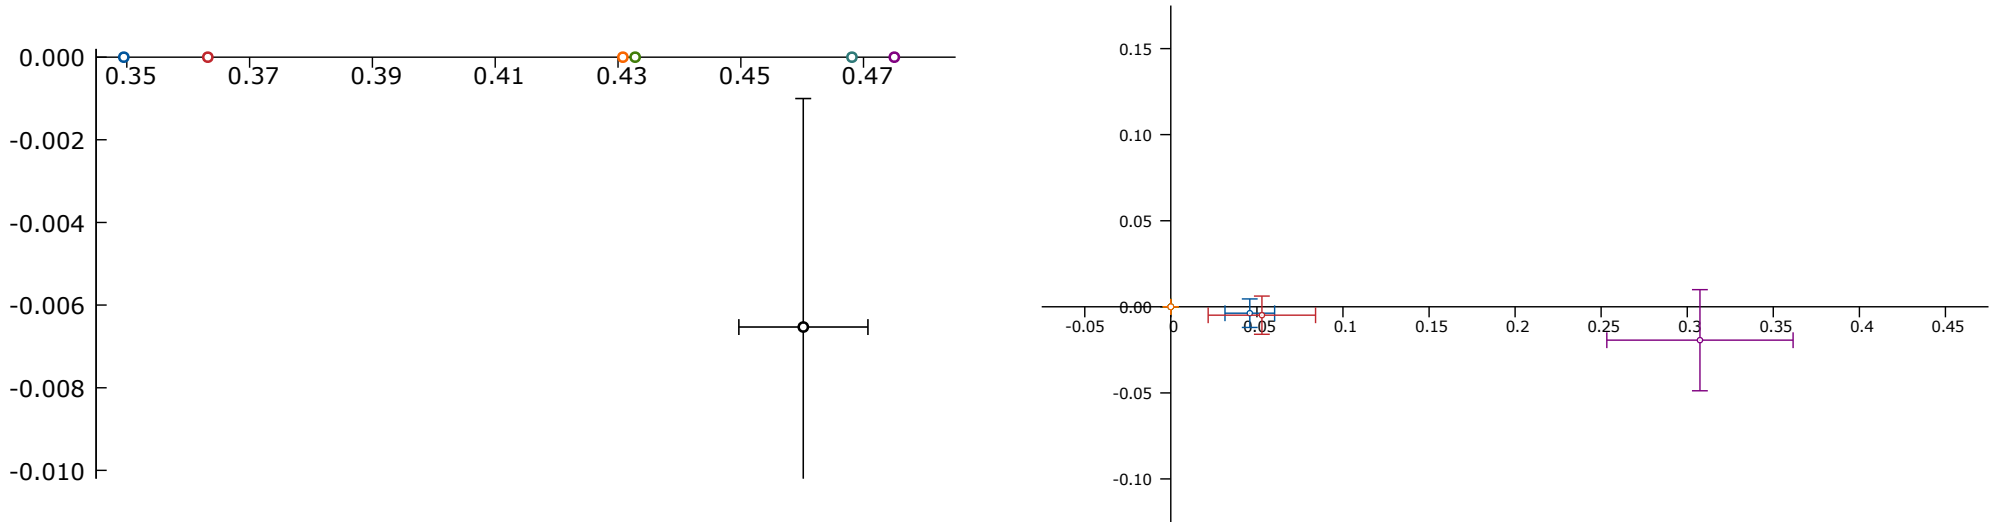

Figure 1.105: Left: Similar to Figure 13 in the manuscript, pole position on the proximal sheet (closest to physical scattering) with  $\text{Re}(a_t \sqrt{s})$  on the horizontal axis and  $2 \text{Im}(a_t \sqrt{s})$  on the vertical axis. Right: Similar to Figure 14 in the manuscript, the corresponding couplings with  $\text{Re}(a_t c)$  on the horizontal axis and  $\text{Im}(a_t c)$  on the vertical axis.

## 1.22 $\{m, g_{a,b,f}^{(0)}, \gamma_{(a,a),(b,b),(c,c),(d_1,d_1),(d_2,d_2),(d_3,d_3),(e,e)}, \gamma_{(a,a)}^{(1)}\}(\mathbf{CM}_m)$

minimised with chisq/nDoF = 41.74 / (53 - 12) = 1.02

|                                                           |  |                       |  |      |      |      |       |       |       |       |       |       |       |       |       |
|-----------------------------------------------------------|--|-----------------------|--|------|------|------|-------|-------|-------|-------|-------|-------|-------|-------|-------|
| =====                                                     |  |                       |  |      |      |      |       |       |       |       |       |       |       |       |       |
| JP1-_g_eta8:eta1/1^P_1_pole0_order0                       |  | 0.35654 +/- 0.32147   |  | 1.00 | 0.94 | 0.88 | -0.25 | 0.26  | 0.39  | -0.03 | -0.02 | 0.04  | -0.04 | -0.04 | 0.66  |
| JP1-_g_h8:eta8/3^S_1_pole0_order0                         |  | 0.97941 +/- 0.96415   |  |      | 1.00 | 0.93 | -0.09 | 0.10  | 0.42  | -0.06 | -0.01 | 0.06  | -0.01 | -0.02 | 0.55  |
| JP1-_g_omega8:eta8/3^P_1_pole0_order0                     |  | 0.30997 +/- 0.28314   |  |      |      | 1.00 | -0.09 | 0.10  | 0.40  | -0.25 | 0.01  | 0.05  | 0.00  | -0.00 | 0.45  |
| JP1-_gamma_eta8:eta1/1^P_1 eta8:eta1/1^P_1_order0         |  | -23.867 +/- 12.42     |  |      |      |      | 1.00  | -1.00 | -0.14 | 0.02  | -0.02 | 0.03  | -0.00 | -0.02 | -0.17 |
| JP1-_gamma_eta8:eta1/1^P_1 eta8:eta1/1^P_1_order1         |  | 115.54 +/- 56.974     |  |      |      |      |       | 1.00  | 0.17  | -0.02 | 0.02  | -0.02 | 0.00  | 0.02  | 0.17  |
| JP1-_gamma_f8:eta8/3^S_1 f8:eta8/3^S_1_order0             |  | -2.0088 +/- 0.30507   |  |      |      |      |       |       | 1.00  | 0.01  | 0.03  | 0.07  | 0.03  | 0.03  | 0.18  |
| JP1-_gamma_omega8:eta8/3^P_1 omega8:eta8/3^P_1_order0     |  | -3.6072 +/- 0.63139   |  |      |      |      |       |       |       | 1.00  | 0.05  | 0.08  | 0.05  | 0.12  | 0.12  |
| JP1-_gamma_omega8:omega1/1^P_1 omega8:omega1/1^P_1_order0 |  | 9.6856 +/- 2.3657     |  |      |      |      |       |       |       |       | 1.00  | 0.05  | 0.39  | 0.43  | -0.06 |
| JP1-_gamma_omega8:omega1/3^P_1 omega8:omega1/3^P_1_order0 |  | 11.745 +/- 4.9154     |  |      |      |      |       |       |       |       |       | 1.00  | 0.13  | 0.10  | 0.04  |
| JP1-_gamma_omega8:omega1/5^P_1 omega8:omega1/5^P_1_order0 |  | 19.282 +/- 3.735      |  |      |      |      |       |       |       |       |       |       | 1.00  | 0.46  | -0.10 |
| JP1-_gamma_omega8:omega8/3^P_1 omega8:omega8/3^P_1_order0 |  | 10.668 +/- 2.9013     |  |      |      |      |       |       |       |       |       |       |       | 1.00  | -0.10 |
| JP1-_m_pole0                                              |  | 0.46120 +/- 0.0011787 |  |      |      |      |       |       |       |       |       |       |       |       | 1.00  |
| =====                                                     |  |                       |  |      |      |      |       |       |       |       |       |       |       |       |       |

Phase space prescription ::

pole0\_sub

eta8:eta1[-] f8:eta8[+] h8:eta8[-] omega8:eta8[-] omega8:omega1[-] omega8:omega8[-] lower half-plane

sqrt(s)\_pole = (0.46115 +/- 0.0011504)  
+ (i/2)\*(-0.0035215 +/- 0.0015155) [-0.14]

s\_pole = (0.21265 +/- 0.0010607)  
+ i\*(-0.0016239 +/- 0.00069944) [-0.15]

| eta8:eta1                | f8:eta8                  | h8:eta8                  | omega8:eta8              | omega8:omega1            | omega8:omega8            |
|--------------------------|--------------------------|--------------------------|--------------------------|--------------------------|--------------------------|
| k_re= 0.1494 +/- 0.0009  | k_re= -0.0046 +/- 0.0020 | k_re= -0.0032 +/- 0.0014 | k_re= 0.1405 +/- 0.0009  | k_re= 0.0796 +/- 0.0017  | k_re= 0.0823 +/- 0.0016  |
| k_im= -0.0013 +/- 0.0006 | k_im= 0.0376 +/- 0.0029  | k_im= 0.0526 +/- 0.0021  | k_im= -0.0014 +/- 0.0006 | k_im= -0.0025 +/- 0.0011 | k_im= -0.0025 +/- 0.0011 |
| corr= [-0.14]            | corr= [ 0.24]            | corr= [ 0.20]            | corr= [-0.14]            | corr= [-0.12]            | corr= [-0.12]            |

  

| eta8:eta1/1^P_1              | f8:eta8/3^S_1                | h8:eta8/3^S_1(*)             | omega8:eta8/3^P_1             | omega8:omega1/1^P_1          | omega8:omega1/3^P_1          | omega8:omega1/5^P_1          | omega8:omega8/3^P_1          |
|------------------------------|------------------------------|------------------------------|-------------------------------|------------------------------|------------------------------|------------------------------|------------------------------|
| g = 0.0400 +/- 0.0119        | g = 0.0000 +/- 0.0000        | g = 0.3633 +/- 0.0446        | g = 0.0317 +/- 0.0102         | g = 0.0000 +/- 0.0000        | g = 0.0000 +/- 0.0000        | g = 0.0000 +/- 0.0000        | g = 0.0000 +/- 0.0000        |
| arg(g)/pi= 0.0169 +/- 0.0154 | arg(g)/pi= 0.4933 +/- 0.0045 | arg(g)/pi= 0.0067 +/- 0.0045 | arg(g)/pi= -0.0514 +/- 0.0098 | arg(g)/pi= 0.4933 +/- 0.0045 | arg(g)/pi= 0.4933 +/- 0.0045 | arg(g)/pi= 0.4933 +/- 0.0045 | arg(g)/pi= 0.4933 +/- 0.0045 |
| g_re= 0.0399 +/- 0.0119      | g_re= 0.0000 +/- 0.0000      | g_re= 0.3632 +/- 0.0445      | g_re= 0.0313 +/- 0.0100       | g_re= 0.0000 +/- 0.0000      | g_re= 0.0000 +/- 0.0000      | g_re= 0.0000 +/- 0.0000      | g_re= 0.0000 +/- 0.0000      |
| g_im= 0.0021 +/- 0.0019      | g_im= 0.0000 +/- 0.0000      | g_im= 0.0077 +/- 0.0059      | g_im= -0.0051 +/- 0.0023      | g_im= 0.0000 +/- 0.0000      | g_im= 0.0000 +/- 0.0000      | g_im= 0.0000 +/- 0.0000      | g_im= 0.0000 +/- 0.0000      |
| corr= [ 0.13]                | corr= [-0.60]                | corr= [ 0.78]                | corr= [-0.93]                 | corr= [-0.60]                | corr= [-0.60]                | corr= [-0.60]                | corr= [-0.60]                |

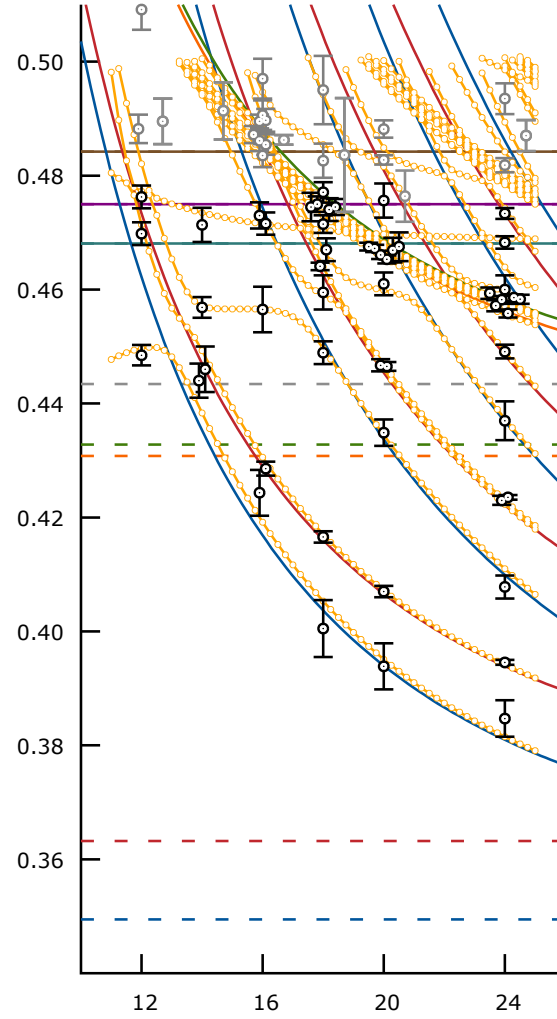

Figure 1.106: Similar to Figure 6 in the manuscript, the finite-volume spectrum, plotted as  $a_t E_{\text{cm}}$ , as a function of spatial extent  $L/a_s$ . Orange points/curves show the spectrum calculated from the amplitude given above (no uncertainties are shown). Black and grey points are the computed lattice energies on each volume, slightly displaced horizontally for clarity (black points correspond to energies used in the fit whereas grey points were not used). Two-meson non-interacting energies are shown as solid coloured curves/lines, two-meson thresholds are shown as dashed/solid horizontal lines, and the  $\eta^s \eta^s \eta^s$  threshold is shown as a dashed grey horizontal line.

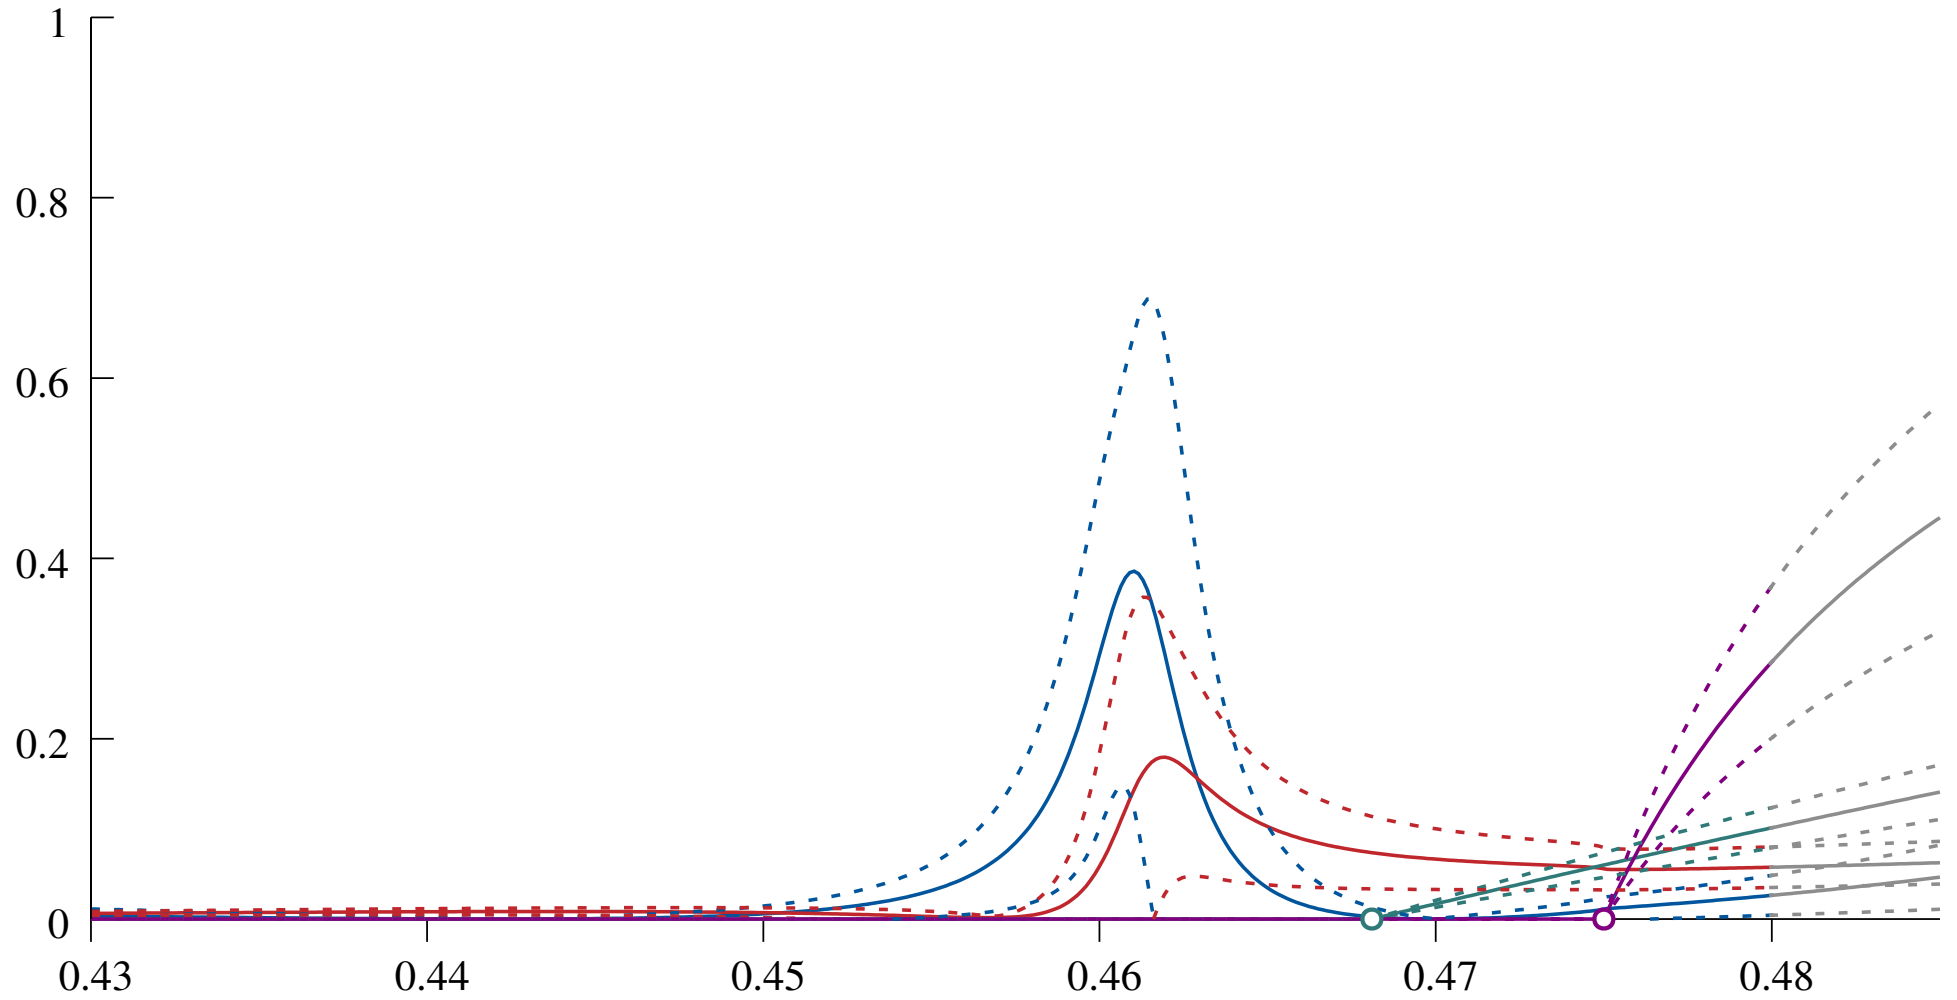

Figure 1.107: Similar to part (a) of Figure 7 in the manuscript,  $\rho_a \rho_b |t_{ab}|^2$  as a function of  $a_t E_{\text{cm}}$  for  $\eta^1 \eta^s \{^1P_1\} \rightarrow \eta^1 \eta^s \{^1P_1\}$  (blue),  $\omega^s \eta^s \{^3P_1\} \rightarrow \omega^s \eta^s \{^3P_1\}$  (red),  $f_1^s \eta^s \{^3S_1\} \rightarrow f_1^s \eta^s \{^3S_1\}$  (cyan), and  $h_1^s \eta^s \{^3S_1\} \rightarrow h_1^s \eta^s \{^3S_1\}$  (purple). Dashed lines indicate one standard deviation statistical uncertainties.

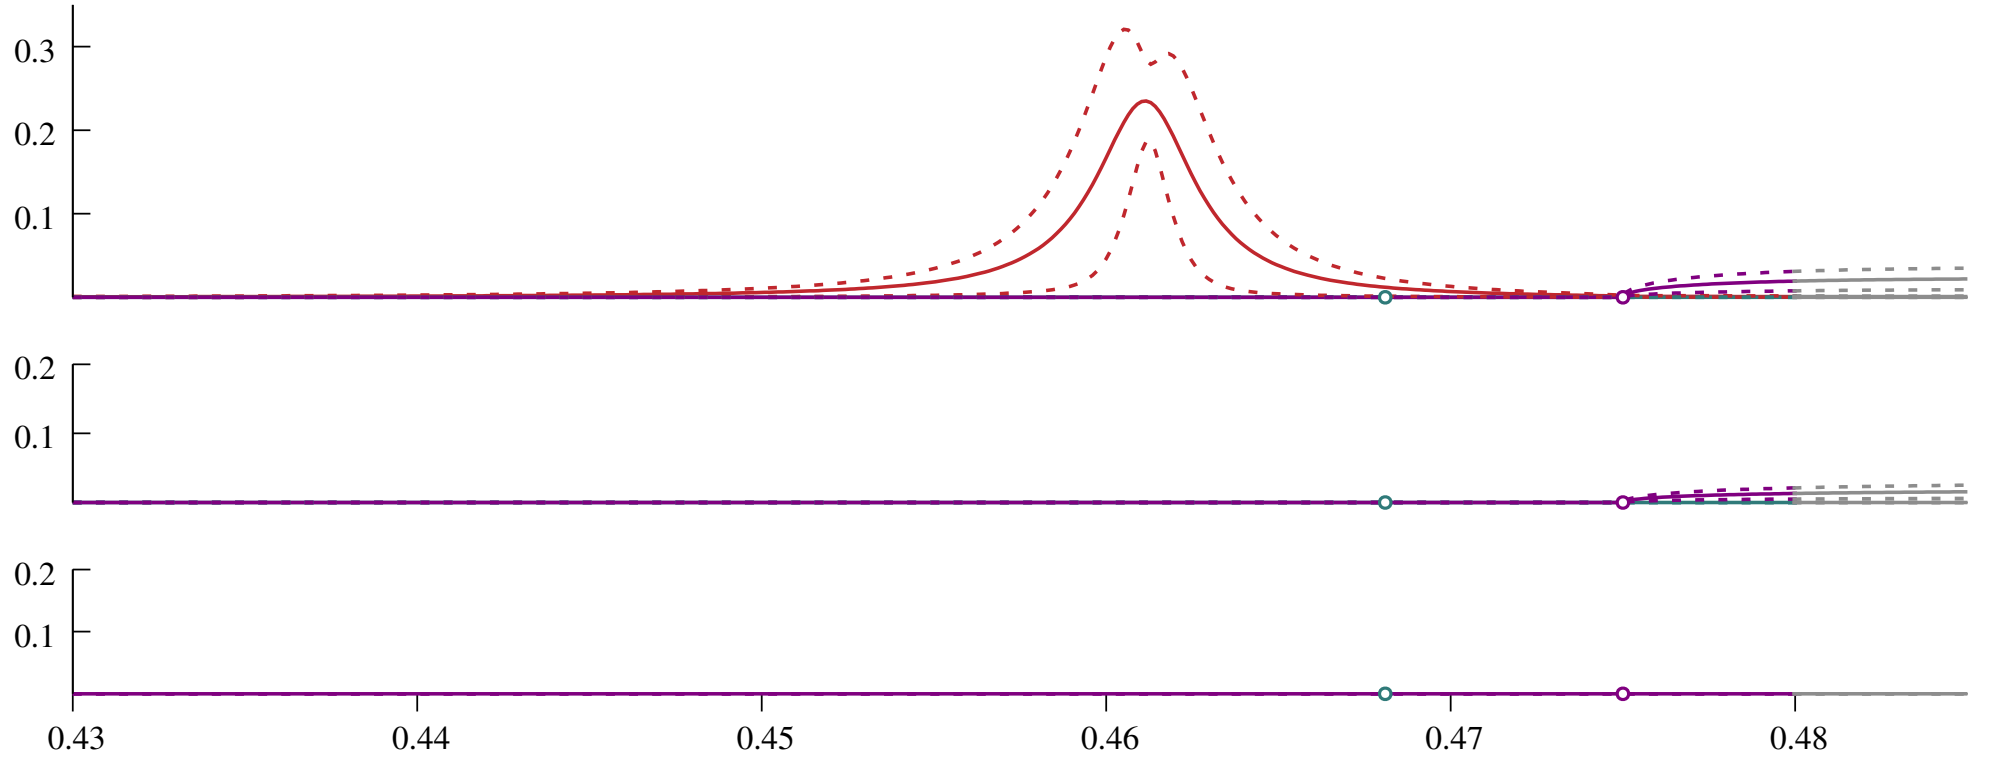

Figure 1.108: Similar to parts (b), (c) and (d) of Figure 7 in the manuscript,  $\rho_a \rho_b |t_{ab}|^2$  as a function of  $a_t E_{\text{cm}}$ . Top:  $\eta^1 \eta^s \{^1P_1\} \rightarrow \omega^s \eta^s \{^3P_1\}$  (red),  $\eta^1 \eta^s \{^1P_1\} \rightarrow f_1^s \eta^s \{^3S_1\}$  (cyan), and  $\eta^1 \eta^s \{^1P_1\} \rightarrow h_1^s \eta^s \{^3S_1\}$  (purple). Middle:  $\omega^s \eta^s \{^3P_1\} \rightarrow f_1^s \eta^s \{^3S_1\}$  (cyan), and  $\omega^s \eta^s \{^3P_1\} \rightarrow h_1^s \eta^s \{^3S_1\}$  (purple). Bottom:  $f_1^s \eta^s \{^3S_1\} \rightarrow h_1^s \eta^s \{^3S_1\}$  (purple). Dashed lines indicate one standard deviation statistical uncertainties.

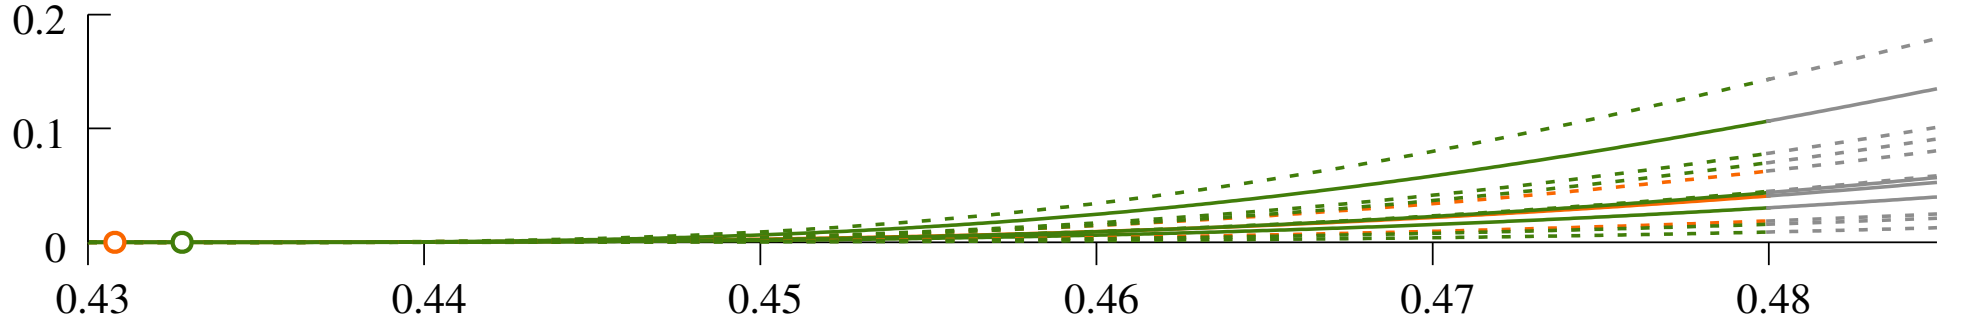

Figure 1.109: Similar to parts (e) and (f) of Figure 7 in the manuscript,  $\rho_a \rho_b |t_{ab}|^2$  as a function of  $a_t E_{\text{cm}}$  for  $\omega^s \omega^s \{^3P_1\} \rightarrow \omega^s \omega^s \{^3P_1\}$  (orange),  $\omega^1 \omega^s \{^1P_1, ^3P_1, ^5P_1\} \rightarrow \omega^s \omega^1 \{^1P_1, ^3P_1, ^5P_1\}$  (green). Dashed lines indicate one standard deviation statistical uncertainties.

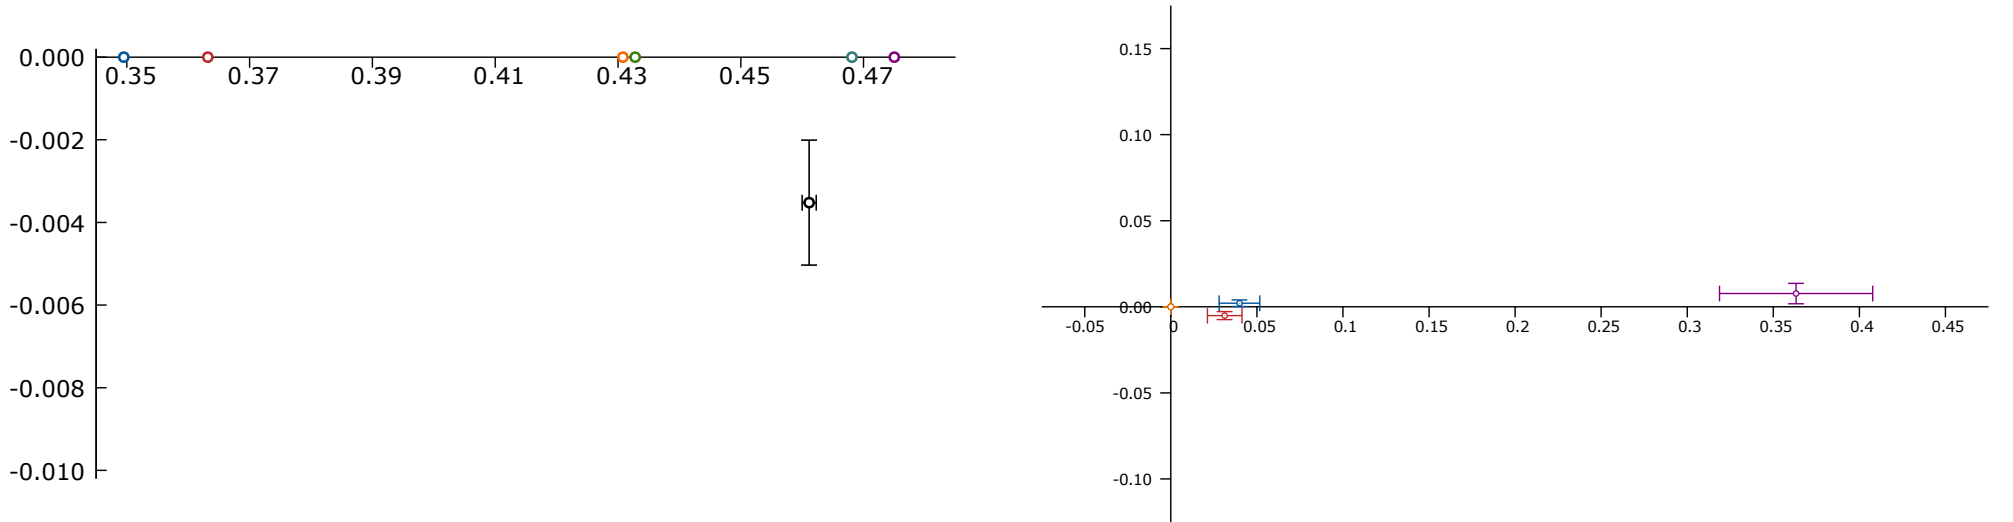

Figure 1.110: Left: Similar to Figure 13 in the manuscript, pole position on the proximal sheet (closest to physical scattering) with  $\text{Re}(a_t \sqrt{s})$  on the horizontal axis and  $2 \text{Im}(a_t \sqrt{s})$  on the vertical axis. Right: Similar to Figure 14 in the manuscript, the corresponding couplings with  $\text{Re}(a_t c)$  on the horizontal axis and  $\text{Im}(a_t c)$  on the vertical axis.

## 1.23 $\{m, g_{a,b,f}^{(0)}, \gamma_{(a,a),(b,b),(c,c),(d_1,d_1),(d_2,d_2),(d_3,d_3),(e,e)}, \gamma_{(a,b)}^{(1)}\}(\mathbf{CM}_m)$

minimised with chisq/nDoF = 41.67 / (53 - 12) = 1.02

|                                                           |  |                       |  |      |      |       |       |       |       |       |      |       |       |       |      |
|-----------------------------------------------------------|--|-----------------------|--|------|------|-------|-------|-------|-------|-------|------|-------|-------|-------|------|
| =====                                                     |  |                       |  |      |      |       |       |       |       |       |      |       |       |       |      |
| JP1-_g_eta8:eta1/1^P_1_pole0_order0                       |  | 0.87191 +/- 3.5524    |  | 1.00 | 1.00 | 0.99  | -0.19 | -0.36 | 0.43  | 0.08  | 0.01 | 0.05  | -0.01 | 0.00  | 0.59 |
| JP1-_g_h8:eta8/3^S_1_pole0_order0                         |  | 2.2882 +/- 9.4759     |  |      | 1.00 | 0.99  | -0.15 | -0.33 | 0.43  | 0.06  | 0.01 | 0.05  | -0.00 | 0.01  | 0.56 |
| JP1-_g_omega8:eta8/3^P_1_pole0_order0                     |  | 0.47481 +/- 1.9314    |  |      | 1.00 | -0.09 | -0.28 | 0.42  | -0.03 | 0.01  | 0.05 | 0.00  | 0.01  | 0.01  | 0.53 |
| JP1-_gamma_eta8:eta1/1^P_1 eta8:eta1/1^P_1_order0         |  | -1.4594 +/- 1.7685    |  |      |      | 1.00  | 0.81  | -0.03 | -0.41 | -0.04 | 0.04 | -0.01 | -0.06 | -0.31 |      |
| JP1-_gamma_eta8:eta1/1^P_1 omega8:eta8/3^P_1_order1       |  | -19.833 +/- 6.1098    |  |      |      |       | 1.00  | -0.33 | -0.32 | -0.05 | 0.01 | -0.02 | -0.06 | -0.29 |      |
| JP1-_gamma_f8:eta8/3^S_1 f8:eta8/3^S_1_order0             |  | -1.9583 +/- 0.29871   |  |      |      |       |       | 1.00  | 0.15  | 0.05  | 0.07 | 0.04  | 0.05  | 0.19  |      |
| JP1-_gamma_omega8:eta8/3^P_1 omega8:eta8/3^P_1_order0     |  | -3.0444 +/- 0.66563   |  |      |      |       |       |       | 1.00  | 0.08  | 0.06 | 0.06  | 0.15  | 0.18  |      |
| JP1-_gamma_omega8:omega1/1^P_1 omega8:omega1/1^P_1_order0 |  | 9.7823 +/- 2.3676     |  |      |      |       |       |       |       | 1.00  | 0.05 | 0.39  | 0.43  | -0.04 |      |
| JP1-_gamma_omega8:omega1/3^P_1 omega8:omega1/3^P_1_order0 |  | 11.828 +/- 4.9172     |  |      |      |       |       |       |       |       | 1.00 | 0.13  | 0.10  | 0.03  |      |
| JP1-_gamma_omega8:omega1/5^P_1 omega8:omega1/5^P_1_order0 |  | 19.309 +/- 3.7271     |  |      |      |       |       |       |       |       |      | 1.00  | 0.46  | -0.08 |      |
| JP1-_gamma_omega8:omega8/3^P_1 omega8:omega8/3^P_1_order0 |  | 10.913 +/- 2.9116     |  |      |      |       |       |       |       |       |      |       | 1.00  | -0.07 |      |
| JP1-_m_pole0                                              |  | 0.46174 +/- 0.0011548 |  |      |      |       |       |       |       |       |      |       |       | 1.00  |      |
| =====                                                     |  |                       |  |      |      |       |       |       |       |       |      |       |       |       |      |

Phase space prescription ::

pole0\_sub

eta8:eta1[-] f8:eta8[+] h8:eta8[+] omega8:eta8[-] omega8:omega1[-] omega8:omega8[-] lower half-plane

sqrt(s)\_pole = (0.46136 +/- 0.0010291)  
+ (i/2)\*(-0.002977 +/- 0.0013691) [-0.15]

s\_pole = (0.21285 +/- 0.00094928)  
+ i\*(-0.0013735 +/- 0.00063211) [-0.16]

| eta8:eta1                | f8:eta8                  | h8:eta8                  | omega8:eta8              | omega8:omega1            | omega8:omega8            |
|--------------------------|--------------------------|--------------------------|--------------------------|--------------------------|--------------------------|
| k_re= 0.1496 +/- 0.0008  | k_re= -0.0040 +/- 0.0019 | k_re= -0.0028 +/- 0.0013 | k_re= 0.1407 +/- 0.0008  | k_re= 0.0799 +/- 0.0015  | k_re= 0.0826 +/- 0.0014  |
| k_im= -0.0011 +/- 0.0005 | k_im= 0.0369 +/- 0.0027  | k_im= 0.0521 +/- 0.0019  | k_im= -0.0012 +/- 0.0006 | k_im= -0.0021 +/- 0.0010 | k_im= -0.0021 +/- 0.0010 |
| corr= [-0.15]            | corr= [ 0.24]            | corr= [ 0.20]            | corr= [-0.15]            | corr= [-0.13]            | corr= [-0.13]            |

  

| eta8:eta1/1^P_1               | f8:eta8/3^S_1                | h8:eta8/3^S_1(*)             | omega8:eta8/3^P_1             | omega8:omega1/1^P_1          | omega8:omega1/3^P_1          | omega8:omega1/5^P_1          | omega8:omega8/3^P_1          |
|-------------------------------|------------------------------|------------------------------|-------------------------------|------------------------------|------------------------------|------------------------------|------------------------------|
| g = 0.0406 +/- 0.0110         | g = 0.0000 +/- 0.0000        | g = 0.3795 +/- 0.0529        | g = 0.0219 +/- 0.0111         | g = 0.0000 +/- 0.0000        | g = 0.0000 +/- 0.0000        | g = 0.0000 +/- 0.0000        | g = 0.0000 +/- 0.0000        |
| arg(g)/pi= -0.0530 +/- 0.0333 | arg(g)/pi= 0.4928 +/- 0.0053 | arg(g)/pi= 0.0072 +/- 0.0053 | arg(g)/pi= -0.1779 +/- 0.1077 | arg(g)/pi= 0.4928 +/- 0.0053 | arg(g)/pi= 0.4928 +/- 0.0053 | arg(g)/pi= 0.4928 +/- 0.0053 | arg(g)/pi= 0.4928 +/- 0.0053 |
| g_re= 0.0400 +/- 0.0108       | g_re= 0.0000 +/- 0.0000      | g_re= 0.3794 +/- 0.0528      | g_re= 0.0186 +/- 0.0128       | g_re= 0.0000 +/- 0.0000      | g_re= 0.0000 +/- 0.0000      | g_re= 0.0000 +/- 0.0000      | g_re= 0.0000 +/- 0.0000      |
| g_im= -0.0067 +/- 0.0048      | g_im= 0.0000 +/- 0.0000      | g_im= 0.0086 +/- 0.0072      | g_im= -0.0116 +/- 0.0038      | g_im= 0.0000 +/- 0.0000      | g_im= 0.0000 +/- 0.0000      | g_im= 0.0000 +/- 0.0000      | g_im= 0.0000 +/- 0.0000      |
| corr= [-0.44]                 | corr= [-0.64]                | corr= [ 0.81]                | corr= [-0.04]                 | corr= [-0.64]                | corr= [-0.64]                | corr= [-0.64]                | corr= [-0.64]                |

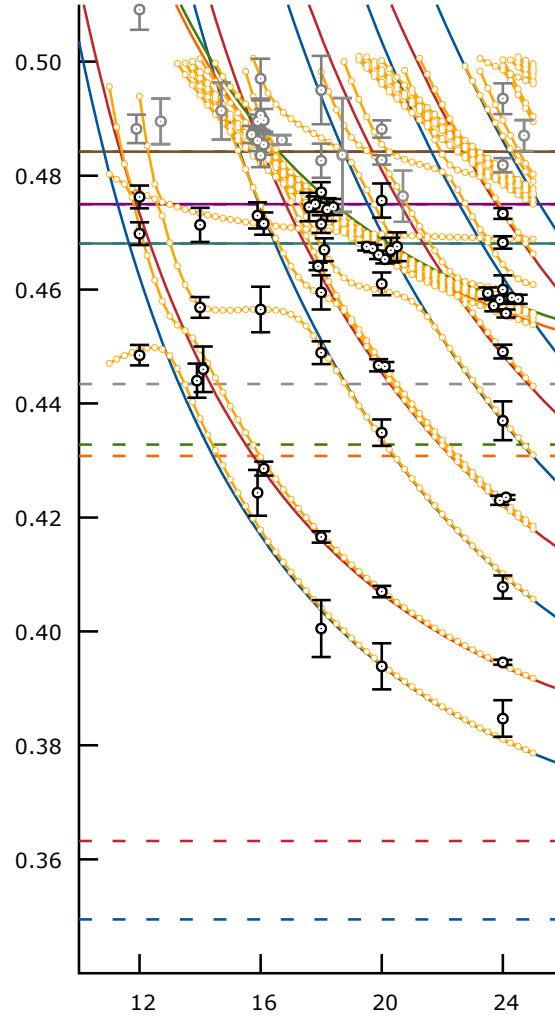

Figure 1.111: Similar to Figure 6 in the manuscript, the finite-volume spectrum, plotted as  $a_t E_{\text{cm}}$ , as a function of spatial extent  $L/a_s$ . Orange points/curves show the spectrum calculated from the amplitude given above (no uncertainties are shown). Black and grey points are the computed lattice energies on each volume, slightly displaced horizontally for clarity (black points correspond to energies used in the fit whereas grey points were not used). Two-meson non-interacting energies are shown as solid coloured curves/lines, two-meson thresholds are shown as dashed/solid horizontal lines, and the  $\eta^s \eta^s \eta^s$  threshold is shown as a dashed grey horizontal line.

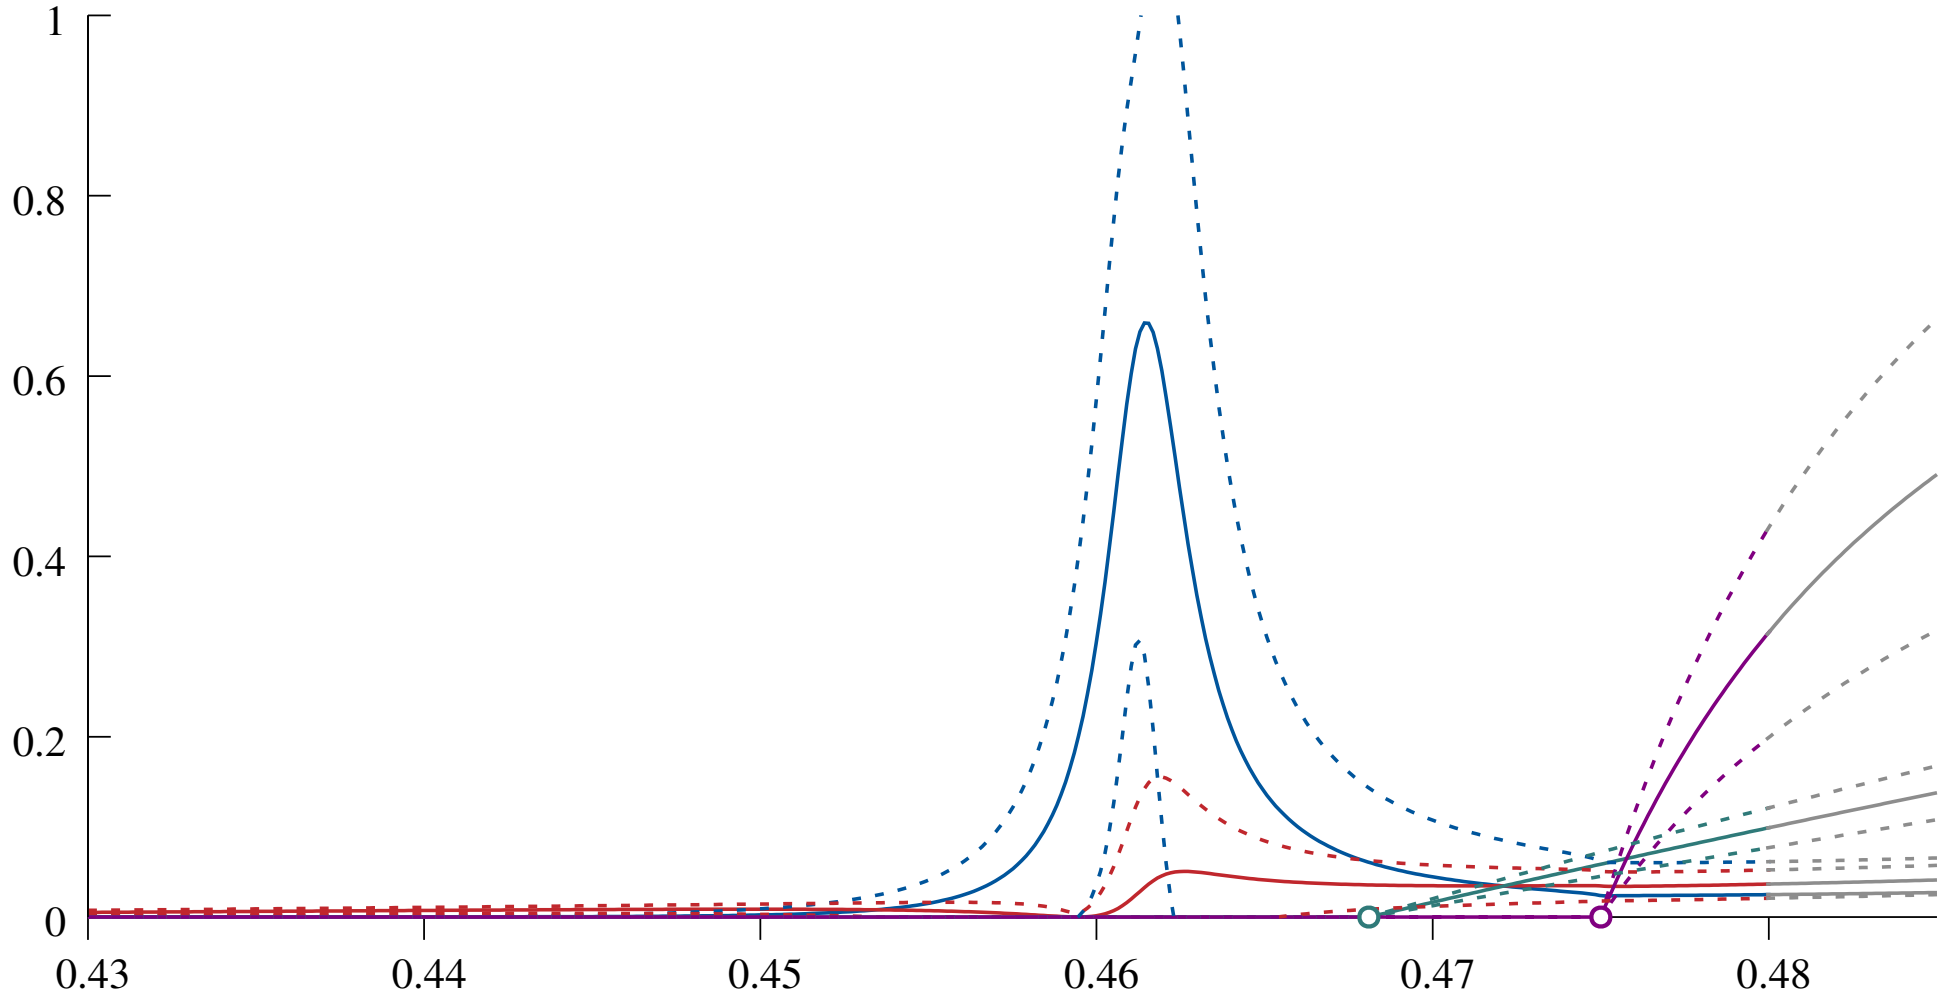

Figure 1.112: Similar to part (a) of Figure 7 in the manuscript,  $\rho_a \rho_b |t_{ab}|^2$  as a function of  $a_t E_{\text{cm}}$  for  $\eta^1 \eta^{\text{s}} \{^1P_1\} \rightarrow \eta^1 \eta^{\text{s}} \{^1P_1\}$  (blue),  $\omega^{\text{s}} \eta^{\text{s}} \{^3P_1\} \rightarrow \omega^{\text{s}} \eta^{\text{s}} \{^3P_1\}$  (red),  $f_1^{\text{s}} \eta^{\text{s}} \{^3S_1\} \rightarrow f_1^{\text{s}} \eta^{\text{s}} \{^3S_1\}$  (cyan), and  $h_1^{\text{s}} \eta^{\text{s}} \{^3S_1\} \rightarrow h_1^{\text{s}} \eta^{\text{s}} \{^3S_1\}$  (purple). Dashed lines indicate one standard deviation statistical uncertainties.

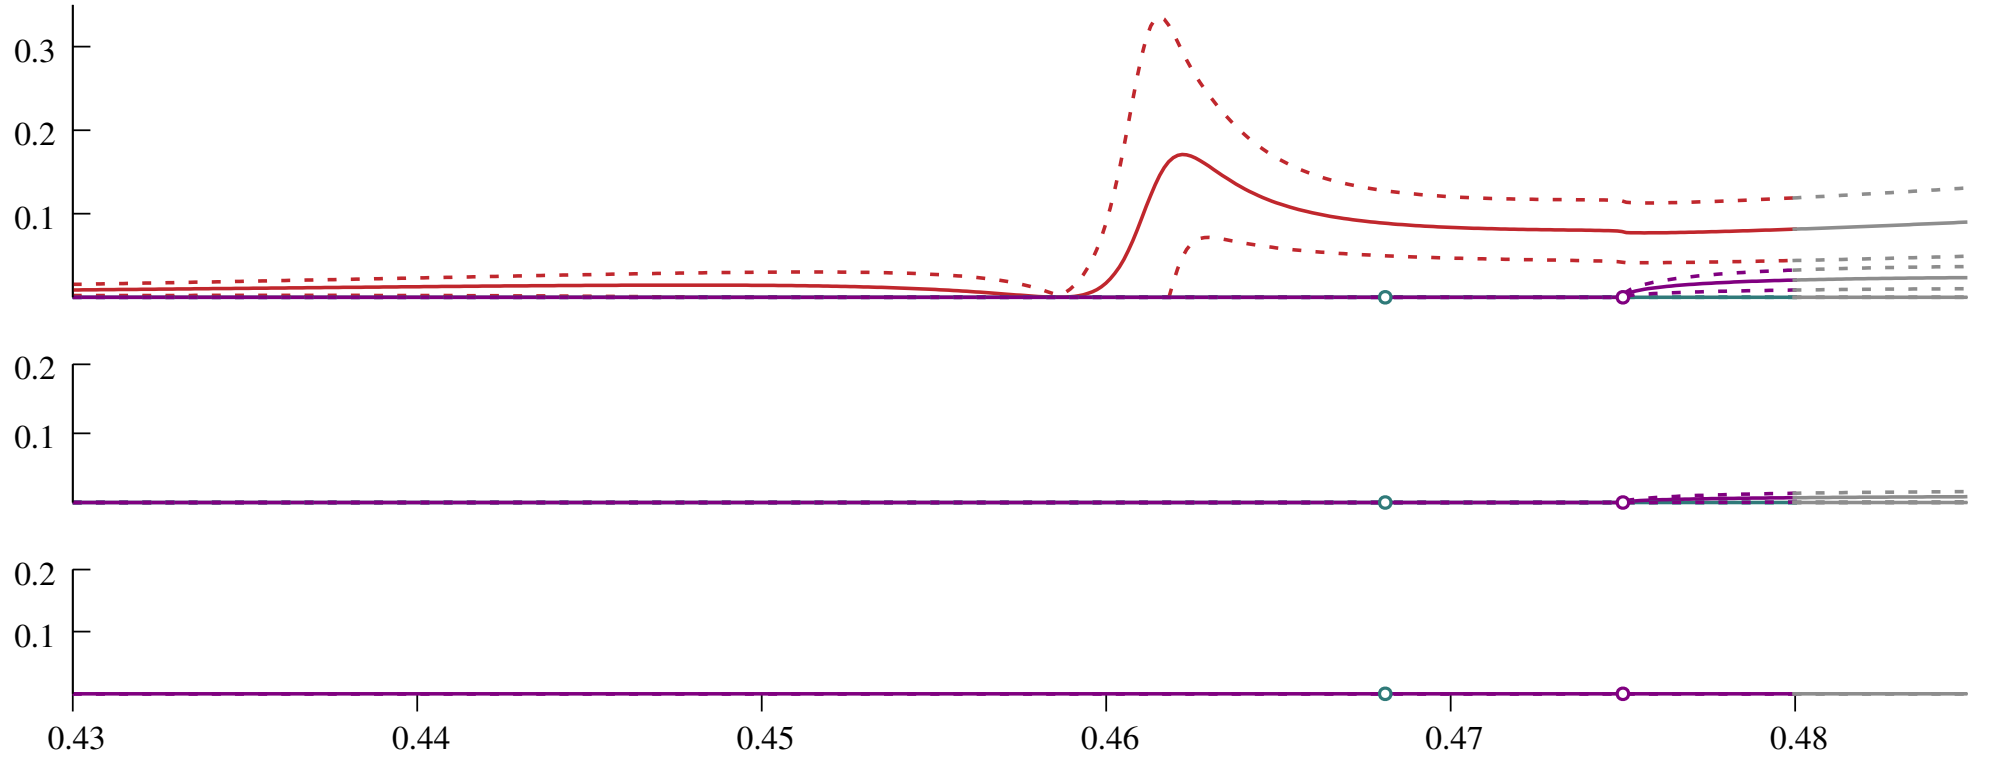

Figure 1.113: Similar to parts (b), (c) and (d) of Figure 7 in the manuscript,  $\rho_a \rho_b |t_{ab}|^2$  as a function of  $a_t E_{\text{cm}}$ . Top:  $\eta^1 \eta^s \{^1P_1\} \rightarrow \omega^s \eta^s \{^3P_1\}$  (red),  $\eta^1 \eta^s \{^1P_1\} \rightarrow f_1^s \eta^s \{^3S_1\}$  (cyan), and  $\eta^1 \eta^s \{^1P_1\} \rightarrow h_1^s \eta^s \{^3S_1\}$  (purple). Middle:  $\omega^s \eta^s \{^3P_1\} \rightarrow f_1^s \eta^s \{^3S_1\}$  (cyan), and  $\omega^s \eta^s \{^3P_1\} \rightarrow h_1^s \eta^s \{^3S_1\}$  (purple). Bottom:  $f_1^s \eta^s \{^3S_1\} \rightarrow h_1^s \eta^s \{^3S_1\}$  (purple). Dashed lines indicate one standard deviation statistical uncertainties.

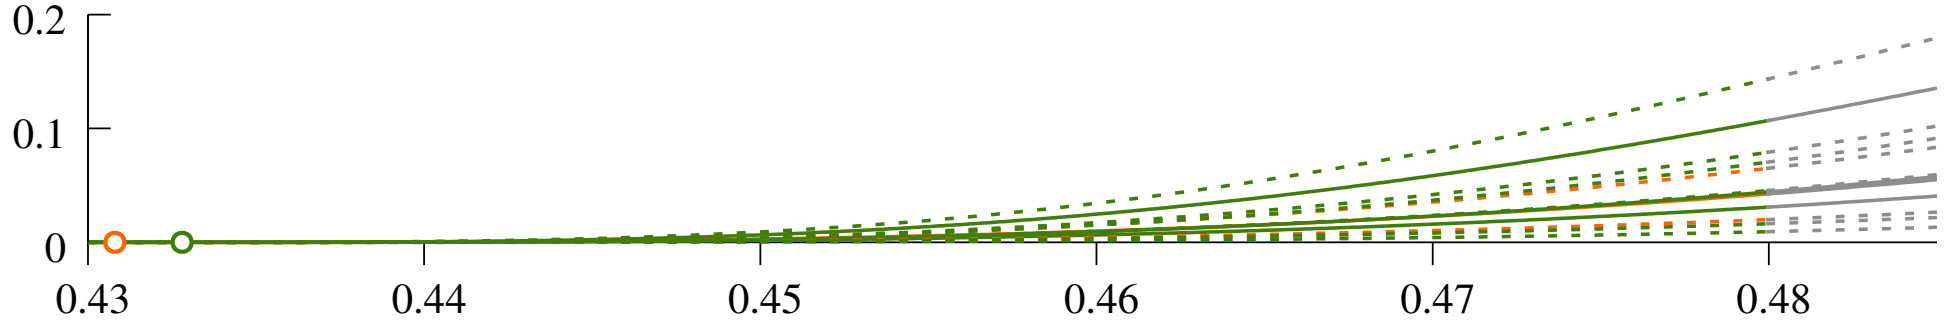

Figure 1.114: Similar to parts (e) and (f) of Figure 7 in the manuscript,  $\rho_a \rho_b |t_{ab}|^2$  as a function of  $a_t E_{\text{cm}}$  for  $\omega^s \omega^s \{^3P_1\} \rightarrow \omega^s \omega^s \{^3P_1\}$  (orange),  $\omega^1 \omega^s \{^1P_1, ^3P_1, ^5P_1\} \rightarrow \omega^s \omega^1 \{^1P_1, ^3P_1, ^5P_1\}$  (green). Dashed lines indicate one standard deviation statistical uncertainties.

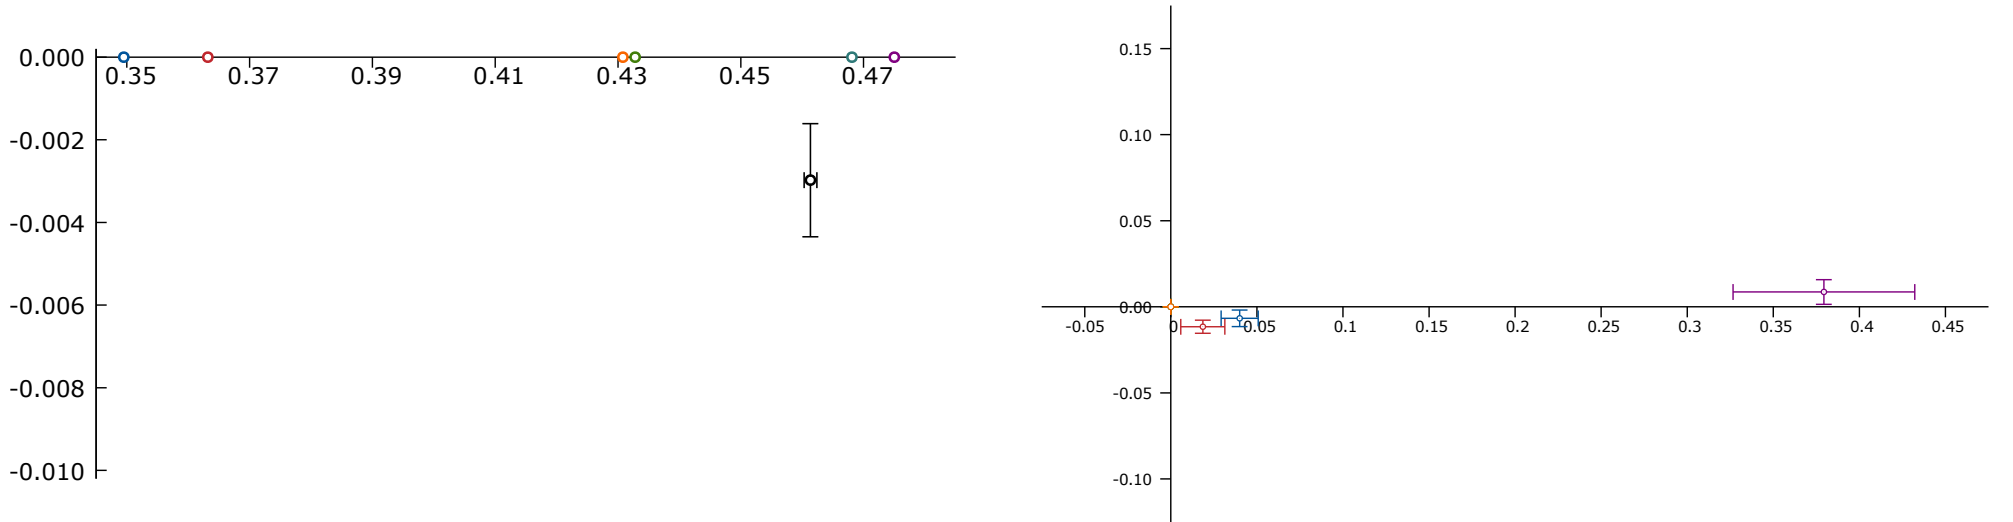

Figure 1.115: Left: Similar to Figure 13 in the manuscript, pole position on the proximal sheet (closest to physical scattering) with  $\text{Re}(a_t \sqrt{s})$  on the horizontal axis and  $2 \text{Im}(a_t \sqrt{s})$  on the vertical axis. Right: Similar to Figure 14 in the manuscript, the corresponding couplings with  $\text{Re}(a_t c)$  on the horizontal axis and  $\text{Im}(a_t c)$  on the vertical axis.

# 1.24 $\{m, g_{a,b,f}^{(0)}, g_f^{(1)}, \gamma_{(a,a),(b,b),(c,c),(\mathfrak{d}_1,\mathfrak{d}_1),(\mathfrak{d}_2,\mathfrak{d}_2),(\mathfrak{d}_3,\mathfrak{d}_3),(\mathfrak{e},\mathfrak{e})}^{(0)}\}(\mathbf{CM}_m)$

minimised with chisq/nDoF = 44.99 / (53 - 12) = 1.10

|                                                           |  |                      |  |      |      |       |      |       |       |       |       |      |       |       |       |
|-----------------------------------------------------------|--|----------------------|--|------|------|-------|------|-------|-------|-------|-------|------|-------|-------|-------|
| =====                                                     |  |                      |  |      |      |       |      |       |       |       |       |      |       |       |       |
| JP1-_g_eta8:eta1/1^P_1_pole0_order0                       |  | 0.22580 +/- 0.18184  |  | 1.00 | 0.30 | -0.01 | 0.78 | 0.06  | 0.30  | -0.21 | -0.03 | 0.02 | -0.06 | -0.05 | 0.65  |
| JP1-_g_h8:eta8/3^S_1_pole0_order0                         |  | 4.4315 +/- 1.9268    |  |      | 1.00 | -0.94 | 0.24 | 0.12  | 0.13  | 0.11  | -0.00 | 0.01 | -0.01 | -0.01 | 0.23  |
| JP1-_g_h8:eta8/3^S_1_pole0_order1                         |  | -17.291 +/- 8.7533   |  |      |      | 1.00  | 0.08 | -0.07 | 0.01  | -0.23 | -0.00 | 0.01 | 0.01  | 0.00  | -0.06 |
| JP1-_g_omega8:eta8/3^P_1_pole0_order0                     |  | 0.25812 +/- 0.21774  |  |      |      |       | 1.00 | 0.15  | 0.38  | -0.37 | 0.01  | 0.05 | 0.01  | -0.00 | 0.39  |
| JP1-_gamma_eta8:eta1/1^P_1 eta8:eta1/1^P_1_order0         |  | 1.4898 +/- 0.57262   |  |      |      |       | 1.00 | 0.50  | 0.01  | 0.01  | 0.01  | 0.05 | 0.02  | 0.01  | -0.08 |
| JP1-_gamma_f8:eta8/3^S_1 f8:eta8/3^S_1_order0             |  | -2.1049 +/- 0.30351  |  |      |      |       |      | 1.00  | -0.08 | 0.03  | 0.08  | 0.03 | 0.03  | 0.03  | 0.11  |
| JP1-_gamma_omega8:eta8/3^P_1 omega8:eta8/3^P_1_order0     |  | -3.2372 +/- 0.58088  |  |      |      |       |      |       | 1.00  | 0.08  | 0.07  | 0.07 | 0.16  | -0.05 |       |
| JP1-_gamma_omega8:omega1/1^P_1 omega8:omega1/1^P_1_order0 |  | 9.5721 +/- 2.3631    |  |      |      |       |      |       |       | 1.00  | 0.06  | 0.39 | 0.43  | -0.07 |       |
| JP1-_gamma_omega8:omega1/3^P_1 omega8:omega1/3^P_1_order0 |  | 11.975 +/- 4.929     |  |      |      |       |      |       |       |       | 1.00  | 0.14 | 0.10  | 0.03  |       |
| JP1-_gamma_omega8:omega1/5^P_1 omega8:omega1/5^P_1_order0 |  | 19.181 +/- 3.7352    |  |      |      |       |      |       |       |       |       | 1.00 | 0.46  | -0.10 |       |
| JP1-_gamma_omega8:omega8/3^P_1 omega8:omega8/3^P_1_order0 |  | 10.537 +/- 2.8984    |  |      |      |       |      |       |       |       |       |      | 1.00  | -0.11 |       |
| JP1-_m_pole0                                              |  | 0.46089 +/- 0.001076 |  |      |      |       |      |       |       |       |       |      |       | 1.00  |       |
| =====                                                     |  |                      |  |      |      |       |      |       |       |       |       |      |       |       |       |

Phase space prescription ::

pole0\_sub

eta8:eta1[-] f8:eta8[+] h8:eta8[+] omega8:eta8[-] omega8:omega1[-] omega8:omega8[-] lower half-plane

sqrt(s)\_pole = (0.46079 +/- 0.0010696)  
+ (i/2)\*(-0.002734 +/- 0.0014956) [-0.16]

s\_pole = (0.21232 +/- 0.00098533)  
+ i\*(-0.0012598 +/- 0.00068966) [-0.17]

| eta8:eta1                | f8:eta8                  | h8:eta8                  | omega8:eta8              | omega8:omega1            | omega8:omega8            |
|--------------------------|--------------------------|--------------------------|--------------------------|--------------------------|--------------------------|
| k_re= 0.1491 +/- 0.0008  | k_re= -0.0035 +/- 0.0020 | k_re= -0.0025 +/- 0.0014 | k_re= 0.1403 +/- 0.0009  | k_re= 0.0791 +/- 0.0016  | k_re= 0.0818 +/- 0.0015  |
| k_im= -0.0010 +/- 0.0006 | k_im= 0.0384 +/- 0.0027  | k_im= 0.0532 +/- 0.0019  | k_im= -0.0011 +/- 0.0006 | k_im= -0.0020 +/- 0.0011 | k_im= -0.0019 +/- 0.0010 |
| corr= [-0.16]            | corr= [ 0.23]            | corr= [ 0.20]            | corr= [-0.16]            | corr= [-0.15]            | corr= [-0.15]            |

  

| eta8:eta1/1^P_1              | f8:eta8/3^S_1                | h8:eta8/3^S_1(*)              | omega8:eta8/3^P_1             | omega8:omega1/1^P_1          | omega8:omega1/3^P_1          | omega8:omega1/5^P_1          | omega8:omega8/3^P_1          |
|------------------------------|------------------------------|-------------------------------|-------------------------------|------------------------------|------------------------------|------------------------------|------------------------------|
| lg = 0.0307 +/- 0.0131       | lg = 0.0000 +/- 0.0000       | lg = 0.3473 +/- 0.0598        | lg = 0.0326 +/- 0.0114        | lg = 0.0000 +/- 0.0000       | lg = 0.0000 +/- 0.0000       | lg = 0.0000 +/- 0.0000       | lg = 0.0000 +/- 0.0000       |
| arg(g)/pi= 0.0150 +/- 0.0175 | arg(g)/pi= 0.5011 +/- 0.0035 | arg(g)/pi= -0.0011 +/- 0.0035 | arg(g)/pi= -0.0618 +/- 0.0140 | arg(g)/pi= 0.5011 +/- 0.0035 | arg(g)/pi= 0.5011 +/- 0.0035 | arg(g)/pi= 0.5011 +/- 0.0035 | arg(g)/pi= 0.5011 +/- 0.0035 |
| g_re= 0.0307 +/- 0.0132      | g_re= -0.0000 +/- 0.0000     | g_re= 0.3473 +/- 0.0598       | g_re= 0.0320 +/- 0.0111       | g_re= -0.0000 +/- 0.0000     | g_re= -0.0000 +/- 0.0000     | g_re= -0.0000 +/- 0.0000     | g_re= -0.0000 +/- 0.0000     |
| g_im= 0.0014 +/- 0.0016      | g_im= 0.0000 +/- 0.0000      | g_im= -0.0012 +/- 0.0037      | g_im= -0.0063 +/- 0.0030      | g_im= 0.0000 +/- 0.0000      | g_im= 0.0000 +/- 0.0000      | g_im= 0.0000 +/- 0.0000      | g_im= 0.0000 +/- 0.0000      |
| corr= [-0.04]                | corr= [-0.64]                | corr= [ 0.58]                 | corr= [-0.89]                 | corr= [-0.64]                | corr= [-0.64]                | corr= [-0.64]                | corr= [-0.64]                |

eta8:eta1[-] f8:eta8[+] h8:eta8[+] omega8:eta8[-] omega8:omega1[-] omega8:omega8[-] lower half-plane

sqrt(s)\_pole = (0.52119 +/- 0.055212)  
+ (i/2)\*(-0.035075 +/- 0.019284) [-0.31]

s\_pole = (0.27133 +/- 0.057431)  
+ i\*(-0.018281 +/- 0.010811) [-0.46]

| eta8:eta1                | f8:eta8                  | h8:eta8                  | omega8:eta8              | omega8:omega1            | omega8:omega8            |
|--------------------------|--------------------------|--------------------------|--------------------------|--------------------------|--------------------------|
| k_re= 0.1925 +/- 0.0372  | k_re= -0.1093 +/- 0.0592 | k_re= -0.1022 +/- 0.0623 | k_re= 0.1855 +/- 0.0385  | k_re= 0.1458 +/- 0.0492  | k_re= 0.1472 +/- 0.0487  |
| k_im= -0.0118 +/- 0.0062 | k_im= 0.0191 +/- 0.0107  | k_im= 0.0202 +/- 0.0118  | k_im= -0.0122 +/- 0.0064 | k_im= -0.0157 +/- 0.0082 | k_im= -0.0155 +/- 0.0081 |
| corr= [-0.16]            | corr= [ 0.39]            | corr= [ 0.47]            | corr= [-0.14]            | corr= [ 0.11]            | corr= [ 0.09]            |

  

| eta8:eta1/1^P_1               | f8:eta8/3^S_1                | h8:eta8/3^S_1(*)             | omega8:eta8/3^P_1             | omega8:omega1/1^P_1          | omega8:omega1/3^P_1          | omega8:omega1/5^P_1          | omega8:omega8/3^P_1          |
|-------------------------------|------------------------------|------------------------------|-------------------------------|------------------------------|------------------------------|------------------------------|------------------------------|
| lg = 0.0403 +/- 0.0257        | lg = 0.0000 +/- 0.0000       | lg = 0.1925 +/- 0.0500       | lg = 0.0429 +/- 0.0299        | lg = 0.0000 +/- 0.0000       | lg = 0.0000 +/- 0.0000       | lg = 0.0000 +/- 0.0000       | lg = 0.0000 +/- 0.0000       |
| arg(g)/pi= -0.5907 +/- 0.0381 | arg(g)/pi= 0.4067 +/- 0.0866 | arg(g)/pi= 0.0933 +/- 0.0866 | arg(g)/pi= -0.7505 +/- 0.0765 | arg(g)/pi= 0.4067 +/- 0.0866 | arg(g)/pi= 0.4067 +/- 0.0866 | arg(g)/pi= 0.4067 +/- 0.0866 | arg(g)/pi= 0.4067 +/- 0.0866 |
| g_re= -0.0113 +/- 0.0087      | g_re= 0.0000 +/- 0.0000      | g_re= 0.1843 +/- 0.0524      | g_re= -0.0304 +/- 0.0280      | g_re= 0.0000 +/- 0.0000      | g_re= 0.0000 +/- 0.0000      | g_re= 0.0000 +/- 0.0000      | g_re= 0.0000 +/- 0.0000      |
| g_im= -0.0387 +/- 0.0247      | g_im= 0.0000 +/- 0.0000      | g_im= 0.0556 +/- 0.0500      | g_im= -0.0303 +/- 0.0148      | g_im= 0.0000 +/- 0.0000      | g_im= 0.0000 +/- 0.0000      | g_im= 0.0000 +/- 0.0000      | g_im= 0.0000 +/- 0.0000      |
| corr= [ 0.82]                 | corr= [ 0.11]                | corr= [-0.16]                | corr= [ 0.95]                 | corr= [ 0.11]                | corr= [ 0.11]                | corr= [ 0.11]                | corr= [ 0.11]                |

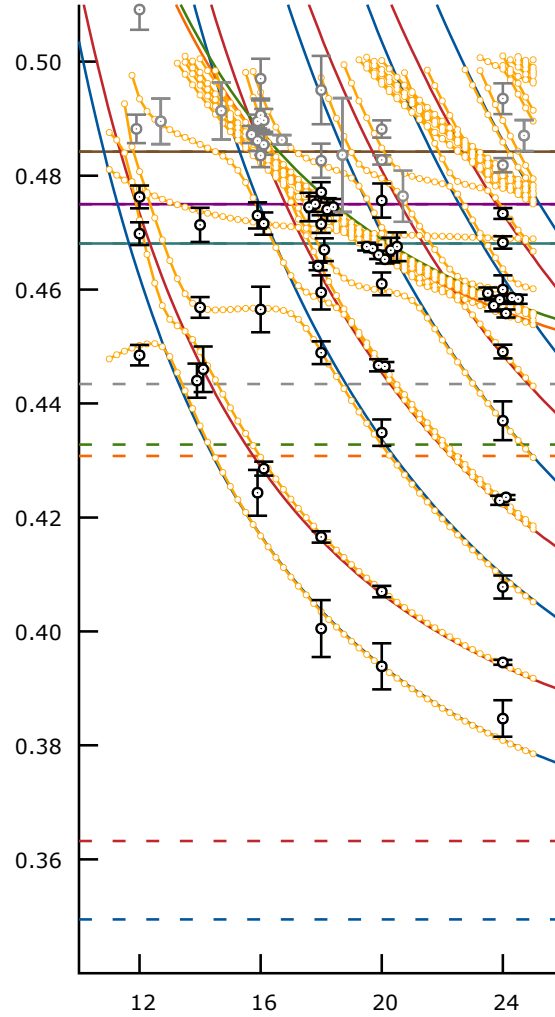

Figure 1.116: Similar to Figure 6 in the manuscript, the finite-volume spectrum, plotted as  $a_t E_{\text{cm}}$ , as a function of spatial extent  $L/a_s$ . Orange points/curves show the spectrum calculated from the amplitude given above (no uncertainties are shown). Black and grey points are the computed lattice energies on each volume, slightly displaced horizontally for clarity (black points correspond to energies used in the fit whereas grey points were not used). Two-meson non-interacting energies are shown as solid coloured curves/lines, two-meson thresholds are shown as dashed/solid horizontal lines, and the  $\eta^s \eta^s \eta^s$  threshold is shown as a dashed grey horizontal line.

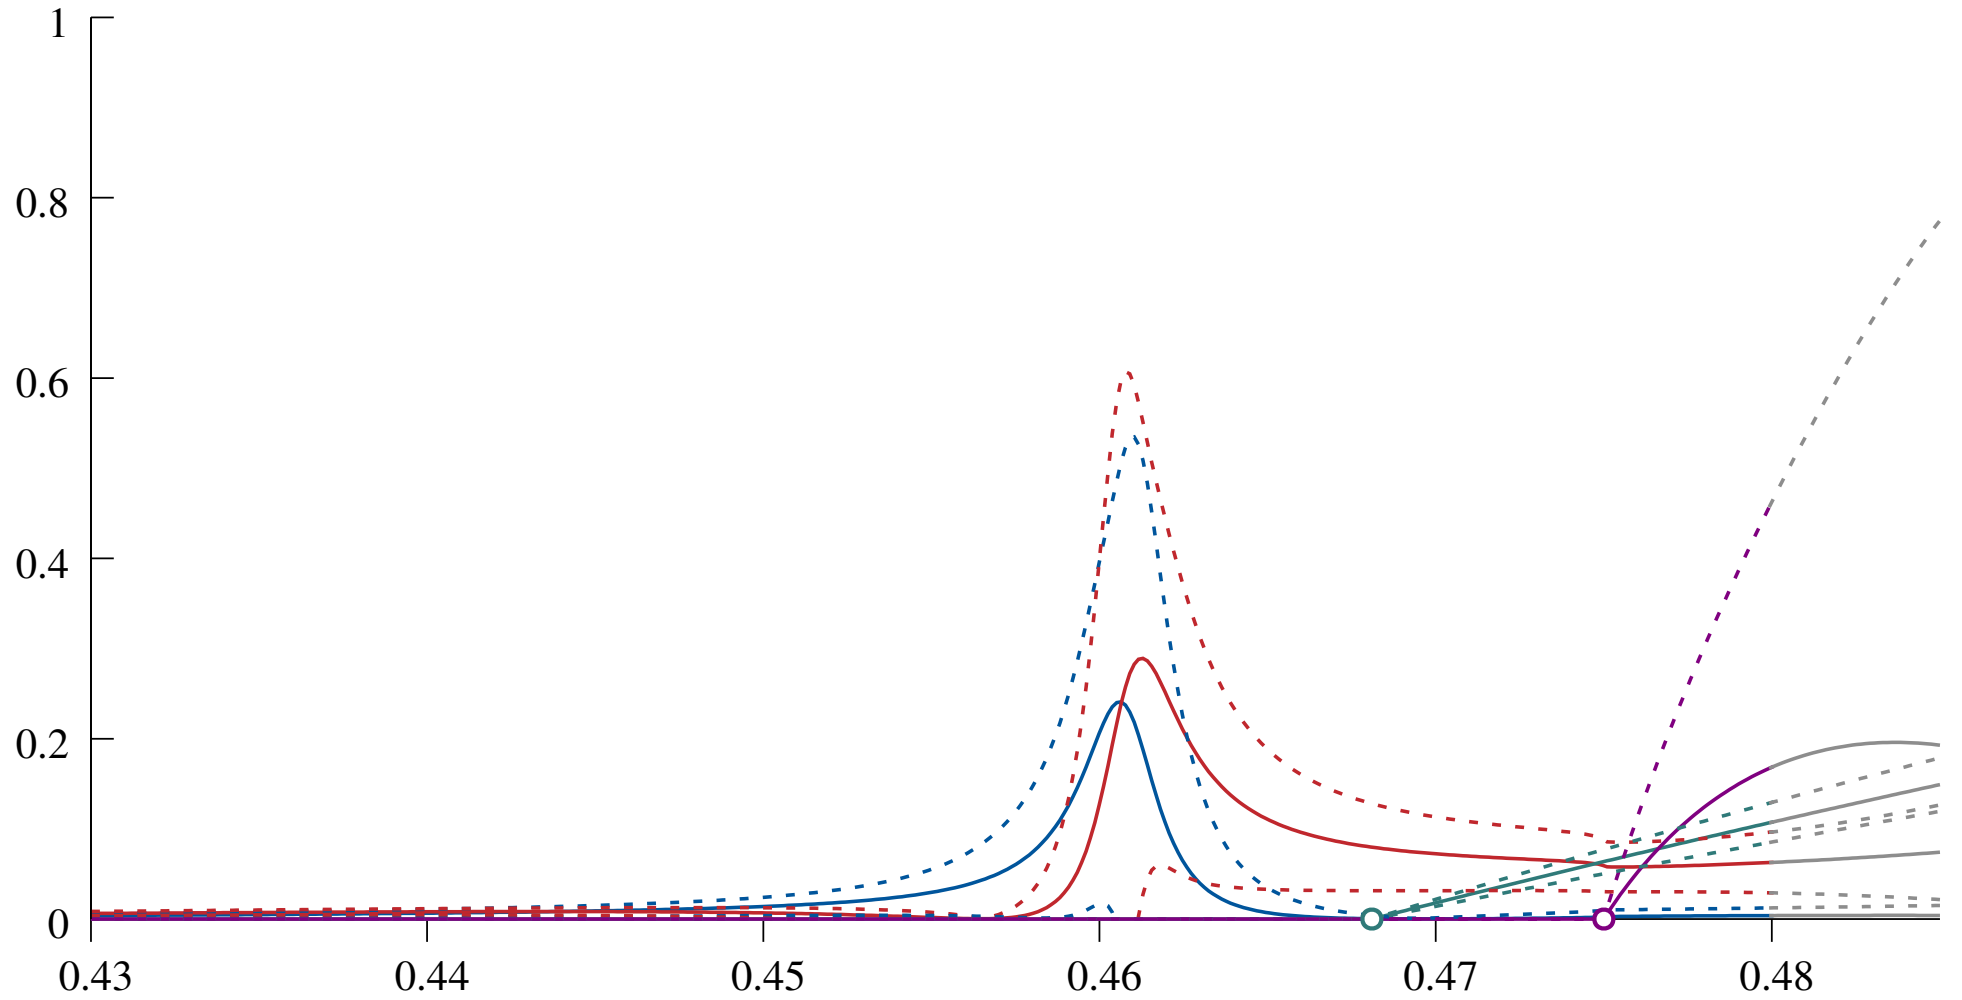

Figure 1.117: Similar to part (a) of Figure 7 in the manuscript,  $\rho_a \rho_b |t_{ab}|^2$  as a function of  $a_t E_{\text{cm}}$  for  $\eta^1 \eta^s \{^1P_1\} \rightarrow \eta^1 \eta^s \{^1P_1\}$  (blue),  $\omega^s \eta^s \{^3P_1\} \rightarrow \omega^s \eta^s \{^3P_1\}$  (red),  $f_1^s \eta^s \{^3S_1\} \rightarrow f_1^s \eta^s \{^3S_1\}$  (cyan), and  $h_1^s \eta^s \{^3S_1\} \rightarrow h_1^s \eta^s \{^3S_1\}$  (purple). Dashed lines indicate one standard deviation statistical uncertainties.

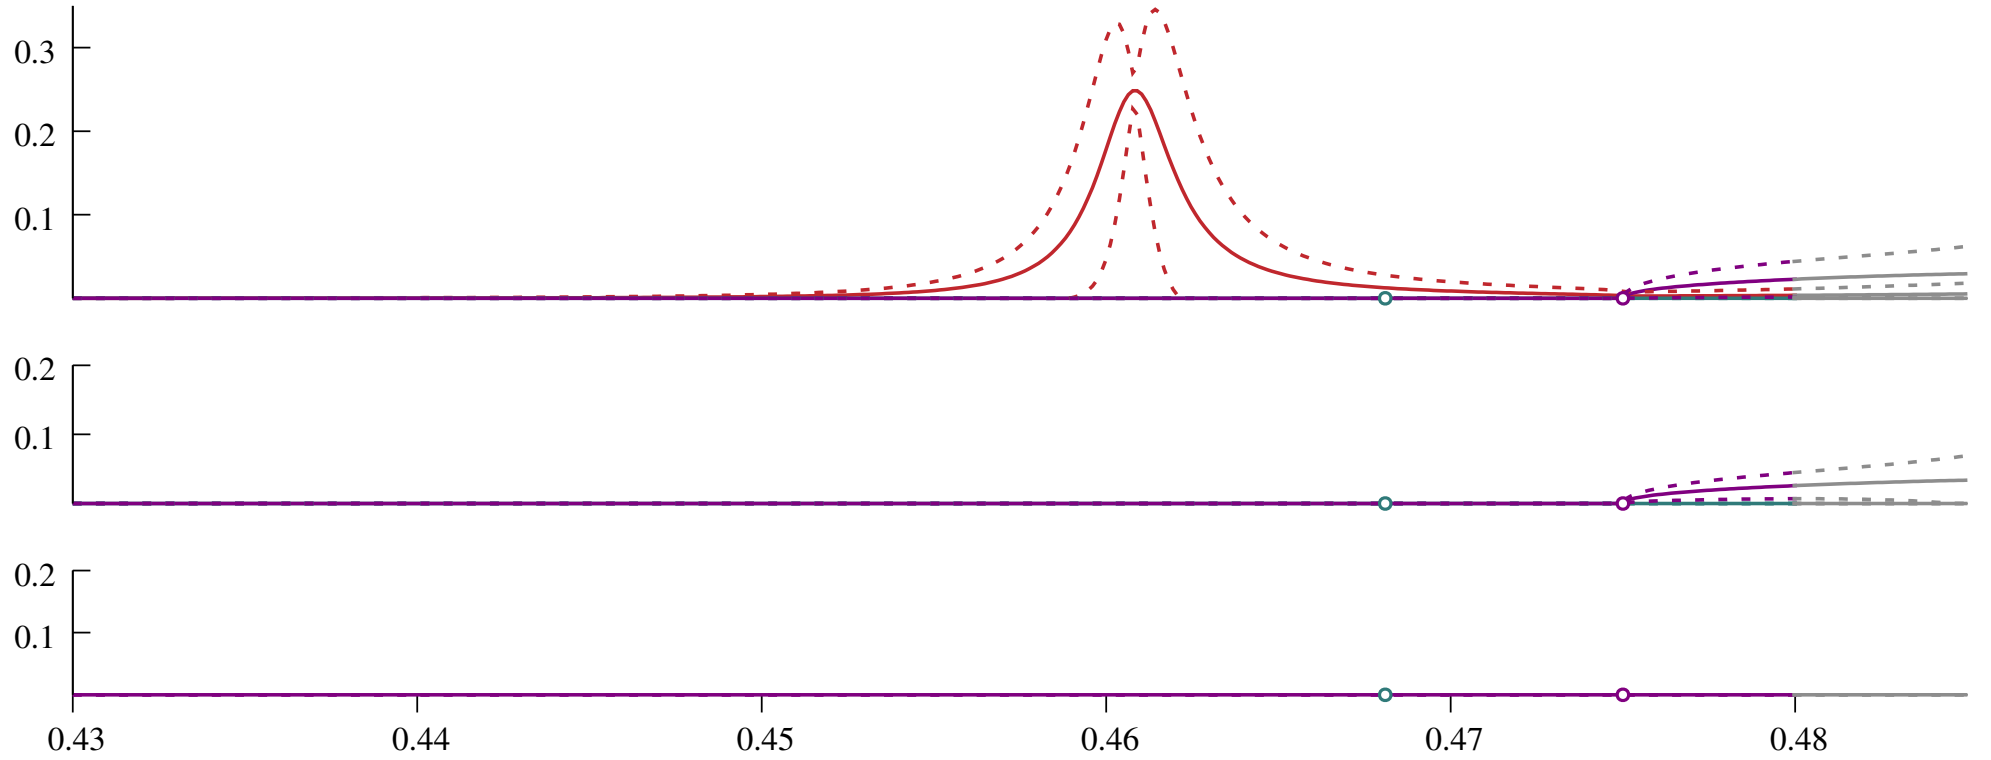

Figure 1.118: Similar to parts (b), (c) and (d) of Figure 7 in the manuscript,  $\rho_a \rho_b |t_{ab}|^2$  as a function of  $a_t E_{\text{cm}}$ . Top:  $\eta^1 \eta^s \{^1P_1\} \rightarrow \omega^s \eta^s \{^3P_1\}$  (red),  $\eta^1 \eta^s \{^1P_1\} \rightarrow f_1^s \eta^s \{^3S_1\}$  (cyan), and  $\eta^1 \eta^s \{^1P_1\} \rightarrow h_1^s \eta^s \{^3S_1\}$  (purple). Middle:  $\omega^s \eta^s \{^3P_1\} \rightarrow f_1^s \eta^s \{^3S_1\}$  (cyan), and  $\omega^s \eta^s \{^3P_1\} \rightarrow h_1^s \eta^s \{^3S_1\}$  (purple). Bottom:  $f_1^s \eta^s \{^3S_1\} \rightarrow h_1^s \eta^s \{^3S_1\}$  (purple). Dashed lines indicate one standard deviation statistical uncertainties.

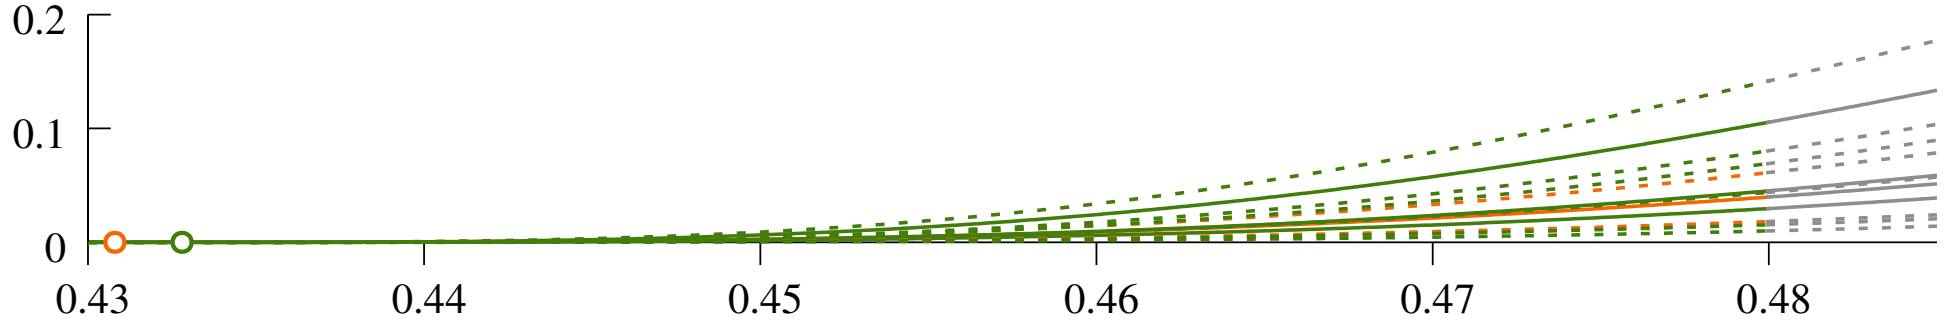

Figure 1.119: Similar to parts (e) and (f) of Figure 7 in the manuscript,  $\rho_a \rho_b |t_{ab}|^2$  as a function of  $a_t E_{cm}$  for  $\omega^s \omega^s \{^3P_1\} \rightarrow \omega^s \omega^s \{^3P_1\}$  (orange),  $\omega^1 \omega^s \{^1P_1, ^3P_1, ^5P_1\} \rightarrow \omega^s \omega^1 \{^1P_1, ^3P_1, ^5P_1\}$  (green). Dashed lines indicate one standard deviation statistical uncertainties.

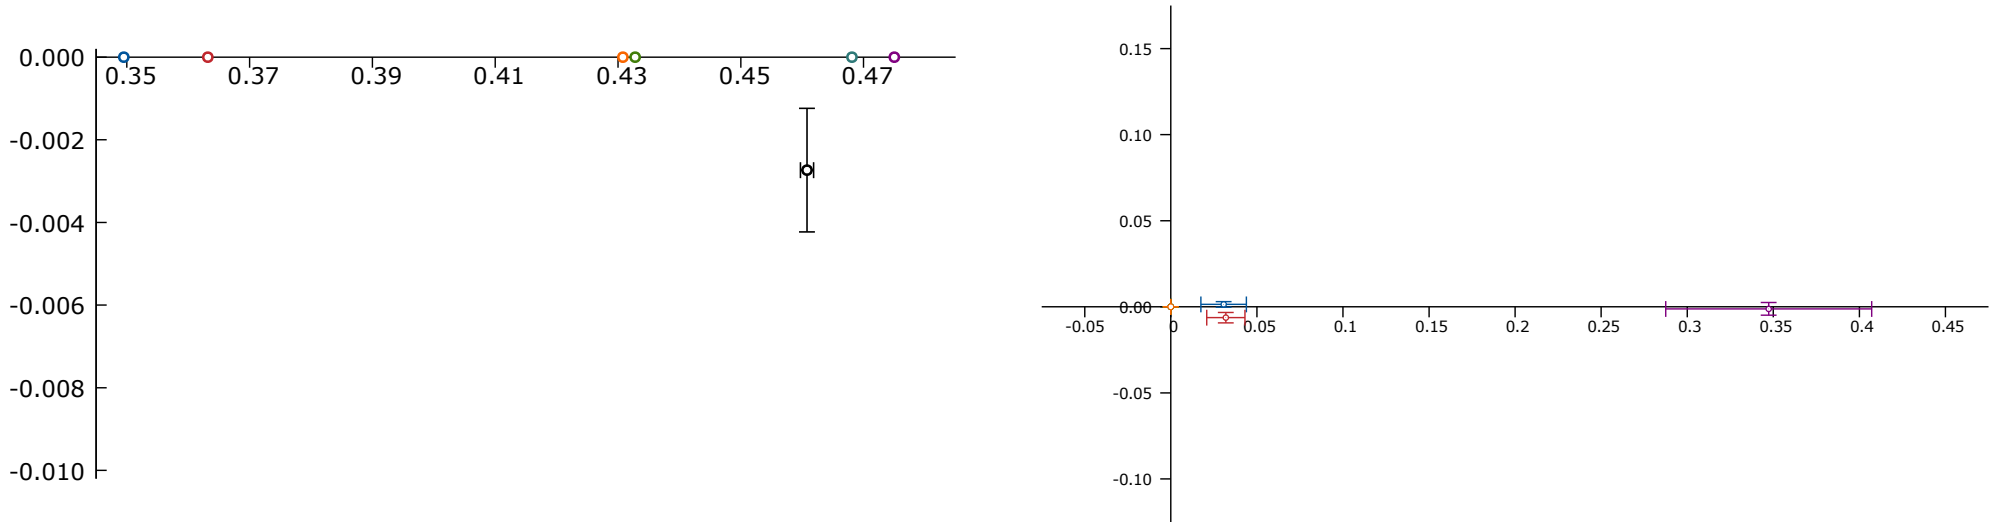

Figure 1.120: Left: Similar to Figure 13 in the manuscript, pole position on the proximal sheet (closest to physical scattering) with  $\text{Re}(a_t \sqrt{s})$  on the horizontal axis and  $2 \text{Im}(a_t \sqrt{s})$  on the vertical axis. Right: Similar to Figure 14 in the manuscript, the corresponding couplings with  $\text{Re}(a_t c)$  on the horizontal axis and  $\text{Im}(a_t c)$  on the vertical axis.

# 1.25 $\{m, g_{a,b,f}^{(0)}, g_a^{(1)}, \gamma_{(a,a),(b,b),(c,c),(d_1,d_1),(d_2,d_2),(d_3,d_3),(e,e)}^{(0)}\}(\mathbf{CM}_m)$

minimised with chisq/nDoF = 44.36 / (53 - 12) = 1.08

|                                                           |  |                        |  |      |       |       |       |       |       |       |       |       |       |       |       |
|-----------------------------------------------------------|--|------------------------|--|------|-------|-------|-------|-------|-------|-------|-------|-------|-------|-------|-------|
| =====                                                     |  |                        |  |      |       |       |       |       |       |       |       |       |       |       |       |
| JP1-_g_eta8:eta1/1^P_1_pole0_order0                       |  | -3.2167 +/- 1.5349     |  | 1.00 | -0.99 | -0.36 | -0.33 | -0.07 | -0.06 | 0.02  | 0.00  | 0.01  | 0.01  | 0.00  | -0.18 |
| JP1-_g_eta8:eta1/1^P_1_pole0_order1                       |  | 17.249 +/- 7.958       |  |      | 1.00  | 0.47  | 0.44  | 0.07  | 0.09  | -0.02 | -0.01 | -0.00 | -0.01 | -0.01 | 0.23  |
| JP1-_g_h8:eta8/3^S_1_pole0_order0                         |  | 1.2616 +/- 0.97214     |  |      |       | 1.00  | 0.92  | 0.10  | 0.31  | -0.04 | -0.00 | 0.07  | 0.02  | -0.01 | 0.19  |
| JP1-_g_omega8:eta8/3^P_1_pole0_order0                     |  | 0.39532 +/- 0.30181    |  |      |       |       | 1.00  | 0.12  | 0.28  | -0.25 | 0.02  | 0.06  | 0.02  | 0.00  | 0.12  |
| JP1-_gamma_eta8:eta1/1^P_1 eta8:eta1/1^P_1_order0         |  | 1.5725 +/- 0.60466     |  |      |       |       |       | 1.00  | 0.48  | 0.01  | 0.01  | 0.05  | 0.02  | 0.01  | -0.15 |
| JP1-_gamma_f8:eta8/3^S_1 f8:eta8/3^S_1_order0             |  | -2.0819 +/- 0.28483    |  |      |       |       |       |       | 1.00  | 0.03  | 0.03  | 0.08  | 0.04  | 0.04  | -0.03 |
| JP1-_gamma_omega8:eta8/3^P_1 omega8:eta8/3^P_1_order0     |  | -3.6142 +/- 0.62704    |  |      |       |       |       |       |       | 1.00  | 0.05  | 0.08  | 0.06  | 0.13  | 0.14  |
| JP1-_gamma_omega8:omega1/1^P_1 omega8:omega1/1^P_1_order0 |  | 9.5505 +/- 2.3517      |  |      |       |       |       |       |       |       | 1.00  | 0.06  | 0.39  | 0.43  | -0.06 |
| JP1-_gamma_omega8:omega1/3^P_1 omega8:omega1/3^P_1_order0 |  | 11.765 +/- 4.9149      |  |      |       |       |       |       |       |       |       | 1.00  | 0.14  | 0.10  | 0.01  |
| JP1-_gamma_omega8:omega1/5^P_1 omega8:omega1/5^P_1_order0 |  | 19.052 +/- 3.7083      |  |      |       |       |       |       |       |       |       |       | 1.00  | 0.46  | -0.10 |
| JP1-_gamma_omega8:omega8/3^P_1 omega8:omega8/3^P_1_order0 |  | 10.504 +/- 2.882       |  |      |       |       |       |       |       |       |       |       |       | 1.00  | -0.11 |
| JP1-_m_pole0                                              |  | 0.46134 +/- 0.00099275 |  |      |       |       |       |       |       |       |       |       |       |       | 1.00  |
| =====                                                     |  |                        |  |      |       |       |       |       |       |       |       |       |       |       |       |

Phase space prescription ::

pole0\_sub

eta8:eta1[-] f8:eta8[+] h8:eta8[-] omega8:eta8[-] omega8:omega1[-] omega8:omega8[-] lower half-plane

sqrt(s)\_pole = ( 0.4612 +/- 0.0010084)  
+ (i/2)\*(-0.0035963 +/- 0.0017867) [-0.08]

s\_pole = ( 0.2127 +/- 0.00092993)  
+ i\*(-0.0016586 +/- 0.00082434) [-0.08]

| eta8:eta1                | f8:eta8                  | h8:eta8                  | omega8:eta8              | omega8:omega1            | omega8:omega8            |
|--------------------------|--------------------------|--------------------------|--------------------------|--------------------------|--------------------------|
| k_re= 0.1495 +/- 0.0008  | k_re= -0.0047 +/- 0.0024 | k_re= -0.0033 +/- 0.0017 | k_re= 0.1406 +/- 0.0008  | k_re= 0.0797 +/- 0.0015  | k_re= 0.0824 +/- 0.0014  |
| k_im= -0.0014 +/- 0.0007 | k_im= 0.0374 +/- 0.0026  | k_im= 0.0525 +/- 0.0018  | k_im= -0.0015 +/- 0.0007 | k_im= -0.0026 +/- 0.0013 | k_im= -0.0025 +/- 0.0012 |
| corr= [-0.08]            | corr= [ 0.11]            | corr= [ 0.09]            | corr= [-0.08]            | corr= [-0.07]            | corr= [-0.07]            |

  

| eta8:eta1/1^P_1              | f8:eta8/3^S_1                | h8:eta8/3^S_1(*)              | omega8:eta8/3^P_1             | omega8:omega1/1^P_1          | omega8:omega1/3^P_1          | omega8:omega1/5^P_1          | omega8:omega8/3^P_1          |
|------------------------------|------------------------------|-------------------------------|-------------------------------|------------------------------|------------------------------|------------------------------|------------------------------|
| g = 0.0399 +/- 0.0136        | g = 0.0000 +/- 0.0000        | g = 0.3721 +/- 0.0237         | g = 0.0321 +/- 0.0104         | g = 0.0000 +/- 0.0000        | g = 0.0000 +/- 0.0000        | g = 0.0000 +/- 0.0000        | g = 0.0000 +/- 0.0000        |
| arg(g)/pi= 0.0009 +/- 0.0268 | arg(g)/pi= 0.5052 +/- 0.0099 | arg(g)/pi= -0.0052 +/- 0.0099 | arg(g)/pi= -0.0635 +/- 0.0139 | arg(g)/pi= 0.5052 +/- 0.0099 | arg(g)/pi= 0.5052 +/- 0.0099 | arg(g)/pi= 0.5052 +/- 0.0099 | arg(g)/pi= 0.5052 +/- 0.0099 |
| g_re= 0.0399 +/- 0.0136      | g_re= -0.0000 +/- 0.0000     | g_re= 0.3720 +/- 0.0238       | g_re= 0.0315 +/- 0.0101       | g_re= -0.0000 +/- 0.0000     | g_re= -0.0000 +/- 0.0000     | g_re= -0.0000 +/- 0.0000     | g_re= -0.0000 +/- 0.0000     |
| g_im= 0.0001 +/- 0.0033      | g_im= 0.0000 +/- 0.0000      | g_im= -0.0061 +/- 0.0113      | g_im= -0.0064 +/- 0.0028      | g_im= 0.0000 +/- 0.0000      | g_im= 0.0000 +/- 0.0000      | g_im= 0.0000 +/- 0.0000      | g_im= 0.0000 +/- 0.0000      |
| corr= [-0.62]                | corr= [-0.82]                | corr= [ 0.80]                 | corr= [-0.88]                 | corr= [-0.82]                | corr= [-0.82]                | corr= [-0.82]                | corr= [-0.82]                |

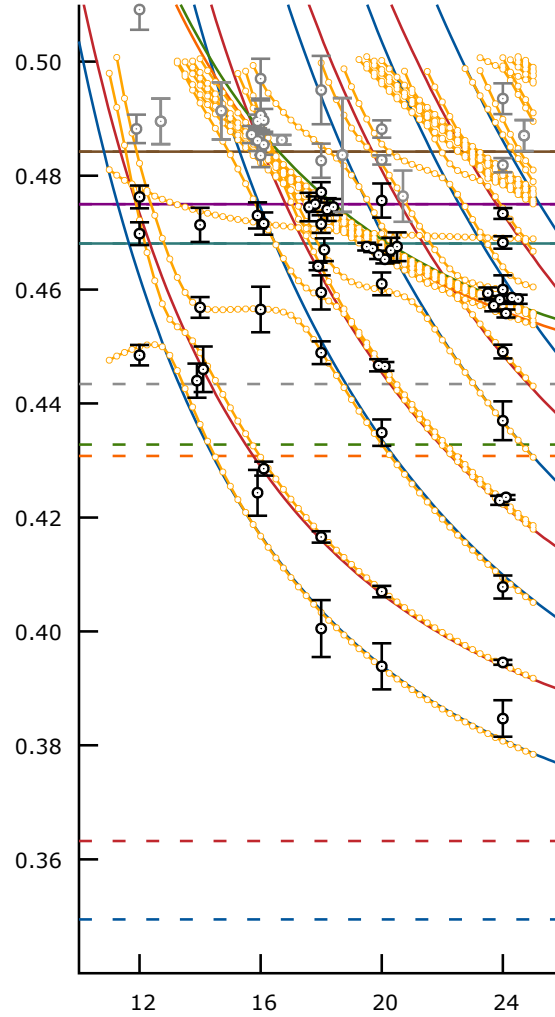

Figure 1.121: Similar to Figure 6 in the manuscript, the finite-volume spectrum, plotted as  $a_t E_{\text{cm}}$ , as a function of spatial extent  $L/a_s$ . Orange points/curves show the spectrum calculated from the amplitude given above (no uncertainties are shown). Black and grey points are the computed lattice energies on each volume, slightly displaced horizontally for clarity (black points correspond to energies used in the fit whereas grey points were not used). Two-meson non-interacting energies are shown as solid coloured curves/lines, two-meson thresholds are shown as dashed/solid horizontal lines, and the  $\eta^s \eta^s \eta^s$  threshold is shown as a dashed grey horizontal line.

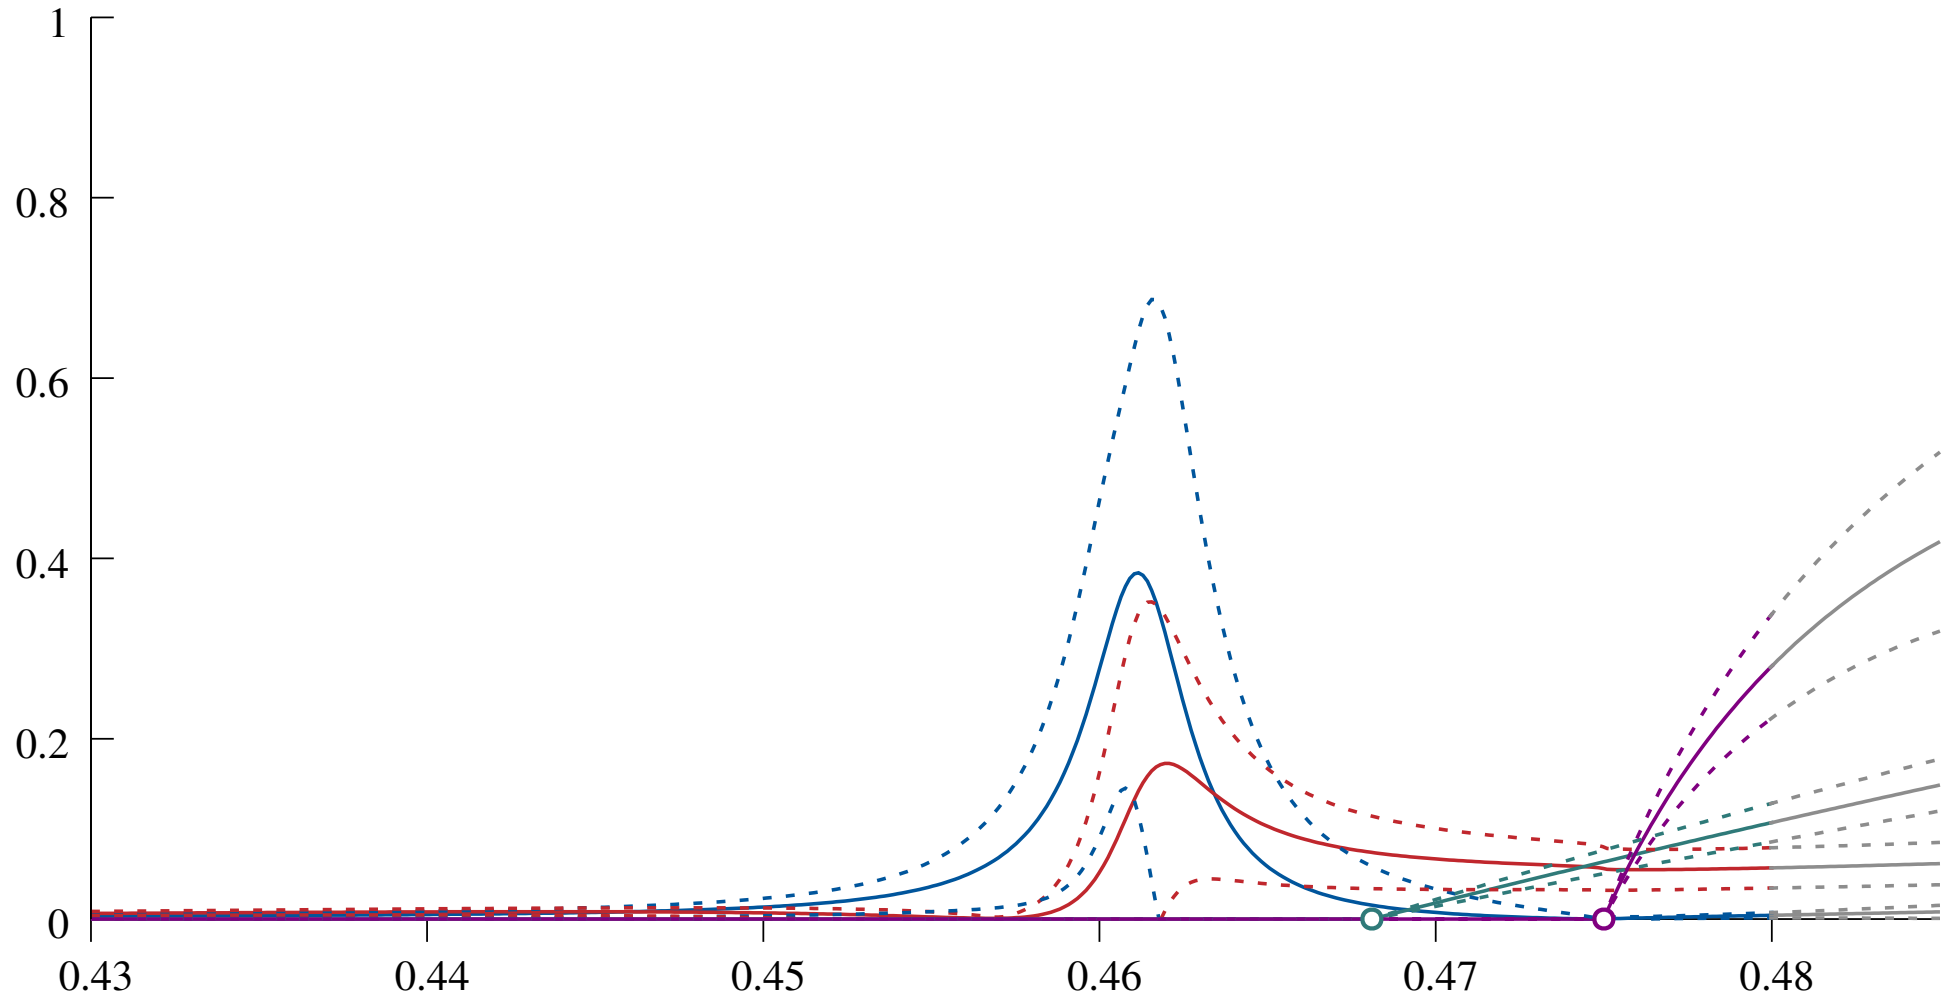

Figure 1.122: Similar to part (a) of Figure 7 in the manuscript,  $\rho_a \rho_b |t_{ab}|^2$  as a function of  $a_t E_{\text{cm}}$  for  $\eta^1 \eta^s \{^1P_1\} \rightarrow \eta^1 \eta^s \{^1P_1\}$  (blue),  $\omega^s \eta^s \{^3P_1\} \rightarrow \omega^s \eta^s \{^3P_1\}$  (red),  $f_1^s \eta^s \{^3S_1\} \rightarrow f_1^s \eta^s \{^3S_1\}$  (cyan), and  $h_1^s \eta^s \{^3S_1\} \rightarrow h_1^s \eta^s \{^3S_1\}$  (purple). Dashed lines indicate one standard deviation statistical uncertainties.

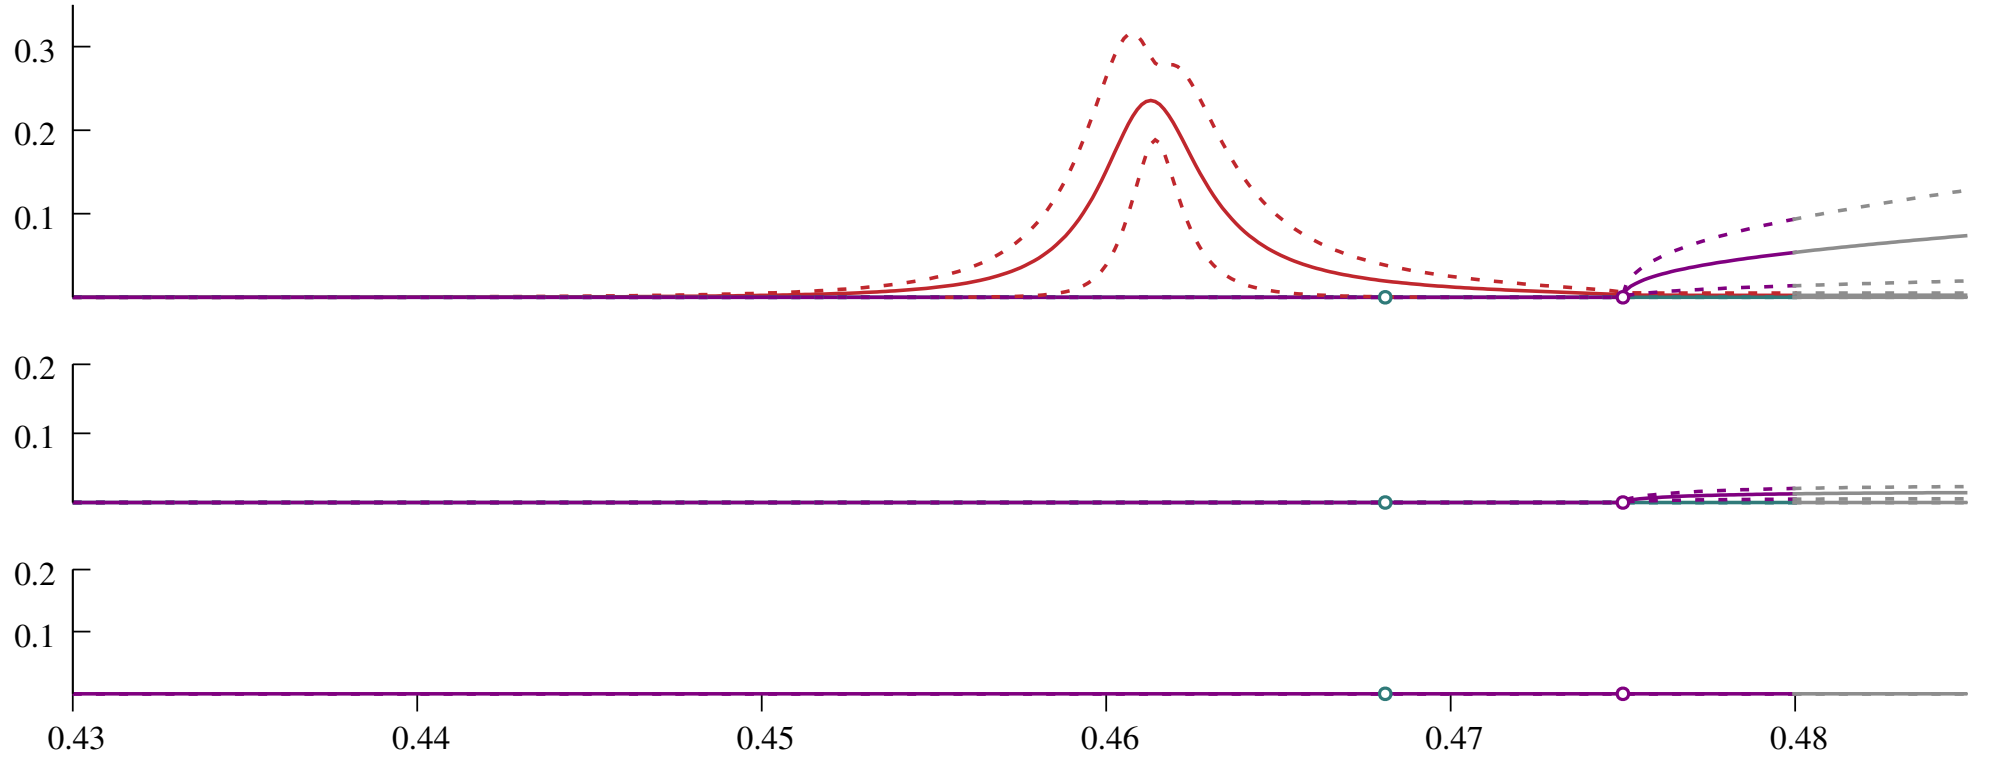

Figure 1.123: Similar to parts (b), (c) and (d) of Figure 7 in the manuscript,  $\rho_a \rho_b |t_{ab}|^2$  as a function of  $a_t E_{\text{cm}}$ . Top:  $\eta^1 \eta^s \{^1P_1\} \rightarrow \omega^s \eta^s \{^3P_1\}$  (red),  $\eta^1 \eta^s \{^1P_1\} \rightarrow f_1^s \eta^s \{^3S_1\}$  (cyan), and  $\eta^1 \eta^s \{^1P_1\} \rightarrow h_1^s \eta^s \{^3S_1\}$  (purple). Middle:  $\omega^s \eta^s \{^3P_1\} \rightarrow f_1^s \eta^s \{^3S_1\}$  (cyan), and  $\omega^s \eta^s \{^3P_1\} \rightarrow h_1^s \eta^s \{^3S_1\}$  (purple). Bottom:  $f_1^s \eta^s \{^3S_1\} \rightarrow h_1^s \eta^s \{^3S_1\}$  (purple). Dashed lines indicate one standard deviation statistical uncertainties.

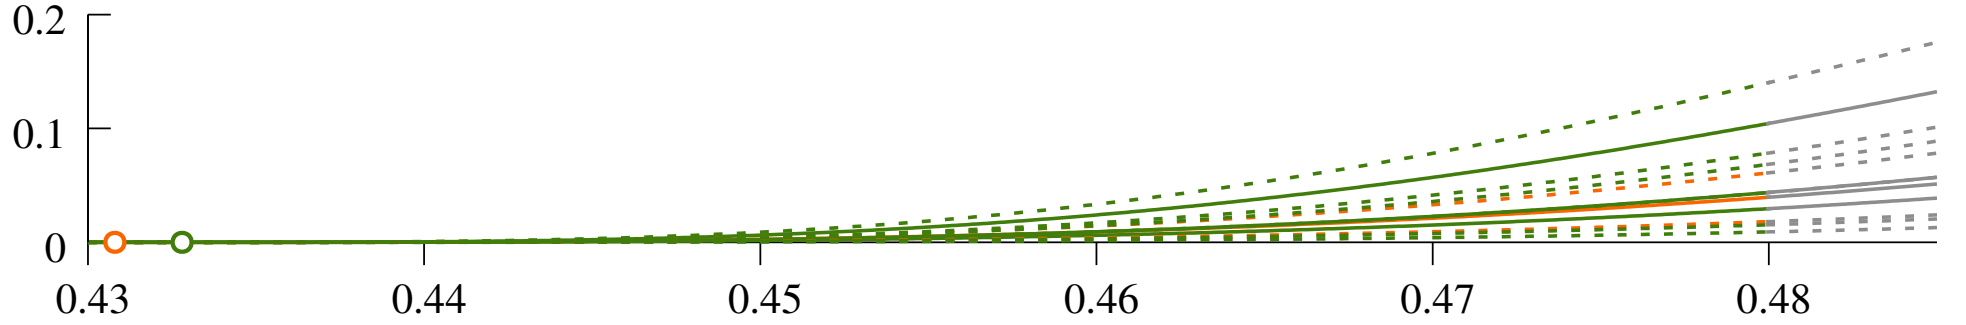

Figure 1.124: Similar to parts (e) and (f) of Figure 7 in the manuscript,  $\rho_a \rho_b |t_{ab}|^2$  as a function of  $a_t E_{cm}$  for  $\omega^s \omega^s \{^3P_1\} \rightarrow \omega^s \omega^s \{^3P_1\}$  (orange),  $\omega^1 \omega^s \{^1P_1, ^3P_1, ^5P_1\} \rightarrow \omega^s \omega^1 \{^1P_1, ^3P_1, ^5P_1\}$  (green). Dashed lines indicate one standard deviation statistical uncertainties.

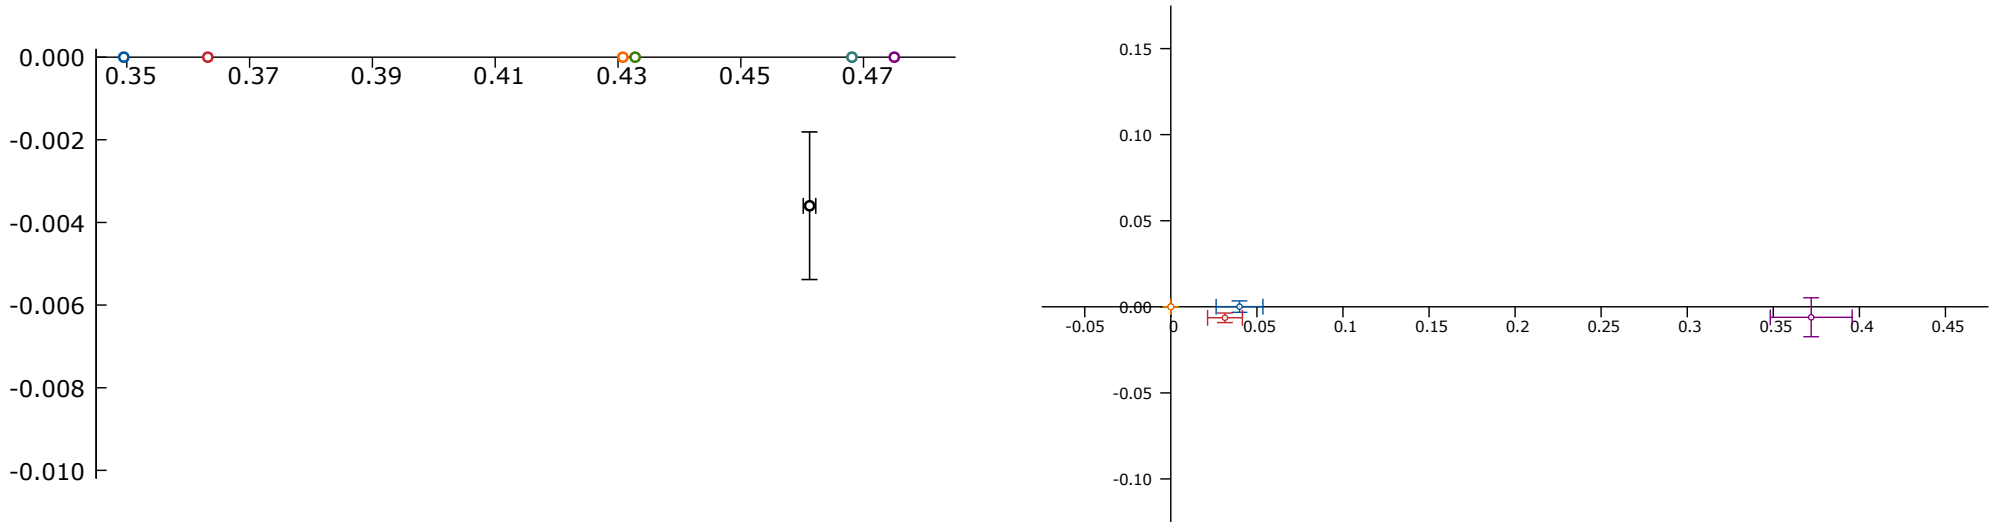

Figure 1.125: Left: Similar to Figure 13 in the manuscript, pole position on the proximal sheet (closest to physical scattering) with  $\text{Re}(a_t \sqrt{s})$  on the horizontal axis and  $2 \text{Im}(a_t \sqrt{s})$  on the vertical axis. Right: Similar to Figure 14 in the manuscript, the corresponding couplings with  $\text{Re}(a_t c)$  on the horizontal axis and  $\text{Im}(a_t c)$  on the vertical axis.

# 1.26 $\{m, g_{a,b,f}^{(0)}, g_b^{(1)}, \gamma_{(a,a),(b,b),(c,c),(d_1,d_1),(d_2,d_2),(d_3,d_3),(e,e)}^{(0)}\}(\mathbf{CM}_m)$

minimised with chisq/nDoF = 45.33 / (53 - 12) = 1.11

|                                                           |  |                       |  |      |      |       |       |       |       |       |       |       |                  |
|-----------------------------------------------------------|--|-----------------------|--|------|------|-------|-------|-------|-------|-------|-------|-------|------------------|
| =====                                                     |  |                       |  |      |      |       |       |       |       |       |       |       |                  |
| JP1-_g_eta8:eta1/1^P_1_pole0_order0                       |  | 0.21963 +/- 0.16331   |  | 1.00 | 0.79 | -0.08 | 0.21  | 0.12  | 0.27  | -0.12 | -0.04 | 0.02  | -0.07 -0.06 0.62 |
| JP1-_g_h8:eta8/3^S_1_pole0_order0                         |  | 0.87472 +/- 0.66019   |  |      | 1.00 | -0.05 | 0.22  | 0.29  | 0.40  | -0.22 | -0.01 | 0.05  | -0.01 -0.02 0.48 |
| JP1-_g_omega8:eta8/3^P_1_pole0_order0                     |  | -0.70197 +/- 1.0811   |  |      | 1.00 | -0.98 | -0.00 | -0.01 | -0.52 | -0.01 | -0.01 | -0.01 | -0.02 -0.03      |
| JP1-_g_omega8:eta8/3^P_1_pole0_order1                     |  | 4.7482 +/- 5.3339     |  |      |      | 1.00  | 0.06  | 0.08  | 0.45  | 0.02  | 0.02  | 0.01  | 0.02 0.10        |
| JP1-_gamma_eta8:eta1/1^P_1 eta8:eta1/1^P_1_order0         |  | 1.4449 +/- 0.56733    |  |      |      |       | 1.00  | 0.54  | -0.05 | 0.01  | 0.06  | 0.02  | 0.01 -0.04       |
| JP1-_gamma_f8:eta8/3^S_1 f8:eta8/3^S_1_order0             |  | -2.0991 +/- 0.30332   |  |      |      |       |       | 1.00  | -0.05 | 0.03  | 0.07  | 0.03  | 0.03 0.11        |
| JP1-_gamma_omega8:eta8/3^P_1 omega8:eta8/3^P_1_order0     |  | -3.1842 +/- 0.67354   |  |      |      |       |       |       | 1.00  | 0.07  | 0.07  | 0.07  | 0.15 -0.01       |
| JP1-_gamma_omega8:omega1/1^P_1 omega8:omega1/1^P_1_order0 |  | 9.5835 +/- 2.3553     |  |      |      |       |       |       |       | 1.00  | 0.05  | 0.39  | 0.43 -0.07       |
| JP1-_gamma_omega8:omega1/3^P_1 omega8:omega1/3^P_1_order0 |  | 12.074 +/- 4.9187     |  |      |      |       |       |       |       |       | 1.00  | 0.13  | 0.10 0.04        |
| JP1-_gamma_omega8:omega1/5^P_1 omega8:omega1/5^P_1_order0 |  | 19.251 +/- 3.7232     |  |      |      |       |       |       |       |       |       | 1.00  | 0.46 -0.10       |
| JP1-_gamma_omega8:omega8/3^P_1 omega8:omega8/3^P_1_order0 |  | 10.572 +/- 2.89       |  |      |      |       |       |       |       |       |       |       | 1.00 -0.11       |
| JP1-_m_pole0                                              |  | 0.46077 +/- 0.0010239 |  |      |      |       |       |       |       |       |       |       | 1.00             |
| =====                                                     |  |                       |  |      |      |       |       |       |       |       |       |       |                  |

Phase space prescription ::

pole0\_sub

eta8:eta1[-] f8:eta8[+] h8:eta8[+] omega8:eta8[-] omega8:omega1[-] omega8:omega8[-] lower half-plane

sqrt(s)\_pole = (0.46067 +/- 0.0010332)  
+ (i/2)\*(-0.0025791 +/- 0.0013117) [ 0.05]

s\_pole = (0.21221 +/- 0.00095198)  
+ i\*(-0.0011881 +/- 0.00060414) [ 0.05]

| eta8:eta1                | f8:eta8                  | h8:eta8                  | omega8:eta8              | omega8:omega1            | omega8:omega8            |
|--------------------------|--------------------------|--------------------------|--------------------------|--------------------------|--------------------------|
| k_re= 0.1491 +/- 0.0008  | k_re= -0.0033 +/- 0.0017 | k_re= -0.0023 +/- 0.0012 | k_re= 0.1402 +/- 0.0008  | k_re= 0.0789 +/- 0.0015  | k_re= 0.0816 +/- 0.0015  |
| k_im= -0.0010 +/- 0.0005 | k_im= 0.0387 +/- 0.0026  | k_im= 0.0534 +/- 0.0019  | k_im= -0.0010 +/- 0.0005 | k_im= -0.0019 +/- 0.0010 | k_im= -0.0018 +/- 0.0009 |
| corr= [ 0.06]            | corr= [ 0.03]            | corr= [-0.01]            | corr= [ 0.06]            | corr= [ 0.07]            | corr= [ 0.07]            |

  

| eta8:eta1/1^P_1              | f8:eta8/3^S_1                | h8:eta8/3^S_1(*)             | omega8:eta8/3^P_1             | omega8:omega1/1^P_1          | omega8:omega1/3^P_1          | omega8:omega1/5^P_1          | omega8:omega8/3^P_1          |
|------------------------------|------------------------------|------------------------------|-------------------------------|------------------------------|------------------------------|------------------------------|------------------------------|
| g = 0.0267 +/- 0.0120        | g = 0.0000 +/- 0.0000        | g = 0.3575 +/- 0.0421        | g = 0.0345 +/- 0.0111         | g = 0.0000 +/- 0.0000        | g = 0.0000 +/- 0.0000        | g = 0.0000 +/- 0.0000        | g = 0.0000 +/- 0.0000        |
| arg(g)/pi= 0.0251 +/- 0.0117 | arg(g)/pi= 0.4994 +/- 0.0052 | arg(g)/pi= 0.0006 +/- 0.0052 | arg(g)/pi= -0.0558 +/- 0.0110 | arg(g)/pi= 0.4994 +/- 0.0052 | arg(g)/pi= 0.4994 +/- 0.0052 | arg(g)/pi= 0.4994 +/- 0.0052 | arg(g)/pi= 0.4994 +/- 0.0052 |
| g_re= 0.0266 +/- 0.0119      | g_re= 0.0000 +/- 0.0000      | g_re= 0.3574 +/- 0.0421      | g_re= 0.0340 +/- 0.0109       | g_re= 0.0000 +/- 0.0000      | g_re= 0.0000 +/- 0.0000      | g_re= 0.0000 +/- 0.0000      | g_re= 0.0000 +/- 0.0000      |
| g_im= 0.0021 +/- 0.0013      | g_im= 0.0000 +/- 0.0000      | g_im= 0.0007 +/- 0.0059      | g_im= -0.0060 +/- 0.0027      | g_im= 0.0000 +/- 0.0000      | g_im= 0.0000 +/- 0.0000      | g_im= 0.0000 +/- 0.0000      | g_im= 0.0000 +/- 0.0000      |
| corr= [ 0.64]                | corr= [-0.58]                | corr= [ 0.60]                | corr= [-0.92]                 | corr= [-0.58]                | corr= [-0.58]                | corr= [-0.58]                | corr= [-0.58]                |

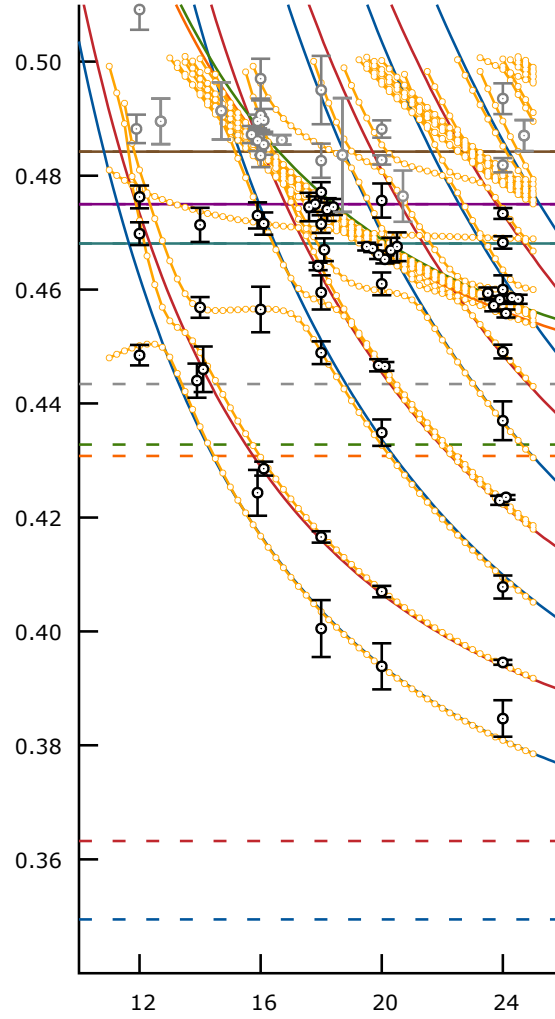

Figure 1.126: Similar to Figure 6 in the manuscript, the finite-volume spectrum, plotted as  $a_t E_{\text{cm}}$ , as a function of spatial extent  $L/a_s$ . Orange points/curves show the spectrum calculated from the amplitude given above (no uncertainties are shown). Black and grey points are the computed lattice energies on each volume, slightly displaced horizontally for clarity (black points correspond to energies used in the fit whereas grey points were not used). Two-meson non-interacting energies are shown as solid coloured curves/lines, two-meson thresholds are shown as dashed/solid horizontal lines, and the  $\eta^s \eta^s \eta^s$  threshold is shown as a dashed grey horizontal line.

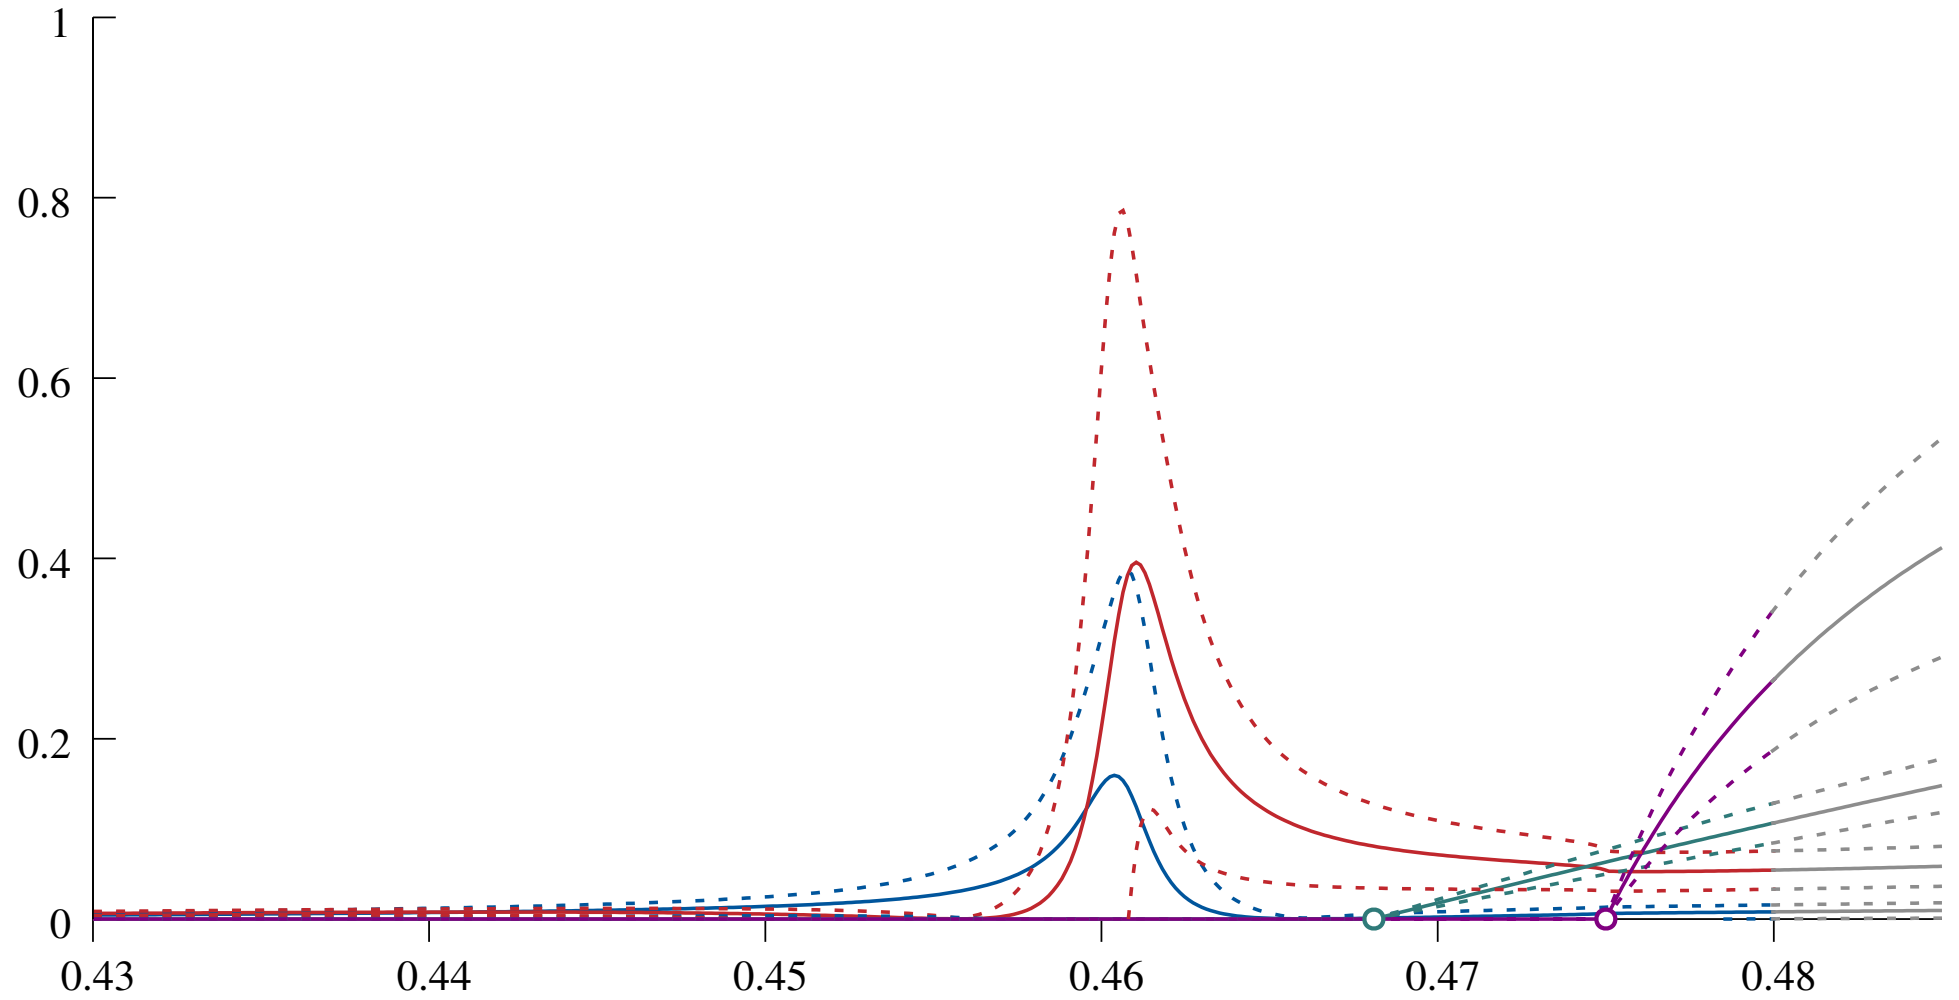

Figure 1.127: Similar to part (a) of Figure 7 in the manuscript,  $\rho_a \rho_b |t_{ab}|^2$  as a function of  $a_t E_{\text{cm}}$  for  $\eta^1 \eta^s \{^1P_1\} \rightarrow \eta^1 \eta^s \{^1P_1\}$  (blue),  $\omega^s \eta^s \{^3P_1\} \rightarrow \omega^s \eta^s \{^3P_1\}$  (red),  $f_1^s \eta^s \{^3S_1\} \rightarrow f_1^s \eta^s \{^3S_1\}$  (cyan), and  $h_1^s \eta^s \{^3S_1\} \rightarrow h_1^s \eta^s \{^3S_1\}$  (purple). Dashed lines indicate one standard deviation statistical uncertainties.

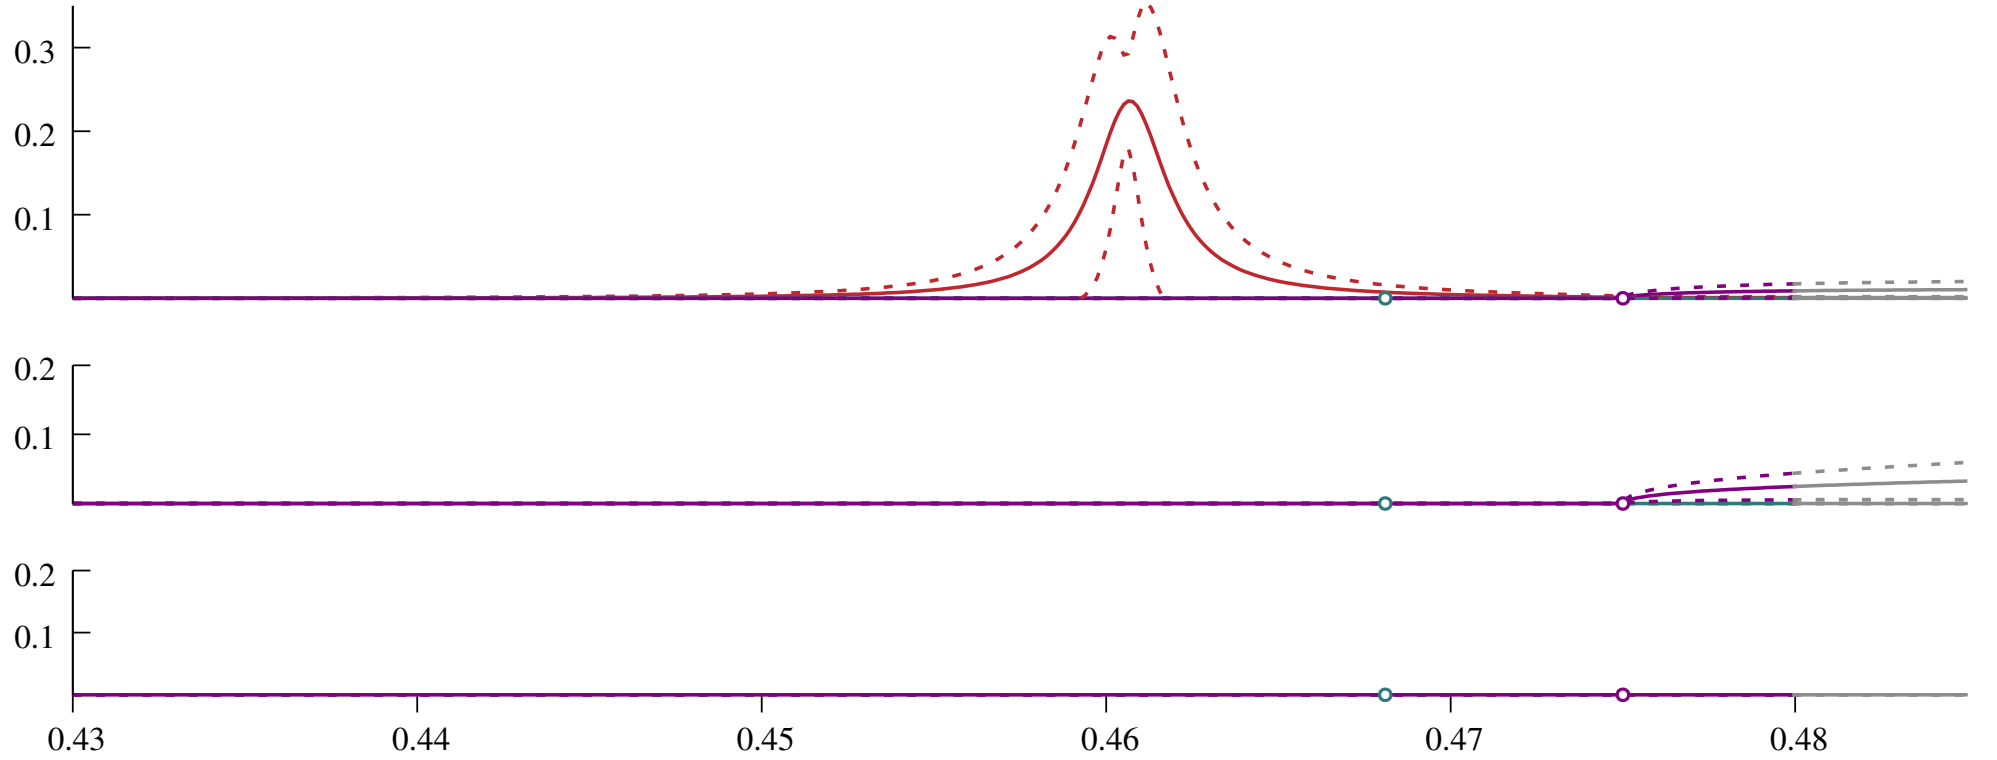

Figure 1.128: Similar to parts (b), (c) and (d) of Figure 7 in the manuscript,  $\rho_a \rho_b |t_{ab}|^2$  as a function of  $a_t E_{\text{cm}}$ . Top:  $\eta^1 \eta^s \{^1P_1\} \rightarrow \omega^s \eta^s \{^3P_1\}$  (red),  $\eta^1 \eta^s \{^1P_1\} \rightarrow f_1^s \eta^s \{^3S_1\}$  (cyan), and  $\eta^1 \eta^s \{^1P_1\} \rightarrow h_1^s \eta^s \{^3S_1\}$  (purple). Middle:  $\omega^s \eta^s \{^3P_1\} \rightarrow f_1^s \eta^s \{^3S_1\}$  (cyan), and  $\omega^s \eta^s \{^3P_1\} \rightarrow h_1^s \eta^s \{^3S_1\}$  (purple). Bottom:  $f_1^s \eta^s \{^3S_1\} \rightarrow h_1^s \eta^s \{^3S_1\}$  (purple). Dashed lines indicate one standard deviation statistical uncertainties.

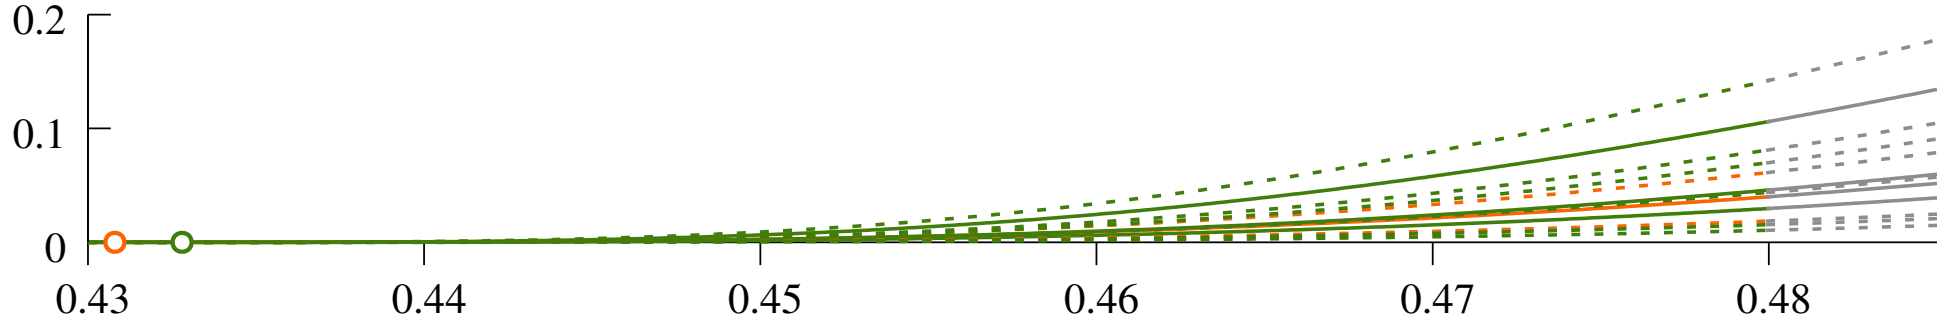

Figure 1.129: Similar to parts (e) and (f) of Figure 7 in the manuscript,  $\rho_a \rho_b |t_{ab}|^2$  as a function of  $a_t E_{cm}$  for  $\omega^s \omega^s \{^3P_1\} \rightarrow \omega^s \omega^s \{^3P_1\}$  (orange),  $\omega^1 \omega^s \{^1P_1, ^3P_1, ^5P_1\} \rightarrow \omega^s \omega^1 \{^1P_1, ^3P_1, ^5P_1\}$  (green). Dashed lines indicate one standard deviation statistical uncertainties.

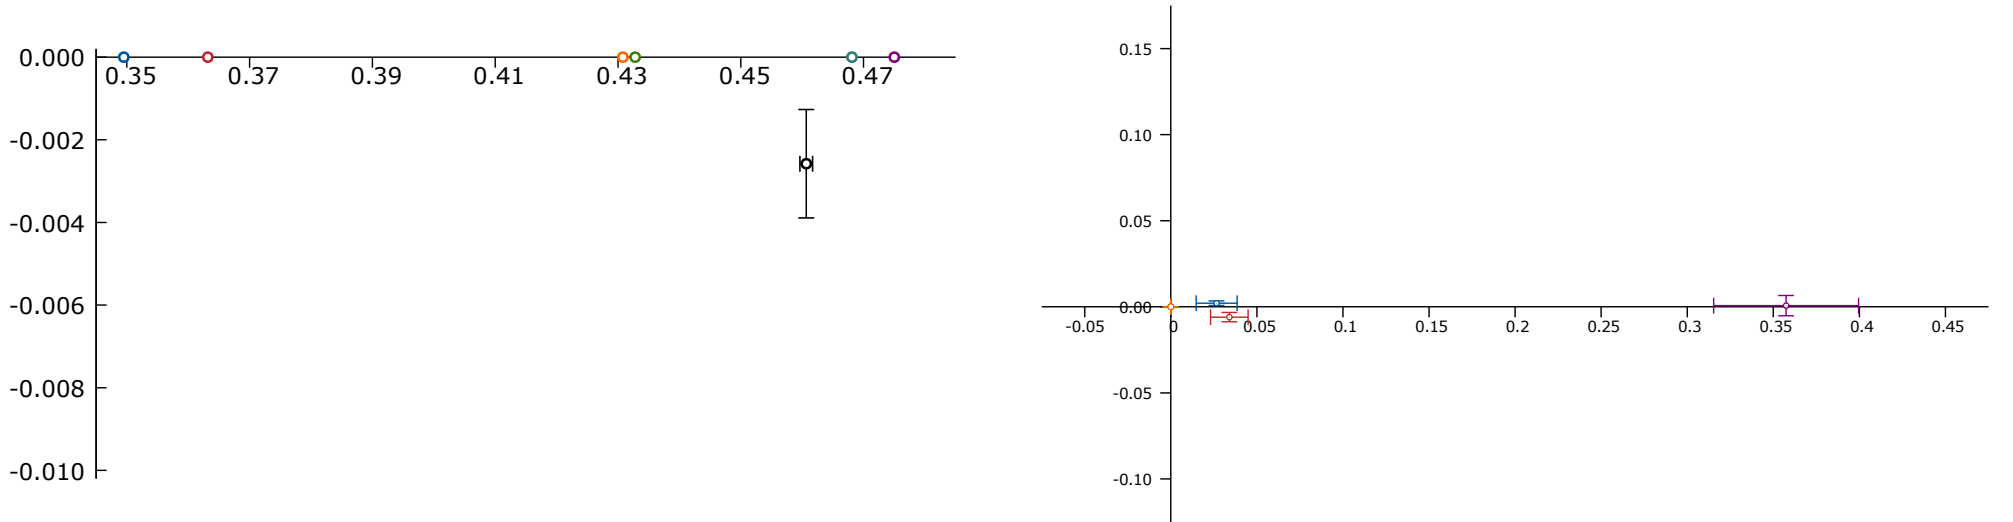

Figure 1.130: Left: Similar to Figure 13 in the manuscript, pole position on the proximal sheet (closest to physical scattering) with  $\text{Re}(a_t \sqrt{s})$  on the horizontal axis and  $2 \text{Im}(a_t \sqrt{s})$  on the vertical axis. Right: Similar to Figure 14 in the manuscript, the corresponding couplings with  $\text{Re}(a_t c)$  on the horizontal axis and  $\text{Im}(a_t c)$  on the vertical axis.

## 1.27 $\{m, g_{a,b}^{(0)}, g_f^{(1)}, \gamma_{(a,a),(b,b),(c,c),(\mathfrak{d}_1,\mathfrak{d}_1),(\mathfrak{d}_2,\mathfrak{d}_2),(\mathfrak{d}_3,\mathfrak{d}_3),(c,c)}^{(0)}\}(\mathbf{CM}_m)$

minimised with chisq/nDoF = 45.77 / (53 - 11) = 1.09

|                                                          |  |                        |  |      |      |      |      |      |       |       |      |       |       |       |
|----------------------------------------------------------|--|------------------------|--|------|------|------|------|------|-------|-------|------|-------|-------|-------|
| JP1-g_eta8:eta1/1^P_1_pole0_order0                       |  | 0.19530 +/- 0.14127    |  | 1.00 | 0.72 | 0.63 | 0.09 | 0.26 | -0.04 | -0.03 | 0.02 | -0.06 | -0.05 | 0.61  |
| JP1-g_h8:eta8/3^S_1_pole0_order1                         |  | 4.0131 +/- 2.9569      |  |      | 1.00 | 0.88 | 0.32 | 0.43 | -0.13 | 0.01  | 0.06 | 0.01  | 0.00  | 0.48  |
| JP1-g_omega8:eta8/3^P_1_pole0_order0                     |  | 0.26613 +/- 0.18063    |  |      |      | 1.00 | 0.31 | 0.38 | -0.40 | 0.03  | 0.05 | 0.02  | 0.02  | 0.35  |
| JP1-gamma_eta8:eta1/1^P_1 eta8:eta1/1^P_1_order0         |  | 1.4273 +/- 0.56916     |  |      |      |      | 1.00 | 0.55 | -0.04 | 0.02  | 0.06 | 0.03  | 0.02  | -0.03 |
| JP1-gamma_f8:eta8/3^S_1 f8:eta8/3^S_1_order0             |  | -2.1082 +/- 0.30838    |  |      |      |      |      | 1.00 | -0.02 | 0.04  | 0.08 | 0.04  | 0.04  | 0.13  |
| JP1-gamma_omega8:eta8/3^P_1 omega8:eta8/3^P_1_order0     |  | -3.6784 +/- 0.66242    |  |      |      |      |      |      | 1.00  | 0.04  | 0.07 | 0.05  | 0.11  | 0.10  |
| JP1-gamma_omega8:omega1/1^P_1 omega8:omega1/1^P_1_order0 |  | 9.5952 +/- 2.3644      |  |      |      |      |      |      |       | 1.00  | 0.06 | 0.39  | 0.43  | -0.06 |
| JP1-gamma_omega8:omega1/3^P_1 omega8:omega1/3^P_1_order0 |  | 12.085 +/- 4.9344      |  |      |      |      |      |      |       |       | 1.00 | 0.13  | 0.10  | 0.05  |
| JP1-gamma_omega8:omega1/5^P_1 omega8:omega1/5^P_1_order0 |  | 19.311 +/- 3.7408      |  |      |      |      |      |      |       |       |      | 1.00  | 0.46  | -0.09 |
| JP1-gamma_omega8:omega8/3^P_1 omega8:omega8/3^P_1_order0 |  | 10.586 +/- 2.9008      |  |      |      |      |      |      |       |       |      |       | 1.00  | -0.10 |
| JP1-m_pole0                                              |  | 0.46071 +/- 0.00098952 |  |      |      |      |      |      |       |       |      |       |       | 1.00  |

Phase space prescription ::

pole0\_sub

eta8:eta1[-] f8:eta8[+] h8:eta8[+] omega8:eta8[-] omega8:omega1[-] omega8:omega8[-] lower half-plane

sqrt(s)\_pole = (0.46064 +/- 0.00097809)  
+ (i/2)\*(-0.002078 +/- 0.0011781) [ 0.07]

s\_pole = (0.21219 +/- 0.00090119)  
+ i\*(-0.00095722 +/- 0.00054254) [ 0.07]

| eta8:eta1                | f8:eta8                  | h8:eta8                  | omega8:eta8              | omega8:omega1            | omega8:omega8            |
|--------------------------|--------------------------|--------------------------|--------------------------|--------------------------|--------------------------|
| k_re= 0.1490 +/- 0.0007  | k_re= -0.0026 +/- 0.0015 | k_re= -0.0019 +/- 0.0011 | k_re= 0.1401 +/- 0.0008  | k_re= 0.0789 +/- 0.0014  | k_re= 0.0816 +/- 0.0014  |
| k_im= -0.0008 +/- 0.0005 | k_im= 0.0387 +/- 0.0025  | k_im= 0.0534 +/- 0.0018  | k_im= -0.0008 +/- 0.0005 | k_im= -0.0015 +/- 0.0009 | k_im= -0.0015 +/- 0.0008 |
| corr= [ 0.07]            | corr= [ 0.01]            | corr= [-0.03]            | corr= [ 0.08]            | corr= [ 0.09]            | corr= [ 0.09]            |

  

| eta8:eta1/1^P_1              | f8:eta8/3^S_1                | h8:eta8/3^S_1(*)             | omega8:eta8/3^P_1             | omega8:omega1/1^P_1          | omega8:omega1/3^P_1          | omega8:omega1/5^P_1          | omega8:omega8/3^P_1          |
|------------------------------|------------------------------|------------------------------|-------------------------------|------------------------------|------------------------------|------------------------------|------------------------------|
| g = 0.0243 +/- 0.0122        | g = 0.0000 +/- 0.0000        | g = 0.3565 +/- 0.0446        | g = 0.0307 +/- 0.0102         | g = 0.0000 +/- 0.0000        | g = 0.0000 +/- 0.0000        | g = 0.0000 +/- 0.0000        | g = 0.0000 +/- 0.0000        |
| arg(g)/pi= 0.0302 +/- 0.0113 | arg(g)/pi= 0.4957 +/- 0.0030 | arg(g)/pi= 0.0043 +/- 0.0030 | arg(g)/pi= -0.0516 +/- 0.0093 | arg(g)/pi= 0.4957 +/- 0.0030 | arg(g)/pi= 0.4957 +/- 0.0030 | arg(g)/pi= 0.4957 +/- 0.0030 | arg(g)/pi= 0.4957 +/- 0.0030 |
| g_re= 0.0242 +/- 0.0122      | g_re= 0.0000 +/- 0.0000      | g_re= 0.3565 +/- 0.0446      | g_re= 0.0303 +/- 0.0100       | g_re= 0.0000 +/- 0.0000      | g_re= 0.0000 +/- 0.0000      | g_re= 0.0000 +/- 0.0000      | g_re= 0.0000 +/- 0.0000      |
| g_im= 0.0023 +/- 0.0013      | g_im= 0.0000 +/- 0.0000      | g_im= 0.0048 +/- 0.0038      | g_im= -0.0050 +/- 0.0022      | g_im= 0.0000 +/- 0.0000      | g_im= 0.0000 +/- 0.0000      | g_im= 0.0000 +/- 0.0000      | g_im= 0.0000 +/- 0.0000      |
| corr= [ 0.77]                | corr= [-0.44]                | corr= [ 0.67]                | corr= [-0.93]                 | corr= [-0.44]                | corr= [-0.44]                | corr= [-0.44]                | corr= [-0.44]                |

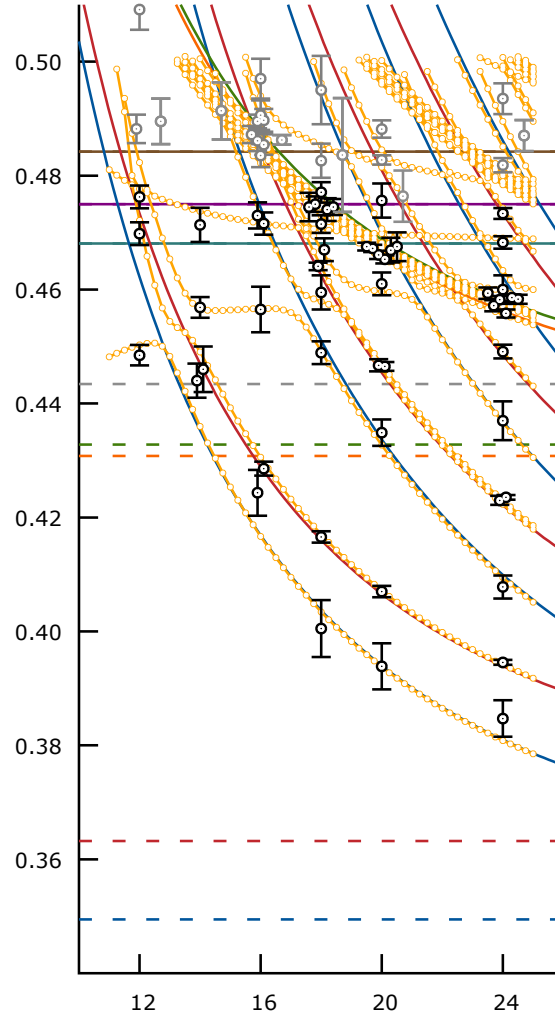

Figure 1.131: Similar to Figure 6 in the manuscript, the finite-volume spectrum, plotted as  $a_t E_{\text{cm}}$ , as a function of spatial extent  $L/a_s$ . Orange points/curves show the spectrum calculated from the amplitude given above (no uncertainties are shown). Black and grey points are the computed lattice energies on each volume, slightly displaced horizontally for clarity (black points correspond to energies used in the fit whereas grey points were not used). Two-meson non-interacting energies are shown as solid coloured curves/lines, two-meson thresholds are shown as dashed/solid horizontal lines, and the  $\eta^s \eta^s \eta^s$  threshold is shown as a dashed grey horizontal line.

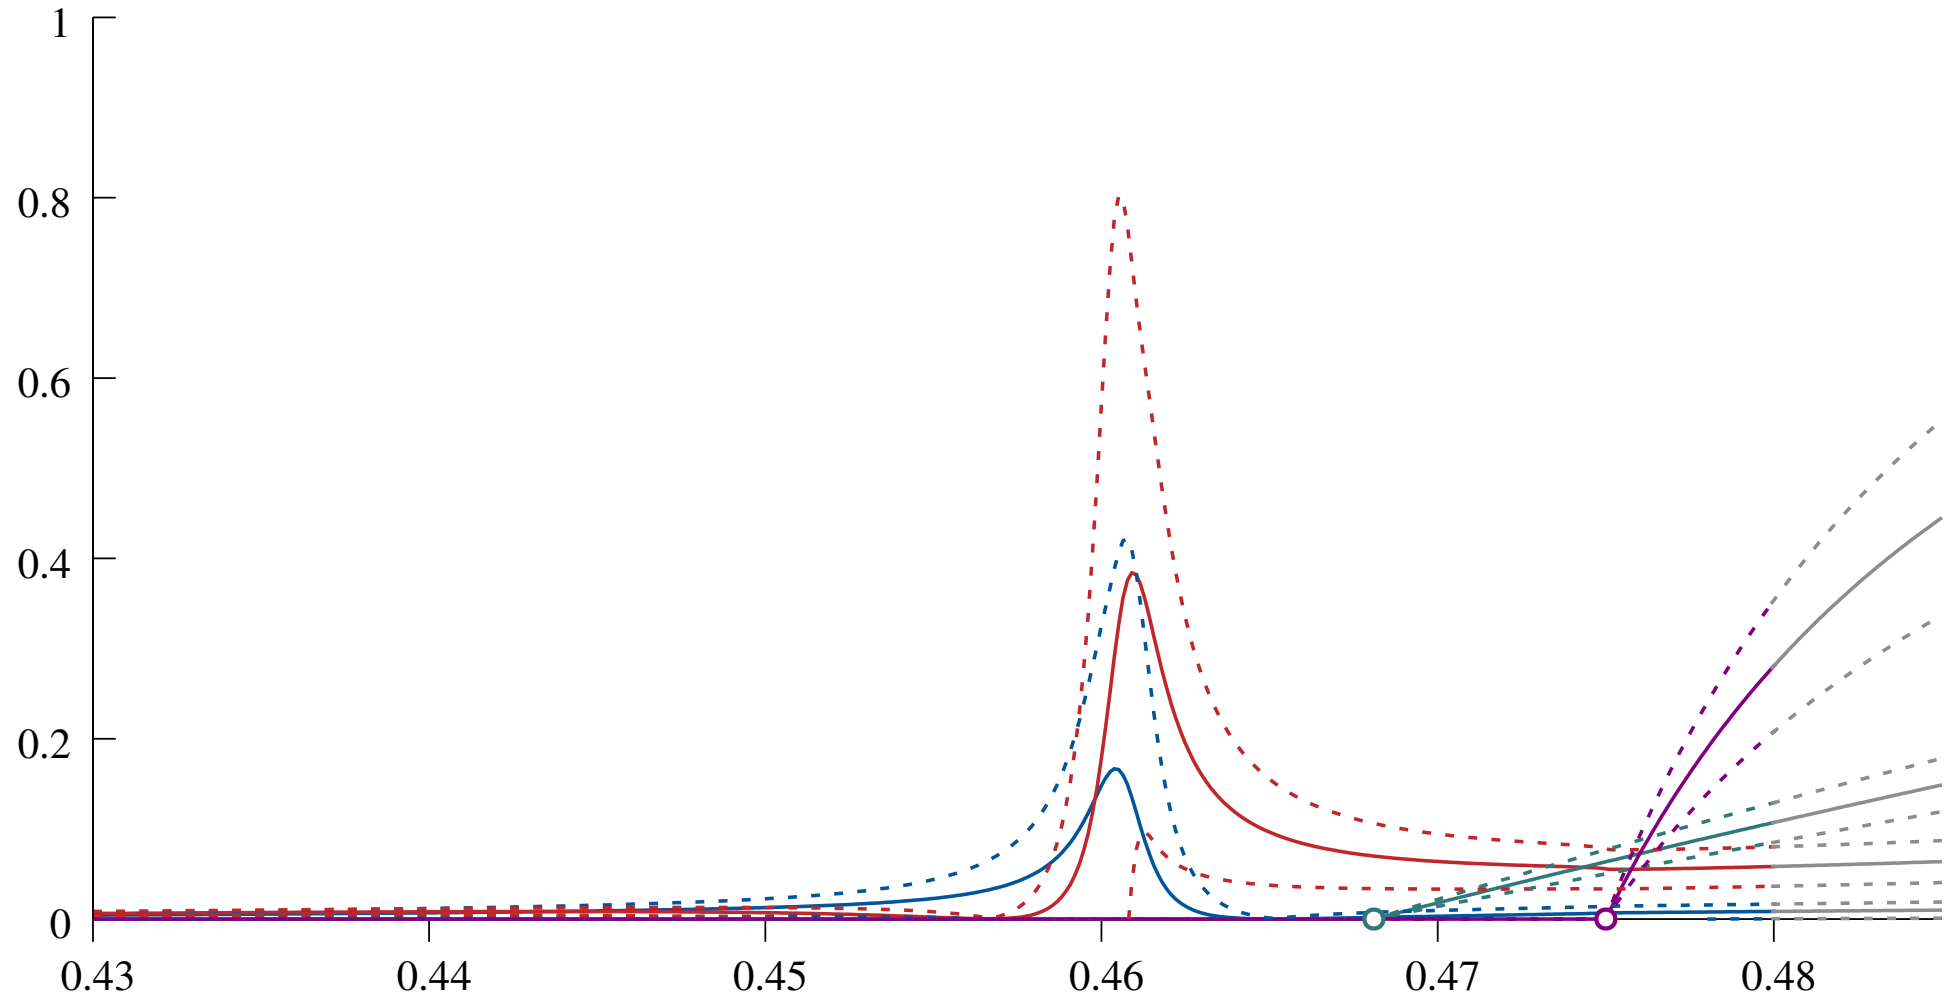

Figure 1.132: Similar to part (a) of Figure 7 in the manuscript,  $\rho_a \rho_b |t_{ab}|^2$  as a function of  $a_t E_{cm}$  for  $\eta^1 \eta^s \{^1P_1\} \rightarrow \eta^1 \eta^s \{^1P_1\}$  (blue),  $\omega^s \eta^s \{^3P_1\} \rightarrow \omega^s \eta^s \{^3P_1\}$  (red),  $f_1^s \eta^s \{^3S_1\} \rightarrow f_1^s \eta^s \{^3S_1\}$  (cyan), and  $h_1^s \eta^s \{^3S_1\} \rightarrow h_1^s \eta^s \{^3S_1\}$  (purple). Dashed lines indicate one standard deviation statistical uncertainties.

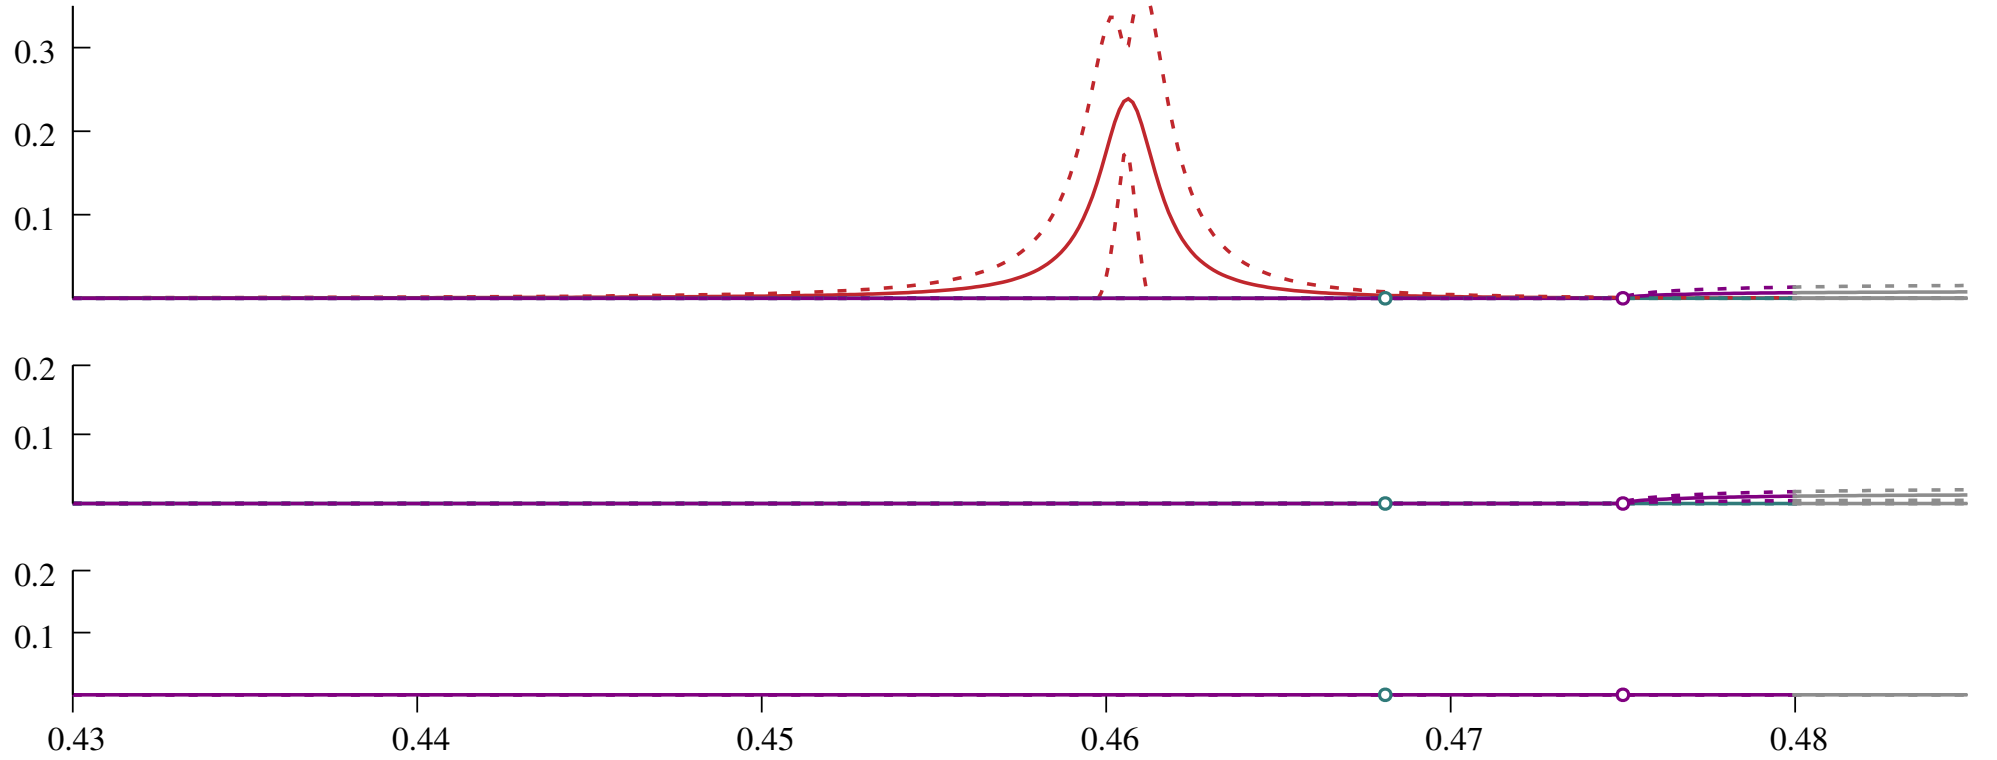

Figure 1.133: Similar to parts (b), (c) and (d) of Figure 7 in the manuscript,  $\rho_a \rho_b |t_{ab}|^2$  as a function of  $a_t E_{\text{cm}}$ . Top:  $\eta^1 \eta^s \{^1P_1\} \rightarrow \omega^s \eta^s \{^3P_1\}$  (red),  $\eta^1 \eta^s \{^1P_1\} \rightarrow f_1^s \eta^s \{^3S_1\}$  (cyan), and  $\eta^1 \eta^s \{^1P_1\} \rightarrow h_1^s \eta^s \{^3S_1\}$  (purple). Middle:  $\omega^s \eta^s \{^3P_1\} \rightarrow f_1^s \eta^s \{^3S_1\}$  (cyan), and  $\omega^s \eta^s \{^3P_1\} \rightarrow h_1^s \eta^s \{^3S_1\}$  (purple). Bottom:  $f_1^s \eta^s \{^3S_1\} \rightarrow h_1^s \eta^s \{^3S_1\}$  (purple). Dashed lines indicate one standard deviation statistical uncertainties.

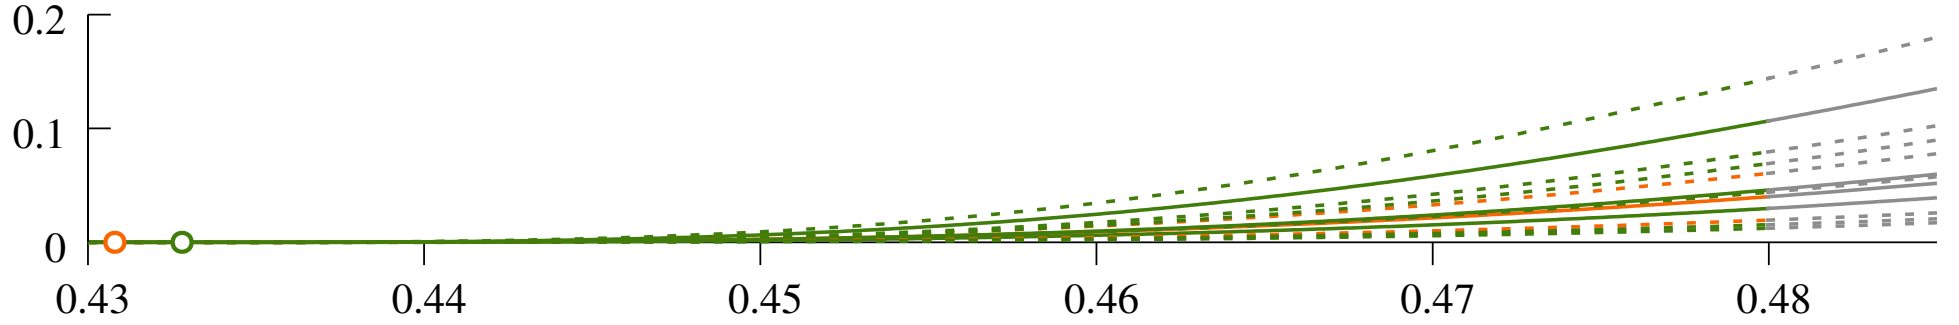

Figure 1.134: Similar to parts (e) and (f) of Figure 7 in the manuscript,  $\rho_a \rho_b |t_{ab}|^2$  as a function of  $a_t E_{cm}$  for  $\omega^s \omega^s \{^3P_1\} \rightarrow \omega^s \omega^s \{^3P_1\}$  (orange),  $\omega^1 \omega^s \{^1P_1, ^3P_1, ^5P_1\} \rightarrow \omega^s \omega^1 \{^1P_1, ^3P_1, ^5P_1\}$  (green). Dashed lines indicate one standard deviation statistical uncertainties.

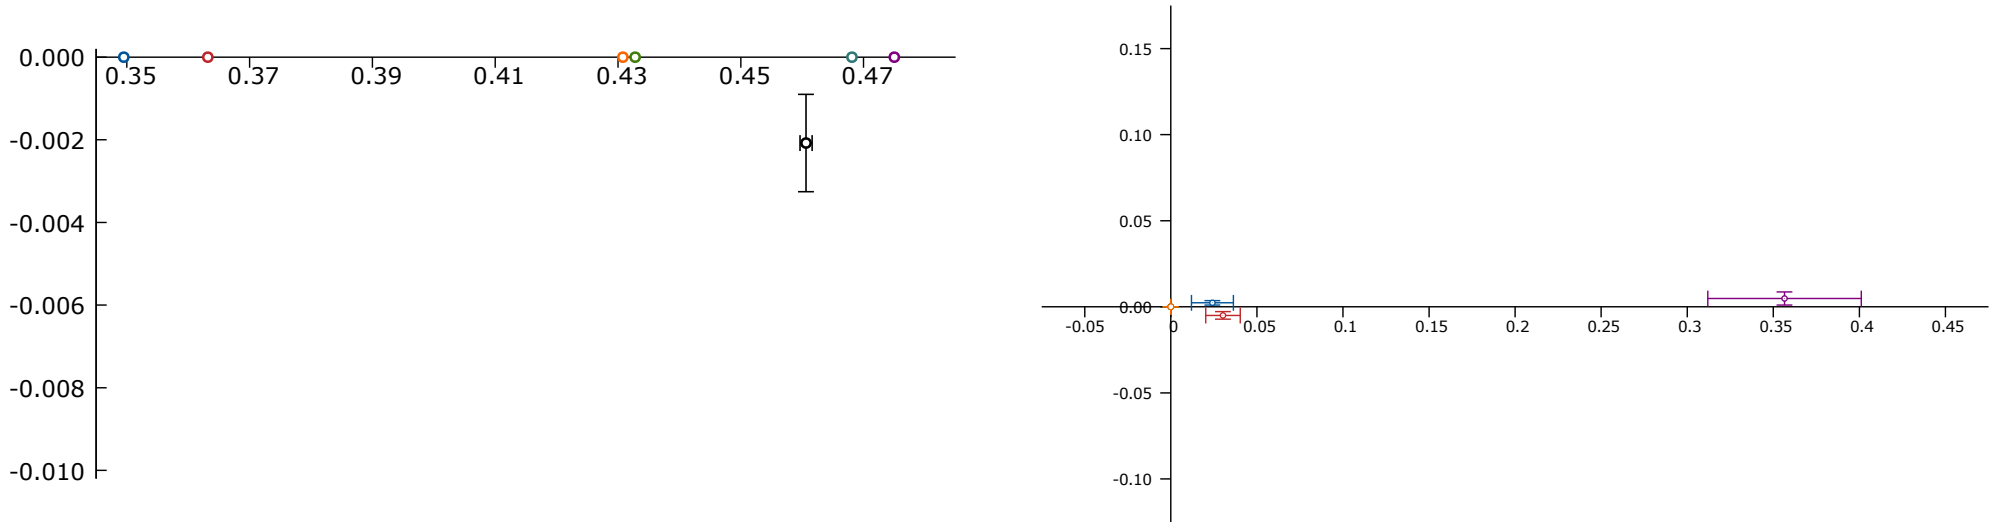

Figure 1.135: Left: Similar to Figure 13 in the manuscript, pole position on the proximal sheet (closest to physical scattering) with  $\text{Re}(a_t \sqrt{s})$  on the horizontal axis and  $2 \text{Im}(a_t \sqrt{s})$  on the vertical axis. Right: Similar to Figure 14 in the manuscript, the corresponding couplings with  $\text{Re}(a_t c)$  on the horizontal axis and  $\text{Im}(a_t c)$  on the vertical axis.
